# Supplementary material for: New graphical criterion for the selection of complete sets of polarization observables and its application to single-meson photoproduction as well as electroproduction
Source: arXiv:2106.00486 ancillary file (2021-10-21)
Supplement: Supplementary file 1 [file supplement.pdf]

# Supplemental material for the manuscript: 'New graphical criterion for the selection of complete sets of polarization observables and its application to single-meson photoproduction as well as electroproduction'

Y. Wunderlich[1, *]

[1] *Helmholtz-Institut für Strahlen- und Kernphysik, Universität Bonn, Germany*

(Dated: October 21, 2021)

This supplement collects the fully complete sets with minimal length $2N$ for both of the cases of single-meson photoproduction ($N = 4$ amplitudes) and electroproduction ($N = 6$ amplitudes), which have been obtained using our graphical criterion. For photoproduction, we evaluated 60 such complete sets (i.e. 20 complete sets derived from each of the 3 relevant graph-topologies), while for electroproduction we obtained a total of 1216 complete sets (i.e. 152 complete sets derived from each of the 8 relevant graph-topologies). Further details on the calculations can be found in the original manuscript.

## I. COMPLETE SETS FOR PSEUDOSCALAR MESON PHOTOPRODUCTION

TABLE I: All the fully complete sets determined from the combination of shape-classes $(b, c)$ (i.e. graph-topology 'I') in pseudoscalar meson photoproduction are listed here. The observables are written in the systematic symbolic notation $\mathcal{O}^{n}_{\nu\pm}$ by Nakayama [1], as well as in the more commonly used names (cf. reference [2]). The given sets of 4 observables have to be combined with the 4 'diagonal' observables $\left\{\sigma_0, \check{\Sigma}, \check{T}, \check{P}\right\}$ in order to form a complete set of minimal length $2N = 8$. All of these sets have been verified to be complete using Mathematica [3].

| Set-Nr. | Observables | | | |
|---|---|---|---|---|
| $(b,c):1$ | $\check{O}_{z'}$ | $\check{C}_{x'}$ | $\check{L}_{x'}$ | $\check{L}_{z'}$ |
| | $\mathcal{O}^{b}_{1+}$ | $\mathcal{O}^{b}_{1-}$ | $\mathcal{O}^{c}_{1+}$ | $\mathcal{O}^{c}_{2+}$ |
| $(b,c):2$ | $\check{O}_{z'}$ | $\check{C}_{x'}$ | $\check{T}_{z'}$ | $\check{T}_{x'}$ |
| | $\mathcal{O}^{b}_{1+}$ | $\mathcal{O}^{b}_{1-}$ | $\mathcal{O}^{c}_{1-}$ | $\mathcal{O}^{c}_{2-}$ |
| $(b,c):3$ | $\check{C}_{z'}$ | $\check{O}_{x'}$ | $\check{L}_{x'}$ | $\check{L}_{z'}$ |
| | $\mathcal{O}^{b}_{2+}$ | $\mathcal{O}^{b}_{2-}$ | $\mathcal{O}^{c}_{1+}$ | $\mathcal{O}^{c}_{2+}$ |
| $(b,c):4$ | $\check{C}_{z'}$ | $\check{O}_{x'}$ | $\check{T}_{z'}$ | $\check{T}_{x'}$ |
| | $\mathcal{O}^{b}_{2+}$ | $\mathcal{O}^{b}_{2-}$ | $\mathcal{O}^{c}_{1-}$ | $\mathcal{O}^{c}_{2-}$ |
| $(b,c):5$ | $\check{O}_{z'}$ | $\check{C}_{z'}$ | $\check{L}_{x'}$ | $\check{L}_{z'}$ |
| | $\mathcal{O}^{b}_{1+}$ | $\mathcal{O}^{b}_{2+}$ | $\mathcal{O}^{c}_{1+}$ | $\mathcal{O}^{c}_{2+}$ |
| $(b,c):6$ | $\check{O}_{z'}$ | $\check{C}_{z'}$ | $\check{T}_{z'}$ | $\check{T}_{x'}$ |
| | $\mathcal{O}^{b}_{1+}$ | $\mathcal{O}^{b}_{2+}$ | $\mathcal{O}^{c}_{1-}$ | $\mathcal{O}^{c}_{2-}$ |
| $(b,c):7$ | $\check{O}_{z'}$ | $\check{O}_{x'}$ | $\check{L}_{x'}$ | $\check{T}_{z'}$ |
| | $\mathcal{O}^{b}_{1+}$ | $\mathcal{O}^{b}_{2-}$ | $\mathcal{O}^{c}_{1+}$ | $\mathcal{O}^{c}_{1-}$ |
| $(b,c):8$ | $\check{O}_{z'}$ | $\check{O}_{x'}$ | $\check{L}_{z'}$ | $\check{T}_{x'}$ |
| | $\mathcal{O}^{b}_{1+}$ | $\mathcal{O}^{b}_{2-}$ | $\mathcal{O}^{c}_{2+}$ | $\mathcal{O}^{c}_{2-}$ |
| $(b,c):9$ | $\check{O}_{z'}$ | $\check{O}_{x'}$ | $\check{L}_{x'}$ | $\check{L}_{z'}$ |
| | $\mathcal{O}^{b}_{1+}$ | $\mathcal{O}^{b}_{2-}$ | $\mathcal{O}^{c}_{1+}$ | $\mathcal{O}^{c}_{2+}$ |
| $(b,c):10$ | $\check{O}_{z'}$ | $\check{O}_{x'}$ | $\check{L}_{x'}$ | $\check{T}_{x'}$ |
| | $\mathcal{O}^{b}_{1+}$ | $\mathcal{O}^{b}_{2-}$ | $\mathcal{O}^{c}_{1+}$ | $\mathcal{O}^{c}_{2-}$ |
| $(b,c):11$ | $\check{O}_{z'}$ | $\check{O}_{x'}$ | $\check{T}_{z'}$ | $\check{L}_{z'}$ |
| | $\mathcal{O}^{b}_{1+}$ | $\mathcal{O}^{b}_{2-}$ | $\mathcal{O}^{c}_{1-}$ | $\mathcal{O}^{c}_{2+}$ |
| $(b,c):12$ | $\check{O}_{z'}$ | $\check{O}_{x'}$ | $\check{T}_{z'}$ | $\check{T}_{x'}$ |
| | $\mathcal{O}^{b}_{1+}$ | $\mathcal{O}^{b}_{2-}$ | $\mathcal{O}^{c}_{1-}$ | $\mathcal{O}^{c}_{2-}$ |
| $(b,c):13$ | $\check{C}_{x'}$ | $\check{C}_{z'}$ | $\check{L}_{x'}$ | $\check{T}_{z'}$ |
| | $\mathcal{O}^{b}_{1-}$ | $\mathcal{O}^{b}_{2+}$ | $\mathcal{O}^{c}_{1+}$ | $\mathcal{O}^{c}_{1-}$ |

* Corresponding author: wunderlich@hiskp.uni-bonn.de

| | | | | |
|---|---|---|---|---|
| $(b,c):14$ | $\check{C}_{x'}$ | $\check{C}_{z'}$ | $\check{L}_{z'}$ | $\check{T}_{x'}$ |
| | $\mathcal{O}^{b}_{1-}$ | $\mathcal{O}^{b}_{2+}$ | $\mathcal{O}^{c}_{2+}$ | $\mathcal{O}^{c}_{2-}$ |
| $(b,c):15$ | $\check{C}_{x'}$ | $\check{C}_{z'}$ | $\check{L}_{x'}$ | $\check{L}_{z'}$ |
| | $\mathcal{O}^{b}_{1-}$ | $\mathcal{O}^{b}_{2+}$ | $\mathcal{O}^{c}_{1+}$ | $\mathcal{O}^{c}_{2+}$ |
| $(b,c):16$ | $\check{C}_{x'}$ | $\check{C}_{z'}$ | $\check{L}_{x'}$ | $\check{T}_{x'}$ |
| | $\mathcal{O}^{b}_{1-}$ | $\mathcal{O}^{b}_{2+}$ | $\mathcal{O}^{c}_{1+}$ | $\mathcal{O}^{c}_{2-}$ |
| $(b,c):17$ | $\check{C}_{x'}$ | $\check{C}_{z'}$ | $\check{T}_{z'}$ | $\check{L}_{z'}$ |
| | $\mathcal{O}^{b}_{1-}$ | $\mathcal{O}^{b}_{2+}$ | $\mathcal{O}^{c}_{1-}$ | $\mathcal{O}^{c}_{2+}$ |
| $(b,c):18$ | $\check{C}_{x'}$ | $\check{C}_{z'}$ | $\check{T}_{z'}$ | $\check{T}_{x'}$ |
| | $\mathcal{O}^{b}_{1-}$ | $\mathcal{O}^{b}_{2+}$ | $\mathcal{O}^{c}_{1-}$ | $\mathcal{O}^{c}_{2-}$ |
| $(b,c):19$ | $\check{C}_{x'}$ | $\check{O}_{x'}$ | $\check{L}_{x'}$ | $\check{L}_{z'}$ |
| | $\mathcal{O}^{b}_{1-}$ | $\mathcal{O}^{b}_{2-}$ | $\mathcal{O}^{c}_{1+}$ | $\mathcal{O}^{c}_{2+}$ |
| $(b,c):20$ | $\check{C}_{x'}$ | $\check{O}_{x'}$ | $\check{T}_{z'}$ | $\check{T}_{x'}$ |
| | $\mathcal{O}^{b}_{1-}$ | $\mathcal{O}^{b}_{2-}$ | $\mathcal{O}^{c}_{1-}$ | $\mathcal{O}^{c}_{2-}$ |

TABLE II: All the fully complete sets determined from the combination of shape-classes $(a,c)$ (i.e. graph-topology 'II') in pseudoscalar meson photoproduction are listed here. The observables are written in the systematic symbolic notation $\mathcal{O}^{n}_{\nu\pm}$ by Nakayama [1], as well as in the more commonly used names (cf. reference [2]). The given sets of 4 observables have to be combined with the 4 'diagonal' observables $\left\{\sigma_0, \check{\Sigma}, \check{T}, \check{P}\right\}$ in order to form a complete set of minimal length $2N = 8$. All of these sets have been verified to be complete using Mathematica [3].

| Set-Nr. | Observables | | | |
|---|---|---|---|---|
| $(a,c):1$ | $\check{G}$ | $\check{F}$ | $\check{L}_{x'}$ | $\check{T}_{x'}$ |
| | $\mathcal{O}^{a}_{1+}$ | $\mathcal{O}^{a}_{1-}$ | $\mathcal{O}^{c}_{1+}$ | $\mathcal{O}^{c}_{2-}$ |
| $(a,c):2$ | $\check{G}$ | $\check{F}$ | $\check{T}_{z'}$ | $\check{L}_{z'}$ |
| | $\mathcal{O}^{a}_{1+}$ | $\mathcal{O}^{a}_{1-}$ | $\mathcal{O}^{c}_{1-}$ | $\mathcal{O}^{c}_{2+}$ |
| $(a,c):3$ | $\check{E}$ | $\check{H}$ | $\check{L}_{x'}$ | $\check{T}_{x'}$ |
| | $\mathcal{O}^{a}_{2+}$ | $\mathcal{O}^{a}_{2-}$ | $\mathcal{O}^{c}_{1+}$ | $\mathcal{O}^{c}_{2-}$ |
| $(a,c):4$ | $\check{E}$ | $\check{H}$ | $\check{T}_{z'}$ | $\check{L}_{z'}$ |
| | $\mathcal{O}^{a}_{2+}$ | $\mathcal{O}^{a}_{2-}$ | $\mathcal{O}^{c}_{1-}$ | $\mathcal{O}^{c}_{2+}$ |
| $(a,c):5$ | $\check{G}$ | $\check{E}$ | $\check{L}_{x'}$ | $\check{T}_{x'}$ |
| | $\mathcal{O}^{a}_{1+}$ | $\mathcal{O}^{a}_{2+}$ | $\mathcal{O}^{c}_{1+}$ | $\mathcal{O}^{c}_{2-}$ |
| $(a,c):6$ | $\check{G}$ | $\check{E}$ | $\check{T}_{z'}$ | $\check{L}_{z'}$ |
| | $\mathcal{O}^{a}_{1+}$ | $\mathcal{O}^{a}_{2+}$ | $\mathcal{O}^{c}_{1-}$ | $\mathcal{O}^{c}_{2+}$ |
| $(a,c):7$ | $\check{G}$ | $\check{H}$ | $\check{L}_{x'}$ | $\check{T}_{z'}$ |
| | $\mathcal{O}^{a}_{1+}$ | $\mathcal{O}^{a}_{2-}$ | $\mathcal{O}^{c}_{1+}$ | $\mathcal{O}^{c}_{1-}$ |
| $(a,c):8$ | $\check{G}$ | $\check{H}$ | $\check{L}_{z'}$ | $\check{T}_{x'}$ |
| | $\mathcal{O}^{a}_{1+}$ | $\mathcal{O}^{a}_{2-}$ | $\mathcal{O}^{c}_{2+}$ | $\mathcal{O}^{c}_{2-}$ |
| $(a,c):9$ | $\check{G}$ | $\check{H}$ | $\check{L}_{x'}$ | $\check{L}_{z'}$ |
| | $\mathcal{O}^{a}_{1+}$ | $\mathcal{O}^{a}_{2-}$ | $\mathcal{O}^{c}_{1+}$ | $\mathcal{O}^{c}_{2+}$ |
| $(a,c):10$ | $\check{G}$ | $\check{H}$ | $\check{L}_{x'}$ | $\check{T}_{x'}$ |
| | $\mathcal{O}^{a}_{1+}$ | $\mathcal{O}^{a}_{2-}$ | $\mathcal{O}^{c}_{1+}$ | $\mathcal{O}^{c}_{2-}$ |
| $(a,c):11$ | $\check{G}$ | $\check{H}$ | $\check{T}_{z'}$ | $\check{L}_{z'}$ |
| | $\mathcal{O}^{a}_{1+}$ | $\mathcal{O}^{a}_{2-}$ | $\mathcal{O}^{c}_{1-}$ | $\mathcal{O}^{c}_{2+}$ |
| $(a,c):12$ | $\check{G}$ | $\check{H}$ | $\check{T}_{z'}$ | $\check{T}_{x'}$ |
| | $\mathcal{O}^{a}_{1+}$ | $\mathcal{O}^{a}_{2-}$ | $\mathcal{O}^{c}_{1-}$ | $\mathcal{O}^{c}_{2-}$ |
| $(a,c):13$ | $\check{F}$ | $\check{E}$ | $\check{L}_{x'}$ | $\check{T}_{z'}$ |
| | $\mathcal{O}^{a}_{1-}$ | $\mathcal{O}^{a}_{2+}$ | $\mathcal{O}^{c}_{1+}$ | $\mathcal{O}^{c}_{1-}$ |
| $(a,c):14$ | $\check{F}$ | $\check{E}$ | $\check{L}_{z'}$ | $\check{T}_{x'}$ |
| | $\mathcal{O}^{a}_{1-}$ | $\mathcal{O}^{a}_{2+}$ | $\mathcal{O}^{c}_{2+}$ | $\mathcal{O}^{c}_{2-}$ |
| $(a,c):15$ | $\check{F}$ | $\check{E}$ | $\check{L}_{x'}$ | $\check{L}_{z'}$ |
| | $\mathcal{O}^{a}_{1-}$ | $\mathcal{O}^{a}_{2+}$ | $\mathcal{O}^{c}_{1+}$ | $\mathcal{O}^{c}_{2+}$ |
| $(a,c):16$ | $\check{F}$ | $\check{E}$ | $\check{L}_{x'}$ | $\check{T}_{x'}$ |
| | $\mathcal{O}^{a}_{1-}$ | $\mathcal{O}^{a}_{2+}$ | $\mathcal{O}^{c}_{1+}$ | $\mathcal{O}^{c}_{2-}$ |
| $(a,c):17$ | $\check{F}$ | $\check{E}$ | $\check{T}_{z'}$ | $\check{L}_{z'}$ |
| | $\mathcal{O}^{a}_{1-}$ | $\mathcal{O}^{a}_{2+}$ | $\mathcal{O}^{c}_{1-}$ | $\mathcal{O}^{c}_{2+}$ |
| $(a,c):18$ | $\check{F}$ | $\check{E}$ | $\check{T}_{z'}$ | $\check{T}_{x'}$ |

| | | | | |
|---|---|---|---|---|
| | $\mathcal{O}^a_{1-}$ | $\mathcal{O}^a_{2+}$ | $\mathcal{O}^c_{1-}$ | $\mathcal{O}^c_{2-}$ |
| $(a,c):19$ | $\check{F}$ | $\check{H}$ | $\check{L}_{x'}$ | $\check{T}_{x'}$ |
| | $\mathcal{O}^a_{1-}$ | $\mathcal{O}^a_{2-}$ | $\mathcal{O}^c_{1+}$ | $\mathcal{O}^c_{2-}$ |
| $(a,c):20$ | $\check{F}$ | $\check{H}$ | $\check{T}_{z'}$ | $\check{L}_{z'}$ |
| | $\mathcal{O}^a_{1-}$ | $\mathcal{O}^a_{2-}$ | $\mathcal{O}^c_{1-}$ | $\mathcal{O}^c_{2+}$ |

TABLE III: All the fully complete sets determined from the combination of shape-classes $(a,b)$ (i.e. graph-topology 'III') in pseudoscalar meson photoproduction are listed here. The observables are written in the systematic symbolic notation $\mathcal{O}^n_{\nu\pm}$ by Nakayama [1], as well as in the more commonly used names (cf. reference [2]). The given sets of 4 observables have to be combined with the 4 'diagonal' observables $\left\{\sigma_0, \check{\Sigma}, \check{T}, \check{P}\right\}$ in order to form a complete set of minimal length $2N = 8$. All of these sets have been verified to be complete using Mathematica [3].

| Set-Nr. | Observables | | | |
|---|---|---|---|---|
| $(a,b):1$ | $\check{G}$ | $\check{F}$ | $\check{O}_{z'}$ | $\check{C}_{z'}$ |
| | $\mathcal{O}^a_{1+}$ | $\mathcal{O}^a_{1-}$ | $\mathcal{O}^b_{1+}$ | $\mathcal{O}^b_{2+}$ |
| $(a,b):2$ | $\check{G}$ | $\check{F}$ | $\check{C}_{x'}$ | $\check{O}_{x'}$ |
| | $\mathcal{O}^a_{1+}$ | $\mathcal{O}^a_{1-}$ | $\mathcal{O}^b_{1-}$ | $\mathcal{O}^b_{2-}$ |
| $(a,b):3$ | $\check{E}$ | $\check{H}$ | $\check{O}_{z'}$ | $\check{C}_{z'}$ |
| | $\mathcal{O}^a_{2+}$ | $\mathcal{O}^a_{2-}$ | $\mathcal{O}^b_{1+}$ | $\mathcal{O}^b_{2+}$ |
| $(a,b):4$ | $\check{E}$ | $\check{H}$ | $\check{C}_{x'}$ | $\check{O}_{x'}$ |
| | $\mathcal{O}^a_{2+}$ | $\mathcal{O}^a_{2-}$ | $\mathcal{O}^b_{1-}$ | $\mathcal{O}^b_{2-}$ |
| $(a,b):5$ | $\check{G}$ | $\check{E}$ | $\check{O}_{z'}$ | $\check{C}_{x'}$ |
| | $\mathcal{O}^a_{1+}$ | $\mathcal{O}^a_{2+}$ | $\mathcal{O}^b_{1+}$ | $\mathcal{O}^b_{1-}$ |
| $(a,b):6$ | $\check{G}$ | $\check{E}$ | $\check{C}_{z'}$ | $\check{O}_{x'}$ |
| | $\mathcal{O}^a_{1+}$ | $\mathcal{O}^a_{2+}$ | $\mathcal{O}^b_{2+}$ | $\mathcal{O}^b_{2-}$ |
| $(a,b):7$ | $\check{G}$ | $\check{E}$ | $\check{O}_{z'}$ | $\check{C}_{z'}$ |
| | $\mathcal{O}^a_{1+}$ | $\mathcal{O}^a_{2+}$ | $\mathcal{O}^b_{1+}$ | $\mathcal{O}^b_{2+}$ |
| $(a,b):8$ | $\check{G}$ | $\check{E}$ | $\check{O}_{z'}$ | $\check{O}_{x'}$ |
| | $\mathcal{O}^a_{1+}$ | $\mathcal{O}^a_{2+}$ | $\mathcal{O}^b_{1+}$ | $\mathcal{O}^b_{2-}$ |
| $(a,b):9$ | $\check{G}$ | $\check{E}$ | $\check{C}_{x'}$ | $\check{C}_{z'}$ |
| | $\mathcal{O}^a_{1+}$ | $\mathcal{O}^a_{2+}$ | $\mathcal{O}^b_{1-}$ | $\mathcal{O}^b_{2+}$ |
| $(a,b):10$ | $\check{G}$ | $\check{E}$ | $\check{C}_{x'}$ | $\check{O}_{x'}$ |
| | $\mathcal{O}^a_{1+}$ | $\mathcal{O}^a_{2+}$ | $\mathcal{O}^b_{1-}$ | $\mathcal{O}^b_{2-}$ |
| $(a,b):11$ | $\check{G}$ | $\check{H}$ | $\check{O}_{z'}$ | $\check{C}_{z'}$ |
| | $\mathcal{O}^a_{1+}$ | $\mathcal{O}^a_{2-}$ | $\mathcal{O}^b_{1+}$ | $\mathcal{O}^b_{2+}$ |
| $(a,b):12$ | $\check{G}$ | $\check{H}$ | $\check{C}_{x'}$ | $\check{O}_{x'}$ |
| | $\mathcal{O}^a_{1+}$ | $\mathcal{O}^a_{2-}$ | $\mathcal{O}^b_{1-}$ | $\mathcal{O}^b_{2-}$ |
| $(a,b):13$ | $\check{F}$ | $\check{E}$ | $\check{O}_{z'}$ | $\check{C}_{z'}$ |
| | $\mathcal{O}^a_{1-}$ | $\mathcal{O}^a_{2+}$ | $\mathcal{O}^b_{1+}$ | $\mathcal{O}^b_{2+}$ |
| $(a,b):14$ | $\check{F}$ | $\check{E}$ | $\check{C}_{x'}$ | $\check{O}_{x'}$ |
| | $\mathcal{O}^a_{1-}$ | $\mathcal{O}^a_{2+}$ | $\mathcal{O}^b_{1-}$ | $\mathcal{O}^b_{2-}$ |
| $(a,b):15$ | $\check{F}$ | $\check{H}$ | $\check{O}_{z'}$ | $\check{C}_{x'}$ |
| | $\mathcal{O}^a_{1-}$ | $\mathcal{O}^a_{2-}$ | $\mathcal{O}^b_{1+}$ | $\mathcal{O}^b_{1-}$ |
| $(a,b):16$ | $\check{F}$ | $\check{H}$ | $\check{C}_{z'}$ | $\check{O}_{x'}$ |
| | $\mathcal{O}^a_{1-}$ | $\mathcal{O}^a_{2-}$ | $\mathcal{O}^b_{2+}$ | $\mathcal{O}^b_{2-}$ |
| $(a,b):17$ | $\check{F}$ | $\check{H}$ | $\check{O}_{z'}$ | $\check{C}_{z'}$ |
| | $\mathcal{O}^a_{1-}$ | $\mathcal{O}^a_{2-}$ | $\mathcal{O}^b_{1+}$ | $\mathcal{O}^b_{2+}$ |
| $(a,b):18$ | $\check{F}$ | $\check{H}$ | $\check{O}_{z'}$ | $\check{O}_{x'}$ |
| | $\mathcal{O}^a_{1-}$ | $\mathcal{O}^a_{2-}$ | $\mathcal{O}^b_{1+}$ | $\mathcal{O}^b_{2-}$ |
| $(a,b):19$ | $\check{F}$ | $\check{H}$ | $\check{C}_{x'}$ | $\check{C}_{z'}$ |
| | $\mathcal{O}^a_{1-}$ | $\mathcal{O}^a_{2-}$ | $\mathcal{O}^b_{1-}$ | $\mathcal{O}^b_{2+}$ |
| $(a,b):20$ | $\check{F}$ | $\check{H}$ | $\check{C}_{x'}$ | $\check{O}_{x'}$ |
| | $\mathcal{O}^a_{1-}$ | $\mathcal{O}^a_{2-}$ | $\mathcal{O}^b_{1-}$ | $\mathcal{O}^b_{2-}$ |

## II. COMPLETE SETS FOR PSEUDOSCALAR MESON ELECTROPRODUCTION

TABLE IV: All the fully complete sets determined from the combination of shape-classes $(a, e, g)$ (i.e. graph-topology 'I') in the case of pseudoscalar meson electroproduction are listed here. The observables are written in the systematic symbolic notation $\mathcal{O}^{n}_{\nu\pm}$ by Nakayama [1], as well as in the more commonly used used notation in terms of 'response-functions' $R_{i}^{\beta\alpha}$ (cf. references [4, 5]). The given sets of 6 observables have to be combined with the 6 'diagonal' observables $\left\{R_{T}^{00}, {}^{c}R_{TT}^{00}, R_{T}^{0y}, R_{T}^{y'0}, R_{L}^{00}, R_{L}^{0y}\right\}$ in order to form a complete set of minimal length $2N = 12$. All of these sets have been verified to be complete using Mathematica [3].

| Set-Nr. | Observables | | | | | |
|---|---|---|---|---|---|---|
| $(a, e, g) : 1$ | ${}^{s}R_{TT}^{0z}$ | $R_{TT'}^{0x}$ | ${}^{s}R_{LT'}^{00}$ | ${}^{s}R_{LT'}^{0y}$ | ${}^{s}R_{LT}^{z'0}$ | ${}^{c}R_{LT'}^{z'0}$ |
| | $\mathcal{O}^{a}_{1+}$ | $\mathcal{O}^{a}_{1-}$ | $\mathcal{O}^{e}_{1+}$ | $\mathcal{O}^{e}_{1-}$ | $\mathcal{O}^{g}_{1+}$ | $\mathcal{O}^{g}_{2+}$ |
| $(a, e, g) : 2$ | ${}^{s}R_{TT}^{0z}$ | $R_{TT'}^{0x}$ | ${}^{s}R_{LT'}^{00}$ | ${}^{s}R_{LT'}^{0y}$ | ${}^{c}R_{LT'}^{x'0}$ | ${}^{s}R_{LT}^{x'0}$ |
| | $\mathcal{O}^{a}_{1+}$ | $\mathcal{O}^{a}_{1-}$ | $\mathcal{O}^{e}_{1+}$ | $\mathcal{O}^{e}_{1-}$ | $\mathcal{O}^{g}_{1-}$ | $\mathcal{O}^{g}_{2-}$ |
| $(a, e, g) : 3$ | ${}^{s}R_{TT}^{0z}$ | $R_{TT'}^{0x}$ | ${}^{c}R_{LT}^{00}$ | ${}^{c}R_{LT}^{0y}$ | ${}^{s}R_{LT}^{z'0}$ | ${}^{c}R_{LT'}^{z'0}$ |
| | $\mathcal{O}^{a}_{1+}$ | $\mathcal{O}^{a}_{1-}$ | $\mathcal{O}^{e}_{2+}$ | $\mathcal{O}^{e}_{2-}$ | $\mathcal{O}^{g}_{1+}$ | $\mathcal{O}^{g}_{2+}$ |
| $(a, e, g) : 4$ | ${}^{s}R_{TT}^{0z}$ | $R_{TT'}^{0x}$ | ${}^{c}R_{LT}^{00}$ | ${}^{c}R_{LT}^{0y}$ | ${}^{c}R_{LT'}^{x'0}$ | ${}^{s}R_{LT}^{x'0}$ |
| | $\mathcal{O}^{a}_{1+}$ | $\mathcal{O}^{a}_{1-}$ | $\mathcal{O}^{e}_{2+}$ | $\mathcal{O}^{e}_{2-}$ | $\mathcal{O}^{g}_{1-}$ | $\mathcal{O}^{g}_{2-}$ |
| $(a, e, g) : 5$ | ${}^{s}R_{TT}^{0z}$ | $R_{TT'}^{0x}$ | ${}^{s}R_{LT'}^{00}$ | ${}^{c}R_{LT}^{00}$ | ${}^{s}R_{LT}^{z'0}$ | ${}^{c}R_{LT'}^{x'0}$ |
| | $\mathcal{O}^{a}_{1+}$ | $\mathcal{O}^{a}_{1-}$ | $\mathcal{O}^{e}_{1+}$ | $\mathcal{O}^{e}_{2+}$ | $\mathcal{O}^{g}_{1+}$ | $\mathcal{O}^{g}_{1-}$ |
| $(a, e, g) : 6$ | ${}^{s}R_{TT}^{0z}$ | $R_{TT'}^{0x}$ | ${}^{s}R_{LT'}^{00}$ | ${}^{c}R_{LT}^{00}$ | ${}^{c}R_{LT'}^{z'0}$ | ${}^{s}R_{LT}^{x'0}$ |
| | $\mathcal{O}^{a}_{1+}$ | $\mathcal{O}^{a}_{1-}$ | $\mathcal{O}^{e}_{1+}$ | $\mathcal{O}^{e}_{2+}$ | $\mathcal{O}^{g}_{2+}$ | $\mathcal{O}^{g}_{2-}$ |
| $(a, e, g) : 7$ | ${}^{s}R_{TT}^{0z}$ | $R_{TT'}^{0x}$ | ${}^{s}R_{LT'}^{00}$ | ${}^{c}R_{LT}^{00}$ | ${}^{s}R_{LT}^{z'0}$ | ${}^{c}R_{LT'}^{z'0}$ |
| | $\mathcal{O}^{a}_{1+}$ | $\mathcal{O}^{a}_{1-}$ | $\mathcal{O}^{e}_{1+}$ | $\mathcal{O}^{e}_{2+}$ | $\mathcal{O}^{g}_{1+}$ | $\mathcal{O}^{g}_{2+}$ |
| $(a, e, g) : 8$ | ${}^{s}R_{TT}^{0z}$ | $R_{TT'}^{0x}$ | ${}^{s}R_{LT'}^{00}$ | ${}^{c}R_{LT}^{00}$ | ${}^{s}R_{LT}^{z'0}$ | ${}^{s}R_{LT}^{x'0}$ |
| | $\mathcal{O}^{a}_{1+}$ | $\mathcal{O}^{a}_{1-}$ | $\mathcal{O}^{e}_{1+}$ | $\mathcal{O}^{e}_{2+}$ | $\mathcal{O}^{g}_{1+}$ | $\mathcal{O}^{g}_{2-}$ |
| $(a, e, g) : 9$ | ${}^{s}R_{TT}^{0z}$ | $R_{TT'}^{0x}$ | ${}^{s}R_{LT'}^{00}$ | ${}^{c}R_{LT}^{00}$ | ${}^{c}R_{LT'}^{x'0}$ | ${}^{c}R_{LT'}^{z'0}$ |
| | $\mathcal{O}^{a}_{1+}$ | $\mathcal{O}^{a}_{1-}$ | $\mathcal{O}^{e}_{1+}$ | $\mathcal{O}^{e}_{2+}$ | $\mathcal{O}^{g}_{1-}$ | $\mathcal{O}^{g}_{2+}$ |
| $(a, e, g) : 10$ | ${}^{s}R_{TT}^{0z}$ | $R_{TT'}^{0x}$ | ${}^{s}R_{LT'}^{00}$ | ${}^{c}R_{LT}^{00}$ | ${}^{c}R_{LT'}^{x'0}$ | ${}^{s}R_{LT}^{x'0}$ |
| | $\mathcal{O}^{a}_{1+}$ | $\mathcal{O}^{a}_{1-}$ | $\mathcal{O}^{e}_{1+}$ | $\mathcal{O}^{e}_{2+}$ | $\mathcal{O}^{g}_{1-}$ | $\mathcal{O}^{g}_{2-}$ |
| $(a, e, g) : 11$ | ${}^{s}R_{TT}^{0z}$ | $R_{TT'}^{0x}$ | ${}^{s}R_{LT'}^{00}$ | ${}^{c}R_{LT}^{0y}$ | ${}^{s}R_{LT}^{z'0}$ | ${}^{c}R_{LT'}^{z'0}$ |
| | $\mathcal{O}^{a}_{1+}$ | $\mathcal{O}^{a}_{1-}$ | $\mathcal{O}^{e}_{1+}$ | $\mathcal{O}^{e}_{2-}$ | $\mathcal{O}^{g}_{1+}$ | $\mathcal{O}^{g}_{2+}$ |
| $(a, e, g) : 12$ | ${}^{s}R_{TT}^{0z}$ | $R_{TT'}^{0x}$ | ${}^{s}R_{LT'}^{00}$ | ${}^{c}R_{LT}^{0y}$ | ${}^{c}R_{LT'}^{x'0}$ | ${}^{s}R_{LT}^{x'0}$ |
| | $\mathcal{O}^{a}_{1+}$ | $\mathcal{O}^{a}_{1-}$ | $\mathcal{O}^{e}_{1+}$ | $\mathcal{O}^{e}_{2-}$ | $\mathcal{O}^{g}_{1-}$ | $\mathcal{O}^{g}_{2-}$ |
| $(a, e, g) : 13$ | ${}^{s}R_{TT}^{0z}$ | $R_{TT'}^{0x}$ | ${}^{s}R_{LT'}^{0y}$ | ${}^{c}R_{LT}^{00}$ | ${}^{s}R_{LT}^{z'0}$ | ${}^{c}R_{LT'}^{z'0}$ |
| | $\mathcal{O}^{a}_{1+}$ | $\mathcal{O}^{a}_{1-}$ | $\mathcal{O}^{e}_{1-}$ | $\mathcal{O}^{e}_{2+}$ | $\mathcal{O}^{g}_{1+}$ | $\mathcal{O}^{g}_{2+}$ |
| $(a, e, g) : 14$ | ${}^{s}R_{TT}^{0z}$ | $R_{TT'}^{0x}$ | ${}^{s}R_{LT'}^{0y}$ | ${}^{c}R_{LT}^{00}$ | ${}^{c}R_{LT'}^{x'0}$ | ${}^{s}R_{LT}^{x'0}$ |
| | $\mathcal{O}^{a}_{1+}$ | $\mathcal{O}^{a}_{1-}$ | $\mathcal{O}^{e}_{1-}$ | $\mathcal{O}^{e}_{2+}$ | $\mathcal{O}^{g}_{1-}$ | $\mathcal{O}^{g}_{2-}$ |
| $(a, e, g) : 15$ | ${}^{s}R_{TT}^{0z}$ | $R_{TT'}^{0x}$ | ${}^{s}R_{LT'}^{0y}$ | ${}^{c}R_{LT}^{0y}$ | ${}^{s}R_{LT}^{z'0}$ | ${}^{c}R_{LT'}^{x'0}$ |
| | $\mathcal{O}^{a}_{1+}$ | $\mathcal{O}^{a}_{1-}$ | $\mathcal{O}^{e}_{1-}$ | $\mathcal{O}^{e}_{2-}$ | $\mathcal{O}^{g}_{1+}$ | $\mathcal{O}^{g}_{1-}$ |
| $(a, e, g) : 16$ | ${}^{s}R_{TT}^{0z}$ | $R_{TT'}^{0x}$ | ${}^{s}R_{LT'}^{0y}$ | ${}^{c}R_{LT}^{0y}$ | ${}^{c}R_{LT'}^{z'0}$ | ${}^{s}R_{LT}^{x'0}$ |
| | $\mathcal{O}^{a}_{1+}$ | $\mathcal{O}^{a}_{1-}$ | $\mathcal{O}^{e}_{1-}$ | $\mathcal{O}^{e}_{2-}$ | $\mathcal{O}^{g}_{2+}$ | $\mathcal{O}^{g}_{2-}$ |
| $(a, e, g) : 17$ | ${}^{s}R_{TT}^{0z}$ | $R_{TT'}^{0x}$ | ${}^{s}R_{LT'}^{0y}$ | ${}^{c}R_{LT}^{0y}$ | ${}^{s}R_{LT}^{z'0}$ | ${}^{c}R_{LT'}^{z'0}$ |
| | $\mathcal{O}^{a}_{1+}$ | $\mathcal{O}^{a}_{1-}$ | $\mathcal{O}^{e}_{1-}$ | $\mathcal{O}^{e}_{2-}$ | $\mathcal{O}^{g}_{1+}$ | $\mathcal{O}^{g}_{2+}$ |
| $(a, e, g) : 18$ | ${}^{s}R_{TT}^{0z}$ | $R_{TT'}^{0x}$ | ${}^{s}R_{LT'}^{0y}$ | ${}^{c}R_{LT}^{0y}$ | ${}^{s}R_{LT}^{z'0}$ | ${}^{s}R_{LT}^{x'0}$ |
| | $\mathcal{O}^{a}_{1+}$ | $\mathcal{O}^{a}_{1-}$ | $\mathcal{O}^{e}_{1-}$ | $\mathcal{O}^{e}_{2-}$ | $\mathcal{O}^{g}_{1+}$ | $\mathcal{O}^{g}_{2-}$ |
| $(a, e, g) : 19$ | ${}^{s}R_{TT}^{0z}$ | $R_{TT'}^{0x}$ | ${}^{s}R_{LT'}^{0y}$ | ${}^{c}R_{LT}^{0y}$ | ${}^{c}R_{LT'}^{x'0}$ | ${}^{c}R_{LT'}^{z'0}$ |
| | $\mathcal{O}^{a}_{1+}$ | $\mathcal{O}^{a}_{1-}$ | $\mathcal{O}^{e}_{1-}$ | $\mathcal{O}^{e}_{2-}$ | $\mathcal{O}^{g}_{1-}$ | $\mathcal{O}^{g}_{2+}$ |
| $(a, e, g) : 20$ | ${}^{s}R_{TT}^{0z}$ | $R_{TT'}^{0x}$ | ${}^{s}R_{LT'}^{0y}$ | ${}^{c}R_{LT}^{0y}$ | ${}^{c}R_{LT'}^{x'0}$ | ${}^{s}R_{LT}^{x'0}$ |
| | $\mathcal{O}^{a}_{1+}$ | $\mathcal{O}^{a}_{1-}$ | $\mathcal{O}^{e}_{1-}$ | $\mathcal{O}^{e}_{2-}$ | $\mathcal{O}^{g}_{1-}$ | $\mathcal{O}^{g}_{2-}$ |
| $(a, e, g) : 21$ | $R_{TT'}^{0z}$ | ${}^{s}R_{TT}^{0x}$ | ${}^{s}R_{LT'}^{00}$ | ${}^{s}R_{LT'}^{0y}$ | ${}^{s}R_{LT}^{z'0}$ | ${}^{c}R_{LT'}^{z'0}$ |
| | $\mathcal{O}^{a}_{2+}$ | $\mathcal{O}^{a}_{2-}$ | $\mathcal{O}^{e}_{1+}$ | $\mathcal{O}^{e}_{1-}$ | $\mathcal{O}^{g}_{1+}$ | $\mathcal{O}^{g}_{2+}$ |
| $(a, e, g) : 22$ | $R_{TT'}^{0z}$ | ${}^{s}R_{TT}^{0x}$ | ${}^{s}R_{LT'}^{00}$ | ${}^{s}R_{LT'}^{0y}$ | ${}^{c}R_{LT'}^{x'0}$ | ${}^{s}R_{LT}^{x'0}$ |
| | $\mathcal{O}^{a}_{2+}$ | $\mathcal{O}^{a}_{2-}$ | $\mathcal{O}^{e}_{1+}$ | $\mathcal{O}^{e}_{1-}$ | $\mathcal{O}^{g}_{1-}$ | $\mathcal{O}^{g}_{2-}$ |
| $(a, e, g) : 23$ | $R_{TT'}^{0z}$ | ${}^{s}R_{TT}^{0x}$ | ${}^{c}R_{LT}^{00}$ | ${}^{c}R_{LT}^{0y}$ | ${}^{s}R_{LT}^{z'0}$ | ${}^{c}R_{LT'}^{z'0}$ |

| | | | | | | |
|---|---|---|---|---|---|---|
| | $\mathcal{O}^a_{2+}$ | $\mathcal{O}^a_{2-}$ | $\mathcal{O}^e_{2+}$ | $\mathcal{O}^e_{2-}$ | $\mathcal{O}^g_{1+}$ | $\mathcal{O}^g_{2+}$ |
| $(a,e,g):24$ | $R^{0z}_{TT'}$ | ${}^{s}R^{0x}_{TT}$ | ${}^{c}R^{00}_{LT}$ | ${}^{c}R^{0y}_{LT}$ | ${}^{c}R^{x'0}_{LT'}$ | ${}^{s}R^{x'0}_{LT}$ |
| | $\mathcal{O}^a_{2+}$ | $\mathcal{O}^a_{2-}$ | $\mathcal{O}^e_{2+}$ | $\mathcal{O}^e_{2-}$ | $\mathcal{O}^g_{1-}$ | $\mathcal{O}^g_{2-}$ |
| $(a,e,g):25$ | $R^{0z}_{TT'}$ | ${}^{s}R^{0x}_{TT}$ | ${}^{s}R^{00}_{LT'}$ | ${}^{c}R^{00}_{LT}$ | ${}^{s}R^{z'0}_{LT}$ | ${}^{c}R^{x'0}_{LT'}$ |
| | $\mathcal{O}^a_{2+}$ | $\mathcal{O}^a_{2-}$ | $\mathcal{O}^e_{1+}$ | $\mathcal{O}^e_{2+}$ | $\mathcal{O}^g_{1+}$ | $\mathcal{O}^g_{1-}$ |
| $(a,e,g):26$ | $R^{0z}_{TT'}$ | ${}^{s}R^{0x}_{TT}$ | ${}^{s}R^{00}_{LT'}$ | ${}^{c}R^{00}_{LT}$ | ${}^{c}R^{z'0}_{LT'}$ | ${}^{s}R^{x'0}_{LT}$ |
| | $\mathcal{O}^a_{2+}$ | $\mathcal{O}^a_{2-}$ | $\mathcal{O}^e_{1+}$ | $\mathcal{O}^e_{2+}$ | $\mathcal{O}^g_{2+}$ | $\mathcal{O}^g_{2-}$ |
| $(a,e,g):27$ | $R^{0z}_{TT'}$ | ${}^{s}R^{0x}_{TT}$ | ${}^{s}R^{00}_{LT'}$ | ${}^{c}R^{00}_{LT}$ | ${}^{s}R^{z'0}_{LT}$ | ${}^{c}R^{z'0}_{LT'}$ |
| | $\mathcal{O}^a_{2+}$ | $\mathcal{O}^a_{2-}$ | $\mathcal{O}^e_{1+}$ | $\mathcal{O}^e_{2+}$ | $\mathcal{O}^g_{1+}$ | $\mathcal{O}^g_{2+}$ |
| $(a,e,g):28$ | $R^{0z}_{TT'}$ | ${}^{s}R^{0x}_{TT}$ | ${}^{s}R^{00}_{LT'}$ | ${}^{c}R^{00}_{LT}$ | ${}^{s}R^{z'0}_{LT}$ | ${}^{s}R^{x'0}_{LT}$ |
| | $\mathcal{O}^a_{2+}$ | $\mathcal{O}^a_{2-}$ | $\mathcal{O}^e_{1+}$ | $\mathcal{O}^e_{2+}$ | $\mathcal{O}^g_{1+}$ | $\mathcal{O}^g_{2-}$ |
| $(a,e,g):29$ | $R^{0z}_{TT'}$ | ${}^{s}R^{0x}_{TT}$ | ${}^{s}R^{00}_{LT'}$ | ${}^{c}R^{00}_{LT}$ | ${}^{c}R^{x'0}_{LT'}$ | ${}^{c}R^{z'0}_{LT'}$ |
| | $\mathcal{O}^a_{2+}$ | $\mathcal{O}^a_{2-}$ | $\mathcal{O}^e_{1+}$ | $\mathcal{O}^e_{2+}$ | $\mathcal{O}^g_{1-}$ | $\mathcal{O}^g_{2+}$ |
| $(a,e,g):30$ | $R^{0z}_{TT'}$ | ${}^{s}R^{0x}_{TT}$ | ${}^{s}R^{00}_{LT'}$ | ${}^{c}R^{00}_{LT}$ | ${}^{c}R^{x'0}_{LT'}$ | ${}^{s}R^{x'0}_{LT}$ |
| | $\mathcal{O}^a_{2+}$ | $\mathcal{O}^a_{2-}$ | $\mathcal{O}^e_{1+}$ | $\mathcal{O}^e_{2+}$ | $\mathcal{O}^g_{1-}$ | $\mathcal{O}^g_{2-}$ |
| $(a,e,g):31$ | $R^{0z}_{TT'}$ | ${}^{s}R^{0x}_{TT}$ | ${}^{s}R^{00}_{LT'}$ | ${}^{c}R^{0y}_{LT}$ | ${}^{s}R^{z'0}_{LT}$ | ${}^{c}R^{z'0}_{LT'}$ |
| | $\mathcal{O}^a_{2+}$ | $\mathcal{O}^a_{2-}$ | $\mathcal{O}^e_{1+}$ | $\mathcal{O}^e_{2-}$ | $\mathcal{O}^g_{1+}$ | $\mathcal{O}^g_{2+}$ |
| $(a,e,g):32$ | $R^{0z}_{TT'}$ | ${}^{s}R^{0x}_{TT}$ | ${}^{s}R^{00}_{LT'}$ | ${}^{c}R^{0y}_{LT}$ | ${}^{c}R^{x'0}_{LT'}$ | ${}^{s}R^{x'0}_{LT}$ |
| | $\mathcal{O}^a_{2+}$ | $\mathcal{O}^a_{2-}$ | $\mathcal{O}^e_{1+}$ | $\mathcal{O}^e_{2-}$ | $\mathcal{O}^g_{1-}$ | $\mathcal{O}^g_{2-}$ |
| $(a,e,g):33$ | $R^{0z}_{TT'}$ | ${}^{s}R^{0x}_{TT}$ | ${}^{s}R^{0y}_{LT'}$ | ${}^{c}R^{00}_{LT}$ | ${}^{s}R^{z'0}_{LT}$ | ${}^{c}R^{z'0}_{LT'}$ |
| | $\mathcal{O}^a_{2+}$ | $\mathcal{O}^a_{2-}$ | $\mathcal{O}^e_{1-}$ | $\mathcal{O}^e_{2+}$ | $\mathcal{O}^g_{1+}$ | $\mathcal{O}^g_{2+}$ |
| $(a,e,g):34$ | $R^{0z}_{TT'}$ | ${}^{s}R^{0x}_{TT}$ | ${}^{s}R^{0y}_{LT'}$ | ${}^{c}R^{00}_{LT}$ | ${}^{c}R^{x'0}_{LT'}$ | ${}^{s}R^{x'0}_{LT}$ |
| | $\mathcal{O}^a_{2+}$ | $\mathcal{O}^a_{2-}$ | $\mathcal{O}^e_{1-}$ | $\mathcal{O}^e_{2+}$ | $\mathcal{O}^g_{1-}$ | $\mathcal{O}^g_{2-}$ |
| $(a,e,g):35$ | $R^{0z}_{TT'}$ | ${}^{s}R^{0x}_{TT}$ | ${}^{s}R^{0y}_{LT'}$ | ${}^{c}R^{0y}_{LT}$ | ${}^{s}R^{z'0}_{LT}$ | ${}^{c}R^{x'0}_{LT'}$ |
| | $\mathcal{O}^a_{2+}$ | $\mathcal{O}^a_{2-}$ | $\mathcal{O}^e_{1-}$ | $\mathcal{O}^e_{2-}$ | $\mathcal{O}^g_{1+}$ | $\mathcal{O}^g_{1-}$ |
| $(a,e,g):36$ | $R^{0z}_{TT'}$ | ${}^{s}R^{0x}_{TT}$ | ${}^{s}R^{0y}_{LT'}$ | ${}^{c}R^{0y}_{LT}$ | ${}^{c}R^{z'0}_{LT'}$ | ${}^{s}R^{x'0}_{LT}$ |
| | $\mathcal{O}^a_{2+}$ | $\mathcal{O}^a_{2-}$ | $\mathcal{O}^e_{1-}$ | $\mathcal{O}^e_{2-}$ | $\mathcal{O}^g_{2+}$ | $\mathcal{O}^g_{2-}$ |
| $(a,e,g):37$ | $R^{0z}_{TT'}$ | ${}^{s}R^{0x}_{TT}$ | ${}^{s}R^{0y}_{LT'}$ | ${}^{c}R^{0y}_{LT}$ | ${}^{s}R^{z'0}_{LT}$ | ${}^{c}R^{z'0}_{LT'}$ |
| | $\mathcal{O}^a_{2+}$ | $\mathcal{O}^a_{2-}$ | $\mathcal{O}^e_{1-}$ | $\mathcal{O}^e_{2-}$ | $\mathcal{O}^g_{1+}$ | $\mathcal{O}^g_{2+}$ |
| $(a,e,g):38$ | $R^{0z}_{TT'}$ | ${}^{s}R^{0x}_{TT}$ | ${}^{s}R^{0y}_{LT'}$ | ${}^{c}R^{0y}_{LT}$ | ${}^{s}R^{z'0}_{LT}$ | ${}^{s}R^{x'0}_{LT}$ |
| | $\mathcal{O}^a_{2+}$ | $\mathcal{O}^a_{2-}$ | $\mathcal{O}^e_{1-}$ | $\mathcal{O}^e_{2-}$ | $\mathcal{O}^g_{1+}$ | $\mathcal{O}^g_{2-}$ |
| $(a,e,g):39$ | $R^{0z}_{TT'}$ | ${}^{s}R^{0x}_{TT}$ | ${}^{s}R^{0y}_{LT'}$ | ${}^{c}R^{0y}_{LT}$ | ${}^{c}R^{x'0}_{LT'}$ | ${}^{c}R^{z'0}_{LT'}$ |
| | $\mathcal{O}^a_{2+}$ | $\mathcal{O}^a_{2-}$ | $\mathcal{O}^e_{1-}$ | $\mathcal{O}^e_{2-}$ | $\mathcal{O}^g_{1-}$ | $\mathcal{O}^g_{2+}$ |
| $(a,e,g):40$ | $R^{0z}_{TT'}$ | ${}^{s}R^{0x}_{TT}$ | ${}^{s}R^{0y}_{LT'}$ | ${}^{c}R^{0y}_{LT}$ | ${}^{c}R^{x'0}_{LT'}$ | ${}^{s}R^{x'0}_{LT}$ |
| | $\mathcal{O}^a_{2+}$ | $\mathcal{O}^a_{2-}$ | $\mathcal{O}^e_{1-}$ | $\mathcal{O}^e_{2-}$ | $\mathcal{O}^g_{1-}$ | $\mathcal{O}^g_{2-}$ |
| $(a,e,g):41$ | ${}^{s}R^{0z}_{TT}$ | $R^{0z}_{TT'}$ | ${}^{s}R^{00}_{LT'}$ | ${}^{s}R^{0y}_{LT'}$ | ${}^{s}R^{z'0}_{LT}$ | ${}^{c}R^{x'0}_{LT'}$ |
| | $\mathcal{O}^a_{1+}$ | $\mathcal{O}^a_{2+}$ | $\mathcal{O}^e_{1+}$ | $\mathcal{O}^e_{1-}$ | $\mathcal{O}^g_{1+}$ | $\mathcal{O}^g_{1-}$ |
| $(a,e,g):42$ | ${}^{s}R^{0z}_{TT}$ | $R^{0z}_{TT'}$ | ${}^{s}R^{00}_{LT'}$ | ${}^{s}R^{0y}_{LT'}$ | ${}^{c}R^{z'0}_{LT'}$ | ${}^{s}R^{x'0}_{LT}$ |
| | $\mathcal{O}^a_{1+}$ | $\mathcal{O}^a_{2+}$ | $\mathcal{O}^e_{1+}$ | $\mathcal{O}^e_{1-}$ | $\mathcal{O}^g_{2+}$ | $\mathcal{O}^g_{2-}$ |
| $(a,e,g):43$ | ${}^{s}R^{0z}_{TT}$ | $R^{0z}_{TT'}$ | ${}^{s}R^{00}_{LT'}$ | ${}^{s}R^{0y}_{LT'}$ | ${}^{s}R^{z'0}_{LT}$ | ${}^{c}R^{z'0}_{LT'}$ |
| | $\mathcal{O}^a_{1+}$ | $\mathcal{O}^a_{2+}$ | $\mathcal{O}^e_{1+}$ | $\mathcal{O}^e_{1-}$ | $\mathcal{O}^g_{1+}$ | $\mathcal{O}^g_{2+}$ |
| $(a,e,g):44$ | ${}^{s}R^{0z}_{TT}$ | $R^{0z}_{TT'}$ | ${}^{s}R^{00}_{LT'}$ | ${}^{s}R^{0y}_{LT'}$ | ${}^{s}R^{z'0}_{LT}$ | ${}^{s}R^{x'0}_{LT}$ |
| | $\mathcal{O}^a_{1+}$ | $\mathcal{O}^a_{2+}$ | $\mathcal{O}^e_{1+}$ | $\mathcal{O}^e_{1-}$ | $\mathcal{O}^g_{1+}$ | $\mathcal{O}^g_{2-}$ |
| $(a,e,g):45$ | ${}^{s}R^{0z}_{TT}$ | $R^{0z}_{TT'}$ | ${}^{s}R^{00}_{LT'}$ | ${}^{s}R^{0y}_{LT'}$ | ${}^{c}R^{x'0}_{LT'}$ | ${}^{c}R^{z'0}_{LT'}$ |
| | $\mathcal{O}^a_{1+}$ | $\mathcal{O}^a_{2+}$ | $\mathcal{O}^e_{1+}$ | $\mathcal{O}^e_{1-}$ | $\mathcal{O}^g_{1-}$ | $\mathcal{O}^g_{2+}$ |
| $(a,e,g):46$ | ${}^{s}R^{0z}_{TT}$ | $R^{0z}_{TT'}$ | ${}^{s}R^{00}_{LT'}$ | ${}^{s}R^{0y}_{LT'}$ | ${}^{c}R^{x'0}_{LT'}$ | ${}^{s}R^{x'0}_{LT}$ |
| | $\mathcal{O}^a_{1+}$ | $\mathcal{O}^a_{2+}$ | $\mathcal{O}^e_{1+}$ | $\mathcal{O}^e_{1-}$ | $\mathcal{O}^g_{1-}$ | $\mathcal{O}^g_{2-}$ |
| $(a,e,g):47$ | ${}^{s}R^{0z}_{TT}$ | $R^{0z}_{TT'}$ | ${}^{c}R^{00}_{LT}$ | ${}^{c}R^{0y}_{LT}$ | ${}^{s}R^{z'0}_{LT}$ | ${}^{c}R^{x'0}_{LT'}$ |
| | $\mathcal{O}^a_{1+}$ | $\mathcal{O}^a_{2+}$ | $\mathcal{O}^e_{2+}$ | $\mathcal{O}^e_{2-}$ | $\mathcal{O}^g_{1+}$ | $\mathcal{O}^g_{1-}$ |
| $(a,e,g):48$ | ${}^{s}R^{0z}_{TT}$ | $R^{0z}_{TT'}$ | ${}^{c}R^{00}_{LT}$ | ${}^{c}R^{0y}_{LT}$ | ${}^{c}R^{z'0}_{LT'}$ | ${}^{s}R^{x'0}_{LT}$ |
| | $\mathcal{O}^a_{1+}$ | $\mathcal{O}^a_{2+}$ | $\mathcal{O}^e_{2+}$ | $\mathcal{O}^e_{2-}$ | $\mathcal{O}^g_{2+}$ | $\mathcal{O}^g_{2-}$ |
| $(a,e,g):49$ | ${}^{s}R^{0z}_{TT}$ | $R^{0z}_{TT'}$ | ${}^{c}R^{00}_{LT}$ | ${}^{c}R^{0y}_{LT}$ | ${}^{s}R^{z'0}_{LT}$ | ${}^{c}R^{z'0}_{LT'}$ |
| | $\mathcal{O}^a_{1+}$ | $\mathcal{O}^a_{2+}$ | $\mathcal{O}^e_{2+}$ | $\mathcal{O}^e_{2-}$ | $\mathcal{O}^g_{1+}$ | $\mathcal{O}^g_{2+}$ |
| $(a,e,g):50$ | ${}^{s}R^{0z}_{TT}$ | $R^{0z}_{TT'}$ | ${}^{c}R^{00}_{LT}$ | ${}^{c}R^{0y}_{LT}$ | ${}^{s}R^{z'0}_{LT}$ | ${}^{s}R^{x'0}_{LT}$ |
| | $\mathcal{O}^a_{1+}$ | $\mathcal{O}^a_{2+}$ | $\mathcal{O}^e_{2+}$ | $\mathcal{O}^e_{2-}$ | $\mathcal{O}^g_{1+}$ | $\mathcal{O}^g_{2-}$ |
| $(a,e,g):51$ | ${}^{s}R^{0z}_{TT}$ | $R^{0z}_{TT'}$ | ${}^{c}R^{00}_{LT}$ | ${}^{c}R^{0y}_{LT}$ | ${}^{c}R^{x'0}_{LT'}$ | ${}^{c}R^{z'0}_{LT'}$ |
| | $\mathcal{O}^a_{1+}$ | $\mathcal{O}^a_{2+}$ | $\mathcal{O}^e_{2+}$ | $\mathcal{O}^e_{2-}$ | $\mathcal{O}^g_{1-}$ | $\mathcal{O}^g_{2+}$ |
| $(a,e,g):52$ | ${}^{s}R^{0z}_{TT}$ | $R^{0z}_{TT'}$ | ${}^{c}R^{00}_{LT}$ | ${}^{c}R^{0y}_{LT}$ | ${}^{c}R^{x'0}_{LT'}$ | ${}^{s}R^{x'0}_{LT}$ |

| | | | | | | |
|---|---|---|---|---|---|---|
| | $\mathcal{O}^{a}_{1+}$ | $\mathcal{O}^{a}_{2+}$ | $\mathcal{O}^{e}_{2+}$ | $\mathcal{O}^{e}_{2-}$ | $\mathcal{O}^{g}_{1-}$ | $\mathcal{O}^{g}_{2-}$ |
| $(a,e,g):53$ | ${}^{s}R^{0z}_{TT}$ | $R^{0z}_{TT'}$ | ${}^{s}R^{00}_{LT'}$ | ${}^{c}R^{00}_{LT}$ | ${}^{s}R^{z'0}_{LT}$ | ${}^{c}R^{x'0}_{LT'}$ |
| | $\mathcal{O}^{a}_{1+}$ | $\mathcal{O}^{a}_{2+}$ | $\mathcal{O}^{e}_{1+}$ | $\mathcal{O}^{e}_{2+}$ | $\mathcal{O}^{g}_{1+}$ | $\mathcal{O}^{g}_{1-}$ |
| $(a,e,g):54$ | ${}^{s}R^{0z}_{TT}$ | $R^{0z}_{TT'}$ | ${}^{s}R^{00}_{LT'}$ | ${}^{c}R^{00}_{LT}$ | ${}^{c}R^{z'0}_{LT'}$ | ${}^{s}R^{x'0}_{LT}$ |
| | $\mathcal{O}^{a}_{1+}$ | $\mathcal{O}^{a}_{2+}$ | $\mathcal{O}^{e}_{1+}$ | $\mathcal{O}^{e}_{2+}$ | $\mathcal{O}^{g}_{2+}$ | $\mathcal{O}^{g}_{2-}$ |
| $(a,e,g):55$ | ${}^{s}R^{0z}_{TT}$ | $R^{0z}_{TT'}$ | ${}^{s}R^{00}_{LT'}$ | ${}^{c}R^{00}_{LT}$ | ${}^{s}R^{z'0}_{LT}$ | ${}^{c}R^{z'0}_{LT'}$ |
| | $\mathcal{O}^{a}_{1+}$ | $\mathcal{O}^{a}_{2+}$ | $\mathcal{O}^{e}_{1+}$ | $\mathcal{O}^{e}_{2+}$ | $\mathcal{O}^{g}_{1+}$ | $\mathcal{O}^{g}_{2+}$ |
| $(a,e,g):56$ | ${}^{s}R^{0z}_{TT}$ | $R^{0z}_{TT'}$ | ${}^{s}R^{00}_{LT'}$ | ${}^{c}R^{00}_{LT}$ | ${}^{s}R^{z'0}_{LT}$ | ${}^{s}R^{x'0}_{LT}$ |
| | $\mathcal{O}^{a}_{1+}$ | $\mathcal{O}^{a}_{2+}$ | $\mathcal{O}^{e}_{1+}$ | $\mathcal{O}^{e}_{2+}$ | $\mathcal{O}^{g}_{1+}$ | $\mathcal{O}^{g}_{2-}$ |
| $(a,e,g):57$ | ${}^{s}R^{0z}_{TT}$ | $R^{0z}_{TT'}$ | ${}^{s}R^{00}_{LT'}$ | ${}^{c}R^{00}_{LT}$ | ${}^{c}R^{x'0}_{LT'}$ | ${}^{c}R^{z'0}_{LT'}$ |
| | $\mathcal{O}^{a}_{1+}$ | $\mathcal{O}^{a}_{2+}$ | $\mathcal{O}^{e}_{1+}$ | $\mathcal{O}^{e}_{2+}$ | $\mathcal{O}^{g}_{1-}$ | $\mathcal{O}^{g}_{2+}$ |
| $(a,e,g):58$ | ${}^{s}R^{0z}_{TT}$ | $R^{0z}_{TT'}$ | ${}^{s}R^{00}_{LT'}$ | ${}^{c}R^{00}_{LT}$ | ${}^{c}R^{x'0}_{LT'}$ | ${}^{s}R^{x'0}_{LT}$ |
| | $\mathcal{O}^{a}_{1+}$ | $\mathcal{O}^{a}_{2+}$ | $\mathcal{O}^{e}_{1+}$ | $\mathcal{O}^{e}_{2+}$ | $\mathcal{O}^{g}_{1-}$ | $\mathcal{O}^{g}_{2-}$ |
| $(a,e,g):59$ | ${}^{s}R^{0z}_{TT}$ | $R^{0z}_{TT'}$ | ${}^{s}R^{00}_{LT'}$ | ${}^{c}R^{0y}_{LT}$ | ${}^{s}R^{z'0}_{LT}$ | ${}^{c}R^{x'0}_{LT'}$ |
| | $\mathcal{O}^{a}_{1+}$ | $\mathcal{O}^{a}_{2+}$ | $\mathcal{O}^{e}_{1+}$ | $\mathcal{O}^{e}_{2-}$ | $\mathcal{O}^{g}_{1+}$ | $\mathcal{O}^{g}_{1-}$ |
| $(a,e,g):60$ | ${}^{s}R^{0z}_{TT}$ | $R^{0z}_{TT'}$ | ${}^{s}R^{00}_{LT'}$ | ${}^{c}R^{0y}_{LT}$ | ${}^{c}R^{z'0}_{LT'}$ | ${}^{s}R^{x'0}_{LT}$ |
| | $\mathcal{O}^{a}_{1+}$ | $\mathcal{O}^{a}_{2+}$ | $\mathcal{O}^{e}_{1+}$ | $\mathcal{O}^{e}_{2-}$ | $\mathcal{O}^{g}_{2+}$ | $\mathcal{O}^{g}_{2-}$ |
| $(a,e,g):61$ | ${}^{s}R^{0z}_{TT}$ | $R^{0z}_{TT'}$ | ${}^{s}R^{00}_{LT'}$ | ${}^{c}R^{0y}_{LT}$ | ${}^{s}R^{z'0}_{LT}$ | ${}^{c}R^{z'0}_{LT'}$ |
| | $\mathcal{O}^{a}_{1+}$ | $\mathcal{O}^{a}_{2+}$ | $\mathcal{O}^{e}_{1+}$ | $\mathcal{O}^{e}_{2-}$ | $\mathcal{O}^{g}_{1+}$ | $\mathcal{O}^{g}_{2+}$ |
| $(a,e,g):62$ | ${}^{s}R^{0z}_{TT}$ | $R^{0z}_{TT'}$ | ${}^{s}R^{00}_{LT'}$ | ${}^{c}R^{0y}_{LT}$ | ${}^{s}R^{z'0}_{LT}$ | ${}^{s}R^{x'0}_{LT}$ |
| | $\mathcal{O}^{a}_{1+}$ | $\mathcal{O}^{a}_{2+}$ | $\mathcal{O}^{e}_{1+}$ | $\mathcal{O}^{e}_{2-}$ | $\mathcal{O}^{g}_{1+}$ | $\mathcal{O}^{g}_{2-}$ |
| $(a,e,g):63$ | ${}^{s}R^{0z}_{TT}$ | $R^{0z}_{TT'}$ | ${}^{s}R^{00}_{LT'}$ | ${}^{c}R^{0y}_{LT}$ | ${}^{c}R^{x'0}_{LT'}$ | ${}^{c}R^{z'0}_{LT'}$ |
| | $\mathcal{O}^{a}_{1+}$ | $\mathcal{O}^{a}_{2+}$ | $\mathcal{O}^{e}_{1+}$ | $\mathcal{O}^{e}_{2-}$ | $\mathcal{O}^{g}_{1-}$ | $\mathcal{O}^{g}_{2+}$ |
| $(a,e,g):64$ | ${}^{s}R^{0z}_{TT}$ | $R^{0z}_{TT'}$ | ${}^{s}R^{00}_{LT'}$ | ${}^{c}R^{0y}_{LT}$ | ${}^{c}R^{x'0}_{LT'}$ | ${}^{s}R^{x'0}_{LT}$ |
| | $\mathcal{O}^{a}_{1+}$ | $\mathcal{O}^{a}_{2+}$ | $\mathcal{O}^{e}_{1+}$ | $\mathcal{O}^{e}_{2-}$ | $\mathcal{O}^{g}_{1-}$ | $\mathcal{O}^{g}_{2-}$ |
| $(a,e,g):65$ | ${}^{s}R^{0z}_{TT}$ | $R^{0z}_{TT'}$ | ${}^{s}R^{0y}_{LT'}$ | ${}^{c}R^{00}_{LT}$ | ${}^{s}R^{z'0}_{LT}$ | ${}^{c}R^{x'0}_{LT'}$ |
| | $\mathcal{O}^{a}_{1+}$ | $\mathcal{O}^{a}_{2+}$ | $\mathcal{O}^{e}_{1-}$ | $\mathcal{O}^{e}_{2+}$ | $\mathcal{O}^{g}_{1+}$ | $\mathcal{O}^{g}_{1-}$ |
| $(a,e,g):66$ | ${}^{s}R^{0z}_{TT}$ | $R^{0z}_{TT'}$ | ${}^{s}R^{0y}_{LT'}$ | ${}^{c}R^{00}_{LT}$ | ${}^{c}R^{z'0}_{LT'}$ | ${}^{s}R^{x'0}_{LT}$ |
| | $\mathcal{O}^{a}_{1+}$ | $\mathcal{O}^{a}_{2+}$ | $\mathcal{O}^{e}_{1-}$ | $\mathcal{O}^{e}_{2+}$ | $\mathcal{O}^{g}_{2+}$ | $\mathcal{O}^{g}_{2-}$ |
| $(a,e,g):67$ | ${}^{s}R^{0z}_{TT}$ | $R^{0z}_{TT'}$ | ${}^{s}R^{0y}_{LT'}$ | ${}^{c}R^{00}_{LT}$ | ${}^{s}R^{z'0}_{LT}$ | ${}^{c}R^{z'0}_{LT'}$ |
| | $\mathcal{O}^{a}_{1+}$ | $\mathcal{O}^{a}_{2+}$ | $\mathcal{O}^{e}_{1-}$ | $\mathcal{O}^{e}_{2+}$ | $\mathcal{O}^{g}_{1+}$ | $\mathcal{O}^{g}_{2+}$ |
| $(a,e,g):68$ | ${}^{s}R^{0z}_{TT}$ | $R^{0z}_{TT'}$ | ${}^{s}R^{0y}_{LT'}$ | ${}^{c}R^{00}_{LT}$ | ${}^{s}R^{z'0}_{LT}$ | ${}^{s}R^{x'0}_{LT}$ |
| | $\mathcal{O}^{a}_{1+}$ | $\mathcal{O}^{a}_{2+}$ | $\mathcal{O}^{e}_{1-}$ | $\mathcal{O}^{e}_{2+}$ | $\mathcal{O}^{g}_{1+}$ | $\mathcal{O}^{g}_{2-}$ |
| $(a,e,g):69$ | ${}^{s}R^{0z}_{TT}$ | $R^{0z}_{TT'}$ | ${}^{s}R^{0y}_{LT'}$ | ${}^{c}R^{00}_{LT}$ | ${}^{c}R^{x'0}_{LT'}$ | ${}^{c}R^{z'0}_{LT'}$ |
| | $\mathcal{O}^{a}_{1+}$ | $\mathcal{O}^{a}_{2+}$ | $\mathcal{O}^{e}_{1-}$ | $\mathcal{O}^{e}_{2+}$ | $\mathcal{O}^{g}_{1-}$ | $\mathcal{O}^{g}_{2+}$ |
| $(a,e,g):70$ | ${}^{s}R^{0z}_{TT}$ | $R^{0z}_{TT'}$ | ${}^{s}R^{0y}_{LT'}$ | ${}^{c}R^{00}_{LT}$ | ${}^{c}R^{x'0}_{LT'}$ | ${}^{s}R^{x'0}_{LT}$ |
| | $\mathcal{O}^{a}_{1+}$ | $\mathcal{O}^{a}_{2+}$ | $\mathcal{O}^{e}_{1-}$ | $\mathcal{O}^{e}_{2+}$ | $\mathcal{O}^{g}_{1-}$ | $\mathcal{O}^{g}_{2-}$ |
| $(a,e,g):71$ | ${}^{s}R^{0z}_{TT}$ | $R^{0z}_{TT'}$ | ${}^{s}R^{0y}_{LT'}$ | ${}^{c}R^{0y}_{LT}$ | ${}^{s}R^{z'0}_{LT}$ | ${}^{c}R^{x'0}_{LT'}$ |
| | $\mathcal{O}^{a}_{1+}$ | $\mathcal{O}^{a}_{2+}$ | $\mathcal{O}^{e}_{1-}$ | $\mathcal{O}^{e}_{2-}$ | $\mathcal{O}^{g}_{1+}$ | $\mathcal{O}^{g}_{1-}$ |
| $(a,e,g):72$ | ${}^{s}R^{0z}_{TT}$ | $R^{0z}_{TT'}$ | ${}^{s}R^{0y}_{LT'}$ | ${}^{c}R^{0y}_{LT}$ | ${}^{c}R^{z'0}_{LT'}$ | ${}^{s}R^{x'0}_{LT}$ |
| | $\mathcal{O}^{a}_{1+}$ | $\mathcal{O}^{a}_{2+}$ | $\mathcal{O}^{e}_{1-}$ | $\mathcal{O}^{e}_{2-}$ | $\mathcal{O}^{g}_{2+}$ | $\mathcal{O}^{g}_{2-}$ |
| $(a,e,g):73$ | ${}^{s}R^{0z}_{TT}$ | $R^{0z}_{TT'}$ | ${}^{s}R^{0y}_{LT'}$ | ${}^{c}R^{0y}_{LT}$ | ${}^{s}R^{z'0}_{LT}$ | ${}^{c}R^{z'0}_{LT'}$ |
| | $\mathcal{O}^{a}_{1+}$ | $\mathcal{O}^{a}_{2+}$ | $\mathcal{O}^{e}_{1-}$ | $\mathcal{O}^{e}_{2-}$ | $\mathcal{O}^{g}_{1+}$ | $\mathcal{O}^{g}_{2+}$ |
| $(a,e,g):74$ | ${}^{s}R^{0z}_{TT}$ | $R^{0z}_{TT'}$ | ${}^{s}R^{0y}_{LT'}$ | ${}^{c}R^{0y}_{LT}$ | ${}^{s}R^{z'0}_{LT}$ | ${}^{s}R^{x'0}_{LT}$ |
| | $\mathcal{O}^{a}_{1+}$ | $\mathcal{O}^{a}_{2+}$ | $\mathcal{O}^{e}_{1-}$ | $\mathcal{O}^{e}_{2-}$ | $\mathcal{O}^{g}_{1+}$ | $\mathcal{O}^{g}_{2-}$ |
| $(a,e,g):75$ | ${}^{s}R^{0z}_{TT}$ | $R^{0z}_{TT'}$ | ${}^{s}R^{0y}_{LT'}$ | ${}^{c}R^{0y}_{LT}$ | ${}^{c}R^{x'0}_{LT'}$ | ${}^{c}R^{z'0}_{LT'}$ |
| | $\mathcal{O}^{a}_{1+}$ | $\mathcal{O}^{a}_{2+}$ | $\mathcal{O}^{e}_{1-}$ | $\mathcal{O}^{e}_{2-}$ | $\mathcal{O}^{g}_{1-}$ | $\mathcal{O}^{g}_{2+}$ |
| $(a,e,g):76$ | ${}^{s}R^{0z}_{TT}$ | $R^{0z}_{TT'}$ | ${}^{s}R^{0y}_{LT'}$ | ${}^{c}R^{0y}_{LT}$ | ${}^{c}R^{x'0}_{LT'}$ | ${}^{s}R^{x'0}_{LT}$ |
| | $\mathcal{O}^{a}_{1+}$ | $\mathcal{O}^{a}_{2+}$ | $\mathcal{O}^{e}_{1-}$ | $\mathcal{O}^{e}_{2-}$ | $\mathcal{O}^{g}_{1-}$ | $\mathcal{O}^{g}_{2-}$ |
| $(a,e,g):77$ | ${}^{s}R^{0z}_{TT}$ | ${}^{s}R^{0x}_{TT}$ | ${}^{s}R^{00}_{LT'}$ | ${}^{s}R^{0y}_{LT'}$ | ${}^{s}R^{z'0}_{LT}$ | ${}^{c}R^{z'0}_{LT'}$ |
| | $\mathcal{O}^{a}_{1+}$ | $\mathcal{O}^{a}_{2-}$ | $\mathcal{O}^{e}_{1+}$ | $\mathcal{O}^{e}_{1-}$ | $\mathcal{O}^{g}_{1+}$ | $\mathcal{O}^{g}_{2+}$ |
| $(a,e,g):78$ | ${}^{s}R^{0z}_{TT}$ | ${}^{s}R^{0x}_{TT}$ | ${}^{s}R^{00}_{LT'}$ | ${}^{s}R^{0y}_{LT'}$ | ${}^{c}R^{x'0}_{LT'}$ | ${}^{s}R^{x'0}_{LT}$ |
| | $\mathcal{O}^{a}_{1+}$ | $\mathcal{O}^{a}_{2-}$ | $\mathcal{O}^{e}_{1+}$ | $\mathcal{O}^{e}_{1-}$ | $\mathcal{O}^{g}_{1-}$ | $\mathcal{O}^{g}_{2-}$ |
| $(a,e,g):79$ | ${}^{s}R^{0z}_{TT}$ | ${}^{s}R^{0x}_{TT}$ | ${}^{c}R^{00}_{LT}$ | ${}^{c}R^{0y}_{LT}$ | ${}^{s}R^{z'0}_{LT}$ | ${}^{c}R^{z'0}_{LT'}$ |
| | $\mathcal{O}^{a}_{1+}$ | $\mathcal{O}^{a}_{2-}$ | $\mathcal{O}^{e}_{2+}$ | $\mathcal{O}^{e}_{2-}$ | $\mathcal{O}^{g}_{1+}$ | $\mathcal{O}^{g}_{2+}$ |
| $(a,e,g):80$ | ${}^{s}R^{0z}_{TT}$ | ${}^{s}R^{0x}_{TT}$ | ${}^{c}R^{00}_{LT}$ | ${}^{c}R^{0y}_{LT}$ | ${}^{c}R^{x'0}_{LT'}$ | ${}^{s}R^{x'0}_{LT}$ |
| | $\mathcal{O}^{a}_{1+}$ | $\mathcal{O}^{a}_{2-}$ | $\mathcal{O}^{e}_{2+}$ | $\mathcal{O}^{e}_{2-}$ | $\mathcal{O}^{g}_{1-}$ | $\mathcal{O}^{g}_{2-}$ |
| $(a,e,g):81$ | ${}^{s}R^{0z}_{TT}$ | ${}^{s}R^{0x}_{TT}$ | ${}^{s}R^{00}_{LT'}$ | ${}^{c}R^{00}_{LT}$ | ${}^{s}R^{z'0}_{LT}$ | ${}^{c}R^{x'0}_{LT'}$ |

| | | | | | | |
|---|---|---|---|---|---|---|
| | $\mathcal{O}^{a}_{1+}$ | $\mathcal{O}^{a}_{2-}$ | $\mathcal{O}^{e}_{1+}$ | $\mathcal{O}^{e}_{2+}$ | $\mathcal{O}^{g}_{1+}$ | $\mathcal{O}^{g}_{1-}$ |
| $(a,e,g):82$ | ${}^{s}R^{0z}_{TT}$ | ${}^{s}R^{0x}_{TT}$ | ${}^{s}R^{00}_{LT'}$ | ${}^{c}R^{00}_{LT}$ | ${}^{c}R^{z'0}_{LT'}$ | ${}^{s}R^{x'0}_{LT}$ |
| | $\mathcal{O}^{a}_{1+}$ | $\mathcal{O}^{a}_{2-}$ | $\mathcal{O}^{e}_{1+}$ | $\mathcal{O}^{e}_{2+}$ | $\mathcal{O}^{g}_{2+}$ | $\mathcal{O}^{g}_{2-}$ |
| $(a,e,g):83$ | ${}^{s}R^{0z}_{TT}$ | ${}^{s}R^{0x}_{TT}$ | ${}^{s}R^{00}_{LT'}$ | ${}^{c}R^{00}_{LT}$ | ${}^{s}R^{z'0}_{LT}$ | ${}^{c}R^{z'0}_{LT'}$ |
| | $\mathcal{O}^{a}_{1+}$ | $\mathcal{O}^{a}_{2-}$ | $\mathcal{O}^{e}_{1+}$ | $\mathcal{O}^{e}_{2+}$ | $\mathcal{O}^{g}_{1+}$ | $\mathcal{O}^{g}_{2+}$ |
| $(a,e,g):84$ | ${}^{s}R^{0z}_{TT}$ | ${}^{s}R^{0x}_{TT}$ | ${}^{s}R^{00}_{LT'}$ | ${}^{c}R^{00}_{LT}$ | ${}^{s}R^{z'0}_{LT}$ | ${}^{s}R^{x'0}_{LT}$ |
| | $\mathcal{O}^{a}_{1+}$ | $\mathcal{O}^{a}_{2-}$ | $\mathcal{O}^{e}_{1+}$ | $\mathcal{O}^{e}_{2+}$ | $\mathcal{O}^{g}_{1+}$ | $\mathcal{O}^{g}_{2-}$ |
| $(a,e,g):85$ | ${}^{s}R^{0z}_{TT}$ | ${}^{s}R^{0x}_{TT}$ | ${}^{s}R^{00}_{LT'}$ | ${}^{c}R^{00}_{LT}$ | ${}^{c}R^{x'0}_{LT'}$ | ${}^{c}R^{z'0}_{LT'}$ |
| | $\mathcal{O}^{a}_{1+}$ | $\mathcal{O}^{a}_{2-}$ | $\mathcal{O}^{e}_{1+}$ | $\mathcal{O}^{e}_{2+}$ | $\mathcal{O}^{g}_{1-}$ | $\mathcal{O}^{g}_{2+}$ |
| $(a,e,g):86$ | ${}^{s}R^{0z}_{TT}$ | ${}^{s}R^{0x}_{TT}$ | ${}^{s}R^{00}_{LT'}$ | ${}^{c}R^{00}_{LT}$ | ${}^{c}R^{x'0}_{LT'}$ | ${}^{s}R^{x'0}_{LT}$ |
| | $\mathcal{O}^{a}_{1+}$ | $\mathcal{O}^{a}_{2-}$ | $\mathcal{O}^{e}_{1+}$ | $\mathcal{O}^{e}_{2+}$ | $\mathcal{O}^{g}_{1-}$ | $\mathcal{O}^{g}_{2-}$ |
| $(a,e,g):87$ | ${}^{s}R^{0z}_{TT}$ | ${}^{s}R^{0x}_{TT}$ | ${}^{s}R^{00}_{LT'}$ | ${}^{c}R^{0y}_{LT}$ | ${}^{s}R^{z'0}_{LT}$ | ${}^{c}R^{z'0}_{LT'}$ |
| | $\mathcal{O}^{a}_{1+}$ | $\mathcal{O}^{a}_{2-}$ | $\mathcal{O}^{e}_{1+}$ | $\mathcal{O}^{e}_{2-}$ | $\mathcal{O}^{g}_{1+}$ | $\mathcal{O}^{g}_{2+}$ |
| $(a,e,g):88$ | ${}^{s}R^{0z}_{TT}$ | ${}^{s}R^{0x}_{TT}$ | ${}^{s}R^{00}_{LT'}$ | ${}^{c}R^{0y}_{LT}$ | ${}^{c}R^{x'0}_{LT'}$ | ${}^{s}R^{x'0}_{LT}$ |
| | $\mathcal{O}^{a}_{1+}$ | $\mathcal{O}^{a}_{2-}$ | $\mathcal{O}^{e}_{1+}$ | $\mathcal{O}^{e}_{2-}$ | $\mathcal{O}^{g}_{1-}$ | $\mathcal{O}^{g}_{2-}$ |
| $(a,e,g):89$ | ${}^{s}R^{0z}_{TT}$ | ${}^{s}R^{0x}_{TT}$ | ${}^{s}R^{0y}_{LT'}$ | ${}^{c}R^{00}_{LT}$ | ${}^{s}R^{z'0}_{LT}$ | ${}^{c}R^{z'0}_{LT'}$ |
| | $\mathcal{O}^{a}_{1+}$ | $\mathcal{O}^{a}_{2-}$ | $\mathcal{O}^{e}_{1-}$ | $\mathcal{O}^{e}_{2+}$ | $\mathcal{O}^{g}_{1+}$ | $\mathcal{O}^{g}_{2+}$ |
| $(a,e,g):90$ | ${}^{s}R^{0z}_{TT}$ | ${}^{s}R^{0x}_{TT}$ | ${}^{s}R^{0y}_{LT'}$ | ${}^{c}R^{00}_{LT}$ | ${}^{c}R^{x'0}_{LT'}$ | ${}^{s}R^{x'0}_{LT}$ |
| | $\mathcal{O}^{a}_{1+}$ | $\mathcal{O}^{a}_{2-}$ | $\mathcal{O}^{e}_{1-}$ | $\mathcal{O}^{e}_{2+}$ | $\mathcal{O}^{g}_{1-}$ | $\mathcal{O}^{g}_{2-}$ |
| $(a,e,g):91$ | ${}^{s}R^{0z}_{TT}$ | ${}^{s}R^{0x}_{TT}$ | ${}^{s}R^{0y}_{LT'}$ | ${}^{c}R^{0y}_{LT}$ | ${}^{s}R^{z'0}_{LT}$ | ${}^{c}R^{x'0}_{LT'}$ |
| | $\mathcal{O}^{a}_{1+}$ | $\mathcal{O}^{a}_{2-}$ | $\mathcal{O}^{e}_{1-}$ | $\mathcal{O}^{e}_{2-}$ | $\mathcal{O}^{g}_{1+}$ | $\mathcal{O}^{g}_{1-}$ |
| $(a,e,g):92$ | ${}^{s}R^{0z}_{TT}$ | ${}^{s}R^{0x}_{TT}$ | ${}^{s}R^{0y}_{LT'}$ | ${}^{c}R^{0y}_{LT}$ | ${}^{c}R^{z'0}_{LT'}$ | ${}^{s}R^{x'0}_{LT}$ |
| | $\mathcal{O}^{a}_{1+}$ | $\mathcal{O}^{a}_{2-}$ | $\mathcal{O}^{e}_{1-}$ | $\mathcal{O}^{e}_{2-}$ | $\mathcal{O}^{g}_{2+}$ | $\mathcal{O}^{g}_{2-}$ |
| $(a,e,g):93$ | ${}^{s}R^{0z}_{TT}$ | ${}^{s}R^{0x}_{TT}$ | ${}^{s}R^{0y}_{LT'}$ | ${}^{c}R^{0y}_{LT}$ | ${}^{s}R^{z'0}_{LT}$ | ${}^{c}R^{z'0}_{LT'}$ |
| | $\mathcal{O}^{a}_{1+}$ | $\mathcal{O}^{a}_{2-}$ | $\mathcal{O}^{e}_{1-}$ | $\mathcal{O}^{e}_{2-}$ | $\mathcal{O}^{g}_{1+}$ | $\mathcal{O}^{g}_{2+}$ |
| $(a,e,g):94$ | ${}^{s}R^{0z}_{TT}$ | ${}^{s}R^{0x}_{TT}$ | ${}^{s}R^{0y}_{LT'}$ | ${}^{c}R^{0y}_{LT}$ | ${}^{s}R^{z'0}_{LT}$ | ${}^{s}R^{x'0}_{LT}$ |
| | $\mathcal{O}^{a}_{1+}$ | $\mathcal{O}^{a}_{2-}$ | $\mathcal{O}^{e}_{1-}$ | $\mathcal{O}^{e}_{2-}$ | $\mathcal{O}^{g}_{1+}$ | $\mathcal{O}^{g}_{2-}$ |
| $(a,e,g):95$ | ${}^{s}R^{0z}_{TT}$ | ${}^{s}R^{0x}_{TT}$ | ${}^{s}R^{0y}_{LT'}$ | ${}^{c}R^{0y}_{LT}$ | ${}^{c}R^{x'0}_{LT'}$ | ${}^{c}R^{z'0}_{LT'}$ |
| | $\mathcal{O}^{a}_{1+}$ | $\mathcal{O}^{a}_{2-}$ | $\mathcal{O}^{e}_{1-}$ | $\mathcal{O}^{e}_{2-}$ | $\mathcal{O}^{g}_{1-}$ | $\mathcal{O}^{g}_{2+}$ |
| $(a,e,g):96$ | ${}^{s}R^{0z}_{TT}$ | ${}^{s}R^{0x}_{TT}$ | ${}^{s}R^{0y}_{LT'}$ | ${}^{c}R^{0y}_{LT}$ | ${}^{c}R^{x'0}_{LT'}$ | ${}^{s}R^{x'0}_{LT}$ |
| | $\mathcal{O}^{a}_{1+}$ | $\mathcal{O}^{a}_{2-}$ | $\mathcal{O}^{e}_{1-}$ | $\mathcal{O}^{e}_{2-}$ | $\mathcal{O}^{g}_{1-}$ | $\mathcal{O}^{g}_{2-}$ |
| $(a,e,g):97$ | $R^{0x}_{TT'}$ | $R^{0z}_{TT'}$ | ${}^{s}R^{00}_{LT'}$ | ${}^{s}R^{0y}_{LT'}$ | ${}^{s}R^{z'0}_{LT}$ | ${}^{c}R^{z'0}_{LT'}$ |
| | $\mathcal{O}^{a}_{1-}$ | $\mathcal{O}^{a}_{2+}$ | $\mathcal{O}^{e}_{1+}$ | $\mathcal{O}^{e}_{1-}$ | $\mathcal{O}^{g}_{1+}$ | $\mathcal{O}^{g}_{2+}$ |
| $(a,e,g):98$ | $R^{0x}_{TT'}$ | $R^{0z}_{TT'}$ | ${}^{s}R^{00}_{LT'}$ | ${}^{s}R^{0y}_{LT'}$ | ${}^{c}R^{x'0}_{LT'}$ | ${}^{s}R^{x'0}_{LT}$ |
| | $\mathcal{O}^{a}_{1-}$ | $\mathcal{O}^{a}_{2+}$ | $\mathcal{O}^{e}_{1+}$ | $\mathcal{O}^{e}_{1-}$ | $\mathcal{O}^{g}_{1-}$ | $\mathcal{O}^{g}_{2-}$ |
| $(a,e,g):99$ | $R^{0x}_{TT'}$ | $R^{0z}_{TT'}$ | ${}^{c}R^{00}_{LT}$ | ${}^{c}R^{0y}_{LT}$ | ${}^{s}R^{z'0}_{LT}$ | ${}^{c}R^{z'0}_{LT'}$ |
| | $\mathcal{O}^{a}_{1-}$ | $\mathcal{O}^{a}_{2+}$ | $\mathcal{O}^{e}_{2+}$ | $\mathcal{O}^{e}_{2-}$ | $\mathcal{O}^{g}_{1+}$ | $\mathcal{O}^{g}_{2+}$ |
| $(a,e,g):100$ | $R^{0x}_{TT'}$ | $R^{0z}_{TT'}$ | ${}^{c}R^{00}_{LT}$ | ${}^{c}R^{0y}_{LT}$ | ${}^{c}R^{x'0}_{LT'}$ | ${}^{s}R^{x'0}_{LT}$ |
| | $\mathcal{O}^{a}_{1-}$ | $\mathcal{O}^{a}_{2+}$ | $\mathcal{O}^{e}_{2+}$ | $\mathcal{O}^{e}_{2-}$ | $\mathcal{O}^{g}_{1-}$ | $\mathcal{O}^{g}_{2-}$ |
| $(a,e,g):101$ | $R^{0x}_{TT'}$ | $R^{0z}_{TT'}$ | ${}^{s}R^{00}_{LT'}$ | ${}^{c}R^{00}_{LT}$ | ${}^{s}R^{z'0}_{LT}$ | ${}^{c}R^{x'0}_{LT'}$ |
| | $\mathcal{O}^{a}_{1-}$ | $\mathcal{O}^{a}_{2+}$ | $\mathcal{O}^{e}_{1+}$ | $\mathcal{O}^{e}_{2+}$ | $\mathcal{O}^{g}_{1+}$ | $\mathcal{O}^{g}_{1-}$ |
| $(a,e,g):102$ | $R^{0x}_{TT'}$ | $R^{0z}_{TT'}$ | ${}^{s}R^{00}_{LT'}$ | ${}^{c}R^{00}_{LT}$ | ${}^{c}R^{z'0}_{LT'}$ | ${}^{s}R^{x'0}_{LT}$ |
| | $\mathcal{O}^{a}_{1-}$ | $\mathcal{O}^{a}_{2+}$ | $\mathcal{O}^{e}_{1+}$ | $\mathcal{O}^{e}_{2+}$ | $\mathcal{O}^{g}_{2+}$ | $\mathcal{O}^{g}_{2-}$ |
| $(a,e,g):103$ | $R^{0x}_{TT'}$ | $R^{0z}_{TT'}$ | ${}^{s}R^{00}_{LT'}$ | ${}^{c}R^{00}_{LT}$ | ${}^{s}R^{z'0}_{LT}$ | ${}^{c}R^{z'0}_{LT'}$ |
| | $\mathcal{O}^{a}_{1-}$ | $\mathcal{O}^{a}_{2+}$ | $\mathcal{O}^{e}_{1+}$ | $\mathcal{O}^{e}_{2+}$ | $\mathcal{O}^{g}_{1+}$ | $\mathcal{O}^{g}_{2+}$ |
| $(a,e,g):104$ | $R^{0x}_{TT'}$ | $R^{0z}_{TT'}$ | ${}^{s}R^{00}_{LT'}$ | ${}^{c}R^{00}_{LT}$ | ${}^{s}R^{z'0}_{LT}$ | ${}^{s}R^{x'0}_{LT}$ |
| | $\mathcal{O}^{a}_{1-}$ | $\mathcal{O}^{a}_{2+}$ | $\mathcal{O}^{e}_{1+}$ | $\mathcal{O}^{e}_{2+}$ | $\mathcal{O}^{g}_{1+}$ | $\mathcal{O}^{g}_{2-}$ |
| $(a,e,g):105$ | $R^{0x}_{TT'}$ | $R^{0z}_{TT'}$ | ${}^{s}R^{00}_{LT'}$ | ${}^{c}R^{00}_{LT}$ | ${}^{c}R^{x'0}_{LT'}$ | ${}^{c}R^{z'0}_{LT'}$ |
| | $\mathcal{O}^{a}_{1-}$ | $\mathcal{O}^{a}_{2+}$ | $\mathcal{O}^{e}_{1+}$ | $\mathcal{O}^{e}_{2+}$ | $\mathcal{O}^{g}_{1-}$ | $\mathcal{O}^{g}_{2+}$ |
| $(a,e,g):106$ | $R^{0x}_{TT'}$ | $R^{0z}_{TT'}$ | ${}^{s}R^{00}_{LT'}$ | ${}^{c}R^{00}_{LT}$ | ${}^{c}R^{x'0}_{LT'}$ | ${}^{s}R^{x'0}_{LT}$ |
| | $\mathcal{O}^{a}_{1-}$ | $\mathcal{O}^{a}_{2+}$ | $\mathcal{O}^{e}_{1+}$ | $\mathcal{O}^{e}_{2+}$ | $\mathcal{O}^{g}_{1-}$ | $\mathcal{O}^{g}_{2-}$ |
| $(a,e,g):107$ | $R^{0x}_{TT'}$ | $R^{0z}_{TT'}$ | ${}^{s}R^{00}_{LT'}$ | ${}^{c}R^{0y}_{LT}$ | ${}^{s}R^{z'0}_{LT}$ | ${}^{c}R^{z'0}_{LT'}$ |
| | $\mathcal{O}^{a}_{1-}$ | $\mathcal{O}^{a}_{2+}$ | $\mathcal{O}^{e}_{1+}$ | $\mathcal{O}^{e}_{2-}$ | $\mathcal{O}^{g}_{1+}$ | $\mathcal{O}^{g}_{2+}$ |
| $(a,e,g):108$ | $R^{0x}_{TT'}$ | $R^{0z}_{TT'}$ | ${}^{s}R^{00}_{LT'}$ | ${}^{c}R^{0y}_{LT}$ | ${}^{c}R^{x'0}_{LT'}$ | ${}^{s}R^{x'0}_{LT}$ |
| | $\mathcal{O}^{a}_{1-}$ | $\mathcal{O}^{a}_{2+}$ | $\mathcal{O}^{e}_{1+}$ | $\mathcal{O}^{e}_{2-}$ | $\mathcal{O}^{g}_{1-}$ | $\mathcal{O}^{g}_{2-}$ |
| $(a,e,g):109$ | $R^{0x}_{TT'}$ | $R^{0z}_{TT'}$ | ${}^{s}R^{0y}_{LT'}$ | ${}^{c}R^{00}_{LT}$ | ${}^{s}R^{z'0}_{LT}$ | ${}^{c}R^{z'0}_{LT'}$ |
| | $\mathcal{O}^{a}_{1-}$ | $\mathcal{O}^{a}_{2+}$ | $\mathcal{O}^{e}_{1-}$ | $\mathcal{O}^{e}_{2+}$ | $\mathcal{O}^{g}_{1+}$ | $\mathcal{O}^{g}_{2+}$ |
| $(a,e,g):110$ | $R^{0x}_{TT'}$ | $R^{0z}_{TT'}$ | ${}^{s}R^{0y}_{LT'}$ | ${}^{c}R^{00}_{LT}$ | ${}^{c}R^{x'0}_{LT'}$ | ${}^{s}R^{x'0}_{LT}$ |

| | | | | | | |
|---|---|---|---|---|---|---|
| | $\mathcal{O}^a_{1-}$ | $\mathcal{O}^a_{2+}$ | $\mathcal{O}^e_{1-}$ | $\mathcal{O}^e_{2+}$ | $\mathcal{O}^g_{1-}$ | $\mathcal{O}^g_{2-}$ |
| $(a,e,g):111$ | $R^{0x}_{TT'}$ | $R^{0z}_{TT'}$ | ${}^sR^{0y}_{LT'}$ | ${}^cR^{0y}_{LT}$ | ${}^sR^{z'0}_{LT}$ | ${}^cR^{x'0}_{LT'}$ |
| | $\mathcal{O}^a_{1-}$ | $\mathcal{O}^a_{2+}$ | $\mathcal{O}^e_{1-}$ | $\mathcal{O}^e_{2-}$ | $\mathcal{O}^g_{1+}$ | $\mathcal{O}^g_{1-}$ |
| $(a,e,g):112$ | $R^{0x}_{TT'}$ | $R^{0z}_{TT'}$ | ${}^sR^{0y}_{LT'}$ | ${}^cR^{0y}_{LT}$ | ${}^cR^{z'0}_{LT'}$ | ${}^sR^{x'0}_{LT}$ |
| | $\mathcal{O}^a_{1-}$ | $\mathcal{O}^a_{2+}$ | $\mathcal{O}^e_{1-}$ | $\mathcal{O}^e_{2-}$ | $\mathcal{O}^g_{2+}$ | $\mathcal{O}^g_{2-}$ |
| $(a,e,g):113$ | $R^{0x}_{TT'}$ | $R^{0z}_{TT'}$ | ${}^sR^{0y}_{LT'}$ | ${}^cR^{0y}_{LT}$ | ${}^sR^{z'0}_{LT}$ | ${}^cR^{z'0}_{LT'}$ |
| | $\mathcal{O}^a_{1-}$ | $\mathcal{O}^a_{2+}$ | $\mathcal{O}^e_{1-}$ | $\mathcal{O}^e_{2-}$ | $\mathcal{O}^g_{1+}$ | $\mathcal{O}^g_{2+}$ |
| $(a,e,g):114$ | $R^{0x}_{TT'}$ | $R^{0z}_{TT'}$ | ${}^sR^{0y}_{LT'}$ | ${}^cR^{0y}_{LT}$ | ${}^sR^{z'0}_{LT}$ | ${}^sR^{x'0}_{LT}$ |
| | $\mathcal{O}^a_{1-}$ | $\mathcal{O}^a_{2+}$ | $\mathcal{O}^e_{1-}$ | $\mathcal{O}^e_{2-}$ | $\mathcal{O}^g_{1+}$ | $\mathcal{O}^g_{2-}$ |
| $(a,e,g):115$ | $R^{0x}_{TT'}$ | $R^{0z}_{TT'}$ | ${}^sR^{0y}_{LT'}$ | ${}^cR^{0y}_{LT}$ | ${}^cR^{x'0}_{LT'}$ | ${}^cR^{z'0}_{LT'}$ |
| | $\mathcal{O}^a_{1-}$ | $\mathcal{O}^a_{2+}$ | $\mathcal{O}^e_{1-}$ | $\mathcal{O}^e_{2-}$ | $\mathcal{O}^g_{1-}$ | $\mathcal{O}^g_{2+}$ |
| $(a,e,g):116$ | $R^{0x}_{TT'}$ | $R^{0z}_{TT'}$ | ${}^sR^{0y}_{LT'}$ | ${}^cR^{0y}_{LT}$ | ${}^cR^{x'0}_{LT'}$ | ${}^sR^{x'0}_{LT}$ |
| | $\mathcal{O}^a_{1-}$ | $\mathcal{O}^a_{2+}$ | $\mathcal{O}^e_{1-}$ | $\mathcal{O}^e_{2-}$ | $\mathcal{O}^g_{1-}$ | $\mathcal{O}^g_{2-}$ |
| $(a,e,g):117$ | $R^{0x}_{TT'}$ | ${}^sR^{0x}_{TT}$ | ${}^sR^{00}_{LT'}$ | ${}^sR^{0y}_{LT'}$ | ${}^sR^{z'0}_{LT}$ | ${}^cR^{x'0}_{LT'}$ |
| | $\mathcal{O}^a_{1-}$ | $\mathcal{O}^a_{2-}$ | $\mathcal{O}^e_{1+}$ | $\mathcal{O}^e_{1-}$ | $\mathcal{O}^g_{1+}$ | $\mathcal{O}^g_{1-}$ |
| $(a,e,g):118$ | $R^{0x}_{TT'}$ | ${}^sR^{0x}_{TT}$ | ${}^sR^{00}_{LT'}$ | ${}^sR^{0y}_{LT'}$ | ${}^cR^{z'0}_{LT'}$ | ${}^sR^{x'0}_{LT}$ |
| | $\mathcal{O}^a_{1-}$ | $\mathcal{O}^a_{2-}$ | $\mathcal{O}^e_{1+}$ | $\mathcal{O}^e_{1-}$ | $\mathcal{O}^g_{2+}$ | $\mathcal{O}^g_{2-}$ |
| $(a,e,g):119$ | $R^{0x}_{TT'}$ | ${}^sR^{0x}_{TT}$ | ${}^sR^{00}_{LT'}$ | ${}^sR^{0y}_{LT'}$ | ${}^sR^{z'0}_{LT}$ | ${}^cR^{z'0}_{LT'}$ |
| | $\mathcal{O}^a_{1-}$ | $\mathcal{O}^a_{2-}$ | $\mathcal{O}^e_{1+}$ | $\mathcal{O}^e_{1-}$ | $\mathcal{O}^g_{1+}$ | $\mathcal{O}^g_{2+}$ |
| $(a,e,g):120$ | $R^{0x}_{TT'}$ | ${}^sR^{0x}_{TT}$ | ${}^sR^{00}_{LT'}$ | ${}^sR^{0y}_{LT'}$ | ${}^sR^{z'0}_{LT}$ | ${}^sR^{x'0}_{LT}$ |
| | $\mathcal{O}^a_{1-}$ | $\mathcal{O}^a_{2-}$ | $\mathcal{O}^e_{1+}$ | $\mathcal{O}^e_{1-}$ | $\mathcal{O}^g_{1+}$ | $\mathcal{O}^g_{2-}$ |
| $(a,e,g):121$ | $R^{0x}_{TT'}$ | ${}^sR^{0x}_{TT}$ | ${}^sR^{00}_{LT'}$ | ${}^sR^{0y}_{LT'}$ | ${}^cR^{x'0}_{LT'}$ | ${}^cR^{z'0}_{LT'}$ |
| | $\mathcal{O}^a_{1-}$ | $\mathcal{O}^a_{2-}$ | $\mathcal{O}^e_{1+}$ | $\mathcal{O}^e_{1-}$ | $\mathcal{O}^g_{1-}$ | $\mathcal{O}^g_{2+}$ |
| $(a,e,g):122$ | $R^{0x}_{TT'}$ | ${}^sR^{0x}_{TT}$ | ${}^sR^{00}_{LT'}$ | ${}^sR^{0y}_{LT'}$ | ${}^cR^{x'0}_{LT'}$ | ${}^sR^{x'0}_{LT}$ |
| | $\mathcal{O}^a_{1-}$ | $\mathcal{O}^a_{2-}$ | $\mathcal{O}^e_{1+}$ | $\mathcal{O}^e_{1-}$ | $\mathcal{O}^g_{1-}$ | $\mathcal{O}^g_{2-}$ |
| $(a,e,g):123$ | $R^{0x}_{TT'}$ | ${}^sR^{0x}_{TT}$ | ${}^cR^{00}_{LT}$ | ${}^cR^{0y}_{LT}$ | ${}^sR^{z'0}_{LT}$ | ${}^cR^{x'0}_{LT'}$ |
| | $\mathcal{O}^a_{1-}$ | $\mathcal{O}^a_{2-}$ | $\mathcal{O}^e_{2+}$ | $\mathcal{O}^e_{2-}$ | $\mathcal{O}^g_{1+}$ | $\mathcal{O}^g_{1-}$ |
| $(a,e,g):124$ | $R^{0x}_{TT'}$ | ${}^sR^{0x}_{TT}$ | ${}^cR^{00}_{LT}$ | ${}^cR^{0y}_{LT}$ | ${}^cR^{z'0}_{LT'}$ | ${}^sR^{x'0}_{LT}$ |
| | $\mathcal{O}^a_{1-}$ | $\mathcal{O}^a_{2-}$ | $\mathcal{O}^e_{2+}$ | $\mathcal{O}^e_{2-}$ | $\mathcal{O}^g_{2+}$ | $\mathcal{O}^g_{2-}$ |
| $(a,e,g):125$ | $R^{0x}_{TT'}$ | ${}^sR^{0x}_{TT}$ | ${}^cR^{00}_{LT}$ | ${}^cR^{0y}_{LT}$ | ${}^sR^{z'0}_{LT}$ | ${}^cR^{z'0}_{LT'}$ |
| | $\mathcal{O}^a_{1-}$ | $\mathcal{O}^a_{2-}$ | $\mathcal{O}^e_{2+}$ | $\mathcal{O}^e_{2-}$ | $\mathcal{O}^g_{1+}$ | $\mathcal{O}^g_{2+}$ |
| $(a,e,g):126$ | $R^{0x}_{TT'}$ | ${}^sR^{0x}_{TT}$ | ${}^cR^{00}_{LT}$ | ${}^cR^{0y}_{LT}$ | ${}^sR^{z'0}_{LT}$ | ${}^sR^{x'0}_{LT}$ |
| | $\mathcal{O}^a_{1-}$ | $\mathcal{O}^a_{2-}$ | $\mathcal{O}^e_{2+}$ | $\mathcal{O}^e_{2-}$ | $\mathcal{O}^g_{1+}$ | $\mathcal{O}^g_{2-}$ |
| $(a,e,g):127$ | $R^{0x}_{TT'}$ | ${}^sR^{0x}_{TT}$ | ${}^cR^{00}_{LT}$ | ${}^cR^{0y}_{LT}$ | ${}^cR^{x'0}_{LT'}$ | ${}^cR^{z'0}_{LT'}$ |
| | $\mathcal{O}^a_{1-}$ | $\mathcal{O}^a_{2-}$ | $\mathcal{O}^e_{2+}$ | $\mathcal{O}^e_{2-}$ | $\mathcal{O}^g_{1-}$ | $\mathcal{O}^g_{2+}$ |
| $(a,e,g):128$ | $R^{0x}_{TT'}$ | ${}^sR^{0x}_{TT}$ | ${}^cR^{00}_{LT}$ | ${}^cR^{0y}_{LT}$ | ${}^cR^{x'0}_{LT'}$ | ${}^sR^{x'0}_{LT}$ |
| | $\mathcal{O}^a_{1-}$ | $\mathcal{O}^a_{2-}$ | $\mathcal{O}^e_{2+}$ | $\mathcal{O}^e_{2-}$ | $\mathcal{O}^g_{1-}$ | $\mathcal{O}^g_{2-}$ |
| $(a,e,g):129$ | $R^{0x}_{TT'}$ | ${}^sR^{0x}_{TT}$ | ${}^sR^{00}_{LT'}$ | ${}^cR^{00}_{LT}$ | ${}^sR^{z'0}_{LT}$ | ${}^cR^{x'0}_{LT'}$ |
| | $\mathcal{O}^a_{1-}$ | $\mathcal{O}^a_{2-}$ | $\mathcal{O}^e_{1+}$ | $\mathcal{O}^e_{2+}$ | $\mathcal{O}^g_{1+}$ | $\mathcal{O}^g_{1-}$ |
| $(a,e,g):130$ | $R^{0x}_{TT'}$ | ${}^sR^{0x}_{TT}$ | ${}^sR^{00}_{LT'}$ | ${}^cR^{00}_{LT}$ | ${}^cR^{z'0}_{LT'}$ | ${}^sR^{x'0}_{LT}$ |
| | $\mathcal{O}^a_{1-}$ | $\mathcal{O}^a_{2-}$ | $\mathcal{O}^e_{1+}$ | $\mathcal{O}^e_{2+}$ | $\mathcal{O}^g_{2+}$ | $\mathcal{O}^g_{2-}$ |
| $(a,e,g):131$ | $R^{0x}_{TT'}$ | ${}^sR^{0x}_{TT}$ | ${}^sR^{00}_{LT'}$ | ${}^cR^{00}_{LT}$ | ${}^sR^{z'0}_{LT}$ | ${}^cR^{z'0}_{LT'}$ |
| | $\mathcal{O}^a_{1-}$ | $\mathcal{O}^a_{2-}$ | $\mathcal{O}^e_{1+}$ | $\mathcal{O}^e_{2+}$ | $\mathcal{O}^g_{1+}$ | $\mathcal{O}^g_{2+}$ |
| $(a,e,g):132$ | $R^{0x}_{TT'}$ | ${}^sR^{0x}_{TT}$ | ${}^sR^{00}_{LT'}$ | ${}^cR^{00}_{LT}$ | ${}^sR^{z'0}_{LT}$ | ${}^sR^{x'0}_{LT}$ |
| | $\mathcal{O}^a_{1-}$ | $\mathcal{O}^a_{2-}$ | $\mathcal{O}^e_{1+}$ | $\mathcal{O}^e_{2+}$ | $\mathcal{O}^g_{1+}$ | $\mathcal{O}^g_{2-}$ |
| $(a,e,g):133$ | $R^{0x}_{TT'}$ | ${}^sR^{0x}_{TT}$ | ${}^sR^{00}_{LT'}$ | ${}^cR^{00}_{LT}$ | ${}^cR^{x'0}_{LT'}$ | ${}^cR^{z'0}_{LT'}$ |
| | $\mathcal{O}^a_{1-}$ | $\mathcal{O}^a_{2-}$ | $\mathcal{O}^e_{1+}$ | $\mathcal{O}^e_{2+}$ | $\mathcal{O}^g_{1-}$ | $\mathcal{O}^g_{2+}$ |
| $(a,e,g):134$ | $R^{0x}_{TT'}$ | ${}^sR^{0x}_{TT}$ | ${}^sR^{00}_{LT'}$ | ${}^cR^{00}_{LT}$ | ${}^cR^{x'0}_{LT'}$ | ${}^sR^{x'0}_{LT}$ |
| | $\mathcal{O}^a_{1-}$ | $\mathcal{O}^a_{2-}$ | $\mathcal{O}^e_{1+}$ | $\mathcal{O}^e_{2+}$ | $\mathcal{O}^g_{1-}$ | $\mathcal{O}^g_{2-}$ |
| $(a,e,g):135$ | $R^{0x}_{TT'}$ | ${}^sR^{0x}_{TT}$ | ${}^sR^{00}_{LT'}$ | ${}^cR^{0y}_{LT}$ | ${}^sR^{z'0}_{LT}$ | ${}^cR^{x'0}_{LT'}$ |
| | $\mathcal{O}^a_{1-}$ | $\mathcal{O}^a_{2-}$ | $\mathcal{O}^e_{1+}$ | $\mathcal{O}^e_{2-}$ | $\mathcal{O}^g_{1+}$ | $\mathcal{O}^g_{1-}$ |
| $(a,e,g):136$ | $R^{0x}_{TT'}$ | ${}^sR^{0x}_{TT}$ | ${}^sR^{00}_{LT'}$ | ${}^cR^{0y}_{LT}$ | ${}^cR^{z'0}_{LT'}$ | ${}^sR^{x'0}_{LT}$ |
| | $\mathcal{O}^a_{1-}$ | $\mathcal{O}^a_{2-}$ | $\mathcal{O}^e_{1+}$ | $\mathcal{O}^e_{2-}$ | $\mathcal{O}^g_{2+}$ | $\mathcal{O}^g_{2-}$ |
| $(a,e,g):137$ | $R^{0x}_{TT'}$ | ${}^sR^{0x}_{TT}$ | ${}^sR^{00}_{LT'}$ | ${}^cR^{0y}_{LT}$ | ${}^sR^{z'0}_{LT}$ | ${}^cR^{z'0}_{LT'}$ |
| | $\mathcal{O}^a_{1-}$ | $\mathcal{O}^a_{2-}$ | $\mathcal{O}^e_{1+}$ | $\mathcal{O}^e_{2-}$ | $\mathcal{O}^g_{1+}$ | $\mathcal{O}^g_{2+}$ |
| $(a,e,g):138$ | $R^{0x}_{TT'}$ | ${}^sR^{0x}_{TT}$ | ${}^sR^{00}_{LT'}$ | ${}^cR^{0y}_{LT}$ | ${}^sR^{z'0}_{LT}$ | ${}^sR^{x'0}_{LT}$ |
| | $\mathcal{O}^a_{1-}$ | $\mathcal{O}^a_{2-}$ | $\mathcal{O}^e_{1+}$ | $\mathcal{O}^e_{2-}$ | $\mathcal{O}^g_{1+}$ | $\mathcal{O}^g_{2-}$ |
| $(a,e,g):139$ | $R^{0x}_{TT'}$ | ${}^sR^{0x}_{TT}$ | ${}^sR^{00}_{LT'}$ | ${}^cR^{0y}_{LT}$ | ${}^cR^{x'0}_{LT'}$ | ${}^cR^{z'0}_{LT'}$ |

| | | | | | | |
|---|---|---|---|---|---|---|
| | $\mathcal{O}^{a}_{1-}$ | $\mathcal{O}^{a}_{2-}$ | $\mathcal{O}^{e}_{1+}$ | $\mathcal{O}^{e}_{2-}$ | $\mathcal{O}^{g}_{1-}$ | $\mathcal{O}^{g}_{2+}$ |
| $(a,e,g):140$ | $R^{0x}_{TT'}$ | ${}^{s}R^{0x}_{TT}$ | ${}^{s}R^{00}_{LT'}$ | ${}^{c}R^{0y}_{LT}$ | ${}^{c}R^{x'0}_{LT'}$ | ${}^{s}R^{x'0}_{LT}$ |
| | $\mathcal{O}^{a}_{1-}$ | $\mathcal{O}^{a}_{2-}$ | $\mathcal{O}^{e}_{1+}$ | $\mathcal{O}^{e}_{2-}$ | $\mathcal{O}^{g}_{1-}$ | $\mathcal{O}^{g}_{2-}$ |
| $(a,e,g):141$ | $R^{0x}_{TT'}$ | ${}^{s}R^{0x}_{TT}$ | ${}^{s}R^{0y}_{LT'}$ | ${}^{c}R^{00}_{LT}$ | ${}^{s}R^{z'0}_{LT}$ | ${}^{c}R^{x'0}_{LT'}$ |
| | $\mathcal{O}^{a}_{1-}$ | $\mathcal{O}^{a}_{2-}$ | $\mathcal{O}^{e}_{1-}$ | $\mathcal{O}^{e}_{2+}$ | $\mathcal{O}^{g}_{1+}$ | $\mathcal{O}^{g}_{1-}$ |
| $(a,e,g):142$ | $R^{0x}_{TT'}$ | ${}^{s}R^{0x}_{TT}$ | ${}^{s}R^{0y}_{LT'}$ | ${}^{c}R^{00}_{LT}$ | ${}^{c}R^{z'0}_{LT'}$ | ${}^{s}R^{x'0}_{LT}$ |
| | $\mathcal{O}^{a}_{1-}$ | $\mathcal{O}^{a}_{2-}$ | $\mathcal{O}^{e}_{1-}$ | $\mathcal{O}^{e}_{2+}$ | $\mathcal{O}^{g}_{2+}$ | $\mathcal{O}^{g}_{2-}$ |
| $(a,e,g):143$ | $R^{0x}_{TT'}$ | ${}^{s}R^{0x}_{TT}$ | ${}^{s}R^{0y}_{LT'}$ | ${}^{c}R^{00}_{LT}$ | ${}^{s}R^{z'0}_{LT}$ | ${}^{c}R^{z'0}_{LT'}$ |
| | $\mathcal{O}^{a}_{1-}$ | $\mathcal{O}^{a}_{2-}$ | $\mathcal{O}^{e}_{1-}$ | $\mathcal{O}^{e}_{2+}$ | $\mathcal{O}^{g}_{1+}$ | $\mathcal{O}^{g}_{2+}$ |
| $(a,e,g):144$ | $R^{0x}_{TT'}$ | ${}^{s}R^{0x}_{TT}$ | ${}^{s}R^{0y}_{LT'}$ | ${}^{c}R^{00}_{LT}$ | ${}^{s}R^{z'0}_{LT}$ | ${}^{s}R^{x'0}_{LT}$ |
| | $\mathcal{O}^{a}_{1-}$ | $\mathcal{O}^{a}_{2-}$ | $\mathcal{O}^{e}_{1-}$ | $\mathcal{O}^{e}_{2+}$ | $\mathcal{O}^{g}_{1+}$ | $\mathcal{O}^{g}_{2-}$ |
| $(a,e,g):145$ | $R^{0x}_{TT'}$ | ${}^{s}R^{0x}_{TT}$ | ${}^{s}R^{0y}_{LT'}$ | ${}^{c}R^{00}_{LT}$ | ${}^{c}R^{x'0}_{LT'}$ | ${}^{c}R^{z'0}_{LT'}$ |
| | $\mathcal{O}^{a}_{1-}$ | $\mathcal{O}^{a}_{2-}$ | $\mathcal{O}^{e}_{1-}$ | $\mathcal{O}^{e}_{2+}$ | $\mathcal{O}^{g}_{1-}$ | $\mathcal{O}^{g}_{2+}$ |
| $(a,e,g):146$ | $R^{0x}_{TT'}$ | ${}^{s}R^{0x}_{TT}$ | ${}^{s}R^{0y}_{LT'}$ | ${}^{c}R^{00}_{LT}$ | ${}^{c}R^{x'0}_{LT'}$ | ${}^{s}R^{x'0}_{LT}$ |
| | $\mathcal{O}^{a}_{1-}$ | $\mathcal{O}^{a}_{2-}$ | $\mathcal{O}^{e}_{1-}$ | $\mathcal{O}^{e}_{2+}$ | $\mathcal{O}^{g}_{1-}$ | $\mathcal{O}^{g}_{2-}$ |
| $(a,e,g):147$ | $R^{0x}_{TT'}$ | ${}^{s}R^{0x}_{TT}$ | ${}^{s}R^{0y}_{LT'}$ | ${}^{c}R^{0y}_{LT}$ | ${}^{s}R^{z'0}_{LT}$ | ${}^{c}R^{x'0}_{LT'}$ |
| | $\mathcal{O}^{a}_{1-}$ | $\mathcal{O}^{a}_{2-}$ | $\mathcal{O}^{e}_{1-}$ | $\mathcal{O}^{e}_{2-}$ | $\mathcal{O}^{g}_{1+}$ | $\mathcal{O}^{g}_{1-}$ |
| $(a,e,g):148$ | $R^{0x}_{TT'}$ | ${}^{s}R^{0x}_{TT}$ | ${}^{s}R^{0y}_{LT'}$ | ${}^{c}R^{0y}_{LT}$ | ${}^{c}R^{z'0}_{LT'}$ | ${}^{s}R^{x'0}_{LT}$ |
| | $\mathcal{O}^{a}_{1-}$ | $\mathcal{O}^{a}_{2-}$ | $\mathcal{O}^{e}_{1-}$ | $\mathcal{O}^{e}_{2-}$ | $\mathcal{O}^{g}_{2+}$ | $\mathcal{O}^{g}_{2-}$ |
| $(a,e,g):149$ | $R^{0x}_{TT'}$ | ${}^{s}R^{0x}_{TT}$ | ${}^{s}R^{0y}_{LT'}$ | ${}^{c}R^{0y}_{LT}$ | ${}^{s}R^{z'0}_{LT}$ | ${}^{c}R^{z'0}_{LT'}$ |
| | $\mathcal{O}^{a}_{1-}$ | $\mathcal{O}^{a}_{2-}$ | $\mathcal{O}^{e}_{1-}$ | $\mathcal{O}^{e}_{2-}$ | $\mathcal{O}^{g}_{1+}$ | $\mathcal{O}^{g}_{2+}$ |
| $(a,e,g):150$ | $R^{0x}_{TT'}$ | ${}^{s}R^{0x}_{TT}$ | ${}^{s}R^{0y}_{LT'}$ | ${}^{c}R^{0y}_{LT}$ | ${}^{s}R^{z'0}_{LT}$ | ${}^{s}R^{x'0}_{LT}$ |
| | $\mathcal{O}^{a}_{1-}$ | $\mathcal{O}^{a}_{2-}$ | $\mathcal{O}^{e}_{1-}$ | $\mathcal{O}^{e}_{2-}$ | $\mathcal{O}^{g}_{1+}$ | $\mathcal{O}^{g}_{2-}$ |
| $(a,e,g):151$ | $R^{0x}_{TT'}$ | ${}^{s}R^{0x}_{TT}$ | ${}^{s}R^{0y}_{LT'}$ | ${}^{c}R^{0y}_{LT}$ | ${}^{c}R^{x'0}_{LT'}$ | ${}^{c}R^{z'0}_{LT'}$ |
| | $\mathcal{O}^{a}_{1-}$ | $\mathcal{O}^{a}_{2-}$ | $\mathcal{O}^{e}_{1-}$ | $\mathcal{O}^{e}_{2-}$ | $\mathcal{O}^{g}_{1-}$ | $\mathcal{O}^{g}_{2+}$ |
| $(a,e,g):152$ | $R^{0x}_{TT'}$ | ${}^{s}R^{0x}_{TT}$ | ${}^{s}R^{0y}_{LT'}$ | ${}^{c}R^{0y}_{LT}$ | ${}^{c}R^{x'0}_{LT'}$ | ${}^{s}R^{x'0}_{LT}$ |
| | $\mathcal{O}^{a}_{1-}$ | $\mathcal{O}^{a}_{2-}$ | $\mathcal{O}^{e}_{1-}$ | $\mathcal{O}^{e}_{2-}$ | $\mathcal{O}^{g}_{1-}$ | $\mathcal{O}^{g}_{2-}$ |

TABLE V: All the fully complete sets determined from the combination of shape-classes $(a,f,h)$ (i.e. graph-topology 'II') in the case of pseudoscalar meson electroproduction are listed here. The observables are written in the systematic symbolic notation $\mathcal{O}^{n}_{\nu\pm}$ by Nakayama [1], as well as in the more commonly used notation in terms of 'response-functions' $R^{\beta\alpha}_{i}$ (cf. references [4, 5]). The given sets of 6 observables have to be combined with the 6 'diagonal' observables $\left\{R^{00}_{T}, {}^{c}R^{00}_{TT}, R^{0y}_{T}, R^{y'0}_{T}, R^{00}_{L}, R^{0y}_{L}\right\}$ in order to form a complete set of minimal length $2N = 12$. All of these sets have been verified to be complete using Mathematica [3].

| Set-Nr. | Observables | | | | | |
|---|---|---|---|---|---|---|
| $(a,f,h):1$ | ${}^{s}R^{0z}_{TT}$ | $R^{0x}_{TT'}$ | ${}^{s}R^{0z}_{LT}$ | ${}^{c}R^{0x}_{LT'}$ | ${}^{s}R^{x'x}_{LT'}$ | ${}^{c}R^{x'x}_{LT}$ |
| | $\mathcal{O}^{a}_{1+}$ | $\mathcal{O}^{a}_{1-}$ | $\mathcal{O}^{f}_{1+}$ | $\mathcal{O}^{f}_{1-}$ | $\mathcal{O}^{h}_{1+}$ | $\mathcal{O}^{h}_{2+}$ |
| $(a,f,h):2$ | ${}^{s}R^{0z}_{TT}$ | $R^{0x}_{TT'}$ | ${}^{s}R^{0z}_{LT}$ | ${}^{c}R^{0x}_{LT'}$ | ${}^{c}R^{z'x}_{LT}$ | ${}^{s}R^{z'x}_{LT'}$ |
| | $\mathcal{O}^{a}_{1+}$ | $\mathcal{O}^{a}_{1-}$ | $\mathcal{O}^{f}_{1+}$ | $\mathcal{O}^{f}_{1-}$ | $\mathcal{O}^{h}_{1-}$ | $\mathcal{O}^{h}_{2-}$ |
| $(a,f,h):3$ | ${}^{s}R^{0z}_{TT}$ | $R^{0x}_{TT'}$ | ${}^{c}R^{0z}_{LT'}$ | ${}^{s}R^{0x}_{LT}$ | ${}^{s}R^{x'x}_{LT'}$ | ${}^{c}R^{x'x}_{LT}$ |
| | $\mathcal{O}^{a}_{1+}$ | $\mathcal{O}^{a}_{1-}$ | $\mathcal{O}^{f}_{2+}$ | $\mathcal{O}^{f}_{2-}$ | $\mathcal{O}^{h}_{1+}$ | $\mathcal{O}^{h}_{2+}$ |
| $(a,f,h):4$ | ${}^{s}R^{0z}_{TT}$ | $R^{0x}_{TT'}$ | ${}^{c}R^{0z}_{LT'}$ | ${}^{s}R^{0x}_{LT}$ | ${}^{c}R^{z'x}_{LT}$ | ${}^{s}R^{z'x}_{LT'}$ |
| | $\mathcal{O}^{a}_{1+}$ | $\mathcal{O}^{a}_{1-}$ | $\mathcal{O}^{f}_{2+}$ | $\mathcal{O}^{f}_{2-}$ | $\mathcal{O}^{h}_{1-}$ | $\mathcal{O}^{h}_{2-}$ |
| $(a,f,h):5$ | ${}^{s}R^{0z}_{TT}$ | $R^{0x}_{TT'}$ | ${}^{s}R^{0z}_{LT}$ | ${}^{c}R^{0z}_{LT'}$ | ${}^{s}R^{x'x}_{LT'}$ | ${}^{c}R^{z'x}_{LT}$ |
| | $\mathcal{O}^{a}_{1+}$ | $\mathcal{O}^{a}_{1-}$ | $\mathcal{O}^{f}_{1+}$ | $\mathcal{O}^{f}_{2+}$ | $\mathcal{O}^{h}_{1+}$ | $\mathcal{O}^{h}_{1-}$ |
| $(a,f,h):6$ | ${}^{s}R^{0z}_{TT}$ | $R^{0x}_{TT'}$ | ${}^{s}R^{0z}_{LT}$ | ${}^{c}R^{0z}_{LT'}$ | ${}^{c}R^{x'x}_{LT}$ | ${}^{s}R^{z'x}_{LT'}$ |
| | $\mathcal{O}^{a}_{1+}$ | $\mathcal{O}^{a}_{1-}$ | $\mathcal{O}^{f}_{1+}$ | $\mathcal{O}^{f}_{2+}$ | $\mathcal{O}^{h}_{2+}$ | $\mathcal{O}^{h}_{2-}$ |
| $(a,f,h):7$ | ${}^{s}R^{0z}_{TT}$ | $R^{0x}_{TT'}$ | ${}^{s}R^{0z}_{LT}$ | ${}^{c}R^{0z}_{LT'}$ | ${}^{s}R^{x'x}_{LT'}$ | ${}^{c}R^{x'x}_{LT}$ |
| | $\mathcal{O}^{a}_{1+}$ | $\mathcal{O}^{a}_{1-}$ | $\mathcal{O}^{f}_{1+}$ | $\mathcal{O}^{f}_{2+}$ | $\mathcal{O}^{h}_{1+}$ | $\mathcal{O}^{h}_{2+}$ |
| $(a,f,h):8$ | ${}^{s}R^{0z}_{TT}$ | $R^{0x}_{TT'}$ | ${}^{s}R^{0z}_{LT}$ | ${}^{c}R^{0z}_{LT'}$ | ${}^{s}R^{x'x}_{LT'}$ | ${}^{s}R^{z'x}_{LT'}$ |

| | | | | | | |
|---|---|---|---|---|---|---|
| | $\mathcal{O}^a_{1+}$ | $\mathcal{O}^a_{1-}$ | $\mathcal{O}^f_{1+}$ | $\mathcal{O}^f_{2+}$ | $\mathcal{O}^h_{1+}$ | $\mathcal{O}^h_{2-}$ |
| $(a,f,h):9$ | ${}^sR^{0z}_{TT}$ | $R^{0x}_{TT'}$ | ${}^sR^{0z}_{LT}$ | ${}^cR^{0z}_{LT'}$ | ${}^cR^{z'x}_{LT}$ | ${}^cR^{x'x}_{LT}$ |
| | $\mathcal{O}^a_{1+}$ | $\mathcal{O}^a_{1-}$ | $\mathcal{O}^f_{1+}$ | $\mathcal{O}^f_{2+}$ | $\mathcal{O}^h_{1-}$ | $\mathcal{O}^h_{2+}$ |
| $(a,f,h):10$ | ${}^sR^{0z}_{TT}$ | $R^{0x}_{TT'}$ | ${}^sR^{0z}_{LT}$ | ${}^cR^{0z}_{LT'}$ | ${}^cR^{z'x}_{LT}$ | ${}^sR^{z'x}_{LT'}$ |
| | $\mathcal{O}^a_{1+}$ | $\mathcal{O}^a_{1-}$ | $\mathcal{O}^f_{1+}$ | $\mathcal{O}^f_{2+}$ | $\mathcal{O}^h_{1-}$ | $\mathcal{O}^h_{2-}$ |
| $(a,f,h):11$ | ${}^sR^{0z}_{TT}$ | $R^{0x}_{TT'}$ | ${}^sR^{0z}_{LT}$ | ${}^sR^{0x}_{LT}$ | ${}^sR^{x'x}_{LT'}$ | ${}^cR^{x'x}_{LT}$ |
| | $\mathcal{O}^a_{1+}$ | $\mathcal{O}^a_{1-}$ | $\mathcal{O}^f_{1+}$ | $\mathcal{O}^f_{2-}$ | $\mathcal{O}^h_{1+}$ | $\mathcal{O}^h_{2+}$ |
| $(a,f,h):12$ | ${}^sR^{0z}_{TT}$ | $R^{0x}_{TT'}$ | ${}^sR^{0z}_{LT}$ | ${}^sR^{0x}_{LT}$ | ${}^cR^{z'x}_{LT}$ | ${}^sR^{z'x}_{LT'}$ |
| | $\mathcal{O}^a_{1+}$ | $\mathcal{O}^a_{1-}$ | $\mathcal{O}^f_{1+}$ | $\mathcal{O}^f_{2-}$ | $\mathcal{O}^h_{1-}$ | $\mathcal{O}^h_{2-}$ |
| $(a,f,h):13$ | ${}^sR^{0z}_{TT}$ | $R^{0x}_{TT'}$ | ${}^cR^{0x}_{LT'}$ | ${}^cR^{0z}_{LT'}$ | ${}^sR^{x'x}_{LT'}$ | ${}^cR^{x'x}_{LT}$ |
| | $\mathcal{O}^a_{1+}$ | $\mathcal{O}^a_{1-}$ | $\mathcal{O}^f_{1-}$ | $\mathcal{O}^f_{2+}$ | $\mathcal{O}^h_{1+}$ | $\mathcal{O}^h_{2+}$ |
| $(a,f,h):14$ | ${}^sR^{0z}_{TT}$ | $R^{0x}_{TT'}$ | ${}^cR^{0x}_{LT'}$ | ${}^cR^{0z}_{LT'}$ | ${}^cR^{z'x}_{LT}$ | ${}^sR^{z'x}_{LT'}$ |
| | $\mathcal{O}^a_{1+}$ | $\mathcal{O}^a_{1-}$ | $\mathcal{O}^f_{1-}$ | $\mathcal{O}^f_{2+}$ | $\mathcal{O}^h_{1-}$ | $\mathcal{O}^h_{2-}$ |
| $(a,f,h):15$ | ${}^sR^{0z}_{TT}$ | $R^{0x}_{TT'}$ | ${}^cR^{0x}_{LT'}$ | ${}^sR^{0x}_{LT}$ | ${}^sR^{x'x}_{LT'}$ | ${}^cR^{z'x}_{LT}$ |
| | $\mathcal{O}^a_{1+}$ | $\mathcal{O}^a_{1-}$ | $\mathcal{O}^f_{1-}$ | $\mathcal{O}^f_{2-}$ | $\mathcal{O}^h_{1+}$ | $\mathcal{O}^h_{1-}$ |
| $(a,f,h):16$ | ${}^sR^{0z}_{TT}$ | $R^{0x}_{TT'}$ | ${}^cR^{0x}_{LT'}$ | ${}^sR^{0x}_{LT}$ | ${}^cR^{x'x}_{LT}$ | ${}^sR^{z'x}_{LT'}$ |
| | $\mathcal{O}^a_{1+}$ | $\mathcal{O}^a_{1-}$ | $\mathcal{O}^f_{1-}$ | $\mathcal{O}^f_{2-}$ | $\mathcal{O}^h_{2+}$ | $\mathcal{O}^h_{2-}$ |
| $(a,f,h):17$ | ${}^sR^{0z}_{TT}$ | $R^{0x}_{TT'}$ | ${}^cR^{0x}_{LT'}$ | ${}^sR^{0x}_{LT}$ | ${}^sR^{x'x}_{LT'}$ | ${}^cR^{x'x}_{LT}$ |
| | $\mathcal{O}^a_{1+}$ | $\mathcal{O}^a_{1-}$ | $\mathcal{O}^f_{1-}$ | $\mathcal{O}^f_{2-}$ | $\mathcal{O}^h_{1+}$ | $\mathcal{O}^h_{2+}$ |
| $(a,f,h):18$ | ${}^sR^{0z}_{TT}$ | $R^{0x}_{TT'}$ | ${}^cR^{0x}_{LT'}$ | ${}^sR^{0x}_{LT}$ | ${}^sR^{x'x}_{LT'}$ | ${}^sR^{z'x}_{LT'}$ |
| | $\mathcal{O}^a_{1+}$ | $\mathcal{O}^a_{1-}$ | $\mathcal{O}^f_{1-}$ | $\mathcal{O}^f_{2-}$ | $\mathcal{O}^h_{1+}$ | $\mathcal{O}^h_{2-}$ |
| $(a,f,h):19$ | ${}^sR^{0z}_{TT}$ | $R^{0x}_{TT'}$ | ${}^cR^{0x}_{LT'}$ | ${}^sR^{0x}_{LT}$ | ${}^cR^{z'x}_{LT}$ | ${}^cR^{x'x}_{LT}$ |
| | $\mathcal{O}^a_{1+}$ | $\mathcal{O}^a_{1-}$ | $\mathcal{O}^f_{1-}$ | $\mathcal{O}^f_{2-}$ | $\mathcal{O}^h_{1-}$ | $\mathcal{O}^h_{2+}$ |
| $(a,f,h):20$ | ${}^sR^{0z}_{TT}$ | $R^{0x}_{TT'}$ | ${}^cR^{0x}_{LT'}$ | ${}^sR^{0x}_{LT}$ | ${}^cR^{z'x}_{LT}$ | ${}^sR^{z'x}_{LT'}$ |
| | $\mathcal{O}^a_{1+}$ | $\mathcal{O}^a_{1-}$ | $\mathcal{O}^f_{1-}$ | $\mathcal{O}^f_{2-}$ | $\mathcal{O}^h_{1-}$ | $\mathcal{O}^h_{2-}$ |
| $(a,f,h):21$ | $R^{0z}_{TT'}$ | ${}^sR^{0x}_{TT}$ | ${}^sR^{0z}_{LT}$ | ${}^cR^{0x}_{LT'}$ | ${}^sR^{x'x}_{LT'}$ | ${}^cR^{x'x}_{LT}$ |
| | $\mathcal{O}^a_{2+}$ | $\mathcal{O}^a_{2-}$ | $\mathcal{O}^f_{1+}$ | $\mathcal{O}^f_{1-}$ | $\mathcal{O}^h_{1+}$ | $\mathcal{O}^h_{2+}$ |
| $(a,f,h):22$ | $R^{0z}_{TT'}$ | ${}^sR^{0x}_{TT}$ | ${}^sR^{0z}_{LT}$ | ${}^cR^{0x}_{LT'}$ | ${}^cR^{z'x}_{LT}$ | ${}^sR^{z'x}_{LT'}$ |
| | $\mathcal{O}^a_{2+}$ | $\mathcal{O}^a_{2-}$ | $\mathcal{O}^f_{1+}$ | $\mathcal{O}^f_{1-}$ | $\mathcal{O}^h_{1-}$ | $\mathcal{O}^h_{2-}$ |
| $(a,f,h):23$ | $R^{0z}_{TT'}$ | ${}^sR^{0x}_{TT}$ | ${}^cR^{0z}_{LT'}$ | ${}^sR^{0x}_{LT}$ | ${}^sR^{x'x}_{LT'}$ | ${}^cR^{x'x}_{LT}$ |
| | $\mathcal{O}^a_{2+}$ | $\mathcal{O}^a_{2-}$ | $\mathcal{O}^f_{2+}$ | $\mathcal{O}^f_{2-}$ | $\mathcal{O}^h_{1+}$ | $\mathcal{O}^h_{2+}$ |
| $(a,f,h):24$ | $R^{0z}_{TT'}$ | ${}^sR^{0x}_{TT}$ | ${}^cR^{0z}_{LT'}$ | ${}^sR^{0x}_{LT}$ | ${}^cR^{z'x}_{LT}$ | ${}^sR^{z'x}_{LT'}$ |
| | $\mathcal{O}^a_{2+}$ | $\mathcal{O}^a_{2-}$ | $\mathcal{O}^f_{2+}$ | $\mathcal{O}^f_{2-}$ | $\mathcal{O}^h_{1-}$ | $\mathcal{O}^h_{2-}$ |
| $(a,f,h):25$ | $R^{0z}_{TT'}$ | ${}^sR^{0x}_{TT}$ | ${}^sR^{0z}_{LT}$ | ${}^cR^{0z}_{LT'}$ | ${}^sR^{x'x}_{LT'}$ | ${}^cR^{z'x}_{LT}$ |
| | $\mathcal{O}^a_{2+}$ | $\mathcal{O}^a_{2-}$ | $\mathcal{O}^f_{1+}$ | $\mathcal{O}^f_{2+}$ | $\mathcal{O}^h_{1+}$ | $\mathcal{O}^h_{1-}$ |
| $(a,f,h):26$ | $R^{0z}_{TT'}$ | ${}^sR^{0x}_{TT}$ | ${}^sR^{0z}_{LT}$ | ${}^cR^{0z}_{LT'}$ | ${}^cR^{x'x}_{LT}$ | ${}^sR^{z'x}_{LT'}$ |
| | $\mathcal{O}^a_{2+}$ | $\mathcal{O}^a_{2-}$ | $\mathcal{O}^f_{1+}$ | $\mathcal{O}^f_{2+}$ | $\mathcal{O}^h_{2+}$ | $\mathcal{O}^h_{2-}$ |
| $(a,f,h):27$ | $R^{0z}_{TT'}$ | ${}^sR^{0x}_{TT}$ | ${}^sR^{0z}_{LT}$ | ${}^cR^{0z}_{LT'}$ | ${}^sR^{x'x}_{LT'}$ | ${}^cR^{x'x}_{LT}$ |
| | $\mathcal{O}^a_{2+}$ | $\mathcal{O}^a_{2-}$ | $\mathcal{O}^f_{1+}$ | $\mathcal{O}^f_{2+}$ | $\mathcal{O}^h_{1+}$ | $\mathcal{O}^h_{2+}$ |
| $(a,f,h):28$ | $R^{0z}_{TT'}$ | ${}^sR^{0x}_{TT}$ | ${}^sR^{0z}_{LT}$ | ${}^cR^{0z}_{LT'}$ | ${}^sR^{x'x}_{LT'}$ | ${}^sR^{z'x}_{LT'}$ |
| | $\mathcal{O}^a_{2+}$ | $\mathcal{O}^a_{2-}$ | $\mathcal{O}^f_{1+}$ | $\mathcal{O}^f_{2+}$ | $\mathcal{O}^h_{1+}$ | $\mathcal{O}^h_{2-}$ |
| $(a,f,h):29$ | $R^{0z}_{TT'}$ | ${}^sR^{0x}_{TT}$ | ${}^sR^{0z}_{LT}$ | ${}^cR^{0z}_{LT'}$ | ${}^cR^{z'x}_{LT}$ | ${}^cR^{x'x}_{LT}$ |
| | $\mathcal{O}^a_{2+}$ | $\mathcal{O}^a_{2-}$ | $\mathcal{O}^f_{1+}$ | $\mathcal{O}^f_{2+}$ | $\mathcal{O}^h_{1-}$ | $\mathcal{O}^h_{2+}$ |
| $(a,f,h):30$ | $R^{0z}_{TT'}$ | ${}^sR^{0x}_{TT}$ | ${}^sR^{0z}_{LT}$ | ${}^cR^{0z}_{LT'}$ | ${}^cR^{z'x}_{LT}$ | ${}^sR^{z'x}_{LT'}$ |
| | $\mathcal{O}^a_{2+}$ | $\mathcal{O}^a_{2-}$ | $\mathcal{O}^f_{1+}$ | $\mathcal{O}^f_{2+}$ | $\mathcal{O}^h_{1-}$ | $\mathcal{O}^h_{2-}$ |
| $(a,f,h):31$ | $R^{0z}_{TT'}$ | ${}^sR^{0x}_{TT}$ | ${}^sR^{0z}_{LT}$ | ${}^sR^{0x}_{LT}$ | ${}^sR^{x'x}_{LT'}$ | ${}^cR^{x'x}_{LT}$ |
| | $\mathcal{O}^a_{2+}$ | $\mathcal{O}^a_{2-}$ | $\mathcal{O}^f_{1+}$ | $\mathcal{O}^f_{2-}$ | $\mathcal{O}^h_{1+}$ | $\mathcal{O}^h_{2+}$ |
| $(a,f,h):32$ | $R^{0z}_{TT'}$ | ${}^sR^{0x}_{TT}$ | ${}^sR^{0z}_{LT}$ | ${}^sR^{0x}_{LT}$ | ${}^cR^{z'x}_{LT}$ | ${}^sR^{z'x}_{LT'}$ |
| | $\mathcal{O}^a_{2+}$ | $\mathcal{O}^a_{2-}$ | $\mathcal{O}^f_{1+}$ | $\mathcal{O}^f_{2-}$ | $\mathcal{O}^h_{1-}$ | $\mathcal{O}^h_{2-}$ |
| $(a,f,h):33$ | $R^{0z}_{TT'}$ | ${}^sR^{0x}_{TT}$ | ${}^cR^{0x}_{LT'}$ | ${}^cR^{0z}_{LT'}$ | ${}^sR^{x'x}_{LT'}$ | ${}^cR^{x'x}_{LT}$ |
| | $\mathcal{O}^a_{2+}$ | $\mathcal{O}^a_{2-}$ | $\mathcal{O}^f_{1-}$ | $\mathcal{O}^f_{2+}$ | $\mathcal{O}^h_{1+}$ | $\mathcal{O}^h_{2+}$ |
| $(a,f,h):34$ | $R^{0z}_{TT'}$ | ${}^sR^{0x}_{TT}$ | ${}^cR^{0x}_{LT'}$ | ${}^cR^{0z}_{LT'}$ | ${}^cR^{z'x}_{LT}$ | ${}^sR^{z'x}_{LT'}$ |
| | $\mathcal{O}^a_{2+}$ | $\mathcal{O}^a_{2-}$ | $\mathcal{O}^f_{1-}$ | $\mathcal{O}^f_{2+}$ | $\mathcal{O}^h_{1-}$ | $\mathcal{O}^h_{2-}$ |
| $(a,f,h):35$ | $R^{0z}_{TT'}$ | ${}^sR^{0x}_{TT}$ | ${}^cR^{0x}_{LT'}$ | ${}^sR^{0x}_{LT}$ | ${}^sR^{x'x}_{LT'}$ | ${}^cR^{z'x}_{LT}$ |
| | $\mathcal{O}^a_{2+}$ | $\mathcal{O}^a_{2-}$ | $\mathcal{O}^f_{1-}$ | $\mathcal{O}^f_{2-}$ | $\mathcal{O}^h_{1+}$ | $\mathcal{O}^h_{1-}$ |

| | | | | | | |
|---|---|---|---|---|---|---|
| $(a,f,h):36$ | $R^{0z}_{TT'}$ | ${}^sR^{0x}_{TT}$ | ${}^cR^{0x}_{LT'}$ | ${}^sR^{0x}_{LT}$ | ${}^cR^{x'x}_{LT}$ | ${}^sR^{z'x}_{LT'}$ |
| | $\mathcal{O}^a_{2+}$ | $\mathcal{O}^a_{2-}$ | $\mathcal{O}^f_{1-}$ | $\mathcal{O}^f_{2-}$ | $\mathcal{O}^h_{2+}$ | $\mathcal{O}^h_{2-}$ |
| $(a,f,h):37$ | $R^{0z}_{TT'}$ | ${}^sR^{0x}_{TT}$ | ${}^cR^{0x}_{LT'}$ | ${}^sR^{0x}_{LT}$ | ${}^sR^{x'x}_{LT'}$ | ${}^cR^{x'x}_{LT}$ |
| | $\mathcal{O}^a_{2+}$ | $\mathcal{O}^a_{2-}$ | $\mathcal{O}^f_{1-}$ | $\mathcal{O}^f_{2-}$ | $\mathcal{O}^h_{1+}$ | $\mathcal{O}^h_{2+}$ |
| $(a,f,h):38$ | $R^{0z}_{TT'}$ | ${}^sR^{0x}_{TT}$ | ${}^cR^{0x}_{LT'}$ | ${}^sR^{0x}_{LT}$ | ${}^sR^{x'x}_{LT'}$ | ${}^sR^{z'x}_{LT'}$ |
| | $\mathcal{O}^a_{2+}$ | $\mathcal{O}^a_{2-}$ | $\mathcal{O}^f_{1-}$ | $\mathcal{O}^f_{2-}$ | $\mathcal{O}^h_{1+}$ | $\mathcal{O}^h_{2-}$ |
| $(a,f,h):39$ | $R^{0z}_{TT'}$ | ${}^sR^{0x}_{TT}$ | ${}^cR^{0x}_{LT'}$ | ${}^sR^{0x}_{LT}$ | ${}^cR^{z'x}_{LT}$ | ${}^cR^{x'x}_{LT}$ |
| | $\mathcal{O}^a_{2+}$ | $\mathcal{O}^a_{2-}$ | $\mathcal{O}^f_{1-}$ | $\mathcal{O}^f_{2-}$ | $\mathcal{O}^h_{1-}$ | $\mathcal{O}^h_{2+}$ |
| $(a,f,h):40$ | $R^{0z}_{TT'}$ | ${}^sR^{0x}_{TT}$ | ${}^cR^{0x}_{LT'}$ | ${}^sR^{0x}_{LT}$ | ${}^cR^{z'x}_{LT}$ | ${}^sR^{z'x}_{LT'}$ |
| | $\mathcal{O}^a_{2+}$ | $\mathcal{O}^a_{2-}$ | $\mathcal{O}^f_{1-}$ | $\mathcal{O}^f_{2-}$ | $\mathcal{O}^h_{1-}$ | $\mathcal{O}^h_{2-}$ |
| $(a,f,h):41$ | ${}^sR^{0z}_{TT}$ | $R^{0z}_{TT'}$ | ${}^sR^{0z}_{LT}$ | ${}^cR^{0x}_{LT'}$ | ${}^sR^{x'x}_{LT'}$ | ${}^cR^{z'x}_{LT}$ |
| | $\mathcal{O}^a_{1+}$ | $\mathcal{O}^a_{2+}$ | $\mathcal{O}^f_{1+}$ | $\mathcal{O}^f_{1-}$ | $\mathcal{O}^h_{1+}$ | $\mathcal{O}^h_{1-}$ |
| $(a,f,h):42$ | ${}^sR^{0z}_{TT}$ | $R^{0z}_{TT'}$ | ${}^sR^{0z}_{LT}$ | ${}^cR^{0x}_{LT'}$ | ${}^cR^{x'x}_{LT}$ | ${}^sR^{z'x}_{LT'}$ |
| | $\mathcal{O}^a_{1+}$ | $\mathcal{O}^a_{2+}$ | $\mathcal{O}^f_{1+}$ | $\mathcal{O}^f_{1-}$ | $\mathcal{O}^h_{2+}$ | $\mathcal{O}^h_{2-}$ |
| $(a,f,h):43$ | ${}^sR^{0z}_{TT}$ | $R^{0z}_{TT'}$ | ${}^sR^{0z}_{LT}$ | ${}^cR^{0x}_{LT'}$ | ${}^sR^{x'x}_{LT'}$ | ${}^cR^{x'x}_{LT}$ |
| | $\mathcal{O}^a_{1+}$ | $\mathcal{O}^a_{2+}$ | $\mathcal{O}^f_{1+}$ | $\mathcal{O}^f_{1-}$ | $\mathcal{O}^h_{1+}$ | $\mathcal{O}^h_{2+}$ |
| $(a,f,h):44$ | ${}^sR^{0z}_{TT}$ | $R^{0z}_{TT'}$ | ${}^sR^{0z}_{LT}$ | ${}^cR^{0x}_{LT'}$ | ${}^sR^{x'x}_{LT'}$ | ${}^sR^{z'x}_{LT'}$ |
| | $\mathcal{O}^a_{1+}$ | $\mathcal{O}^a_{2+}$ | $\mathcal{O}^f_{1+}$ | $\mathcal{O}^f_{1-}$ | $\mathcal{O}^h_{1+}$ | $\mathcal{O}^h_{2-}$ |
| $(a,f,h):45$ | ${}^sR^{0z}_{TT}$ | $R^{0z}_{TT'}$ | ${}^sR^{0z}_{LT}$ | ${}^cR^{0x}_{LT'}$ | ${}^cR^{z'x}_{LT}$ | ${}^cR^{x'x}_{LT}$ |
| | $\mathcal{O}^a_{1+}$ | $\mathcal{O}^a_{2+}$ | $\mathcal{O}^f_{1+}$ | $\mathcal{O}^f_{1-}$ | $\mathcal{O}^h_{1-}$ | $\mathcal{O}^h_{2+}$ |
| $(a,f,h):46$ | ${}^sR^{0z}_{TT}$ | $R^{0z}_{TT'}$ | ${}^sR^{0z}_{LT}$ | ${}^cR^{0x}_{LT'}$ | ${}^cR^{z'x}_{LT}$ | ${}^sR^{z'x}_{LT'}$ |
| | $\mathcal{O}^a_{1+}$ | $\mathcal{O}^a_{2+}$ | $\mathcal{O}^f_{1+}$ | $\mathcal{O}^f_{1-}$ | $\mathcal{O}^h_{1-}$ | $\mathcal{O}^h_{2-}$ |
| $(a,f,h):47$ | ${}^sR^{0z}_{TT}$ | $R^{0z}_{TT'}$ | ${}^cR^{0z}_{LT'}$ | ${}^sR^{0x}_{LT}$ | ${}^sR^{x'x}_{LT'}$ | ${}^cR^{z'x}_{LT}$ |
| | $\mathcal{O}^a_{1+}$ | $\mathcal{O}^a_{2+}$ | $\mathcal{O}^f_{2+}$ | $\mathcal{O}^f_{2-}$ | $\mathcal{O}^h_{1+}$ | $\mathcal{O}^h_{1-}$ |
| $(a,f,h):48$ | ${}^sR^{0z}_{TT}$ | $R^{0z}_{TT'}$ | ${}^cR^{0z}_{LT'}$ | ${}^sR^{0x}_{LT}$ | ${}^cR^{x'x}_{LT}$ | ${}^sR^{z'x}_{LT'}$ |
| | $\mathcal{O}^a_{1+}$ | $\mathcal{O}^a_{2+}$ | $\mathcal{O}^f_{2+}$ | $\mathcal{O}^f_{2-}$ | $\mathcal{O}^h_{2+}$ | $\mathcal{O}^h_{2-}$ |
| $(a,f,h):49$ | ${}^sR^{0z}_{TT}$ | $R^{0z}_{TT'}$ | ${}^cR^{0z}_{LT'}$ | ${}^sR^{0x}_{LT}$ | ${}^sR^{x'x}_{LT'}$ | ${}^cR^{x'x}_{LT}$ |
| | $\mathcal{O}^a_{1+}$ | $\mathcal{O}^a_{2+}$ | $\mathcal{O}^f_{2+}$ | $\mathcal{O}^f_{2-}$ | $\mathcal{O}^h_{1+}$ | $\mathcal{O}^h_{2+}$ |
| $(a,f,h):50$ | ${}^sR^{0z}_{TT}$ | $R^{0z}_{TT'}$ | ${}^cR^{0z}_{LT'}$ | ${}^sR^{0x}_{LT}$ | ${}^sR^{x'x}_{LT'}$ | ${}^sR^{z'x}_{LT'}$ |
| | $\mathcal{O}^a_{1+}$ | $\mathcal{O}^a_{2+}$ | $\mathcal{O}^f_{2+}$ | $\mathcal{O}^f_{2-}$ | $\mathcal{O}^h_{1+}$ | $\mathcal{O}^h_{2-}$ |
| $(a,f,h):51$ | ${}^sR^{0z}_{TT}$ | $R^{0z}_{TT'}$ | ${}^cR^{0z}_{LT'}$ | ${}^sR^{0x}_{LT}$ | ${}^cR^{z'x}_{LT}$ | ${}^cR^{x'x}_{LT}$ |
| | $\mathcal{O}^a_{1+}$ | $\mathcal{O}^a_{2+}$ | $\mathcal{O}^f_{2+}$ | $\mathcal{O}^f_{2-}$ | $\mathcal{O}^h_{1-}$ | $\mathcal{O}^h_{2+}$ |
| $(a,f,h):52$ | ${}^sR^{0z}_{TT}$ | $R^{0z}_{TT'}$ | ${}^cR^{0z}_{LT'}$ | ${}^sR^{0x}_{LT}$ | ${}^cR^{z'x}_{LT}$ | ${}^sR^{z'x}_{LT'}$ |
| | $\mathcal{O}^a_{1+}$ | $\mathcal{O}^a_{2+}$ | $\mathcal{O}^f_{2+}$ | $\mathcal{O}^f_{2-}$ | $\mathcal{O}^h_{1-}$ | $\mathcal{O}^h_{2-}$ |
| $(a,f,h):53$ | ${}^sR^{0z}_{TT}$ | $R^{0z}_{TT'}$ | ${}^sR^{0z}_{LT}$ | ${}^cR^{0z}_{LT'}$ | ${}^sR^{x'x}_{LT'}$ | ${}^cR^{z'x}_{LT}$ |
| | $\mathcal{O}^a_{1+}$ | $\mathcal{O}^a_{2+}$ | $\mathcal{O}^f_{1+}$ | $\mathcal{O}^f_{2+}$ | $\mathcal{O}^h_{1+}$ | $\mathcal{O}^h_{1-}$ |
| $(a,f,h):54$ | ${}^sR^{0z}_{TT}$ | $R^{0z}_{TT'}$ | ${}^sR^{0z}_{LT}$ | ${}^cR^{0z}_{LT'}$ | ${}^cR^{x'x}_{LT}$ | ${}^sR^{z'x}_{LT'}$ |
| | $\mathcal{O}^a_{1+}$ | $\mathcal{O}^a_{2+}$ | $\mathcal{O}^f_{1+}$ | $\mathcal{O}^f_{2+}$ | $\mathcal{O}^h_{2+}$ | $\mathcal{O}^h_{2-}$ |
| $(a,f,h):55$ | ${}^sR^{0z}_{TT}$ | $R^{0z}_{TT'}$ | ${}^sR^{0z}_{LT}$ | ${}^cR^{0z}_{LT'}$ | ${}^sR^{x'x}_{LT'}$ | ${}^cR^{x'x}_{LT}$ |
| | $\mathcal{O}^a_{1+}$ | $\mathcal{O}^a_{2+}$ | $\mathcal{O}^f_{1+}$ | $\mathcal{O}^f_{2+}$ | $\mathcal{O}^h_{1+}$ | $\mathcal{O}^h_{2+}$ |
| $(a,f,h):56$ | ${}^sR^{0z}_{TT}$ | $R^{0z}_{TT'}$ | ${}^sR^{0z}_{LT}$ | ${}^cR^{0z}_{LT'}$ | ${}^sR^{x'x}_{LT'}$ | ${}^sR^{z'x}_{LT'}$ |
| | $\mathcal{O}^a_{1+}$ | $\mathcal{O}^a_{2+}$ | $\mathcal{O}^f_{1+}$ | $\mathcal{O}^f_{2+}$ | $\mathcal{O}^h_{1+}$ | $\mathcal{O}^h_{2-}$ |
| $(a,f,h):57$ | ${}^sR^{0z}_{TT}$ | $R^{0z}_{TT'}$ | ${}^sR^{0z}_{LT}$ | ${}^cR^{0z}_{LT'}$ | ${}^cR^{z'x}_{LT}$ | ${}^cR^{x'x}_{LT}$ |
| | $\mathcal{O}^a_{1+}$ | $\mathcal{O}^a_{2+}$ | $\mathcal{O}^f_{1+}$ | $\mathcal{O}^f_{2+}$ | $\mathcal{O}^h_{1-}$ | $\mathcal{O}^h_{2+}$ |
| $(a,f,h):58$ | ${}^sR^{0z}_{TT}$ | $R^{0z}_{TT'}$ | ${}^sR^{0z}_{LT}$ | ${}^cR^{0z}_{LT'}$ | ${}^cR^{z'x}_{LT}$ | ${}^sR^{z'x}_{LT'}$ |
| | $\mathcal{O}^a_{1+}$ | $\mathcal{O}^a_{2+}$ | $\mathcal{O}^f_{1+}$ | $\mathcal{O}^f_{2+}$ | $\mathcal{O}^h_{1-}$ | $\mathcal{O}^h_{2-}$ |
| $(a,f,h):59$ | ${}^sR^{0z}_{TT}$ | $R^{0z}_{TT'}$ | ${}^sR^{0z}_{LT}$ | ${}^sR^{0x}_{LT}$ | ${}^sR^{x'x}_{LT'}$ | ${}^cR^{z'x}_{LT}$ |
| | $\mathcal{O}^a_{1+}$ | $\mathcal{O}^a_{2+}$ | $\mathcal{O}^f_{1+}$ | $\mathcal{O}^f_{2-}$ | $\mathcal{O}^h_{1+}$ | $\mathcal{O}^h_{1-}$ |
| $(a,f,h):60$ | ${}^sR^{0z}_{TT}$ | $R^{0z}_{TT'}$ | ${}^sR^{0z}_{LT}$ | ${}^sR^{0x}_{LT}$ | ${}^cR^{x'x}_{LT}$ | ${}^sR^{z'x}_{LT'}$ |
| | $\mathcal{O}^a_{1+}$ | $\mathcal{O}^a_{2+}$ | $\mathcal{O}^f_{1+}$ | $\mathcal{O}^f_{2-}$ | $\mathcal{O}^h_{2+}$ | $\mathcal{O}^h_{2-}$ |
| $(a,f,h):61$ | ${}^sR^{0z}_{TT}$ | $R^{0z}_{TT'}$ | ${}^sR^{0z}_{LT}$ | ${}^sR^{0x}_{LT}$ | ${}^sR^{x'x}_{LT'}$ | ${}^cR^{x'x}_{LT}$ |
| | $\mathcal{O}^a_{1+}$ | $\mathcal{O}^a_{2+}$ | $\mathcal{O}^f_{1+}$ | $\mathcal{O}^f_{2-}$ | $\mathcal{O}^h_{1+}$ | $\mathcal{O}^h_{2+}$ |
| $(a,f,h):62$ | ${}^sR^{0z}_{TT}$ | $R^{0z}_{TT'}$ | ${}^sR^{0z}_{LT}$ | ${}^sR^{0x}_{LT}$ | ${}^sR^{x'x}_{LT'}$ | ${}^sR^{z'x}_{LT'}$ |
| | $\mathcal{O}^a_{1+}$ | $\mathcal{O}^a_{2+}$ | $\mathcal{O}^f_{1+}$ | $\mathcal{O}^f_{2-}$ | $\mathcal{O}^h_{1+}$ | $\mathcal{O}^h_{2-}$ |
| $(a,f,h):63$ | ${}^sR^{0z}_{TT}$ | $R^{0z}_{TT'}$ | ${}^sR^{0z}_{LT}$ | ${}^sR^{0x}_{LT}$ | ${}^cR^{z'x}_{LT}$ | ${}^cR^{x'x}_{LT}$ |

| | | | | | | |
|---|---|---|---|---|---|---|
| | $\mathcal{O}^a_{1+}$ | $\mathcal{O}^a_{2+}$ | $\mathcal{O}^f_{1+}$ | $\mathcal{O}^f_{2-}$ | $\mathcal{O}^h_{1-}$ | $\mathcal{O}^h_{2+}$ |
| $(a, f, h) : 64$ | ${}^sR^{0z}_{TT}$ | $R^{0z}_{TT'}$ | ${}^sR^{0z}_{LT}$ | ${}^sR^{0x}_{LT}$ | ${}^cR^{z'x}_{LT}$ | ${}^sR^{z'x}_{LT'}$ |
| | $\mathcal{O}^a_{1+}$ | $\mathcal{O}^a_{2+}$ | $\mathcal{O}^f_{1+}$ | $\mathcal{O}^f_{2-}$ | $\mathcal{O}^h_{1-}$ | $\mathcal{O}^h_{2-}$ |
| $(a, f, h) : 65$ | ${}^sR^{0z}_{TT}$ | $R^{0z}_{TT'}$ | ${}^cR^{0x}_{LT'}$ | ${}^cR^{0z}_{LT'}$ | ${}^sR^{x'x}_{LT'}$ | ${}^cR^{z'x}_{LT}$ |
| | $\mathcal{O}^a_{1+}$ | $\mathcal{O}^a_{2+}$ | $\mathcal{O}^f_{1-}$ | $\mathcal{O}^f_{2+}$ | $\mathcal{O}^h_{1+}$ | $\mathcal{O}^h_{1-}$ |
| $(a, f, h) : 66$ | ${}^sR^{0z}_{TT}$ | $R^{0z}_{TT'}$ | ${}^cR^{0x}_{LT'}$ | ${}^cR^{0z}_{LT'}$ | ${}^cR^{x'x}_{LT}$ | ${}^sR^{z'x}_{LT'}$ |
| | $\mathcal{O}^a_{1+}$ | $\mathcal{O}^a_{2+}$ | $\mathcal{O}^f_{1-}$ | $\mathcal{O}^f_{2+}$ | $\mathcal{O}^h_{2+}$ | $\mathcal{O}^h_{2-}$ |
| $(a, f, h) : 67$ | ${}^sR^{0z}_{TT}$ | $R^{0z}_{TT'}$ | ${}^cR^{0x}_{LT'}$ | ${}^cR^{0z}_{LT'}$ | ${}^sR^{x'x}_{LT'}$ | ${}^cR^{x'x}_{LT}$ |
| | $\mathcal{O}^a_{1+}$ | $\mathcal{O}^a_{2+}$ | $\mathcal{O}^f_{1-}$ | $\mathcal{O}^f_{2+}$ | $\mathcal{O}^h_{1+}$ | $\mathcal{O}^h_{2+}$ |
| $(a, f, h) : 68$ | ${}^sR^{0z}_{TT}$ | $R^{0z}_{TT'}$ | ${}^cR^{0x}_{LT'}$ | ${}^cR^{0z}_{LT'}$ | ${}^sR^{x'x}_{LT'}$ | ${}^sR^{z'x}_{LT'}$ |
| | $\mathcal{O}^a_{1+}$ | $\mathcal{O}^a_{2+}$ | $\mathcal{O}^f_{1-}$ | $\mathcal{O}^f_{2+}$ | $\mathcal{O}^h_{1+}$ | $\mathcal{O}^h_{2-}$ |
| $(a, f, h) : 69$ | ${}^sR^{0z}_{TT}$ | $R^{0z}_{TT'}$ | ${}^cR^{0x}_{LT'}$ | ${}^cR^{0z}_{LT'}$ | ${}^cR^{z'x}_{LT}$ | ${}^cR^{x'x}_{LT}$ |
| | $\mathcal{O}^a_{1+}$ | $\mathcal{O}^a_{2+}$ | $\mathcal{O}^f_{1-}$ | $\mathcal{O}^f_{2+}$ | $\mathcal{O}^h_{1-}$ | $\mathcal{O}^h_{2+}$ |
| $(a, f, h) : 70$ | ${}^sR^{0z}_{TT}$ | $R^{0z}_{TT'}$ | ${}^cR^{0x}_{LT'}$ | ${}^cR^{0z}_{LT'}$ | ${}^cR^{z'x}_{LT}$ | ${}^sR^{z'x}_{LT'}$ |
| | $\mathcal{O}^a_{1+}$ | $\mathcal{O}^a_{2+}$ | $\mathcal{O}^f_{1-}$ | $\mathcal{O}^f_{2+}$ | $\mathcal{O}^h_{1-}$ | $\mathcal{O}^h_{2-}$ |
| $(a, f, h) : 71$ | ${}^sR^{0z}_{TT}$ | $R^{0z}_{TT'}$ | ${}^cR^{0x}_{LT'}$ | ${}^sR^{0x}_{LT}$ | ${}^sR^{x'x}_{LT'}$ | ${}^cR^{z'x}_{LT}$ |
| | $\mathcal{O}^a_{1+}$ | $\mathcal{O}^a_{2+}$ | $\mathcal{O}^f_{1-}$ | $\mathcal{O}^f_{2-}$ | $\mathcal{O}^h_{1+}$ | $\mathcal{O}^h_{1-}$ |
| $(a, f, h) : 72$ | ${}^sR^{0z}_{TT}$ | $R^{0z}_{TT'}$ | ${}^cR^{0x}_{LT'}$ | ${}^sR^{0x}_{LT}$ | ${}^cR^{x'x}_{LT}$ | ${}^sR^{z'x}_{LT'}$ |
| | $\mathcal{O}^a_{1+}$ | $\mathcal{O}^a_{2+}$ | $\mathcal{O}^f_{1-}$ | $\mathcal{O}^f_{2-}$ | $\mathcal{O}^h_{2+}$ | $\mathcal{O}^h_{2-}$ |
| $(a, f, h) : 73$ | ${}^sR^{0z}_{TT}$ | $R^{0z}_{TT'}$ | ${}^cR^{0x}_{LT'}$ | ${}^sR^{0x}_{LT}$ | ${}^sR^{x'x}_{LT'}$ | ${}^cR^{x'x}_{LT}$ |
| | $\mathcal{O}^a_{1+}$ | $\mathcal{O}^a_{2+}$ | $\mathcal{O}^f_{1-}$ | $\mathcal{O}^f_{2-}$ | $\mathcal{O}^h_{1+}$ | $\mathcal{O}^h_{2+}$ |
| $(a, f, h) : 74$ | ${}^sR^{0z}_{TT}$ | $R^{0z}_{TT'}$ | ${}^cR^{0x}_{LT'}$ | ${}^sR^{0x}_{LT}$ | ${}^sR^{x'x}_{LT'}$ | ${}^sR^{z'x}_{LT'}$ |
| | $\mathcal{O}^a_{1+}$ | $\mathcal{O}^a_{2+}$ | $\mathcal{O}^f_{1-}$ | $\mathcal{O}^f_{2-}$ | $\mathcal{O}^h_{1+}$ | $\mathcal{O}^h_{2-}$ |
| $(a, f, h) : 75$ | ${}^sR^{0z}_{TT}$ | $R^{0z}_{TT'}$ | ${}^cR^{0x}_{LT'}$ | ${}^sR^{0x}_{LT}$ | ${}^cR^{z'x}_{LT}$ | ${}^cR^{x'x}_{LT}$ |
| | $\mathcal{O}^a_{1+}$ | $\mathcal{O}^a_{2+}$ | $\mathcal{O}^f_{1-}$ | $\mathcal{O}^f_{2-}$ | $\mathcal{O}^h_{1-}$ | $\mathcal{O}^h_{2+}$ |
| $(a, f, h) : 76$ | ${}^sR^{0z}_{TT}$ | $R^{0z}_{TT'}$ | ${}^cR^{0x}_{LT'}$ | ${}^sR^{0x}_{LT}$ | ${}^cR^{z'x}_{LT}$ | ${}^sR^{z'x}_{LT'}$ |
| | $\mathcal{O}^a_{1+}$ | $\mathcal{O}^a_{2+}$ | $\mathcal{O}^f_{1-}$ | $\mathcal{O}^f_{2-}$ | $\mathcal{O}^h_{1-}$ | $\mathcal{O}^h_{2-}$ |
| $(a, f, h) : 77$ | ${}^sR^{0z}_{TT}$ | ${}^sR^{0x}_{TT}$ | ${}^sR^{0z}_{LT}$ | ${}^cR^{0x}_{LT'}$ | ${}^sR^{x'x}_{LT'}$ | ${}^cR^{x'x}_{LT}$ |
| | $\mathcal{O}^a_{1+}$ | $\mathcal{O}^a_{2-}$ | $\mathcal{O}^f_{1+}$ | $\mathcal{O}^f_{1-}$ | $\mathcal{O}^h_{1+}$ | $\mathcal{O}^h_{2+}$ |
| $(a, f, h) : 78$ | ${}^sR^{0z}_{TT}$ | ${}^sR^{0x}_{TT}$ | ${}^sR^{0z}_{LT}$ | ${}^cR^{0x}_{LT'}$ | ${}^cR^{z'x}_{LT}$ | ${}^sR^{z'x}_{LT'}$ |
| | $\mathcal{O}^a_{1+}$ | $\mathcal{O}^a_{2-}$ | $\mathcal{O}^f_{1+}$ | $\mathcal{O}^f_{1-}$ | $\mathcal{O}^h_{1-}$ | $\mathcal{O}^h_{2-}$ |
| $(a, f, h) : 79$ | ${}^sR^{0z}_{TT}$ | ${}^sR^{0x}_{TT}$ | ${}^cR^{0z}_{LT'}$ | ${}^sR^{0x}_{LT}$ | ${}^sR^{x'x}_{LT'}$ | ${}^cR^{x'x}_{LT}$ |
| | $\mathcal{O}^a_{1+}$ | $\mathcal{O}^a_{2-}$ | $\mathcal{O}^f_{2+}$ | $\mathcal{O}^f_{2-}$ | $\mathcal{O}^h_{1+}$ | $\mathcal{O}^h_{2+}$ |
| $(a, f, h) : 80$ | ${}^sR^{0z}_{TT}$ | ${}^sR^{0x}_{TT}$ | ${}^cR^{0z}_{LT'}$ | ${}^sR^{0x}_{LT}$ | ${}^cR^{z'x}_{LT}$ | ${}^sR^{z'x}_{LT'}$ |
| | $\mathcal{O}^a_{1+}$ | $\mathcal{O}^a_{2-}$ | $\mathcal{O}^f_{2+}$ | $\mathcal{O}^f_{2-}$ | $\mathcal{O}^h_{1-}$ | $\mathcal{O}^h_{2-}$ |
| $(a, f, h) : 81$ | ${}^sR^{0z}_{TT}$ | ${}^sR^{0x}_{TT}$ | ${}^sR^{0z}_{LT}$ | ${}^cR^{0z}_{LT'}$ | ${}^sR^{x'x}_{LT'}$ | ${}^cR^{z'x}_{LT}$ |
| | $\mathcal{O}^a_{1+}$ | $\mathcal{O}^a_{2-}$ | $\mathcal{O}^f_{1+}$ | $\mathcal{O}^f_{2+}$ | $\mathcal{O}^h_{1+}$ | $\mathcal{O}^h_{1-}$ |
| $(a, f, h) : 82$ | ${}^sR^{0z}_{TT}$ | ${}^sR^{0x}_{TT}$ | ${}^sR^{0z}_{LT}$ | ${}^cR^{0z}_{LT'}$ | ${}^cR^{x'x}_{LT}$ | ${}^sR^{z'x}_{LT'}$ |
| | $\mathcal{O}^a_{1+}$ | $\mathcal{O}^a_{2-}$ | $\mathcal{O}^f_{1+}$ | $\mathcal{O}^f_{2+}$ | $\mathcal{O}^h_{2+}$ | $\mathcal{O}^h_{2-}$ |
| $(a, f, h) : 83$ | ${}^sR^{0z}_{TT}$ | ${}^sR^{0x}_{TT}$ | ${}^sR^{0z}_{LT}$ | ${}^cR^{0z}_{LT'}$ | ${}^sR^{x'x}_{LT'}$ | ${}^cR^{x'x}_{LT}$ |
| | $\mathcal{O}^a_{1+}$ | $\mathcal{O}^a_{2-}$ | $\mathcal{O}^f_{1+}$ | $\mathcal{O}^f_{2+}$ | $\mathcal{O}^h_{1+}$ | $\mathcal{O}^h_{2+}$ |
| $(a, f, h) : 84$ | ${}^sR^{0z}_{TT}$ | ${}^sR^{0x}_{TT}$ | ${}^sR^{0z}_{LT}$ | ${}^cR^{0z}_{LT'}$ | ${}^sR^{x'x}_{LT'}$ | ${}^sR^{z'x}_{LT'}$ |
| | $\mathcal{O}^a_{1+}$ | $\mathcal{O}^a_{2-}$ | $\mathcal{O}^f_{1+}$ | $\mathcal{O}^f_{2+}$ | $\mathcal{O}^h_{1+}$ | $\mathcal{O}^h_{2-}$ |
| $(a, f, h) : 85$ | ${}^sR^{0z}_{TT}$ | ${}^sR^{0x}_{TT}$ | ${}^sR^{0z}_{LT}$ | ${}^cR^{0z}_{LT'}$ | ${}^cR^{z'x}_{LT}$ | ${}^cR^{x'x}_{LT}$ |
| | $\mathcal{O}^a_{1+}$ | $\mathcal{O}^a_{2-}$ | $\mathcal{O}^f_{1+}$ | $\mathcal{O}^f_{2+}$ | $\mathcal{O}^h_{1-}$ | $\mathcal{O}^h_{2+}$ |
| $(a, f, h) : 86$ | ${}^sR^{0z}_{TT}$ | ${}^sR^{0x}_{TT}$ | ${}^sR^{0z}_{LT}$ | ${}^cR^{0z}_{LT'}$ | ${}^cR^{z'x}_{LT}$ | ${}^sR^{z'x}_{LT'}$ |
| | $\mathcal{O}^a_{1+}$ | $\mathcal{O}^a_{2-}$ | $\mathcal{O}^f_{1+}$ | $\mathcal{O}^f_{2+}$ | $\mathcal{O}^h_{1-}$ | $\mathcal{O}^h_{2-}$ |
| $(a, f, h) : 87$ | ${}^sR^{0z}_{TT}$ | ${}^sR^{0x}_{TT}$ | ${}^sR^{0z}_{LT}$ | ${}^sR^{0x}_{LT}$ | ${}^sR^{x'x}_{LT'}$ | ${}^cR^{x'x}_{LT}$ |
| | $\mathcal{O}^a_{1+}$ | $\mathcal{O}^a_{2-}$ | $\mathcal{O}^f_{1+}$ | $\mathcal{O}^f_{2-}$ | $\mathcal{O}^h_{1+}$ | $\mathcal{O}^h_{2+}$ |
| $(a, f, h) : 88$ | ${}^sR^{0z}_{TT}$ | ${}^sR^{0x}_{TT}$ | ${}^sR^{0z}_{LT}$ | ${}^sR^{0x}_{LT}$ | ${}^cR^{z'x}_{LT}$ | ${}^sR^{z'x}_{LT'}$ |
| | $\mathcal{O}^a_{1+}$ | $\mathcal{O}^a_{2-}$ | $\mathcal{O}^f_{1+}$ | $\mathcal{O}^f_{2-}$ | $\mathcal{O}^h_{1-}$ | $\mathcal{O}^h_{2-}$ |
| $(a, f, h) : 89$ | ${}^sR^{0z}_{TT}$ | ${}^sR^{0x}_{TT}$ | ${}^cR^{0x}_{LT'}$ | ${}^cR^{0z}_{LT'}$ | ${}^sR^{x'x}_{LT'}$ | ${}^cR^{x'x}_{LT}$ |
| | $\mathcal{O}^a_{1+}$ | $\mathcal{O}^a_{2-}$ | $\mathcal{O}^f_{1-}$ | $\mathcal{O}^f_{2+}$ | $\mathcal{O}^h_{1+}$ | $\mathcal{O}^h_{2+}$ |
| $(a, f, h) : 90$ | ${}^sR^{0z}_{TT}$ | ${}^sR^{0x}_{TT}$ | ${}^cR^{0x}_{LT'}$ | ${}^cR^{0z}_{LT'}$ | ${}^cR^{z'x}_{LT}$ | ${}^sR^{z'x}_{LT'}$ |
| | $\mathcal{O}^a_{1+}$ | $\mathcal{O}^a_{2-}$ | $\mathcal{O}^f_{1-}$ | $\mathcal{O}^f_{2+}$ | $\mathcal{O}^h_{1-}$ | $\mathcal{O}^h_{2-}$ |

| | | | | | | |
|---|---|---|---|---|---|---|
| $(a,f,h):91$ | ${}^sR^{0z}_{TT}$ | ${}^sR^{0x}_{TT}$ | ${}^cR^{0x}_{LT'}$ | ${}^sR^{0x}_{LT}$ | ${}^sR^{x'x}_{LT'}$ | ${}^cR^{z'x}_{LT}$ |
| | $\mathcal{O}^a_{1+}$ | $\mathcal{O}^a_{2-}$ | $\mathcal{O}^f_{1-}$ | $\mathcal{O}^f_{2-}$ | $\mathcal{O}^h_{1+}$ | $\mathcal{O}^h_{1-}$ |
| $(a,f,h):92$ | ${}^sR^{0z}_{TT}$ | ${}^sR^{0x}_{TT}$ | ${}^cR^{0x}_{LT'}$ | ${}^sR^{0x}_{LT}$ | ${}^cR^{x'x}_{LT}$ | ${}^sR^{z'x}_{LT'}$ |
| | $\mathcal{O}^a_{1+}$ | $\mathcal{O}^a_{2-}$ | $\mathcal{O}^f_{1-}$ | $\mathcal{O}^f_{2-}$ | $\mathcal{O}^h_{2+}$ | $\mathcal{O}^h_{2-}$ |
| $(a,f,h):93$ | ${}^sR^{0z}_{TT}$ | ${}^sR^{0x}_{TT}$ | ${}^cR^{0x}_{LT'}$ | ${}^sR^{0x}_{LT}$ | ${}^sR^{x'x}_{LT'}$ | ${}^cR^{x'x}_{LT}$ |
| | $\mathcal{O}^a_{1+}$ | $\mathcal{O}^a_{2-}$ | $\mathcal{O}^f_{1-}$ | $\mathcal{O}^f_{2-}$ | $\mathcal{O}^h_{1+}$ | $\mathcal{O}^h_{2+}$ |
| $(a,f,h):94$ | ${}^sR^{0z}_{TT}$ | ${}^sR^{0x}_{TT}$ | ${}^cR^{0x}_{LT'}$ | ${}^sR^{0x}_{LT}$ | ${}^sR^{x'x}_{LT'}$ | ${}^sR^{z'x}_{LT'}$ |
| | $\mathcal{O}^a_{1+}$ | $\mathcal{O}^a_{2-}$ | $\mathcal{O}^f_{1-}$ | $\mathcal{O}^f_{2-}$ | $\mathcal{O}^h_{1+}$ | $\mathcal{O}^h_{2-}$ |
| $(a,f,h):95$ | ${}^sR^{0z}_{TT}$ | ${}^sR^{0x}_{TT}$ | ${}^cR^{0x}_{LT'}$ | ${}^sR^{0x}_{LT}$ | ${}^cR^{z'x}_{LT}$ | ${}^cR^{x'x}_{LT}$ |
| | $\mathcal{O}^a_{1+}$ | $\mathcal{O}^a_{2-}$ | $\mathcal{O}^f_{1-}$ | $\mathcal{O}^f_{2-}$ | $\mathcal{O}^h_{1-}$ | $\mathcal{O}^h_{2+}$ |
| $(a,f,h):96$ | ${}^sR^{0z}_{TT}$ | ${}^sR^{0x}_{TT}$ | ${}^cR^{0x}_{LT'}$ | ${}^sR^{0x}_{LT}$ | ${}^cR^{z'x}_{LT}$ | ${}^sR^{z'x}_{LT'}$ |
| | $\mathcal{O}^a_{1+}$ | $\mathcal{O}^a_{2-}$ | $\mathcal{O}^f_{1-}$ | $\mathcal{O}^f_{2-}$ | $\mathcal{O}^h_{1-}$ | $\mathcal{O}^h_{2-}$ |
| $(a,f,h):97$ | $R^{0x}_{TT'}$ | $R^{0z}_{TT'}$ | ${}^sR^{0z}_{LT}$ | ${}^cR^{0x}_{LT'}$ | ${}^sR^{x'x}_{LT'}$ | ${}^cR^{x'x}_{LT}$ |
| | $\mathcal{O}^a_{1-}$ | $\mathcal{O}^a_{2+}$ | $\mathcal{O}^f_{1+}$ | $\mathcal{O}^f_{1-}$ | $\mathcal{O}^h_{1+}$ | $\mathcal{O}^h_{2+}$ |
| $(a,f,h):98$ | $R^{0x}_{TT'}$ | $R^{0z}_{TT'}$ | ${}^sR^{0z}_{LT}$ | ${}^cR^{0x}_{LT'}$ | ${}^cR^{z'x}_{LT}$ | ${}^sR^{z'x}_{LT'}$ |
| | $\mathcal{O}^a_{1-}$ | $\mathcal{O}^a_{2+}$ | $\mathcal{O}^f_{1+}$ | $\mathcal{O}^f_{1-}$ | $\mathcal{O}^h_{1-}$ | $\mathcal{O}^h_{2-}$ |
| $(a,f,h):99$ | $R^{0x}_{TT'}$ | $R^{0z}_{TT'}$ | ${}^cR^{0z}_{LT'}$ | ${}^sR^{0x}_{LT}$ | ${}^sR^{x'x}_{LT'}$ | ${}^cR^{x'x}_{LT}$ |
| | $\mathcal{O}^a_{1-}$ | $\mathcal{O}^a_{2+}$ | $\mathcal{O}^f_{2+}$ | $\mathcal{O}^f_{2-}$ | $\mathcal{O}^h_{1+}$ | $\mathcal{O}^h_{2+}$ |
| $(a,f,h):100$ | $R^{0x}_{TT'}$ | $R^{0z}_{TT'}$ | ${}^cR^{0z}_{LT'}$ | ${}^sR^{0x}_{LT}$ | ${}^cR^{z'x}_{LT}$ | ${}^sR^{z'x}_{LT'}$ |
| | $\mathcal{O}^a_{1-}$ | $\mathcal{O}^a_{2+}$ | $\mathcal{O}^f_{2+}$ | $\mathcal{O}^f_{2-}$ | $\mathcal{O}^h_{1-}$ | $\mathcal{O}^h_{2-}$ |
| $(a,f,h):101$ | $R^{0x}_{TT'}$ | $R^{0z}_{TT'}$ | ${}^sR^{0z}_{LT}$ | ${}^cR^{0z}_{LT'}$ | ${}^sR^{x'x}_{LT'}$ | ${}^cR^{z'x}_{LT}$ |
| | $\mathcal{O}^a_{1-}$ | $\mathcal{O}^a_{2+}$ | $\mathcal{O}^f_{1+}$ | $\mathcal{O}^f_{2+}$ | $\mathcal{O}^h_{1+}$ | $\mathcal{O}^h_{1-}$ |
| $(a,f,h):102$ | $R^{0x}_{TT'}$ | $R^{0z}_{TT'}$ | ${}^sR^{0z}_{LT}$ | ${}^cR^{0z}_{LT'}$ | ${}^cR^{x'x}_{LT}$ | ${}^sR^{z'x}_{LT'}$ |
| | $\mathcal{O}^a_{1-}$ | $\mathcal{O}^a_{2+}$ | $\mathcal{O}^f_{1+}$ | $\mathcal{O}^f_{2+}$ | $\mathcal{O}^h_{2+}$ | $\mathcal{O}^h_{2-}$ |
| $(a,f,h):103$ | $R^{0x}_{TT'}$ | $R^{0z}_{TT'}$ | ${}^sR^{0z}_{LT}$ | ${}^cR^{0z}_{LT'}$ | ${}^sR^{x'x}_{LT'}$ | ${}^cR^{x'x}_{LT}$ |
| | $\mathcal{O}^a_{1-}$ | $\mathcal{O}^a_{2+}$ | $\mathcal{O}^f_{1+}$ | $\mathcal{O}^f_{2+}$ | $\mathcal{O}^h_{1+}$ | $\mathcal{O}^h_{2+}$ |
| $(a,f,h):104$ | $R^{0x}_{TT'}$ | $R^{0z}_{TT'}$ | ${}^sR^{0z}_{LT}$ | ${}^cR^{0z}_{LT'}$ | ${}^sR^{x'x}_{LT'}$ | ${}^sR^{z'x}_{LT'}$ |
| | $\mathcal{O}^a_{1-}$ | $\mathcal{O}^a_{2+}$ | $\mathcal{O}^f_{1+}$ | $\mathcal{O}^f_{2+}$ | $\mathcal{O}^h_{1+}$ | $\mathcal{O}^h_{2-}$ |
| $(a,f,h):105$ | $R^{0x}_{TT'}$ | $R^{0z}_{TT'}$ | ${}^sR^{0z}_{LT}$ | ${}^cR^{0z}_{LT'}$ | ${}^cR^{z'x}_{LT}$ | ${}^cR^{x'x}_{LT}$ |
| | $\mathcal{O}^a_{1-}$ | $\mathcal{O}^a_{2+}$ | $\mathcal{O}^f_{1+}$ | $\mathcal{O}^f_{2+}$ | $\mathcal{O}^h_{1-}$ | $\mathcal{O}^h_{2+}$ |
| $(a,f,h):106$ | $R^{0x}_{TT'}$ | $R^{0z}_{TT'}$ | ${}^sR^{0z}_{LT}$ | ${}^cR^{0z}_{LT'}$ | ${}^cR^{z'x}_{LT}$ | ${}^sR^{z'x}_{LT'}$ |
| | $\mathcal{O}^a_{1-}$ | $\mathcal{O}^a_{2+}$ | $\mathcal{O}^f_{1+}$ | $\mathcal{O}^f_{2+}$ | $\mathcal{O}^h_{1-}$ | $\mathcal{O}^h_{2-}$ |
| $(a,f,h):107$ | $R^{0x}_{TT'}$ | $R^{0z}_{TT'}$ | ${}^sR^{0z}_{LT}$ | ${}^sR^{0x}_{LT}$ | ${}^sR^{x'x}_{LT'}$ | ${}^cR^{x'x}_{LT}$ |
| | $\mathcal{O}^a_{1-}$ | $\mathcal{O}^a_{2+}$ | $\mathcal{O}^f_{1+}$ | $\mathcal{O}^f_{2-}$ | $\mathcal{O}^h_{1+}$ | $\mathcal{O}^h_{2+}$ |
| $(a,f,h):108$ | $R^{0x}_{TT'}$ | $R^{0z}_{TT'}$ | ${}^sR^{0z}_{LT}$ | ${}^sR^{0x}_{LT}$ | ${}^cR^{z'x}_{LT}$ | ${}^sR^{z'x}_{LT'}$ |
| | $\mathcal{O}^a_{1-}$ | $\mathcal{O}^a_{2+}$ | $\mathcal{O}^f_{1+}$ | $\mathcal{O}^f_{2-}$ | $\mathcal{O}^h_{1-}$ | $\mathcal{O}^h_{2-}$ |
| $(a,f,h):109$ | $R^{0x}_{TT'}$ | $R^{0z}_{TT'}$ | ${}^cR^{0x}_{LT'}$ | ${}^cR^{0z}_{LT'}$ | ${}^sR^{x'x}_{LT'}$ | ${}^cR^{x'x}_{LT}$ |
| | $\mathcal{O}^a_{1-}$ | $\mathcal{O}^a_{2+}$ | $\mathcal{O}^f_{1-}$ | $\mathcal{O}^f_{2+}$ | $\mathcal{O}^h_{1+}$ | $\mathcal{O}^h_{2+}$ |
| $(a,f,h):110$ | $R^{0x}_{TT'}$ | $R^{0z}_{TT'}$ | ${}^cR^{0x}_{LT'}$ | ${}^cR^{0z}_{LT'}$ | ${}^cR^{z'x}_{LT}$ | ${}^sR^{z'x}_{LT'}$ |
| | $\mathcal{O}^a_{1-}$ | $\mathcal{O}^a_{2+}$ | $\mathcal{O}^f_{1-}$ | $\mathcal{O}^f_{2+}$ | $\mathcal{O}^h_{1-}$ | $\mathcal{O}^h_{2-}$ |
| $(a,f,h):111$ | $R^{0x}_{TT'}$ | $R^{0z}_{TT'}$ | ${}^cR^{0x}_{LT'}$ | ${}^sR^{0x}_{LT}$ | ${}^sR^{x'x}_{LT'}$ | ${}^cR^{z'x}_{LT}$ |
| | $\mathcal{O}^a_{1-}$ | $\mathcal{O}^a_{2+}$ | $\mathcal{O}^f_{1-}$ | $\mathcal{O}^f_{2-}$ | $\mathcal{O}^h_{1+}$ | $\mathcal{O}^h_{1-}$ |
| $(a,f,h):112$ | $R^{0x}_{TT'}$ | $R^{0z}_{TT'}$ | ${}^cR^{0x}_{LT'}$ | ${}^sR^{0x}_{LT}$ | ${}^cR^{x'x}_{LT}$ | ${}^sR^{z'x}_{LT'}$ |
| | $\mathcal{O}^a_{1-}$ | $\mathcal{O}^a_{2+}$ | $\mathcal{O}^f_{1-}$ | $\mathcal{O}^f_{2-}$ | $\mathcal{O}^h_{2+}$ | $\mathcal{O}^h_{2-}$ |
| $(a,f,h):113$ | $R^{0x}_{TT'}$ | $R^{0z}_{TT'}$ | ${}^cR^{0x}_{LT'}$ | ${}^sR^{0x}_{LT}$ | ${}^sR^{x'x}_{LT'}$ | ${}^cR^{x'x}_{LT}$ |
| | $\mathcal{O}^a_{1-}$ | $\mathcal{O}^a_{2+}$ | $\mathcal{O}^f_{1-}$ | $\mathcal{O}^f_{2-}$ | $\mathcal{O}^h_{1+}$ | $\mathcal{O}^h_{2+}$ |
| $(a,f,h):114$ | $R^{0x}_{TT'}$ | $R^{0z}_{TT'}$ | ${}^cR^{0x}_{LT'}$ | ${}^sR^{0x}_{LT}$ | ${}^sR^{x'x}_{LT'}$ | ${}^sR^{z'x}_{LT'}$ |
| | $\mathcal{O}^a_{1-}$ | $\mathcal{O}^a_{2+}$ | $\mathcal{O}^f_{1-}$ | $\mathcal{O}^f_{2-}$ | $\mathcal{O}^h_{1+}$ | $\mathcal{O}^h_{2-}$ |
| $(a,f,h):115$ | $R^{0x}_{TT'}$ | $R^{0z}_{TT'}$ | ${}^cR^{0x}_{LT'}$ | ${}^sR^{0x}_{LT}$ | ${}^cR^{z'x}_{LT}$ | ${}^cR^{x'x}_{LT}$ |
| | $\mathcal{O}^a_{1-}$ | $\mathcal{O}^a_{2+}$ | $\mathcal{O}^f_{1-}$ | $\mathcal{O}^f_{2-}$ | $\mathcal{O}^h_{1-}$ | $\mathcal{O}^h_{2+}$ |
| $(a,f,h):116$ | $R^{0x}_{TT'}$ | $R^{0z}_{TT'}$ | ${}^cR^{0x}_{LT'}$ | ${}^sR^{0x}_{LT}$ | ${}^cR^{z'x}_{LT}$ | ${}^sR^{z'x}_{LT'}$ |
| | $\mathcal{O}^a_{1-}$ | $\mathcal{O}^a_{2+}$ | $\mathcal{O}^f_{1-}$ | $\mathcal{O}^f_{2-}$ | $\mathcal{O}^h_{1-}$ | $\mathcal{O}^h_{2-}$ |
| $(a,f,h):117$ | $R^{0x}_{TT'}$ | ${}^sR^{0x}_{TT}$ | ${}^sR^{0z}_{LT}$ | ${}^cR^{0x}_{LT'}$ | ${}^sR^{x'x}_{LT'}$ | ${}^cR^{z'x}_{LT}$ |
| | $\mathcal{O}^a_{1-}$ | $\mathcal{O}^a_{2-}$ | $\mathcal{O}^f_{1+}$ | $\mathcal{O}^f_{1-}$ | $\mathcal{O}^h_{1+}$ | $\mathcal{O}^h_{1-}$ |
| $(a,f,h):118$ | $R^{0x}_{TT'}$ | ${}^sR^{0x}_{TT}$ | ${}^sR^{0z}_{LT}$ | ${}^cR^{0x}_{LT'}$ | ${}^cR^{x'x}_{LT}$ | ${}^sR^{z'x}_{LT'}$ |

| | | | | | | |
|---|---|---|---|---|---|---|
| | $\mathcal{O}^{a}_{1-}$ | $\mathcal{O}^{a}_{2-}$ | $\mathcal{O}^{f}_{1+}$ | $\mathcal{O}^{f}_{1-}$ | $\mathcal{O}^{h}_{2+}$ | $\mathcal{O}^{h}_{2-}$ |
| $(a,f,h):119$ | $R^{0x}_{TT'}$ | ${}^{s}R^{0x}_{TT}$ | ${}^{s}R^{0z}_{LT}$ | ${}^{c}R^{0x}_{LT'}$ | ${}^{s}R^{x'x}_{LT'}$ | ${}^{c}R^{x'x}_{LT}$ |
| | $\mathcal{O}^{a}_{1-}$ | $\mathcal{O}^{a}_{2-}$ | $\mathcal{O}^{f}_{1+}$ | $\mathcal{O}^{f}_{1-}$ | $\mathcal{O}^{h}_{1+}$ | $\mathcal{O}^{h}_{2+}$ |
| $(a,f,h):120$ | $R^{0x}_{TT'}$ | ${}^{s}R^{0x}_{TT}$ | ${}^{s}R^{0z}_{LT}$ | ${}^{c}R^{0x}_{LT'}$ | ${}^{s}R^{x'x}_{LT'}$ | ${}^{s}R^{z'x}_{LT'}$ |
| | $\mathcal{O}^{a}_{1-}$ | $\mathcal{O}^{a}_{2-}$ | $\mathcal{O}^{f}_{1+}$ | $\mathcal{O}^{f}_{1-}$ | $\mathcal{O}^{h}_{1+}$ | $\mathcal{O}^{h}_{2-}$ |
| $(a,f,h):121$ | $R^{0x}_{TT'}$ | ${}^{s}R^{0x}_{TT}$ | ${}^{s}R^{0z}_{LT}$ | ${}^{c}R^{0x}_{LT'}$ | ${}^{c}R^{z'x}_{LT}$ | ${}^{c}R^{x'x}_{LT}$ |
| | $\mathcal{O}^{a}_{1-}$ | $\mathcal{O}^{a}_{2-}$ | $\mathcal{O}^{f}_{1+}$ | $\mathcal{O}^{f}_{1-}$ | $\mathcal{O}^{h}_{1-}$ | $\mathcal{O}^{h}_{2+}$ |
| $(a,f,h):122$ | $R^{0x}_{TT'}$ | ${}^{s}R^{0x}_{TT}$ | ${}^{s}R^{0z}_{LT}$ | ${}^{c}R^{0x}_{LT'}$ | ${}^{c}R^{z'x}_{LT}$ | ${}^{s}R^{z'x}_{LT'}$ |
| | $\mathcal{O}^{a}_{1-}$ | $\mathcal{O}^{a}_{2-}$ | $\mathcal{O}^{f}_{1+}$ | $\mathcal{O}^{f}_{1-}$ | $\mathcal{O}^{h}_{1-}$ | $\mathcal{O}^{h}_{2-}$ |
| $(a,f,h):123$ | $R^{0x}_{TT'}$ | ${}^{s}R^{0x}_{TT}$ | ${}^{c}R^{0z}_{LT'}$ | ${}^{s}R^{0x}_{LT}$ | ${}^{s}R^{x'x}_{LT'}$ | ${}^{c}R^{z'x}_{LT}$ |
| | $\mathcal{O}^{a}_{1-}$ | $\mathcal{O}^{a}_{2-}$ | $\mathcal{O}^{f}_{2+}$ | $\mathcal{O}^{f}_{2-}$ | $\mathcal{O}^{h}_{1+}$ | $\mathcal{O}^{h}_{1-}$ |
| $(a,f,h):124$ | $R^{0x}_{TT'}$ | ${}^{s}R^{0x}_{TT}$ | ${}^{c}R^{0z}_{LT'}$ | ${}^{s}R^{0x}_{LT}$ | ${}^{c}R^{x'x}_{LT}$ | ${}^{s}R^{z'x}_{LT'}$ |
| | $\mathcal{O}^{a}_{1-}$ | $\mathcal{O}^{a}_{2-}$ | $\mathcal{O}^{f}_{2+}$ | $\mathcal{O}^{f}_{2-}$ | $\mathcal{O}^{h}_{2+}$ | $\mathcal{O}^{h}_{2-}$ |
| $(a,f,h):125$ | $R^{0x}_{TT'}$ | ${}^{s}R^{0x}_{TT}$ | ${}^{c}R^{0z}_{LT'}$ | ${}^{s}R^{0x}_{LT}$ | ${}^{s}R^{x'x}_{LT'}$ | ${}^{c}R^{x'x}_{LT}$ |
| | $\mathcal{O}^{a}_{1-}$ | $\mathcal{O}^{a}_{2-}$ | $\mathcal{O}^{f}_{2+}$ | $\mathcal{O}^{f}_{2-}$ | $\mathcal{O}^{h}_{1+}$ | $\mathcal{O}^{h}_{2+}$ |
| $(a,f,h):126$ | $R^{0x}_{TT'}$ | ${}^{s}R^{0x}_{TT}$ | ${}^{c}R^{0z}_{LT'}$ | ${}^{s}R^{0x}_{LT}$ | ${}^{s}R^{x'x}_{LT'}$ | ${}^{s}R^{z'x}_{LT'}$ |
| | $\mathcal{O}^{a}_{1-}$ | $\mathcal{O}^{a}_{2-}$ | $\mathcal{O}^{f}_{2+}$ | $\mathcal{O}^{f}_{2-}$ | $\mathcal{O}^{h}_{1+}$ | $\mathcal{O}^{h}_{2-}$ |
| $(a,f,h):127$ | $R^{0x}_{TT'}$ | ${}^{s}R^{0x}_{TT}$ | ${}^{c}R^{0z}_{LT'}$ | ${}^{s}R^{0x}_{LT}$ | ${}^{c}R^{z'x}_{LT}$ | ${}^{c}R^{x'x}_{LT}$ |
| | $\mathcal{O}^{a}_{1-}$ | $\mathcal{O}^{a}_{2-}$ | $\mathcal{O}^{f}_{2+}$ | $\mathcal{O}^{f}_{2-}$ | $\mathcal{O}^{h}_{1-}$ | $\mathcal{O}^{h}_{2+}$ |
| $(a,f,h):128$ | $R^{0x}_{TT'}$ | ${}^{s}R^{0x}_{TT}$ | ${}^{c}R^{0z}_{LT'}$ | ${}^{s}R^{0x}_{LT}$ | ${}^{c}R^{z'x}_{LT}$ | ${}^{s}R^{z'x}_{LT'}$ |
| | $\mathcal{O}^{a}_{1-}$ | $\mathcal{O}^{a}_{2-}$ | $\mathcal{O}^{f}_{2+}$ | $\mathcal{O}^{f}_{2-}$ | $\mathcal{O}^{h}_{1-}$ | $\mathcal{O}^{h}_{2-}$ |
| $(a,f,h):129$ | $R^{0x}_{TT'}$ | ${}^{s}R^{0x}_{TT}$ | ${}^{s}R^{0z}_{LT}$ | ${}^{c}R^{0z}_{LT'}$ | ${}^{s}R^{x'x}_{LT'}$ | ${}^{c}R^{z'x}_{LT}$ |
| | $\mathcal{O}^{a}_{1-}$ | $\mathcal{O}^{a}_{2-}$ | $\mathcal{O}^{f}_{1+}$ | $\mathcal{O}^{f}_{2+}$ | $\mathcal{O}^{h}_{1+}$ | $\mathcal{O}^{h}_{1-}$ |
| $(a,f,h):130$ | $R^{0x}_{TT'}$ | ${}^{s}R^{0x}_{TT}$ | ${}^{s}R^{0z}_{LT}$ | ${}^{c}R^{0z}_{LT'}$ | ${}^{c}R^{x'x}_{LT}$ | ${}^{s}R^{z'x}_{LT'}$ |
| | $\mathcal{O}^{a}_{1-}$ | $\mathcal{O}^{a}_{2-}$ | $\mathcal{O}^{f}_{1+}$ | $\mathcal{O}^{f}_{2+}$ | $\mathcal{O}^{h}_{2+}$ | $\mathcal{O}^{h}_{2-}$ |
| $(a,f,h):131$ | $R^{0x}_{TT'}$ | ${}^{s}R^{0x}_{TT}$ | ${}^{s}R^{0z}_{LT}$ | ${}^{c}R^{0z}_{LT'}$ | ${}^{s}R^{x'x}_{LT'}$ | ${}^{c}R^{x'x}_{LT}$ |
| | $\mathcal{O}^{a}_{1-}$ | $\mathcal{O}^{a}_{2-}$ | $\mathcal{O}^{f}_{1+}$ | $\mathcal{O}^{f}_{2+}$ | $\mathcal{O}^{h}_{1+}$ | $\mathcal{O}^{h}_{2+}$ |
| $(a,f,h):132$ | $R^{0x}_{TT'}$ | ${}^{s}R^{0x}_{TT}$ | ${}^{s}R^{0z}_{LT}$ | ${}^{c}R^{0z}_{LT'}$ | ${}^{s}R^{x'x}_{LT'}$ | ${}^{s}R^{z'x}_{LT'}$ |
| | $\mathcal{O}^{a}_{1-}$ | $\mathcal{O}^{a}_{2-}$ | $\mathcal{O}^{f}_{1+}$ | $\mathcal{O}^{f}_{2+}$ | $\mathcal{O}^{h}_{1+}$ | $\mathcal{O}^{h}_{2-}$ |
| $(a,f,h):133$ | $R^{0x}_{TT'}$ | ${}^{s}R^{0x}_{TT}$ | ${}^{s}R^{0z}_{LT}$ | ${}^{c}R^{0z}_{LT'}$ | ${}^{c}R^{z'x}_{LT}$ | ${}^{c}R^{x'x}_{LT}$ |
| | $\mathcal{O}^{a}_{1-}$ | $\mathcal{O}^{a}_{2-}$ | $\mathcal{O}^{f}_{1+}$ | $\mathcal{O}^{f}_{2+}$ | $\mathcal{O}^{h}_{1-}$ | $\mathcal{O}^{h}_{2+}$ |
| $(a,f,h):134$ | $R^{0x}_{TT'}$ | ${}^{s}R^{0x}_{TT}$ | ${}^{s}R^{0z}_{LT}$ | ${}^{c}R^{0z}_{LT'}$ | ${}^{c}R^{z'x}_{LT}$ | ${}^{s}R^{z'x}_{LT'}$ |
| | $\mathcal{O}^{a}_{1-}$ | $\mathcal{O}^{a}_{2-}$ | $\mathcal{O}^{f}_{1+}$ | $\mathcal{O}^{f}_{2+}$ | $\mathcal{O}^{h}_{1-}$ | $\mathcal{O}^{h}_{2-}$ |
| $(a,f,h):135$ | $R^{0x}_{TT'}$ | ${}^{s}R^{0x}_{TT}$ | ${}^{s}R^{0z}_{LT}$ | ${}^{s}R^{0x}_{LT}$ | ${}^{s}R^{x'x}_{LT'}$ | ${}^{c}R^{z'x}_{LT}$ |
| | $\mathcal{O}^{a}_{1-}$ | $\mathcal{O}^{a}_{2-}$ | $\mathcal{O}^{f}_{1+}$ | $\mathcal{O}^{f}_{2-}$ | $\mathcal{O}^{h}_{1+}$ | $\mathcal{O}^{h}_{1-}$ |
| $(a,f,h):136$ | $R^{0x}_{TT'}$ | ${}^{s}R^{0x}_{TT}$ | ${}^{s}R^{0z}_{LT}$ | ${}^{s}R^{0x}_{LT}$ | ${}^{c}R^{x'x}_{LT}$ | ${}^{s}R^{z'x}_{LT'}$ |
| | $\mathcal{O}^{a}_{1-}$ | $\mathcal{O}^{a}_{2-}$ | $\mathcal{O}^{f}_{1+}$ | $\mathcal{O}^{f}_{2-}$ | $\mathcal{O}^{h}_{2+}$ | $\mathcal{O}^{h}_{2-}$ |
| $(a,f,h):137$ | $R^{0x}_{TT'}$ | ${}^{s}R^{0x}_{TT}$ | ${}^{s}R^{0z}_{LT}$ | ${}^{s}R^{0x}_{LT}$ | ${}^{s}R^{x'x}_{LT'}$ | ${}^{c}R^{x'x}_{LT}$ |
| | $\mathcal{O}^{a}_{1-}$ | $\mathcal{O}^{a}_{2-}$ | $\mathcal{O}^{f}_{1+}$ | $\mathcal{O}^{f}_{2-}$ | $\mathcal{O}^{h}_{1+}$ | $\mathcal{O}^{h}_{2+}$ |
| $(a,f,h):138$ | $R^{0x}_{TT'}$ | ${}^{s}R^{0x}_{TT}$ | ${}^{s}R^{0z}_{LT}$ | ${}^{s}R^{0x}_{LT}$ | ${}^{s}R^{x'x}_{LT'}$ | ${}^{s}R^{z'x}_{LT'}$ |
| | $\mathcal{O}^{a}_{1-}$ | $\mathcal{O}^{a}_{2-}$ | $\mathcal{O}^{f}_{1+}$ | $\mathcal{O}^{f}_{2-}$ | $\mathcal{O}^{h}_{1+}$ | $\mathcal{O}^{h}_{2-}$ |
| $(a,f,h):139$ | $R^{0x}_{TT'}$ | ${}^{s}R^{0x}_{TT}$ | ${}^{s}R^{0z}_{LT}$ | ${}^{s}R^{0x}_{LT}$ | ${}^{c}R^{z'x}_{LT}$ | ${}^{c}R^{x'x}_{LT}$ |
| | $\mathcal{O}^{a}_{1-}$ | $\mathcal{O}^{a}_{2-}$ | $\mathcal{O}^{f}_{1+}$ | $\mathcal{O}^{f}_{2-}$ | $\mathcal{O}^{h}_{1-}$ | $\mathcal{O}^{h}_{2+}$ |
| $(a,f,h):140$ | $R^{0x}_{TT'}$ | ${}^{s}R^{0x}_{TT}$ | ${}^{s}R^{0z}_{LT}$ | ${}^{s}R^{0x}_{LT}$ | ${}^{c}R^{z'x}_{LT}$ | ${}^{s}R^{z'x}_{LT'}$ |
| | $\mathcal{O}^{a}_{1-}$ | $\mathcal{O}^{a}_{2-}$ | $\mathcal{O}^{f}_{1+}$ | $\mathcal{O}^{f}_{2-}$ | $\mathcal{O}^{h}_{1-}$ | $\mathcal{O}^{h}_{2-}$ |
| $(a,f,h):141$ | $R^{0x}_{TT'}$ | ${}^{s}R^{0x}_{TT}$ | ${}^{c}R^{0x}_{LT'}$ | ${}^{c}R^{0z}_{LT'}$ | ${}^{s}R^{x'x}_{LT'}$ | ${}^{c}R^{z'x}_{LT}$ |
| | $\mathcal{O}^{a}_{1-}$ | $\mathcal{O}^{a}_{2-}$ | $\mathcal{O}^{f}_{1-}$ | $\mathcal{O}^{f}_{2+}$ | $\mathcal{O}^{h}_{1+}$ | $\mathcal{O}^{h}_{1-}$ |
| $(a,f,h):142$ | $R^{0x}_{TT'}$ | ${}^{s}R^{0x}_{TT}$ | ${}^{c}R^{0x}_{LT'}$ | ${}^{c}R^{0z}_{LT'}$ | ${}^{c}R^{x'x}_{LT}$ | ${}^{s}R^{z'x}_{LT'}$ |
| | $\mathcal{O}^{a}_{1-}$ | $\mathcal{O}^{a}_{2-}$ | $\mathcal{O}^{f}_{1-}$ | $\mathcal{O}^{f}_{2+}$ | $\mathcal{O}^{h}_{2+}$ | $\mathcal{O}^{h}_{2-}$ |
| $(a,f,h):143$ | $R^{0x}_{TT'}$ | ${}^{s}R^{0x}_{TT}$ | ${}^{c}R^{0x}_{LT'}$ | ${}^{c}R^{0z}_{LT'}$ | ${}^{s}R^{x'x}_{LT'}$ | ${}^{c}R^{x'x}_{LT}$ |
| | $\mathcal{O}^{a}_{1-}$ | $\mathcal{O}^{a}_{2-}$ | $\mathcal{O}^{f}_{1-}$ | $\mathcal{O}^{f}_{2+}$ | $\mathcal{O}^{h}_{1+}$ | $\mathcal{O}^{h}_{2+}$ |
| $(a,f,h):144$ | $R^{0x}_{TT'}$ | ${}^{s}R^{0x}_{TT}$ | ${}^{c}R^{0x}_{LT'}$ | ${}^{c}R^{0z}_{LT'}$ | ${}^{s}R^{x'x}_{LT'}$ | ${}^{s}R^{z'x}_{LT'}$ |
| | $\mathcal{O}^{a}_{1-}$ | $\mathcal{O}^{a}_{2-}$ | $\mathcal{O}^{f}_{1-}$ | $\mathcal{O}^{f}_{2+}$ | $\mathcal{O}^{h}_{1+}$ | $\mathcal{O}^{h}_{2-}$ |
| $(a,f,h):145$ | $R^{0x}_{TT'}$ | ${}^{s}R^{0x}_{TT}$ | ${}^{c}R^{0x}_{LT'}$ | ${}^{c}R^{0z}_{LT'}$ | ${}^{c}R^{z'x}_{LT}$ | ${}^{c}R^{x'x}_{LT}$ |
| | $\mathcal{O}^{a}_{1-}$ | $\mathcal{O}^{a}_{2-}$ | $\mathcal{O}^{f}_{1-}$ | $\mathcal{O}^{f}_{2+}$ | $\mathcal{O}^{h}_{1-}$ | $\mathcal{O}^{h}_{2+}$ |

| | | | | | | |
|---|---|---|---|---|---|---|
| $(a,f,h):146$ | $R^{0x}_{TT'}$ | ${}^{s}R^{0x}_{TT}$ | ${}^{c}R^{0x}_{LT'}$ | ${}^{c}R^{0z}_{LT'}$ | ${}^{c}R^{z'x}_{LT}$ | ${}^{s}R^{z'x}_{LT'}$ |
| | $\mathcal{O}^{a}_{1-}$ | $\mathcal{O}^{a}_{2-}$ | $\mathcal{O}^{f}_{1-}$ | $\mathcal{O}^{f}_{2+}$ | $\mathcal{O}^{h}_{1-}$ | $\mathcal{O}^{h}_{2-}$ |
| $(a,f,h):147$ | $R^{0x}_{TT'}$ | ${}^{s}R^{0x}_{TT}$ | ${}^{c}R^{0x}_{LT'}$ | ${}^{s}R^{0x}_{LT}$ | ${}^{s}R^{x'x}_{LT'}$ | ${}^{c}R^{z'x}_{LT}$ |
| | $\mathcal{O}^{a}_{1-}$ | $\mathcal{O}^{a}_{2-}$ | $\mathcal{O}^{f}_{1-}$ | $\mathcal{O}^{f}_{2-}$ | $\mathcal{O}^{h}_{1+}$ | $\mathcal{O}^{h}_{1-}$ |
| $(a,f,h):148$ | $R^{0x}_{TT'}$ | ${}^{s}R^{0x}_{TT}$ | ${}^{c}R^{0x}_{LT'}$ | ${}^{s}R^{0x}_{LT}$ | ${}^{c}R^{x'x}_{LT}$ | ${}^{s}R^{z'x}_{LT'}$ |
| | $\mathcal{O}^{a}_{1-}$ | $\mathcal{O}^{a}_{2-}$ | $\mathcal{O}^{f}_{1-}$ | $\mathcal{O}^{f}_{2-}$ | $\mathcal{O}^{h}_{2+}$ | $\mathcal{O}^{h}_{2-}$ |
| $(a,f,h):149$ | $R^{0x}_{TT'}$ | ${}^{s}R^{0x}_{TT}$ | ${}^{c}R^{0x}_{LT'}$ | ${}^{s}R^{0x}_{LT}$ | ${}^{s}R^{x'x}_{LT'}$ | ${}^{c}R^{x'x}_{LT}$ |
| | $\mathcal{O}^{a}_{1-}$ | $\mathcal{O}^{a}_{2-}$ | $\mathcal{O}^{f}_{1-}$ | $\mathcal{O}^{f}_{2-}$ | $\mathcal{O}^{h}_{1+}$ | $\mathcal{O}^{h}_{2+}$ |
| $(a,f,h):150$ | $R^{0x}_{TT'}$ | ${}^{s}R^{0x}_{TT}$ | ${}^{c}R^{0x}_{LT'}$ | ${}^{s}R^{0x}_{LT}$ | ${}^{s}R^{x'x}_{LT'}$ | ${}^{s}R^{z'x}_{LT'}$ |
| | $\mathcal{O}^{a}_{1-}$ | $\mathcal{O}^{a}_{2-}$ | $\mathcal{O}^{f}_{1-}$ | $\mathcal{O}^{f}_{2-}$ | $\mathcal{O}^{h}_{1+}$ | $\mathcal{O}^{h}_{2-}$ |
| $(a,f,h):151$ | $R^{0x}_{TT'}$ | ${}^{s}R^{0x}_{TT}$ | ${}^{c}R^{0x}_{LT'}$ | ${}^{s}R^{0x}_{LT}$ | ${}^{c}R^{z'x}_{LT}$ | ${}^{c}R^{x'x}_{LT}$ |
| | $\mathcal{O}^{a}_{1-}$ | $\mathcal{O}^{a}_{2-}$ | $\mathcal{O}^{f}_{1-}$ | $\mathcal{O}^{f}_{2-}$ | $\mathcal{O}^{h}_{1-}$ | $\mathcal{O}^{h}_{2+}$ |
| $(a,f,h):152$ | $R^{0x}_{TT'}$ | ${}^{s}R^{0x}_{TT}$ | ${}^{c}R^{0x}_{LT'}$ | ${}^{s}R^{0x}_{LT}$ | ${}^{c}R^{z'x}_{LT}$ | ${}^{s}R^{z'x}_{LT'}$ |
| | $\mathcal{O}^{a}_{1-}$ | $\mathcal{O}^{a}_{2-}$ | $\mathcal{O}^{f}_{1-}$ | $\mathcal{O}^{f}_{2-}$ | $\mathcal{O}^{h}_{1-}$ | $\mathcal{O}^{h}_{2-}$ |

TABLE VI: All the fully complete sets determined from the combination of shape-classes $(b,e,f)$ (i.e. graph-topology 'III') in the case of pseudoscalar meson electroproduction are listed here. The observables are written in the systematic symbolic notation $\mathcal{O}^{n}_{\nu\pm}$ by Nakayama [1], as well as in the more commonly used notation in terms of 'response-functions' $R^{\beta\alpha}_{i}$ (cf. references [4, 5]). The given sets of 6 observables have to be combined with the 6 'diagonal' observables $\left\{R^{00}_{T}, {}^{c}R^{00}_{TT}, R^{0y}_{T}, R^{y'0}_{T}, R^{00}_{L}, R^{0y}_{L}\right\}$ in order to form a complete set of minimal length $2N = 12$. All of these sets have been verified to be complete using Mathematica [3].

| Set-Nr. | Observables | | | | | |
|---|---|---|---|---|---|---|
| $(b,e,f):1$ | ${}^{s}R^{z'0}_{TT}$ | $R^{x'0}_{TT'}$ | ${}^{s}R^{00}_{LT'}$ | ${}^{s}R^{0y}_{LT'}$ | ${}^{s}R^{0z}_{LT}$ | ${}^{c}R^{0z}_{LT'}$ |
| | $\mathcal{O}^{b}_{1+}$ | $\mathcal{O}^{b}_{1-}$ | $\mathcal{O}^{e}_{1+}$ | $\mathcal{O}^{e}_{1-}$ | $\mathcal{O}^{f}_{1+}$ | $\mathcal{O}^{f}_{2+}$ |
| $(b,e,f):2$ | ${}^{s}R^{z'0}_{TT}$ | $R^{x'0}_{TT'}$ | ${}^{s}R^{00}_{LT'}$ | ${}^{s}R^{0y}_{LT'}$ | ${}^{c}R^{0x}_{LT'}$ | ${}^{s}R^{0x}_{LT}$ |
| | $\mathcal{O}^{b}_{1+}$ | $\mathcal{O}^{b}_{1-}$ | $\mathcal{O}^{e}_{1+}$ | $\mathcal{O}^{e}_{1-}$ | $\mathcal{O}^{f}_{1-}$ | $\mathcal{O}^{f}_{2-}$ |
| $(b,e,f):3$ | ${}^{s}R^{z'0}_{TT}$ | $R^{x'0}_{TT'}$ | ${}^{c}R^{00}_{LT}$ | ${}^{c}R^{0y}_{LT}$ | ${}^{s}R^{0z}_{LT}$ | ${}^{c}R^{0z}_{LT'}$ |
| | $\mathcal{O}^{b}_{1+}$ | $\mathcal{O}^{b}_{1-}$ | $\mathcal{O}^{e}_{2+}$ | $\mathcal{O}^{e}_{2-}$ | $\mathcal{O}^{f}_{1+}$ | $\mathcal{O}^{f}_{2+}$ |
| $(b,e,f):4$ | ${}^{s}R^{z'0}_{TT}$ | $R^{x'0}_{TT'}$ | ${}^{c}R^{00}_{LT}$ | ${}^{c}R^{0y}_{LT}$ | ${}^{c}R^{0x}_{LT'}$ | ${}^{s}R^{0x}_{LT}$ |
| | $\mathcal{O}^{b}_{1+}$ | $\mathcal{O}^{b}_{1-}$ | $\mathcal{O}^{e}_{2+}$ | $\mathcal{O}^{e}_{2-}$ | $\mathcal{O}^{f}_{1-}$ | $\mathcal{O}^{f}_{2-}$ |
| $(b,e,f):5$ | ${}^{s}R^{z'0}_{TT}$ | $R^{x'0}_{TT'}$ | ${}^{s}R^{00}_{LT'}$ | ${}^{c}R^{00}_{LT}$ | ${}^{s}R^{0z}_{LT}$ | ${}^{c}R^{0x}_{LT'}$ |
| | $\mathcal{O}^{b}_{1+}$ | $\mathcal{O}^{b}_{1-}$ | $\mathcal{O}^{e}_{1+}$ | $\mathcal{O}^{e}_{2+}$ | $\mathcal{O}^{f}_{1+}$ | $\mathcal{O}^{f}_{1-}$ |
| $(b,e,f):6$ | ${}^{s}R^{z'0}_{TT}$ | $R^{x'0}_{TT'}$ | ${}^{s}R^{00}_{LT'}$ | ${}^{c}R^{00}_{LT}$ | ${}^{c}R^{0z}_{LT'}$ | ${}^{s}R^{0x}_{LT}$ |
| | $\mathcal{O}^{b}_{1+}$ | $\mathcal{O}^{b}_{1-}$ | $\mathcal{O}^{e}_{1+}$ | $\mathcal{O}^{e}_{2+}$ | $\mathcal{O}^{f}_{2+}$ | $\mathcal{O}^{f}_{2-}$ |
| $(b,e,f):7$ | ${}^{s}R^{z'0}_{TT}$ | $R^{x'0}_{TT'}$ | ${}^{s}R^{00}_{LT'}$ | ${}^{c}R^{00}_{LT}$ | ${}^{s}R^{0z}_{LT}$ | ${}^{c}R^{0z}_{LT'}$ |
| | $\mathcal{O}^{b}_{1+}$ | $\mathcal{O}^{b}_{1-}$ | $\mathcal{O}^{e}_{1+}$ | $\mathcal{O}^{e}_{2+}$ | $\mathcal{O}^{f}_{1+}$ | $\mathcal{O}^{f}_{2+}$ |
| $(b,e,f):8$ | ${}^{s}R^{z'0}_{TT}$ | $R^{x'0}_{TT'}$ | ${}^{s}R^{00}_{LT'}$ | ${}^{c}R^{00}_{LT}$ | ${}^{s}R^{0z}_{LT}$ | ${}^{s}R^{0x}_{LT}$ |
| | $\mathcal{O}^{b}_{1+}$ | $\mathcal{O}^{b}_{1-}$ | $\mathcal{O}^{e}_{1+}$ | $\mathcal{O}^{e}_{2+}$ | $\mathcal{O}^{f}_{1+}$ | $\mathcal{O}^{f}_{2-}$ |
| $(b,e,f):9$ | ${}^{s}R^{z'0}_{TT}$ | $R^{x'0}_{TT'}$ | ${}^{s}R^{00}_{LT'}$ | ${}^{c}R^{00}_{LT}$ | ${}^{c}R^{0x}_{LT'}$ | ${}^{c}R^{0z}_{LT'}$ |
| | $\mathcal{O}^{b}_{1+}$ | $\mathcal{O}^{b}_{1-}$ | $\mathcal{O}^{e}_{1+}$ | $\mathcal{O}^{e}_{2+}$ | $\mathcal{O}^{f}_{1-}$ | $\mathcal{O}^{f}_{2+}$ |
| $(b,e,f):10$ | ${}^{s}R^{z'0}_{TT}$ | $R^{x'0}_{TT'}$ | ${}^{s}R^{00}_{LT'}$ | ${}^{c}R^{00}_{LT}$ | ${}^{c}R^{0x}_{LT'}$ | ${}^{s}R^{0x}_{LT}$ |
| | $\mathcal{O}^{b}_{1+}$ | $\mathcal{O}^{b}_{1-}$ | $\mathcal{O}^{e}_{1+}$ | $\mathcal{O}^{e}_{2+}$ | $\mathcal{O}^{f}_{1-}$ | $\mathcal{O}^{f}_{2-}$ |
| $(b,e,f):11$ | ${}^{s}R^{z'0}_{TT}$ | $R^{x'0}_{TT'}$ | ${}^{s}R^{00}_{LT'}$ | ${}^{c}R^{0y}_{LT}$ | ${}^{s}R^{0z}_{LT}$ | ${}^{c}R^{0z}_{LT'}$ |
| | $\mathcal{O}^{b}_{1+}$ | $\mathcal{O}^{b}_{1-}$ | $\mathcal{O}^{e}_{1+}$ | $\mathcal{O}^{e}_{2-}$ | $\mathcal{O}^{f}_{1+}$ | $\mathcal{O}^{f}_{2+}$ |
| $(b,e,f):12$ | ${}^{s}R^{z'0}_{TT}$ | $R^{x'0}_{TT'}$ | ${}^{s}R^{00}_{LT'}$ | ${}^{c}R^{0y}_{LT}$ | ${}^{c}R^{0x}_{LT'}$ | ${}^{s}R^{0x}_{LT}$ |
| | $\mathcal{O}^{b}_{1+}$ | $\mathcal{O}^{b}_{1-}$ | $\mathcal{O}^{e}_{1+}$ | $\mathcal{O}^{e}_{2-}$ | $\mathcal{O}^{f}_{1-}$ | $\mathcal{O}^{f}_{2-}$ |
| $(b,e,f):13$ | ${}^{s}R^{z'0}_{TT}$ | $R^{x'0}_{TT'}$ | ${}^{s}R^{0y}_{LT'}$ | ${}^{c}R^{00}_{LT}$ | ${}^{s}R^{0z}_{LT}$ | ${}^{c}R^{0z}_{LT'}$ |
| | $\mathcal{O}^{b}_{1+}$ | $\mathcal{O}^{b}_{1-}$ | $\mathcal{O}^{e}_{1-}$ | $\mathcal{O}^{e}_{2+}$ | $\mathcal{O}^{f}_{1+}$ | $\mathcal{O}^{f}_{2+}$ |
| $(b,e,f):14$ | ${}^{s}R^{z'0}_{TT}$ | $R^{x'0}_{TT'}$ | ${}^{s}R^{0y}_{LT'}$ | ${}^{c}R^{00}_{LT}$ | ${}^{c}R^{0x}_{LT'}$ | ${}^{s}R^{0x}_{LT}$ |

| | | | | | | |
|---|---|---|---|---|---|---|
| | $\mathcal{O}^b_{1+}$ | $\mathcal{O}^b_{1-}$ | $\mathcal{O}^e_{1-}$ | $\mathcal{O}^e_{2+}$ | $\mathcal{O}^f_{1-}$ | $\mathcal{O}^f_{2-}$ |
| $(b,e,f):15$ | ${}^{s}R^{z'0}_{TT}$ | $R^{x'0}_{TT'}$ | ${}^{s}R^{0y}_{LT'}$ | ${}^{c}R^{0y}_{LT}$ | ${}^{s}R^{0z}_{LT}$ | ${}^{c}R^{0x}_{LT'}$ |
| | $\mathcal{O}^b_{1+}$ | $\mathcal{O}^b_{1-}$ | $\mathcal{O}^e_{1-}$ | $\mathcal{O}^e_{2-}$ | $\mathcal{O}^f_{1+}$ | $\mathcal{O}^f_{1-}$ |
| $(b,e,f):16$ | ${}^{s}R^{z'0}_{TT}$ | $R^{x'0}_{TT'}$ | ${}^{s}R^{0y}_{LT'}$ | ${}^{c}R^{0y}_{LT}$ | ${}^{c}R^{0z}_{LT'}$ | ${}^{s}R^{0x}_{LT}$ |
| | $\mathcal{O}^b_{1+}$ | $\mathcal{O}^b_{1-}$ | $\mathcal{O}^e_{1-}$ | $\mathcal{O}^e_{2-}$ | $\mathcal{O}^f_{2+}$ | $\mathcal{O}^f_{2-}$ |
| $(b,e,f):17$ | ${}^{s}R^{z'0}_{TT}$ | $R^{x'0}_{TT'}$ | ${}^{s}R^{0y}_{LT'}$ | ${}^{c}R^{0y}_{LT}$ | ${}^{s}R^{0z}_{LT}$ | ${}^{c}R^{0z}_{LT'}$ |
| | $\mathcal{O}^b_{1+}$ | $\mathcal{O}^b_{1-}$ | $\mathcal{O}^e_{1-}$ | $\mathcal{O}^e_{2-}$ | $\mathcal{O}^f_{1+}$ | $\mathcal{O}^f_{2+}$ |
| $(b,e,f):18$ | ${}^{s}R^{z'0}_{TT}$ | $R^{x'0}_{TT'}$ | ${}^{s}R^{0y}_{LT'}$ | ${}^{c}R^{0y}_{LT}$ | ${}^{s}R^{0z}_{LT}$ | ${}^{s}R^{0x}_{LT}$ |
| | $\mathcal{O}^b_{1+}$ | $\mathcal{O}^b_{1-}$ | $\mathcal{O}^e_{1-}$ | $\mathcal{O}^e_{2-}$ | $\mathcal{O}^f_{1+}$ | $\mathcal{O}^f_{2-}$ |
| $(b,e,f):19$ | ${}^{s}R^{z'0}_{TT}$ | $R^{x'0}_{TT'}$ | ${}^{s}R^{0y}_{LT'}$ | ${}^{c}R^{0y}_{LT}$ | ${}^{c}R^{0x}_{LT'}$ | ${}^{c}R^{0z}_{LT'}$ |
| | $\mathcal{O}^b_{1+}$ | $\mathcal{O}^b_{1-}$ | $\mathcal{O}^e_{1-}$ | $\mathcal{O}^e_{2-}$ | $\mathcal{O}^f_{1-}$ | $\mathcal{O}^f_{2+}$ |
| $(b,e,f):20$ | ${}^{s}R^{z'0}_{TT}$ | $R^{x'0}_{TT'}$ | ${}^{s}R^{0y}_{LT'}$ | ${}^{c}R^{0y}_{LT}$ | ${}^{c}R^{0x}_{LT'}$ | ${}^{s}R^{0x}_{LT}$ |
| | $\mathcal{O}^b_{1+}$ | $\mathcal{O}^b_{1-}$ | $\mathcal{O}^e_{1-}$ | $\mathcal{O}^e_{2-}$ | $\mathcal{O}^f_{1-}$ | $\mathcal{O}^f_{2-}$ |
| $(b,e,f):21$ | $R^{z'0}_{TT'}$ | ${}^{s}R^{x'0}_{TT}$ | ${}^{s}R^{00}_{LT'}$ | ${}^{s}R^{0y}_{LT'}$ | ${}^{s}R^{0z}_{LT}$ | ${}^{c}R^{0z}_{LT'}$ |
| | $\mathcal{O}^b_{2+}$ | $\mathcal{O}^b_{2-}$ | $\mathcal{O}^e_{1+}$ | $\mathcal{O}^e_{1-}$ | $\mathcal{O}^f_{1+}$ | $\mathcal{O}^f_{2+}$ |
| $(b,e,f):22$ | $R^{z'0}_{TT'}$ | ${}^{s}R^{x'0}_{TT}$ | ${}^{s}R^{00}_{LT'}$ | ${}^{s}R^{0y}_{LT'}$ | ${}^{c}R^{0x}_{LT'}$ | ${}^{s}R^{0x}_{LT}$ |
| | $\mathcal{O}^b_{2+}$ | $\mathcal{O}^b_{2-}$ | $\mathcal{O}^e_{1+}$ | $\mathcal{O}^e_{1-}$ | $\mathcal{O}^f_{1-}$ | $\mathcal{O}^f_{2-}$ |
| $(b,e,f):23$ | $R^{z'0}_{TT'}$ | ${}^{s}R^{x'0}_{TT}$ | ${}^{c}R^{00}_{LT}$ | ${}^{c}R^{0y}_{LT}$ | ${}^{s}R^{0z}_{LT}$ | ${}^{c}R^{0z}_{LT'}$ |
| | $\mathcal{O}^b_{2+}$ | $\mathcal{O}^b_{2-}$ | $\mathcal{O}^e_{2+}$ | $\mathcal{O}^e_{2-}$ | $\mathcal{O}^f_{1+}$ | $\mathcal{O}^f_{2+}$ |
| $(b,e,f):24$ | $R^{z'0}_{TT'}$ | ${}^{s}R^{x'0}_{TT}$ | ${}^{c}R^{00}_{LT}$ | ${}^{c}R^{0y}_{LT}$ | ${}^{c}R^{0x}_{LT'}$ | ${}^{s}R^{0x}_{LT}$ |
| | $\mathcal{O}^b_{2+}$ | $\mathcal{O}^b_{2-}$ | $\mathcal{O}^e_{2+}$ | $\mathcal{O}^e_{2-}$ | $\mathcal{O}^f_{1-}$ | $\mathcal{O}^f_{2-}$ |
| $(b,e,f):25$ | $R^{z'0}_{TT'}$ | ${}^{s}R^{x'0}_{TT}$ | ${}^{s}R^{00}_{LT'}$ | ${}^{c}R^{00}_{LT}$ | ${}^{s}R^{0z}_{LT}$ | ${}^{c}R^{0x}_{LT'}$ |
| | $\mathcal{O}^b_{2+}$ | $\mathcal{O}^b_{2-}$ | $\mathcal{O}^e_{1+}$ | $\mathcal{O}^e_{2+}$ | $\mathcal{O}^f_{1+}$ | $\mathcal{O}^f_{1-}$ |
| $(b,e,f):26$ | $R^{z'0}_{TT'}$ | ${}^{s}R^{x'0}_{TT}$ | ${}^{s}R^{00}_{LT'}$ | ${}^{c}R^{00}_{LT}$ | ${}^{c}R^{0z}_{LT'}$ | ${}^{s}R^{0x}_{LT}$ |
| | $\mathcal{O}^b_{2+}$ | $\mathcal{O}^b_{2-}$ | $\mathcal{O}^e_{1+}$ | $\mathcal{O}^e_{2+}$ | $\mathcal{O}^f_{2+}$ | $\mathcal{O}^f_{2-}$ |
| $(b,e,f):27$ | $R^{z'0}_{TT'}$ | ${}^{s}R^{x'0}_{TT}$ | ${}^{s}R^{00}_{LT'}$ | ${}^{c}R^{00}_{LT}$ | ${}^{s}R^{0z}_{LT}$ | ${}^{c}R^{0z}_{LT'}$ |
| | $\mathcal{O}^b_{2+}$ | $\mathcal{O}^b_{2-}$ | $\mathcal{O}^e_{1+}$ | $\mathcal{O}^e_{2+}$ | $\mathcal{O}^f_{1+}$ | $\mathcal{O}^f_{2+}$ |
| $(b,e,f):28$ | $R^{z'0}_{TT'}$ | ${}^{s}R^{x'0}_{TT}$ | ${}^{s}R^{00}_{LT'}$ | ${}^{c}R^{00}_{LT}$ | ${}^{s}R^{0z}_{LT}$ | ${}^{s}R^{0x}_{LT}$ |
| | $\mathcal{O}^b_{2+}$ | $\mathcal{O}^b_{2-}$ | $\mathcal{O}^e_{1+}$ | $\mathcal{O}^e_{2+}$ | $\mathcal{O}^f_{1+}$ | $\mathcal{O}^f_{2-}$ |
| $(b,e,f):29$ | $R^{z'0}_{TT'}$ | ${}^{s}R^{x'0}_{TT}$ | ${}^{s}R^{00}_{LT'}$ | ${}^{c}R^{00}_{LT}$ | ${}^{c}R^{0x}_{LT'}$ | ${}^{c}R^{0z}_{LT'}$ |
| | $\mathcal{O}^b_{2+}$ | $\mathcal{O}^b_{2-}$ | $\mathcal{O}^e_{1+}$ | $\mathcal{O}^e_{2+}$ | $\mathcal{O}^f_{1-}$ | $\mathcal{O}^f_{2+}$ |
| $(b,e,f):30$ | $R^{z'0}_{TT'}$ | ${}^{s}R^{x'0}_{TT}$ | ${}^{s}R^{00}_{LT'}$ | ${}^{c}R^{00}_{LT}$ | ${}^{c}R^{0x}_{LT'}$ | ${}^{s}R^{0x}_{LT}$ |
| | $\mathcal{O}^b_{2+}$ | $\mathcal{O}^b_{2-}$ | $\mathcal{O}^e_{1+}$ | $\mathcal{O}^e_{2+}$ | $\mathcal{O}^f_{1-}$ | $\mathcal{O}^f_{2-}$ |
| $(b,e,f):31$ | $R^{z'0}_{TT'}$ | ${}^{s}R^{x'0}_{TT}$ | ${}^{s}R^{00}_{LT'}$ | ${}^{c}R^{0y}_{LT}$ | ${}^{s}R^{0z}_{LT}$ | ${}^{c}R^{0z}_{LT'}$ |
| | $\mathcal{O}^b_{2+}$ | $\mathcal{O}^b_{2-}$ | $\mathcal{O}^e_{1+}$ | $\mathcal{O}^e_{2-}$ | $\mathcal{O}^f_{1+}$ | $\mathcal{O}^f_{2+}$ |
| $(b,e,f):32$ | $R^{z'0}_{TT'}$ | ${}^{s}R^{x'0}_{TT}$ | ${}^{s}R^{00}_{LT'}$ | ${}^{c}R^{0y}_{LT}$ | ${}^{c}R^{0x}_{LT'}$ | ${}^{s}R^{0x}_{LT}$ |
| | $\mathcal{O}^b_{2+}$ | $\mathcal{O}^b_{2-}$ | $\mathcal{O}^e_{1+}$ | $\mathcal{O}^e_{2-}$ | $\mathcal{O}^f_{1-}$ | $\mathcal{O}^f_{2-}$ |
| $(b,e,f):33$ | $R^{z'0}_{TT'}$ | ${}^{s}R^{x'0}_{TT}$ | ${}^{s}R^{0y}_{LT'}$ | ${}^{c}R^{00}_{LT}$ | ${}^{s}R^{0z}_{LT}$ | ${}^{c}R^{0z}_{LT'}$ |
| | $\mathcal{O}^b_{2+}$ | $\mathcal{O}^b_{2-}$ | $\mathcal{O}^e_{1-}$ | $\mathcal{O}^e_{2+}$ | $\mathcal{O}^f_{1+}$ | $\mathcal{O}^f_{2+}$ |
| $(b,e,f):34$ | $R^{z'0}_{TT'}$ | ${}^{s}R^{x'0}_{TT}$ | ${}^{s}R^{0y}_{LT'}$ | ${}^{c}R^{00}_{LT}$ | ${}^{c}R^{0x}_{LT'}$ | ${}^{s}R^{0x}_{LT}$ |
| | $\mathcal{O}^b_{2+}$ | $\mathcal{O}^b_{2-}$ | $\mathcal{O}^e_{1-}$ | $\mathcal{O}^e_{2+}$ | $\mathcal{O}^f_{1-}$ | $\mathcal{O}^f_{2-}$ |
| $(b,e,f):35$ | $R^{z'0}_{TT'}$ | ${}^{s}R^{x'0}_{TT}$ | ${}^{s}R^{0y}_{LT'}$ | ${}^{c}R^{0y}_{LT}$ | ${}^{s}R^{0z}_{LT}$ | ${}^{c}R^{0x}_{LT'}$ |
| | $\mathcal{O}^b_{2+}$ | $\mathcal{O}^b_{2-}$ | $\mathcal{O}^e_{1-}$ | $\mathcal{O}^e_{2-}$ | $\mathcal{O}^f_{1+}$ | $\mathcal{O}^f_{1-}$ |
| $(b,e,f):36$ | $R^{z'0}_{TT'}$ | ${}^{s}R^{x'0}_{TT}$ | ${}^{s}R^{0y}_{LT'}$ | ${}^{c}R^{0y}_{LT}$ | ${}^{c}R^{0z}_{LT'}$ | ${}^{s}R^{0x}_{LT}$ |
| | $\mathcal{O}^b_{2+}$ | $\mathcal{O}^b_{2-}$ | $\mathcal{O}^e_{1-}$ | $\mathcal{O}^e_{2-}$ | $\mathcal{O}^f_{2+}$ | $\mathcal{O}^f_{2-}$ |
| $(b,e,f):37$ | $R^{z'0}_{TT'}$ | ${}^{s}R^{x'0}_{TT}$ | ${}^{s}R^{0y}_{LT'}$ | ${}^{c}R^{0y}_{LT}$ | ${}^{s}R^{0z}_{LT}$ | ${}^{c}R^{0z}_{LT'}$ |
| | $\mathcal{O}^b_{2+}$ | $\mathcal{O}^b_{2-}$ | $\mathcal{O}^e_{1-}$ | $\mathcal{O}^e_{2-}$ | $\mathcal{O}^f_{1+}$ | $\mathcal{O}^f_{2+}$ |
| $(b,e,f):38$ | $R^{z'0}_{TT'}$ | ${}^{s}R^{x'0}_{TT}$ | ${}^{s}R^{0y}_{LT'}$ | ${}^{c}R^{0y}_{LT}$ | ${}^{s}R^{0z}_{LT}$ | ${}^{s}R^{0x}_{LT}$ |
| | $\mathcal{O}^b_{2+}$ | $\mathcal{O}^b_{2-}$ | $\mathcal{O}^e_{1-}$ | $\mathcal{O}^e_{2-}$ | $\mathcal{O}^f_{1+}$ | $\mathcal{O}^f_{2-}$ |
| $(b,e,f):39$ | $R^{z'0}_{TT'}$ | ${}^{s}R^{x'0}_{TT}$ | ${}^{s}R^{0y}_{LT'}$ | ${}^{c}R^{0y}_{LT}$ | ${}^{c}R^{0x}_{LT'}$ | ${}^{c}R^{0z}_{LT'}$ |
| | $\mathcal{O}^b_{2+}$ | $\mathcal{O}^b_{2-}$ | $\mathcal{O}^e_{1-}$ | $\mathcal{O}^e_{2-}$ | $\mathcal{O}^f_{1-}$ | $\mathcal{O}^f_{2+}$ |
| $(b,e,f):40$ | $R^{z'0}_{TT'}$ | ${}^{s}R^{x'0}_{TT}$ | ${}^{s}R^{0y}_{LT'}$ | ${}^{c}R^{0y}_{LT}$ | ${}^{c}R^{0x}_{LT'}$ | ${}^{s}R^{0x}_{LT}$ |
| | $\mathcal{O}^b_{2+}$ | $\mathcal{O}^b_{2-}$ | $\mathcal{O}^e_{1-}$ | $\mathcal{O}^e_{2-}$ | $\mathcal{O}^f_{1-}$ | $\mathcal{O}^f_{2-}$ |
| $(b,e,f):41$ | ${}^{s}R^{z'0}_{TT}$ | $R^{z'0}_{TT'}$ | ${}^{s}R^{00}_{LT'}$ | ${}^{s}R^{0y}_{LT'}$ | ${}^{s}R^{0z}_{LT}$ | ${}^{c}R^{0x}_{LT'}$ |
| | $\mathcal{O}^b_{1+}$ | $\mathcal{O}^b_{2+}$ | $\mathcal{O}^e_{1+}$ | $\mathcal{O}^e_{1-}$ | $\mathcal{O}^f_{1+}$ | $\mathcal{O}^f_{1-}$ |

| | | | | | | |
|---|---|---|---|---|---|---|
| $(b,e,f):42$ | ${}^sR^{z'0}_{TT}$ | $R^{z'0}_{TT'}$ | ${}^sR^{00}_{LT'}$ | ${}^sR^{0y}_{LT'}$ | ${}^cR^{0z}_{LT'}$ | ${}^sR^{0x}_{LT}$ |
| | $\mathcal{O}^b_{1+}$ | $\mathcal{O}^b_{2+}$ | $\mathcal{O}^e_{1+}$ | $\mathcal{O}^e_{1-}$ | $\mathcal{O}^f_{2+}$ | $\mathcal{O}^f_{2-}$ |
| $(b,e,f):43$ | ${}^sR^{z'0}_{TT}$ | $R^{z'0}_{TT'}$ | ${}^sR^{00}_{LT'}$ | ${}^sR^{0y}_{LT'}$ | ${}^sR^{0z}_{LT}$ | ${}^cR^{0z}_{LT'}$ |
| | $\mathcal{O}^b_{1+}$ | $\mathcal{O}^b_{2+}$ | $\mathcal{O}^e_{1+}$ | $\mathcal{O}^e_{1-}$ | $\mathcal{O}^f_{1+}$ | $\mathcal{O}^f_{2+}$ |
| $(b,e,f):44$ | ${}^sR^{z'0}_{TT}$ | $R^{z'0}_{TT'}$ | ${}^sR^{00}_{LT'}$ | ${}^sR^{0y}_{LT'}$ | ${}^sR^{0z}_{LT}$ | ${}^sR^{0x}_{LT}$ |
| | $\mathcal{O}^b_{1+}$ | $\mathcal{O}^b_{2+}$ | $\mathcal{O}^e_{1+}$ | $\mathcal{O}^e_{1-}$ | $\mathcal{O}^f_{1+}$ | $\mathcal{O}^f_{2-}$ |
| $(b,e,f):45$ | ${}^sR^{z'0}_{TT}$ | $R^{z'0}_{TT'}$ | ${}^sR^{00}_{LT'}$ | ${}^sR^{0y}_{LT'}$ | ${}^cR^{0x}_{LT'}$ | ${}^cR^{0z}_{LT'}$ |
| | $\mathcal{O}^b_{1+}$ | $\mathcal{O}^b_{2+}$ | $\mathcal{O}^e_{1+}$ | $\mathcal{O}^e_{1-}$ | $\mathcal{O}^f_{1-}$ | $\mathcal{O}^f_{2+}$ |
| $(b,e,f):46$ | ${}^sR^{z'0}_{TT}$ | $R^{z'0}_{TT'}$ | ${}^sR^{00}_{LT'}$ | ${}^sR^{0y}_{LT'}$ | ${}^cR^{0x}_{LT'}$ | ${}^sR^{0x}_{LT}$ |
| | $\mathcal{O}^b_{1+}$ | $\mathcal{O}^b_{2+}$ | $\mathcal{O}^e_{1+}$ | $\mathcal{O}^e_{1-}$ | $\mathcal{O}^f_{1-}$ | $\mathcal{O}^f_{2-}$ |
| $(b,e,f):47$ | ${}^sR^{z'0}_{TT}$ | $R^{z'0}_{TT'}$ | ${}^cR^{00}_{LT}$ | ${}^cR^{0y}_{LT}$ | ${}^sR^{0z}_{LT}$ | ${}^cR^{0x}_{LT'}$ |
| | $\mathcal{O}^b_{1+}$ | $\mathcal{O}^b_{2+}$ | $\mathcal{O}^e_{2+}$ | $\mathcal{O}^e_{2-}$ | $\mathcal{O}^f_{1+}$ | $\mathcal{O}^f_{1-}$ |
| $(b,e,f):48$ | ${}^sR^{z'0}_{TT}$ | $R^{z'0}_{TT'}$ | ${}^cR^{00}_{LT}$ | ${}^cR^{0y}_{LT}$ | ${}^cR^{0z}_{LT'}$ | ${}^sR^{0x}_{LT}$ |
| | $\mathcal{O}^b_{1+}$ | $\mathcal{O}^b_{2+}$ | $\mathcal{O}^e_{2+}$ | $\mathcal{O}^e_{2-}$ | $\mathcal{O}^f_{2+}$ | $\mathcal{O}^f_{2-}$ |
| $(b,e,f):49$ | ${}^sR^{z'0}_{TT}$ | $R^{z'0}_{TT'}$ | ${}^cR^{00}_{LT}$ | ${}^cR^{0y}_{LT}$ | ${}^sR^{0z}_{LT}$ | ${}^cR^{0z}_{LT'}$ |
| | $\mathcal{O}^b_{1+}$ | $\mathcal{O}^b_{2+}$ | $\mathcal{O}^e_{2+}$ | $\mathcal{O}^e_{2-}$ | $\mathcal{O}^f_{1+}$ | $\mathcal{O}^f_{2+}$ |
| $(b,e,f):50$ | ${}^sR^{z'0}_{TT}$ | $R^{z'0}_{TT'}$ | ${}^cR^{00}_{LT}$ | ${}^cR^{0y}_{LT}$ | ${}^sR^{0z}_{LT}$ | ${}^sR^{0x}_{LT}$ |
| | $\mathcal{O}^b_{1+}$ | $\mathcal{O}^b_{2+}$ | $\mathcal{O}^e_{2+}$ | $\mathcal{O}^e_{2-}$ | $\mathcal{O}^f_{1+}$ | $\mathcal{O}^f_{2-}$ |
| $(b,e,f):51$ | ${}^sR^{z'0}_{TT}$ | $R^{z'0}_{TT'}$ | ${}^cR^{00}_{LT}$ | ${}^cR^{0y}_{LT}$ | ${}^cR^{0x}_{LT'}$ | ${}^cR^{0z}_{LT'}$ |
| | $\mathcal{O}^b_{1+}$ | $\mathcal{O}^b_{2+}$ | $\mathcal{O}^e_{2+}$ | $\mathcal{O}^e_{2-}$ | $\mathcal{O}^f_{1-}$ | $\mathcal{O}^f_{2+}$ |
| $(b,e,f):52$ | ${}^sR^{z'0}_{TT}$ | $R^{z'0}_{TT'}$ | ${}^cR^{00}_{LT}$ | ${}^cR^{0y}_{LT}$ | ${}^cR^{0x}_{LT'}$ | ${}^sR^{0x}_{LT}$ |
| | $\mathcal{O}^b_{1+}$ | $\mathcal{O}^b_{2+}$ | $\mathcal{O}^e_{2+}$ | $\mathcal{O}^e_{2-}$ | $\mathcal{O}^f_{1-}$ | $\mathcal{O}^f_{2-}$ |
| $(b,e,f):53$ | ${}^sR^{z'0}_{TT}$ | $R^{z'0}_{TT'}$ | ${}^sR^{00}_{LT'}$ | ${}^cR^{00}_{LT}$ | ${}^sR^{0z}_{LT}$ | ${}^cR^{0x}_{LT'}$ |
| | $\mathcal{O}^b_{1+}$ | $\mathcal{O}^b_{2+}$ | $\mathcal{O}^e_{1+}$ | $\mathcal{O}^e_{2+}$ | $\mathcal{O}^f_{1+}$ | $\mathcal{O}^f_{1-}$ |
| $(b,e,f):54$ | ${}^sR^{z'0}_{TT}$ | $R^{z'0}_{TT'}$ | ${}^sR^{00}_{LT'}$ | ${}^cR^{00}_{LT}$ | ${}^cR^{0z}_{LT'}$ | ${}^sR^{0x}_{LT}$ |
| | $\mathcal{O}^b_{1+}$ | $\mathcal{O}^b_{2+}$ | $\mathcal{O}^e_{1+}$ | $\mathcal{O}^e_{2+}$ | $\mathcal{O}^f_{2+}$ | $\mathcal{O}^f_{2-}$ |
| $(b,e,f):55$ | ${}^sR^{z'0}_{TT}$ | $R^{z'0}_{TT'}$ | ${}^sR^{00}_{LT'}$ | ${}^cR^{00}_{LT}$ | ${}^sR^{0z}_{LT}$ | ${}^cR^{0z}_{LT'}$ |
| | $\mathcal{O}^b_{1+}$ | $\mathcal{O}^b_{2+}$ | $\mathcal{O}^e_{1+}$ | $\mathcal{O}^e_{2+}$ | $\mathcal{O}^f_{1+}$ | $\mathcal{O}^f_{2+}$ |
| $(b,e,f):56$ | ${}^sR^{z'0}_{TT}$ | $R^{z'0}_{TT'}$ | ${}^sR^{00}_{LT'}$ | ${}^cR^{00}_{LT}$ | ${}^sR^{0z}_{LT}$ | ${}^sR^{0x}_{LT}$ |
| | $\mathcal{O}^b_{1+}$ | $\mathcal{O}^b_{2+}$ | $\mathcal{O}^e_{1+}$ | $\mathcal{O}^e_{2+}$ | $\mathcal{O}^f_{1+}$ | $\mathcal{O}^f_{2-}$ |
| $(b,e,f):57$ | ${}^sR^{z'0}_{TT}$ | $R^{z'0}_{TT'}$ | ${}^sR^{00}_{LT'}$ | ${}^cR^{00}_{LT}$ | ${}^cR^{0x}_{LT'}$ | ${}^cR^{0z}_{LT'}$ |
| | $\mathcal{O}^b_{1+}$ | $\mathcal{O}^b_{2+}$ | $\mathcal{O}^e_{1+}$ | $\mathcal{O}^e_{2+}$ | $\mathcal{O}^f_{1-}$ | $\mathcal{O}^f_{2+}$ |
| $(b,e,f):58$ | ${}^sR^{z'0}_{TT}$ | $R^{z'0}_{TT'}$ | ${}^sR^{00}_{LT'}$ | ${}^cR^{00}_{LT}$ | ${}^cR^{0x}_{LT'}$ | ${}^sR^{0x}_{LT}$ |
| | $\mathcal{O}^b_{1+}$ | $\mathcal{O}^b_{2+}$ | $\mathcal{O}^e_{1+}$ | $\mathcal{O}^e_{2+}$ | $\mathcal{O}^f_{1-}$ | $\mathcal{O}^f_{2-}$ |
| $(b,e,f):59$ | ${}^sR^{z'0}_{TT}$ | $R^{z'0}_{TT'}$ | ${}^sR^{00}_{LT'}$ | ${}^cR^{0y}_{LT}$ | ${}^sR^{0z}_{LT}$ | ${}^cR^{0x}_{LT'}$ |
| | $\mathcal{O}^b_{1+}$ | $\mathcal{O}^b_{2+}$ | $\mathcal{O}^e_{1+}$ | $\mathcal{O}^e_{2-}$ | $\mathcal{O}^f_{1+}$ | $\mathcal{O}^f_{1-}$ |
| $(b,e,f):60$ | ${}^sR^{z'0}_{TT}$ | $R^{z'0}_{TT'}$ | ${}^sR^{00}_{LT'}$ | ${}^cR^{0y}_{LT}$ | ${}^cR^{0z}_{LT'}$ | ${}^sR^{0x}_{LT}$ |
| | $\mathcal{O}^b_{1+}$ | $\mathcal{O}^b_{2+}$ | $\mathcal{O}^e_{1+}$ | $\mathcal{O}^e_{2-}$ | $\mathcal{O}^f_{2+}$ | $\mathcal{O}^f_{2-}$ |
| $(b,e,f):61$ | ${}^sR^{z'0}_{TT}$ | $R^{z'0}_{TT'}$ | ${}^sR^{00}_{LT'}$ | ${}^cR^{0y}_{LT}$ | ${}^sR^{0z}_{LT}$ | ${}^cR^{0z}_{LT'}$ |
| | $\mathcal{O}^b_{1+}$ | $\mathcal{O}^b_{2+}$ | $\mathcal{O}^e_{1+}$ | $\mathcal{O}^e_{2-}$ | $\mathcal{O}^f_{1+}$ | $\mathcal{O}^f_{2+}$ |
| $(b,e,f):62$ | ${}^sR^{z'0}_{TT}$ | $R^{z'0}_{TT'}$ | ${}^sR^{00}_{LT'}$ | ${}^cR^{0y}_{LT}$ | ${}^sR^{0z}_{LT}$ | ${}^sR^{0x}_{LT}$ |
| | $\mathcal{O}^b_{1+}$ | $\mathcal{O}^b_{2+}$ | $\mathcal{O}^e_{1+}$ | $\mathcal{O}^e_{2-}$ | $\mathcal{O}^f_{1+}$ | $\mathcal{O}^f_{2-}$ |
| $(b,e,f):63$ | ${}^sR^{z'0}_{TT}$ | $R^{z'0}_{TT'}$ | ${}^sR^{00}_{LT'}$ | ${}^cR^{0y}_{LT}$ | ${}^cR^{0x}_{LT'}$ | ${}^cR^{0z}_{LT'}$ |
| | $\mathcal{O}^b_{1+}$ | $\mathcal{O}^b_{2+}$ | $\mathcal{O}^e_{1+}$ | $\mathcal{O}^e_{2-}$ | $\mathcal{O}^f_{1-}$ | $\mathcal{O}^f_{2+}$ |
| $(b,e,f):64$ | ${}^sR^{z'0}_{TT}$ | $R^{z'0}_{TT'}$ | ${}^sR^{00}_{LT'}$ | ${}^cR^{0y}_{LT}$ | ${}^cR^{0x}_{LT'}$ | ${}^sR^{0x}_{LT}$ |
| | $\mathcal{O}^b_{1+}$ | $\mathcal{O}^b_{2+}$ | $\mathcal{O}^e_{1+}$ | $\mathcal{O}^e_{2-}$ | $\mathcal{O}^f_{1-}$ | $\mathcal{O}^f_{2-}$ |
| $(b,e,f):65$ | ${}^sR^{z'0}_{TT}$ | $R^{z'0}_{TT'}$ | ${}^sR^{0y}_{LT'}$ | ${}^cR^{00}_{LT}$ | ${}^sR^{0z}_{LT}$ | ${}^cR^{0x}_{LT'}$ |
| | $\mathcal{O}^b_{1+}$ | $\mathcal{O}^b_{2+}$ | $\mathcal{O}^e_{1-}$ | $\mathcal{O}^e_{2+}$ | $\mathcal{O}^f_{1+}$ | $\mathcal{O}^f_{1-}$ |
| $(b,e,f):66$ | ${}^sR^{z'0}_{TT}$ | $R^{z'0}_{TT'}$ | ${}^sR^{0y}_{LT'}$ | ${}^cR^{00}_{LT}$ | ${}^cR^{0z}_{LT'}$ | ${}^sR^{0x}_{LT}$ |
| | $\mathcal{O}^b_{1+}$ | $\mathcal{O}^b_{2+}$ | $\mathcal{O}^e_{1-}$ | $\mathcal{O}^e_{2+}$ | $\mathcal{O}^f_{2+}$ | $\mathcal{O}^f_{2-}$ |
| $(b,e,f):67$ | ${}^sR^{z'0}_{TT}$ | $R^{z'0}_{TT'}$ | ${}^sR^{0y}_{LT'}$ | ${}^cR^{00}_{LT}$ | ${}^sR^{0z}_{LT}$ | ${}^cR^{0z}_{LT'}$ |
| | $\mathcal{O}^b_{1+}$ | $\mathcal{O}^b_{2+}$ | $\mathcal{O}^e_{1-}$ | $\mathcal{O}^e_{2+}$ | $\mathcal{O}^f_{1+}$ | $\mathcal{O}^f_{2+}$ |
| $(b,e,f):68$ | ${}^sR^{z'0}_{TT}$ | $R^{z'0}_{TT'}$ | ${}^sR^{0y}_{LT'}$ | ${}^cR^{00}_{LT}$ | ${}^sR^{0z}_{LT}$ | ${}^sR^{0x}_{LT}$ |
| | $\mathcal{O}^b_{1+}$ | $\mathcal{O}^b_{2+}$ | $\mathcal{O}^e_{1-}$ | $\mathcal{O}^e_{2+}$ | $\mathcal{O}^f_{1+}$ | $\mathcal{O}^f_{2-}$ |
| $(b,e,f):69$ | ${}^sR^{z'0}_{TT}$ | $R^{z'0}_{TT'}$ | ${}^sR^{0y}_{LT'}$ | ${}^cR^{00}_{LT}$ | ${}^cR^{0x}_{LT'}$ | ${}^cR^{0z}_{LT'}$ |

| | | | | | | |
|---|---|---|---|---|---|---|
| | $\mathcal{O}^{b}_{1+}$ | $\mathcal{O}^{b}_{2+}$ | $\mathcal{O}^{e}_{1-}$ | $\mathcal{O}^{e}_{2+}$ | $\mathcal{O}^{f}_{1-}$ | $\mathcal{O}^{f}_{2+}$ |
| $(b,e,f):70$ | ${}^{s}R^{z'0}_{TT}$ | $R^{z'0}_{TT'}$ | ${}^{s}R^{0y}_{LT'}$ | ${}^{c}R^{00}_{LT}$ | ${}^{c}R^{0x}_{LT'}$ | ${}^{s}R^{0x}_{LT}$ |
| | $\mathcal{O}^{b}_{1+}$ | $\mathcal{O}^{b}_{2+}$ | $\mathcal{O}^{e}_{1-}$ | $\mathcal{O}^{e}_{2+}$ | $\mathcal{O}^{f}_{1-}$ | $\mathcal{O}^{f}_{2-}$ |
| $(b,e,f):71$ | ${}^{s}R^{z'0}_{TT}$ | $R^{z'0}_{TT'}$ | ${}^{s}R^{0y}_{LT'}$ | ${}^{c}R^{0y}_{LT}$ | ${}^{s}R^{0z}_{LT}$ | ${}^{c}R^{0x}_{LT'}$ |
| | $\mathcal{O}^{b}_{1+}$ | $\mathcal{O}^{b}_{2+}$ | $\mathcal{O}^{e}_{1-}$ | $\mathcal{O}^{e}_{2-}$ | $\mathcal{O}^{f}_{1+}$ | $\mathcal{O}^{f}_{1-}$ |
| $(b,e,f):72$ | ${}^{s}R^{z'0}_{TT}$ | $R^{z'0}_{TT'}$ | ${}^{s}R^{0y}_{LT'}$ | ${}^{c}R^{0y}_{LT}$ | ${}^{c}R^{0z}_{LT'}$ | ${}^{s}R^{0x}_{LT}$ |
| | $\mathcal{O}^{b}_{1+}$ | $\mathcal{O}^{b}_{2+}$ | $\mathcal{O}^{e}_{1-}$ | $\mathcal{O}^{e}_{2-}$ | $\mathcal{O}^{f}_{2+}$ | $\mathcal{O}^{f}_{2-}$ |
| $(b,e,f):73$ | ${}^{s}R^{z'0}_{TT}$ | $R^{z'0}_{TT'}$ | ${}^{s}R^{0y}_{LT'}$ | ${}^{c}R^{0y}_{LT}$ | ${}^{s}R^{0z}_{LT}$ | ${}^{c}R^{0z}_{LT'}$ |
| | $\mathcal{O}^{b}_{1+}$ | $\mathcal{O}^{b}_{2+}$ | $\mathcal{O}^{e}_{1-}$ | $\mathcal{O}^{e}_{2-}$ | $\mathcal{O}^{f}_{1+}$ | $\mathcal{O}^{f}_{2+}$ |
| $(b,e,f):74$ | ${}^{s}R^{z'0}_{TT}$ | $R^{z'0}_{TT'}$ | ${}^{s}R^{0y}_{LT'}$ | ${}^{c}R^{0y}_{LT}$ | ${}^{s}R^{0z}_{LT}$ | ${}^{s}R^{0x}_{LT}$ |
| | $\mathcal{O}^{b}_{1+}$ | $\mathcal{O}^{b}_{2+}$ | $\mathcal{O}^{e}_{1-}$ | $\mathcal{O}^{e}_{2-}$ | $\mathcal{O}^{f}_{1+}$ | $\mathcal{O}^{f}_{2-}$ |
| $(b,e,f):75$ | ${}^{s}R^{z'0}_{TT}$ | $R^{z'0}_{TT'}$ | ${}^{s}R^{0y}_{LT'}$ | ${}^{c}R^{0y}_{LT}$ | ${}^{c}R^{0x}_{LT'}$ | ${}^{c}R^{0z}_{LT'}$ |
| | $\mathcal{O}^{b}_{1+}$ | $\mathcal{O}^{b}_{2+}$ | $\mathcal{O}^{e}_{1-}$ | $\mathcal{O}^{e}_{2-}$ | $\mathcal{O}^{f}_{1-}$ | $\mathcal{O}^{f}_{2+}$ |
| $(b,e,f):76$ | ${}^{s}R^{z'0}_{TT}$ | $R^{z'0}_{TT'}$ | ${}^{s}R^{0y}_{LT'}$ | ${}^{c}R^{0y}_{LT}$ | ${}^{c}R^{0x}_{LT'}$ | ${}^{s}R^{0x}_{LT}$ |
| | $\mathcal{O}^{b}_{1+}$ | $\mathcal{O}^{b}_{2+}$ | $\mathcal{O}^{e}_{1-}$ | $\mathcal{O}^{e}_{2-}$ | $\mathcal{O}^{f}_{1-}$ | $\mathcal{O}^{f}_{2-}$ |
| $(b,e,f):77$ | ${}^{s}R^{z'0}_{TT}$ | ${}^{s}R^{x'0}_{TT}$ | ${}^{s}R^{00}_{LT'}$ | ${}^{s}R^{0y}_{LT'}$ | ${}^{s}R^{0z}_{LT}$ | ${}^{c}R^{0z}_{LT'}$ |
| | $\mathcal{O}^{b}_{1+}$ | $\mathcal{O}^{b}_{2-}$ | $\mathcal{O}^{e}_{1+}$ | $\mathcal{O}^{e}_{1-}$ | $\mathcal{O}^{f}_{1+}$ | $\mathcal{O}^{f}_{2+}$ |
| $(b,e,f):78$ | ${}^{s}R^{z'0}_{TT}$ | ${}^{s}R^{x'0}_{TT}$ | ${}^{s}R^{00}_{LT'}$ | ${}^{s}R^{0y}_{LT'}$ | ${}^{c}R^{0x}_{LT'}$ | ${}^{s}R^{0x}_{LT}$ |
| | $\mathcal{O}^{b}_{1+}$ | $\mathcal{O}^{b}_{2-}$ | $\mathcal{O}^{e}_{1+}$ | $\mathcal{O}^{e}_{1-}$ | $\mathcal{O}^{f}_{1-}$ | $\mathcal{O}^{f}_{2-}$ |
| $(b,e,f):79$ | ${}^{s}R^{z'0}_{TT}$ | ${}^{s}R^{x'0}_{TT}$ | ${}^{c}R^{00}_{LT}$ | ${}^{c}R^{0y}_{LT}$ | ${}^{s}R^{0z}_{LT}$ | ${}^{c}R^{0z}_{LT'}$ |
| | $\mathcal{O}^{b}_{1+}$ | $\mathcal{O}^{b}_{2-}$ | $\mathcal{O}^{e}_{2+}$ | $\mathcal{O}^{e}_{2-}$ | $\mathcal{O}^{f}_{1+}$ | $\mathcal{O}^{f}_{2+}$ |
| $(b,e,f):80$ | ${}^{s}R^{z'0}_{TT}$ | ${}^{s}R^{x'0}_{TT}$ | ${}^{c}R^{00}_{LT}$ | ${}^{c}R^{0y}_{LT}$ | ${}^{c}R^{0x}_{LT'}$ | ${}^{s}R^{0x}_{LT}$ |
| | $\mathcal{O}^{b}_{1+}$ | $\mathcal{O}^{b}_{2-}$ | $\mathcal{O}^{e}_{2+}$ | $\mathcal{O}^{e}_{2-}$ | $\mathcal{O}^{f}_{1-}$ | $\mathcal{O}^{f}_{2-}$ |
| $(b,e,f):81$ | ${}^{s}R^{z'0}_{TT}$ | ${}^{s}R^{x'0}_{TT}$ | ${}^{s}R^{00}_{LT'}$ | ${}^{c}R^{00}_{LT}$ | ${}^{s}R^{0z}_{LT}$ | ${}^{c}R^{0x}_{LT'}$ |
| | $\mathcal{O}^{b}_{1+}$ | $\mathcal{O}^{b}_{2-}$ | $\mathcal{O}^{e}_{1+}$ | $\mathcal{O}^{e}_{2+}$ | $\mathcal{O}^{f}_{1+}$ | $\mathcal{O}^{f}_{1-}$ |
| $(b,e,f):82$ | ${}^{s}R^{z'0}_{TT}$ | ${}^{s}R^{x'0}_{TT}$ | ${}^{s}R^{00}_{LT'}$ | ${}^{c}R^{00}_{LT}$ | ${}^{c}R^{0z}_{LT'}$ | ${}^{s}R^{0x}_{LT}$ |
| | $\mathcal{O}^{b}_{1+}$ | $\mathcal{O}^{b}_{2-}$ | $\mathcal{O}^{e}_{1+}$ | $\mathcal{O}^{e}_{2+}$ | $\mathcal{O}^{f}_{2+}$ | $\mathcal{O}^{f}_{2-}$ |
| $(b,e,f):83$ | ${}^{s}R^{z'0}_{TT}$ | ${}^{s}R^{x'0}_{TT}$ | ${}^{s}R^{00}_{LT'}$ | ${}^{c}R^{00}_{LT}$ | ${}^{s}R^{0z}_{LT}$ | ${}^{c}R^{0z}_{LT'}$ |
| | $\mathcal{O}^{b}_{1+}$ | $\mathcal{O}^{b}_{2-}$ | $\mathcal{O}^{e}_{1+}$ | $\mathcal{O}^{e}_{2+}$ | $\mathcal{O}^{f}_{1+}$ | $\mathcal{O}^{f}_{2+}$ |
| $(b,e,f):84$ | ${}^{s}R^{z'0}_{TT}$ | ${}^{s}R^{x'0}_{TT}$ | ${}^{s}R^{00}_{LT'}$ | ${}^{c}R^{00}_{LT}$ | ${}^{s}R^{0z}_{LT}$ | ${}^{s}R^{0x}_{LT}$ |
| | $\mathcal{O}^{b}_{1+}$ | $\mathcal{O}^{b}_{2-}$ | $\mathcal{O}^{e}_{1+}$ | $\mathcal{O}^{e}_{2+}$ | $\mathcal{O}^{f}_{1+}$ | $\mathcal{O}^{f}_{2-}$ |
| $(b,e,f):85$ | ${}^{s}R^{z'0}_{TT}$ | ${}^{s}R^{x'0}_{TT}$ | ${}^{s}R^{00}_{LT'}$ | ${}^{c}R^{00}_{LT}$ | ${}^{c}R^{0x}_{LT'}$ | ${}^{c}R^{0z}_{LT'}$ |
| | $\mathcal{O}^{b}_{1+}$ | $\mathcal{O}^{b}_{2-}$ | $\mathcal{O}^{e}_{1+}$ | $\mathcal{O}^{e}_{2+}$ | $\mathcal{O}^{f}_{1-}$ | $\mathcal{O}^{f}_{2+}$ |
| $(b,e,f):86$ | ${}^{s}R^{z'0}_{TT}$ | ${}^{s}R^{x'0}_{TT}$ | ${}^{s}R^{00}_{LT'}$ | ${}^{c}R^{00}_{LT}$ | ${}^{c}R^{0x}_{LT'}$ | ${}^{s}R^{0x}_{LT}$ |
| | $\mathcal{O}^{b}_{1+}$ | $\mathcal{O}^{b}_{2-}$ | $\mathcal{O}^{e}_{1+}$ | $\mathcal{O}^{e}_{2+}$ | $\mathcal{O}^{f}_{1-}$ | $\mathcal{O}^{f}_{2-}$ |
| $(b,e,f):87$ | ${}^{s}R^{z'0}_{TT}$ | ${}^{s}R^{x'0}_{TT}$ | ${}^{s}R^{00}_{LT'}$ | ${}^{c}R^{0y}_{LT}$ | ${}^{s}R^{0z}_{LT}$ | ${}^{c}R^{0z}_{LT'}$ |
| | $\mathcal{O}^{b}_{1+}$ | $\mathcal{O}^{b}_{2-}$ | $\mathcal{O}^{e}_{1+}$ | $\mathcal{O}^{e}_{2-}$ | $\mathcal{O}^{f}_{1+}$ | $\mathcal{O}^{f}_{2+}$ |
| $(b,e,f):88$ | ${}^{s}R^{z'0}_{TT}$ | ${}^{s}R^{x'0}_{TT}$ | ${}^{s}R^{00}_{LT'}$ | ${}^{c}R^{0y}_{LT}$ | ${}^{c}R^{0x}_{LT'}$ | ${}^{s}R^{0x}_{LT}$ |
| | $\mathcal{O}^{b}_{1+}$ | $\mathcal{O}^{b}_{2-}$ | $\mathcal{O}^{e}_{1+}$ | $\mathcal{O}^{e}_{2-}$ | $\mathcal{O}^{f}_{1-}$ | $\mathcal{O}^{f}_{2-}$ |
| $(b,e,f):89$ | ${}^{s}R^{z'0}_{TT}$ | ${}^{s}R^{x'0}_{TT}$ | ${}^{s}R^{0y}_{LT'}$ | ${}^{c}R^{00}_{LT}$ | ${}^{s}R^{0z}_{LT}$ | ${}^{c}R^{0z}_{LT'}$ |
| | $\mathcal{O}^{b}_{1+}$ | $\mathcal{O}^{b}_{2-}$ | $\mathcal{O}^{e}_{1-}$ | $\mathcal{O}^{e}_{2+}$ | $\mathcal{O}^{f}_{1+}$ | $\mathcal{O}^{f}_{2+}$ |
| $(b,e,f):90$ | ${}^{s}R^{z'0}_{TT}$ | ${}^{s}R^{x'0}_{TT}$ | ${}^{s}R^{0y}_{LT'}$ | ${}^{c}R^{00}_{LT}$ | ${}^{c}R^{0x}_{LT'}$ | ${}^{s}R^{0x}_{LT}$ |
| | $\mathcal{O}^{b}_{1+}$ | $\mathcal{O}^{b}_{2-}$ | $\mathcal{O}^{e}_{1-}$ | $\mathcal{O}^{e}_{2+}$ | $\mathcal{O}^{f}_{1-}$ | $\mathcal{O}^{f}_{2-}$ |
| $(b,e,f):91$ | ${}^{s}R^{z'0}_{TT}$ | ${}^{s}R^{x'0}_{TT}$ | ${}^{s}R^{0y}_{LT'}$ | ${}^{c}R^{0y}_{LT}$ | ${}^{s}R^{0z}_{LT}$ | ${}^{c}R^{0x}_{LT'}$ |
| | $\mathcal{O}^{b}_{1+}$ | $\mathcal{O}^{b}_{2-}$ | $\mathcal{O}^{e}_{1-}$ | $\mathcal{O}^{e}_{2-}$ | $\mathcal{O}^{f}_{1+}$ | $\mathcal{O}^{f}_{1-}$ |
| $(b,e,f):92$ | ${}^{s}R^{z'0}_{TT}$ | ${}^{s}R^{x'0}_{TT}$ | ${}^{s}R^{0y}_{LT'}$ | ${}^{c}R^{0y}_{LT}$ | ${}^{c}R^{0z}_{LT'}$ | ${}^{s}R^{0x}_{LT}$ |
| | $\mathcal{O}^{b}_{1+}$ | $\mathcal{O}^{b}_{2-}$ | $\mathcal{O}^{e}_{1-}$ | $\mathcal{O}^{e}_{2-}$ | $\mathcal{O}^{f}_{2+}$ | $\mathcal{O}^{f}_{2-}$ |
| $(b,e,f):93$ | ${}^{s}R^{z'0}_{TT}$ | ${}^{s}R^{x'0}_{TT}$ | ${}^{s}R^{0y}_{LT'}$ | ${}^{c}R^{0y}_{LT}$ | ${}^{s}R^{0z}_{LT}$ | ${}^{c}R^{0z}_{LT'}$ |
| | $\mathcal{O}^{b}_{1+}$ | $\mathcal{O}^{b}_{2-}$ | $\mathcal{O}^{e}_{1-}$ | $\mathcal{O}^{e}_{2-}$ | $\mathcal{O}^{f}_{1+}$ | $\mathcal{O}^{f}_{2+}$ |
| $(b,e,f):94$ | ${}^{s}R^{z'0}_{TT}$ | ${}^{s}R^{x'0}_{TT}$ | ${}^{s}R^{0y}_{LT'}$ | ${}^{c}R^{0y}_{LT}$ | ${}^{s}R^{0z}_{LT}$ | ${}^{s}R^{0x}_{LT}$ |
| | $\mathcal{O}^{b}_{1+}$ | $\mathcal{O}^{b}_{2-}$ | $\mathcal{O}^{e}_{1-}$ | $\mathcal{O}^{e}_{2-}$ | $\mathcal{O}^{f}_{1+}$ | $\mathcal{O}^{f}_{2-}$ |
| $(b,e,f):95$ | ${}^{s}R^{z'0}_{TT}$ | ${}^{s}R^{x'0}_{TT}$ | ${}^{s}R^{0y}_{LT'}$ | ${}^{c}R^{0y}_{LT}$ | ${}^{c}R^{0x}_{LT'}$ | ${}^{c}R^{0z}_{LT'}$ |
| | $\mathcal{O}^{b}_{1+}$ | $\mathcal{O}^{b}_{2-}$ | $\mathcal{O}^{e}_{1-}$ | $\mathcal{O}^{e}_{2-}$ | $\mathcal{O}^{f}_{1-}$ | $\mathcal{O}^{f}_{2+}$ |
| $(b,e,f):96$ | ${}^{s}R^{z'0}_{TT}$ | ${}^{s}R^{x'0}_{TT}$ | ${}^{s}R^{0y}_{LT'}$ | ${}^{c}R^{0y}_{LT}$ | ${}^{c}R^{0x}_{LT'}$ | ${}^{s}R^{0x}_{LT}$ |
| | $\mathcal{O}^{b}_{1+}$ | $\mathcal{O}^{b}_{2-}$ | $\mathcal{O}^{e}_{1-}$ | $\mathcal{O}^{e}_{2-}$ | $\mathcal{O}^{f}_{1-}$ | $\mathcal{O}^{f}_{2-}$ |

| | | | | | | |
|---|---|---|---|---|---|---|
| $(b,e,f):97$ | $R^{x'0}_{TT'}$ | $R^{z'0}_{TT'}$ | ${}^sR^{00}_{LT'}$ | ${}^sR^{0y}_{LT'}$ | ${}^sR^{0z}_{LT}$ | ${}^cR^{0z}_{LT'}$ |
| | $\mathcal{O}^b_{1-}$ | $\mathcal{O}^b_{2+}$ | $\mathcal{O}^e_{1+}$ | $\mathcal{O}^e_{1-}$ | $\mathcal{O}^f_{1+}$ | $\mathcal{O}^f_{2+}$ |
| $(b,e,f):98$ | $R^{x'0}_{TT'}$ | $R^{z'0}_{TT'}$ | ${}^sR^{00}_{LT'}$ | ${}^sR^{0y}_{LT'}$ | ${}^cR^{0x}_{LT'}$ | ${}^sR^{0x}_{LT}$ |
| | $\mathcal{O}^b_{1-}$ | $\mathcal{O}^b_{2+}$ | $\mathcal{O}^e_{1+}$ | $\mathcal{O}^e_{1-}$ | $\mathcal{O}^f_{1-}$ | $\mathcal{O}^f_{2-}$ |
| $(b,e,f):99$ | $R^{x'0}_{TT'}$ | $R^{z'0}_{TT'}$ | ${}^cR^{00}_{LT}$ | ${}^cR^{0y}_{LT}$ | ${}^sR^{0z}_{LT}$ | ${}^cR^{0z}_{LT'}$ |
| | $\mathcal{O}^b_{1-}$ | $\mathcal{O}^b_{2+}$ | $\mathcal{O}^e_{2+}$ | $\mathcal{O}^e_{2-}$ | $\mathcal{O}^f_{1+}$ | $\mathcal{O}^f_{2+}$ |
| $(b,e,f):100$ | $R^{x'0}_{TT'}$ | $R^{z'0}_{TT'}$ | ${}^cR^{00}_{LT}$ | ${}^cR^{0y}_{LT}$ | ${}^cR^{0x}_{LT'}$ | ${}^sR^{0x}_{LT}$ |
| | $\mathcal{O}^b_{1-}$ | $\mathcal{O}^b_{2+}$ | $\mathcal{O}^e_{2+}$ | $\mathcal{O}^e_{2-}$ | $\mathcal{O}^f_{1-}$ | $\mathcal{O}^f_{2-}$ |
| $(b,e,f):101$ | $R^{x'0}_{TT'}$ | $R^{z'0}_{TT'}$ | ${}^sR^{00}_{LT'}$ | ${}^cR^{00}_{LT}$ | ${}^sR^{0z}_{LT}$ | ${}^cR^{0x}_{LT'}$ |
| | $\mathcal{O}^b_{1-}$ | $\mathcal{O}^b_{2+}$ | $\mathcal{O}^e_{1+}$ | $\mathcal{O}^e_{2+}$ | $\mathcal{O}^f_{1+}$ | $\mathcal{O}^f_{1-}$ |
| $(b,e,f):102$ | $R^{x'0}_{TT'}$ | $R^{z'0}_{TT'}$ | ${}^sR^{00}_{LT'}$ | ${}^cR^{00}_{LT}$ | ${}^cR^{0z}_{LT'}$ | ${}^sR^{0x}_{LT}$ |
| | $\mathcal{O}^b_{1-}$ | $\mathcal{O}^b_{2+}$ | $\mathcal{O}^e_{1+}$ | $\mathcal{O}^e_{2+}$ | $\mathcal{O}^f_{2+}$ | $\mathcal{O}^f_{2-}$ |
| $(b,e,f):103$ | $R^{x'0}_{TT'}$ | $R^{z'0}_{TT'}$ | ${}^sR^{00}_{LT'}$ | ${}^cR^{00}_{LT}$ | ${}^sR^{0z}_{LT}$ | ${}^cR^{0z}_{LT'}$ |
| | $\mathcal{O}^b_{1-}$ | $\mathcal{O}^b_{2+}$ | $\mathcal{O}^e_{1+}$ | $\mathcal{O}^e_{2+}$ | $\mathcal{O}^f_{1+}$ | $\mathcal{O}^f_{2+}$ |
| $(b,e,f):104$ | $R^{x'0}_{TT'}$ | $R^{z'0}_{TT'}$ | ${}^sR^{00}_{LT'}$ | ${}^cR^{00}_{LT}$ | ${}^sR^{0z}_{LT}$ | ${}^sR^{0x}_{LT}$ |
| | $\mathcal{O}^b_{1-}$ | $\mathcal{O}^b_{2+}$ | $\mathcal{O}^e_{1+}$ | $\mathcal{O}^e_{2+}$ | $\mathcal{O}^f_{1+}$ | $\mathcal{O}^f_{2-}$ |
| $(b,e,f):105$ | $R^{x'0}_{TT'}$ | $R^{z'0}_{TT'}$ | ${}^sR^{00}_{LT'}$ | ${}^cR^{00}_{LT}$ | ${}^cR^{0x}_{LT'}$ | ${}^cR^{0z}_{LT'}$ |
| | $\mathcal{O}^b_{1-}$ | $\mathcal{O}^b_{2+}$ | $\mathcal{O}^e_{1+}$ | $\mathcal{O}^e_{2+}$ | $\mathcal{O}^f_{1-}$ | $\mathcal{O}^f_{2+}$ |
| $(b,e,f):106$ | $R^{x'0}_{TT'}$ | $R^{z'0}_{TT'}$ | ${}^sR^{00}_{LT'}$ | ${}^cR^{00}_{LT}$ | ${}^cR^{0x}_{LT'}$ | ${}^sR^{0x}_{LT}$ |
| | $\mathcal{O}^b_{1-}$ | $\mathcal{O}^b_{2+}$ | $\mathcal{O}^e_{1+}$ | $\mathcal{O}^e_{2+}$ | $\mathcal{O}^f_{1-}$ | $\mathcal{O}^f_{2-}$ |
| $(b,e,f):107$ | $R^{x'0}_{TT'}$ | $R^{z'0}_{TT'}$ | ${}^sR^{00}_{LT'}$ | ${}^cR^{0y}_{LT}$ | ${}^sR^{0z}_{LT}$ | ${}^cR^{0z}_{LT'}$ |
| | $\mathcal{O}^b_{1-}$ | $\mathcal{O}^b_{2+}$ | $\mathcal{O}^e_{1+}$ | $\mathcal{O}^e_{2-}$ | $\mathcal{O}^f_{1+}$ | $\mathcal{O}^f_{2+}$ |
| $(b,e,f):108$ | $R^{x'0}_{TT'}$ | $R^{z'0}_{TT'}$ | ${}^sR^{00}_{LT'}$ | ${}^cR^{0y}_{LT}$ | ${}^cR^{0x}_{LT'}$ | ${}^sR^{0x}_{LT}$ |
| | $\mathcal{O}^b_{1-}$ | $\mathcal{O}^b_{2+}$ | $\mathcal{O}^e_{1+}$ | $\mathcal{O}^e_{2-}$ | $\mathcal{O}^f_{1-}$ | $\mathcal{O}^f_{2-}$ |
| $(b,e,f):109$ | $R^{x'0}_{TT'}$ | $R^{z'0}_{TT'}$ | ${}^sR^{0y}_{LT'}$ | ${}^cR^{00}_{LT}$ | ${}^sR^{0z}_{LT}$ | ${}^cR^{0z}_{LT'}$ |
| | $\mathcal{O}^b_{1-}$ | $\mathcal{O}^b_{2+}$ | $\mathcal{O}^e_{1-}$ | $\mathcal{O}^e_{2+}$ | $\mathcal{O}^f_{1+}$ | $\mathcal{O}^f_{2+}$ |
| $(b,e,f):110$ | $R^{x'0}_{TT'}$ | $R^{z'0}_{TT'}$ | ${}^sR^{0y}_{LT'}$ | ${}^cR^{00}_{LT}$ | ${}^cR^{0x}_{LT'}$ | ${}^sR^{0x}_{LT}$ |
| | $\mathcal{O}^b_{1-}$ | $\mathcal{O}^b_{2+}$ | $\mathcal{O}^e_{1-}$ | $\mathcal{O}^e_{2+}$ | $\mathcal{O}^f_{1-}$ | $\mathcal{O}^f_{2-}$ |
| $(b,e,f):111$ | $R^{x'0}_{TT'}$ | $R^{z'0}_{TT'}$ | ${}^sR^{0y}_{LT'}$ | ${}^cR^{0y}_{LT}$ | ${}^sR^{0z}_{LT}$ | ${}^cR^{0x}_{LT'}$ |
| | $\mathcal{O}^b_{1-}$ | $\mathcal{O}^b_{2+}$ | $\mathcal{O}^e_{1-}$ | $\mathcal{O}^e_{2-}$ | $\mathcal{O}^f_{1+}$ | $\mathcal{O}^f_{1-}$ |
| $(b,e,f):112$ | $R^{x'0}_{TT'}$ | $R^{z'0}_{TT'}$ | ${}^sR^{0y}_{LT'}$ | ${}^cR^{0y}_{LT}$ | ${}^cR^{0z}_{LT'}$ | ${}^sR^{0x}_{LT}$ |
| | $\mathcal{O}^b_{1-}$ | $\mathcal{O}^b_{2+}$ | $\mathcal{O}^e_{1-}$ | $\mathcal{O}^e_{2-}$ | $\mathcal{O}^f_{2+}$ | $\mathcal{O}^f_{2-}$ |
| $(b,e,f):113$ | $R^{x'0}_{TT'}$ | $R^{z'0}_{TT'}$ | ${}^sR^{0y}_{LT'}$ | ${}^cR^{0y}_{LT}$ | ${}^sR^{0z}_{LT}$ | ${}^cR^{0z}_{LT'}$ |
| | $\mathcal{O}^b_{1-}$ | $\mathcal{O}^b_{2+}$ | $\mathcal{O}^e_{1-}$ | $\mathcal{O}^e_{2-}$ | $\mathcal{O}^f_{1+}$ | $\mathcal{O}^f_{2+}$ |
| $(b,e,f):114$ | $R^{x'0}_{TT'}$ | $R^{z'0}_{TT'}$ | ${}^sR^{0y}_{LT'}$ | ${}^cR^{0y}_{LT}$ | ${}^sR^{0z}_{LT}$ | ${}^sR^{0x}_{LT}$ |
| | $\mathcal{O}^b_{1-}$ | $\mathcal{O}^b_{2+}$ | $\mathcal{O}^e_{1-}$ | $\mathcal{O}^e_{2-}$ | $\mathcal{O}^f_{1+}$ | $\mathcal{O}^f_{2-}$ |
| $(b,e,f):115$ | $R^{x'0}_{TT'}$ | $R^{z'0}_{TT'}$ | ${}^sR^{0y}_{LT'}$ | ${}^cR^{0y}_{LT}$ | ${}^cR^{0x}_{LT'}$ | ${}^cR^{0z}_{LT'}$ |
| | $\mathcal{O}^b_{1-}$ | $\mathcal{O}^b_{2+}$ | $\mathcal{O}^e_{1-}$ | $\mathcal{O}^e_{2-}$ | $\mathcal{O}^f_{1-}$ | $\mathcal{O}^f_{2+}$ |
| $(b,e,f):116$ | $R^{x'0}_{TT'}$ | $R^{z'0}_{TT'}$ | ${}^sR^{0y}_{LT'}$ | ${}^cR^{0y}_{LT}$ | ${}^cR^{0x}_{LT'}$ | ${}^sR^{0x}_{LT}$ |
| | $\mathcal{O}^b_{1-}$ | $\mathcal{O}^b_{2+}$ | $\mathcal{O}^e_{1-}$ | $\mathcal{O}^e_{2-}$ | $\mathcal{O}^f_{1-}$ | $\mathcal{O}^f_{2-}$ |
| $(b,e,f):117$ | $R^{x'0}_{TT'}$ | ${}^sR^{x'0}_{TT}$ | ${}^sR^{00}_{LT'}$ | ${}^sR^{0y}_{LT'}$ | ${}^sR^{0z}_{LT}$ | ${}^cR^{0x}_{LT'}$ |
| | $\mathcal{O}^b_{1-}$ | $\mathcal{O}^b_{2-}$ | $\mathcal{O}^e_{1+}$ | $\mathcal{O}^e_{1-}$ | $\mathcal{O}^f_{1+}$ | $\mathcal{O}^f_{1-}$ |
| $(b,e,f):118$ | $R^{x'0}_{TT'}$ | ${}^sR^{x'0}_{TT}$ | ${}^sR^{00}_{LT'}$ | ${}^sR^{0y}_{LT'}$ | ${}^cR^{0z}_{LT'}$ | ${}^sR^{0x}_{LT}$ |
| | $\mathcal{O}^b_{1-}$ | $\mathcal{O}^b_{2-}$ | $\mathcal{O}^e_{1+}$ | $\mathcal{O}^e_{1-}$ | $\mathcal{O}^f_{2+}$ | $\mathcal{O}^f_{2-}$ |
| $(b,e,f):119$ | $R^{x'0}_{TT'}$ | ${}^sR^{x'0}_{TT}$ | ${}^sR^{00}_{LT'}$ | ${}^sR^{0y}_{LT'}$ | ${}^sR^{0z}_{LT}$ | ${}^cR^{0z}_{LT'}$ |
| | $\mathcal{O}^b_{1-}$ | $\mathcal{O}^b_{2-}$ | $\mathcal{O}^e_{1+}$ | $\mathcal{O}^e_{1-}$ | $\mathcal{O}^f_{1+}$ | $\mathcal{O}^f_{2+}$ |
| $(b,e,f):120$ | $R^{x'0}_{TT'}$ | ${}^sR^{x'0}_{TT}$ | ${}^sR^{00}_{LT'}$ | ${}^sR^{0y}_{LT'}$ | ${}^sR^{0z}_{LT}$ | ${}^sR^{0x}_{LT}$ |
| | $\mathcal{O}^b_{1-}$ | $\mathcal{O}^b_{2-}$ | $\mathcal{O}^e_{1+}$ | $\mathcal{O}^e_{1-}$ | $\mathcal{O}^f_{1+}$ | $\mathcal{O}^f_{2-}$ |
| $(b,e,f):121$ | $R^{x'0}_{TT'}$ | ${}^sR^{x'0}_{TT}$ | ${}^sR^{00}_{LT'}$ | ${}^sR^{0y}_{LT'}$ | ${}^cR^{0x}_{LT'}$ | ${}^cR^{0z}_{LT'}$ |
| | $\mathcal{O}^b_{1-}$ | $\mathcal{O}^b_{2-}$ | $\mathcal{O}^e_{1+}$ | $\mathcal{O}^e_{1-}$ | $\mathcal{O}^f_{1-}$ | $\mathcal{O}^f_{2+}$ |
| $(b,e,f):122$ | $R^{x'0}_{TT'}$ | ${}^sR^{x'0}_{TT}$ | ${}^sR^{00}_{LT'}$ | ${}^sR^{0y}_{LT'}$ | ${}^cR^{0x}_{LT'}$ | ${}^sR^{0x}_{LT}$ |
| | $\mathcal{O}^b_{1-}$ | $\mathcal{O}^b_{2-}$ | $\mathcal{O}^e_{1+}$ | $\mathcal{O}^e_{1-}$ | $\mathcal{O}^f_{1-}$ | $\mathcal{O}^f_{2-}$ |
| $(b,e,f):123$ | $R^{x'0}_{TT'}$ | ${}^sR^{x'0}_{TT}$ | ${}^cR^{00}_{LT}$ | ${}^cR^{0y}_{LT}$ | ${}^sR^{0z}_{LT}$ | ${}^cR^{0x}_{LT'}$ |
| | $\mathcal{O}^b_{1-}$ | $\mathcal{O}^b_{2-}$ | $\mathcal{O}^e_{2+}$ | $\mathcal{O}^e_{2-}$ | $\mathcal{O}^f_{1+}$ | $\mathcal{O}^f_{1-}$ |
| $(b,e,f):124$ | $R^{x'0}_{TT'}$ | ${}^sR^{x'0}_{TT}$ | ${}^cR^{00}_{LT}$ | ${}^cR^{0y}_{LT}$ | ${}^cR^{0z}_{LT'}$ | ${}^sR^{0x}_{LT}$ |

| | | | | | | |
|---|---|---|---|---|---|---|
| | $\mathcal{O}^b_{1-}$ | $\mathcal{O}^b_{2-}$ | $\mathcal{O}^e_{2+}$ | $\mathcal{O}^e_{2-}$ | $\mathcal{O}^f_{2+}$ | $\mathcal{O}^f_{2-}$ |
| $(b,e,f):125$ | $R^{x'0}_{TT'}$ | ${}^sR^{x'0}_{TT}$ | ${}^cR^{00}_{LT}$ | ${}^cR^{0y}_{LT}$ | ${}^sR^{0z}_{LT}$ | ${}^cR^{0z}_{LT'}$ |
| | $\mathcal{O}^b_{1-}$ | $\mathcal{O}^b_{2-}$ | $\mathcal{O}^e_{2+}$ | $\mathcal{O}^e_{2-}$ | $\mathcal{O}^f_{1+}$ | $\mathcal{O}^f_{2+}$ |
| $(b,e,f):126$ | $R^{x'0}_{TT'}$ | ${}^sR^{x'0}_{TT}$ | ${}^cR^{00}_{LT}$ | ${}^cR^{0y}_{LT}$ | ${}^sR^{0z}_{LT}$ | ${}^sR^{0x}_{LT}$ |
| | $\mathcal{O}^b_{1-}$ | $\mathcal{O}^b_{2-}$ | $\mathcal{O}^e_{2+}$ | $\mathcal{O}^e_{2-}$ | $\mathcal{O}^f_{1+}$ | $\mathcal{O}^f_{2-}$ |
| $(b,e,f):127$ | $R^{x'0}_{TT'}$ | ${}^sR^{x'0}_{TT}$ | ${}^cR^{00}_{LT}$ | ${}^cR^{0y}_{LT}$ | ${}^cR^{0x}_{LT'}$ | ${}^cR^{0z}_{LT'}$ |
| | $\mathcal{O}^b_{1-}$ | $\mathcal{O}^b_{2-}$ | $\mathcal{O}^e_{2+}$ | $\mathcal{O}^e_{2-}$ | $\mathcal{O}^f_{1-}$ | $\mathcal{O}^f_{2+}$ |
| $(b,e,f):128$ | $R^{x'0}_{TT'}$ | ${}^sR^{x'0}_{TT}$ | ${}^cR^{00}_{LT}$ | ${}^cR^{0y}_{LT}$ | ${}^cR^{0x}_{LT'}$ | ${}^sR^{0x}_{LT}$ |
| | $\mathcal{O}^b_{1-}$ | $\mathcal{O}^b_{2-}$ | $\mathcal{O}^e_{2+}$ | $\mathcal{O}^e_{2-}$ | $\mathcal{O}^f_{1-}$ | $\mathcal{O}^f_{2-}$ |
| $(b,e,f):129$ | $R^{x'0}_{TT'}$ | ${}^sR^{x'0}_{TT}$ | ${}^sR^{00}_{LT'}$ | ${}^cR^{00}_{LT}$ | ${}^sR^{0z}_{LT}$ | ${}^cR^{0x}_{LT'}$ |
| | $\mathcal{O}^b_{1-}$ | $\mathcal{O}^b_{2-}$ | $\mathcal{O}^e_{1+}$ | $\mathcal{O}^e_{2+}$ | $\mathcal{O}^f_{1+}$ | $\mathcal{O}^f_{1-}$ |
| $(b,e,f):130$ | $R^{x'0}_{TT'}$ | ${}^sR^{x'0}_{TT}$ | ${}^sR^{00}_{LT'}$ | ${}^cR^{00}_{LT}$ | ${}^cR^{0z}_{LT'}$ | ${}^sR^{0x}_{LT}$ |
| | $\mathcal{O}^b_{1-}$ | $\mathcal{O}^b_{2-}$ | $\mathcal{O}^e_{1+}$ | $\mathcal{O}^e_{2+}$ | $\mathcal{O}^f_{2+}$ | $\mathcal{O}^f_{2-}$ |
| $(b,e,f):131$ | $R^{x'0}_{TT'}$ | ${}^sR^{x'0}_{TT}$ | ${}^sR^{00}_{LT'}$ | ${}^cR^{00}_{LT}$ | ${}^sR^{0z}_{LT}$ | ${}^cR^{0z}_{LT'}$ |
| | $\mathcal{O}^b_{1-}$ | $\mathcal{O}^b_{2-}$ | $\mathcal{O}^e_{1+}$ | $\mathcal{O}^e_{2+}$ | $\mathcal{O}^f_{1+}$ | $\mathcal{O}^f_{2+}$ |
| $(b,e,f):132$ | $R^{x'0}_{TT'}$ | ${}^sR^{x'0}_{TT}$ | ${}^sR^{00}_{LT'}$ | ${}^cR^{00}_{LT}$ | ${}^sR^{0z}_{LT}$ | ${}^sR^{0x}_{LT}$ |
| | $\mathcal{O}^b_{1-}$ | $\mathcal{O}^b_{2-}$ | $\mathcal{O}^e_{1+}$ | $\mathcal{O}^e_{2+}$ | $\mathcal{O}^f_{1+}$ | $\mathcal{O}^f_{2-}$ |
| $(b,e,f):133$ | $R^{x'0}_{TT'}$ | ${}^sR^{x'0}_{TT}$ | ${}^sR^{00}_{LT'}$ | ${}^cR^{00}_{LT}$ | ${}^cR^{0x}_{LT'}$ | ${}^cR^{0z}_{LT'}$ |
| | $\mathcal{O}^b_{1-}$ | $\mathcal{O}^b_{2-}$ | $\mathcal{O}^e_{1+}$ | $\mathcal{O}^e_{2+}$ | $\mathcal{O}^f_{1-}$ | $\mathcal{O}^f_{2+}$ |
| $(b,e,f):134$ | $R^{x'0}_{TT'}$ | ${}^sR^{x'0}_{TT}$ | ${}^sR^{00}_{LT'}$ | ${}^cR^{00}_{LT}$ | ${}^cR^{0x}_{LT'}$ | ${}^sR^{0x}_{LT}$ |
| | $\mathcal{O}^b_{1-}$ | $\mathcal{O}^b_{2-}$ | $\mathcal{O}^e_{1+}$ | $\mathcal{O}^e_{2+}$ | $\mathcal{O}^f_{1-}$ | $\mathcal{O}^f_{2-}$ |
| $(b,e,f):135$ | $R^{x'0}_{TT'}$ | ${}^sR^{x'0}_{TT}$ | ${}^sR^{00}_{LT'}$ | ${}^cR^{0y}_{LT}$ | ${}^sR^{0z}_{LT}$ | ${}^cR^{0x}_{LT'}$ |
| | $\mathcal{O}^b_{1-}$ | $\mathcal{O}^b_{2-}$ | $\mathcal{O}^e_{1+}$ | $\mathcal{O}^e_{2-}$ | $\mathcal{O}^f_{1+}$ | $\mathcal{O}^f_{1-}$ |
| $(b,e,f):136$ | $R^{x'0}_{TT'}$ | ${}^sR^{x'0}_{TT}$ | ${}^sR^{00}_{LT'}$ | ${}^cR^{0y}_{LT}$ | ${}^cR^{0z}_{LT'}$ | ${}^sR^{0x}_{LT}$ |
| | $\mathcal{O}^b_{1-}$ | $\mathcal{O}^b_{2-}$ | $\mathcal{O}^e_{1+}$ | $\mathcal{O}^e_{2-}$ | $\mathcal{O}^f_{2+}$ | $\mathcal{O}^f_{2-}$ |
| $(b,e,f):137$ | $R^{x'0}_{TT'}$ | ${}^sR^{x'0}_{TT}$ | ${}^sR^{00}_{LT'}$ | ${}^cR^{0y}_{LT}$ | ${}^sR^{0z}_{LT}$ | ${}^cR^{0z}_{LT'}$ |
| | $\mathcal{O}^b_{1-}$ | $\mathcal{O}^b_{2-}$ | $\mathcal{O}^e_{1+}$ | $\mathcal{O}^e_{2-}$ | $\mathcal{O}^f_{1+}$ | $\mathcal{O}^f_{2+}$ |
| $(b,e,f):138$ | $R^{x'0}_{TT'}$ | ${}^sR^{x'0}_{TT}$ | ${}^sR^{00}_{LT'}$ | ${}^cR^{0y}_{LT}$ | ${}^sR^{0z}_{LT}$ | ${}^sR^{0x}_{LT}$ |
| | $\mathcal{O}^b_{1-}$ | $\mathcal{O}^b_{2-}$ | $\mathcal{O}^e_{1+}$ | $\mathcal{O}^e_{2-}$ | $\mathcal{O}^f_{1+}$ | $\mathcal{O}^f_{2-}$ |
| $(b,e,f):139$ | $R^{x'0}_{TT'}$ | ${}^sR^{x'0}_{TT}$ | ${}^sR^{00}_{LT'}$ | ${}^cR^{0y}_{LT}$ | ${}^cR^{0x}_{LT'}$ | ${}^cR^{0z}_{LT'}$ |
| | $\mathcal{O}^b_{1-}$ | $\mathcal{O}^b_{2-}$ | $\mathcal{O}^e_{1+}$ | $\mathcal{O}^e_{2-}$ | $\mathcal{O}^f_{1-}$ | $\mathcal{O}^f_{2+}$ |
| $(b,e,f):140$ | $R^{x'0}_{TT'}$ | ${}^sR^{x'0}_{TT}$ | ${}^sR^{00}_{LT'}$ | ${}^cR^{0y}_{LT}$ | ${}^cR^{0x}_{LT'}$ | ${}^sR^{0x}_{LT}$ |
| | $\mathcal{O}^b_{1-}$ | $\mathcal{O}^b_{2-}$ | $\mathcal{O}^e_{1+}$ | $\mathcal{O}^e_{2-}$ | $\mathcal{O}^f_{1-}$ | $\mathcal{O}^f_{2-}$ |
| $(b,e,f):141$ | $R^{x'0}_{TT'}$ | ${}^sR^{x'0}_{TT}$ | ${}^sR^{0y}_{LT'}$ | ${}^cR^{00}_{LT}$ | ${}^sR^{0z}_{LT}$ | ${}^cR^{0x}_{LT'}$ |
| | $\mathcal{O}^b_{1-}$ | $\mathcal{O}^b_{2-}$ | $\mathcal{O}^e_{1-}$ | $\mathcal{O}^e_{2+}$ | $\mathcal{O}^f_{1+}$ | $\mathcal{O}^f_{1-}$ |
| $(b,e,f):142$ | $R^{x'0}_{TT'}$ | ${}^sR^{x'0}_{TT}$ | ${}^sR^{0y}_{LT'}$ | ${}^cR^{00}_{LT}$ | ${}^cR^{0z}_{LT'}$ | ${}^sR^{0x}_{LT}$ |
| | $\mathcal{O}^b_{1-}$ | $\mathcal{O}^b_{2-}$ | $\mathcal{O}^e_{1-}$ | $\mathcal{O}^e_{2+}$ | $\mathcal{O}^f_{2+}$ | $\mathcal{O}^f_{2-}$ |
| $(b,e,f):143$ | $R^{x'0}_{TT'}$ | ${}^sR^{x'0}_{TT}$ | ${}^sR^{0y}_{LT'}$ | ${}^cR^{00}_{LT}$ | ${}^sR^{0z}_{LT}$ | ${}^cR^{0z}_{LT'}$ |
| | $\mathcal{O}^b_{1-}$ | $\mathcal{O}^b_{2-}$ | $\mathcal{O}^e_{1-}$ | $\mathcal{O}^e_{2+}$ | $\mathcal{O}^f_{1+}$ | $\mathcal{O}^f_{2+}$ |
| $(b,e,f):144$ | $R^{x'0}_{TT'}$ | ${}^sR^{x'0}_{TT}$ | ${}^sR^{0y}_{LT'}$ | ${}^cR^{00}_{LT}$ | ${}^sR^{0z}_{LT}$ | ${}^sR^{0x}_{LT}$ |
| | $\mathcal{O}^b_{1-}$ | $\mathcal{O}^b_{2-}$ | $\mathcal{O}^e_{1-}$ | $\mathcal{O}^e_{2+}$ | $\mathcal{O}^f_{1+}$ | $\mathcal{O}^f_{2-}$ |
| $(b,e,f):145$ | $R^{x'0}_{TT'}$ | ${}^sR^{x'0}_{TT}$ | ${}^sR^{0y}_{LT'}$ | ${}^cR^{00}_{LT}$ | ${}^cR^{0x}_{LT'}$ | ${}^cR^{0z}_{LT'}$ |
| | $\mathcal{O}^b_{1-}$ | $\mathcal{O}^b_{2-}$ | $\mathcal{O}^e_{1-}$ | $\mathcal{O}^e_{2+}$ | $\mathcal{O}^f_{1-}$ | $\mathcal{O}^f_{2+}$ |
| $(b,e,f):146$ | $R^{x'0}_{TT'}$ | ${}^sR^{x'0}_{TT}$ | ${}^sR^{0y}_{LT'}$ | ${}^cR^{00}_{LT}$ | ${}^cR^{0x}_{LT'}$ | ${}^sR^{0x}_{LT}$ |
| | $\mathcal{O}^b_{1-}$ | $\mathcal{O}^b_{2-}$ | $\mathcal{O}^e_{1-}$ | $\mathcal{O}^e_{2+}$ | $\mathcal{O}^f_{1-}$ | $\mathcal{O}^f_{2-}$ |
| $(b,e,f):147$ | $R^{x'0}_{TT'}$ | ${}^sR^{x'0}_{TT}$ | ${}^sR^{0y}_{LT'}$ | ${}^cR^{0y}_{LT}$ | ${}^sR^{0z}_{LT}$ | ${}^cR^{0x}_{LT'}$ |
| | $\mathcal{O}^b_{1-}$ | $\mathcal{O}^b_{2-}$ | $\mathcal{O}^e_{1-}$ | $\mathcal{O}^e_{2-}$ | $\mathcal{O}^f_{1+}$ | $\mathcal{O}^f_{1-}$ |
| $(b,e,f):148$ | $R^{x'0}_{TT'}$ | ${}^sR^{x'0}_{TT}$ | ${}^sR^{0y}_{LT'}$ | ${}^cR^{0y}_{LT}$ | ${}^cR^{0z}_{LT'}$ | ${}^sR^{0x}_{LT}$ |
| | $\mathcal{O}^b_{1-}$ | $\mathcal{O}^b_{2-}$ | $\mathcal{O}^e_{1-}$ | $\mathcal{O}^e_{2-}$ | $\mathcal{O}^f_{2+}$ | $\mathcal{O}^f_{2-}$ |
| $(b,e,f):149$ | $R^{x'0}_{TT'}$ | ${}^sR^{x'0}_{TT}$ | ${}^sR^{0y}_{LT'}$ | ${}^cR^{0y}_{LT}$ | ${}^sR^{0z}_{LT}$ | ${}^cR^{0z}_{LT'}$ |
| | $\mathcal{O}^b_{1-}$ | $\mathcal{O}^b_{2-}$ | $\mathcal{O}^e_{1-}$ | $\mathcal{O}^e_{2-}$ | $\mathcal{O}^f_{1+}$ | $\mathcal{O}^f_{2+}$ |
| $(b,e,f):150$ | $R^{x'0}_{TT'}$ | ${}^sR^{x'0}_{TT}$ | ${}^sR^{0y}_{LT'}$ | ${}^cR^{0y}_{LT}$ | ${}^sR^{0z}_{LT}$ | ${}^sR^{0x}_{LT}$ |
| | $\mathcal{O}^b_{1-}$ | $\mathcal{O}^b_{2-}$ | $\mathcal{O}^e_{1-}$ | $\mathcal{O}^e_{2-}$ | $\mathcal{O}^f_{1+}$ | $\mathcal{O}^f_{2-}$ |
| $(b,e,f):151$ | $R^{x'0}_{TT'}$ | ${}^sR^{x'0}_{TT}$ | ${}^sR^{0y}_{LT'}$ | ${}^cR^{0y}_{LT}$ | ${}^cR^{0x}_{LT'}$ | ${}^cR^{0z}_{LT'}$ |
| | $\mathcal{O}^b_{1-}$ | $\mathcal{O}^b_{2-}$ | $\mathcal{O}^e_{1-}$ | $\mathcal{O}^e_{2-}$ | $\mathcal{O}^f_{1-}$ | $\mathcal{O}^f_{2+}$ |

| | | | | | | |
|---|---|---|---|---|---|---|
| $(b,e,f):152$ | $R_{TT'}^{x'0}$ | ${}^{s}R_{TT}^{x'0}$ | ${}^{s}R_{LT'}^{0y}$ | ${}^{c}R_{LT}^{0y}$ | ${}^{c}R_{LT'}^{0x}$ | ${}^{s}R_{LT}^{0x}$ |
| | $\mathcal{O}_{1-}^{b}$ | $\mathcal{O}_{2-}^{b}$ | $\mathcal{O}_{1-}^{e}$ | $\mathcal{O}_{2-}^{e}$ | $\mathcal{O}_{1-}^{f}$ | $\mathcal{O}_{2-}^{f}$ |

TABLE VII: All the fully complete sets determined from the combination of shape-classes $(b,g,h)$ (i.e. graph-topology 'IV') in the case of pseudoscalar meson electroproduction are listed here. The observables are written in the systematic symbolic notation $\mathcal{O}_{\nu\pm}^{n}$ by Nakayama [1], as well as in the more commonly used notation in terms of 'response-functions' $R_{i}^{\beta\alpha}$ (cf. references [4, 5]). The given sets of 6 observables have to be combined with the 6 'diagonal' observables $\left\{R_{T}^{00}, {}^{c}R_{TT}^{00}, R_{T}^{0y}, R_{T}^{y'0}, R_{L}^{00}, R_{L}^{0y}\right\}$ in order to form a complete set of minimal length $2N = 12$. All of these sets have been verified to be complete using Mathematica [3].

| Set-Nr. | Observables | | | | | |
|---|---|---|---|---|---|---|
| $(b,g,h):1$ | ${}^{s}R_{TT}^{z'0}$ | $R_{TT'}^{x'0}$ | ${}^{s}R_{LT}^{z'0}$ | ${}^{c}R_{LT'}^{x'0}$ | ${}^{s}R_{LT'}^{x'x}$ | ${}^{c}R_{LT}^{x'x}$ |
| | $\mathcal{O}_{1+}^{b}$ | $\mathcal{O}_{1-}^{b}$ | $\mathcal{O}_{1+}^{g}$ | $\mathcal{O}_{1-}^{g}$ | $\mathcal{O}_{1+}^{h}$ | $\mathcal{O}_{2+}^{h}$ |
| $(b,g,h):2$ | ${}^{s}R_{TT}^{z'0}$ | $R_{TT'}^{x'0}$ | ${}^{s}R_{LT}^{z'0}$ | ${}^{c}R_{LT'}^{x'0}$ | ${}^{c}R_{LT}^{z'x}$ | ${}^{s}R_{LT'}^{z'x}$ |
| | $\mathcal{O}_{1+}^{b}$ | $\mathcal{O}_{1-}^{b}$ | $\mathcal{O}_{1+}^{g}$ | $\mathcal{O}_{1-}^{g}$ | $\mathcal{O}_{1-}^{h}$ | $\mathcal{O}_{2-}^{h}$ |
| $(b,g,h):3$ | ${}^{s}R_{TT}^{z'0}$ | $R_{TT'}^{x'0}$ | ${}^{c}R_{LT'}^{z'0}$ | ${}^{s}R_{LT}^{x'0}$ | ${}^{s}R_{LT'}^{x'x}$ | ${}^{c}R_{LT}^{x'x}$ |
| | $\mathcal{O}_{1+}^{b}$ | $\mathcal{O}_{1-}^{b}$ | $\mathcal{O}_{2+}^{g}$ | $\mathcal{O}_{2-}^{g}$ | $\mathcal{O}_{1+}^{h}$ | $\mathcal{O}_{2+}^{h}$ |
| $(b,g,h):4$ | ${}^{s}R_{TT}^{z'0}$ | $R_{TT'}^{x'0}$ | ${}^{c}R_{LT'}^{z'0}$ | ${}^{s}R_{LT}^{x'0}$ | ${}^{c}R_{LT}^{z'x}$ | ${}^{s}R_{LT'}^{z'x}$ |
| | $\mathcal{O}_{1+}^{b}$ | $\mathcal{O}_{1-}^{b}$ | $\mathcal{O}_{2+}^{g}$ | $\mathcal{O}_{2-}^{g}$ | $\mathcal{O}_{1-}^{h}$ | $\mathcal{O}_{2-}^{h}$ |
| $(b,g,h):5$ | ${}^{s}R_{TT}^{z'0}$ | $R_{TT'}^{x'0}$ | ${}^{s}R_{LT}^{z'0}$ | ${}^{c}R_{LT'}^{z'0}$ | ${}^{s}R_{LT'}^{x'x}$ | ${}^{c}R_{LT}^{z'x}$ |
| | $\mathcal{O}_{1+}^{b}$ | $\mathcal{O}_{1-}^{b}$ | $\mathcal{O}_{1+}^{g}$ | $\mathcal{O}_{2+}^{g}$ | $\mathcal{O}_{1+}^{h}$ | $\mathcal{O}_{1-}^{h}$ |
| $(b,g,h):6$ | ${}^{s}R_{TT}^{z'0}$ | $R_{TT'}^{x'0}$ | ${}^{s}R_{LT}^{z'0}$ | ${}^{c}R_{LT'}^{z'0}$ | ${}^{c}R_{LT}^{x'x}$ | ${}^{s}R_{LT'}^{z'x}$ |
| | $\mathcal{O}_{1+}^{b}$ | $\mathcal{O}_{1-}^{b}$ | $\mathcal{O}_{1+}^{g}$ | $\mathcal{O}_{2+}^{g}$ | $\mathcal{O}_{2+}^{h}$ | $\mathcal{O}_{2-}^{h}$ |
| $(b,g,h):7$ | ${}^{s}R_{TT}^{z'0}$ | $R_{TT'}^{x'0}$ | ${}^{s}R_{LT}^{z'0}$ | ${}^{c}R_{LT'}^{z'0}$ | ${}^{s}R_{LT'}^{x'x}$ | ${}^{c}R_{LT}^{x'x}$ |
| | $\mathcal{O}_{1+}^{b}$ | $\mathcal{O}_{1-}^{b}$ | $\mathcal{O}_{1+}^{g}$ | $\mathcal{O}_{2+}^{g}$ | $\mathcal{O}_{1+}^{h}$ | $\mathcal{O}_{2+}^{h}$ |
| $(b,g,h):8$ | ${}^{s}R_{TT}^{z'0}$ | $R_{TT'}^{x'0}$ | ${}^{s}R_{LT}^{z'0}$ | ${}^{c}R_{LT'}^{z'0}$ | ${}^{s}R_{LT'}^{x'x}$ | ${}^{s}R_{LT'}^{z'x}$ |
| | $\mathcal{O}_{1+}^{b}$ | $\mathcal{O}_{1-}^{b}$ | $\mathcal{O}_{1+}^{g}$ | $\mathcal{O}_{2+}^{g}$ | $\mathcal{O}_{1+}^{h}$ | $\mathcal{O}_{2-}^{h}$ |
| $(b,g,h):9$ | ${}^{s}R_{TT}^{z'0}$ | $R_{TT'}^{x'0}$ | ${}^{s}R_{LT}^{z'0}$ | ${}^{c}R_{LT'}^{z'0}$ | ${}^{c}R_{LT}^{z'x}$ | ${}^{c}R_{LT}^{x'x}$ |
| | $\mathcal{O}_{1+}^{b}$ | $\mathcal{O}_{1-}^{b}$ | $\mathcal{O}_{1+}^{g}$ | $\mathcal{O}_{2+}^{g}$ | $\mathcal{O}_{1-}^{h}$ | $\mathcal{O}_{2+}^{h}$ |
| $(b,g,h):10$ | ${}^{s}R_{TT}^{z'0}$ | $R_{TT'}^{x'0}$ | ${}^{s}R_{LT}^{z'0}$ | ${}^{c}R_{LT'}^{z'0}$ | ${}^{c}R_{LT}^{z'x}$ | ${}^{s}R_{LT'}^{z'x}$ |
| | $\mathcal{O}_{1+}^{b}$ | $\mathcal{O}_{1-}^{b}$ | $\mathcal{O}_{1+}^{g}$ | $\mathcal{O}_{2+}^{g}$ | $\mathcal{O}_{1-}^{h}$ | $\mathcal{O}_{2-}^{h}$ |
| $(b,g,h):11$ | ${}^{s}R_{TT}^{z'0}$ | $R_{TT'}^{x'0}$ | ${}^{s}R_{LT}^{z'0}$ | ${}^{s}R_{LT}^{x'0}$ | ${}^{s}R_{LT'}^{x'x}$ | ${}^{c}R_{LT}^{x'x}$ |
| | $\mathcal{O}_{1+}^{b}$ | $\mathcal{O}_{1-}^{b}$ | $\mathcal{O}_{1+}^{g}$ | $\mathcal{O}_{2-}^{g}$ | $\mathcal{O}_{1+}^{h}$ | $\mathcal{O}_{2+}^{h}$ |
| $(b,g,h):12$ | ${}^{s}R_{TT}^{z'0}$ | $R_{TT'}^{x'0}$ | ${}^{s}R_{LT}^{z'0}$ | ${}^{s}R_{LT}^{x'0}$ | ${}^{c}R_{LT}^{z'x}$ | ${}^{s}R_{LT'}^{z'x}$ |
| | $\mathcal{O}_{1+}^{b}$ | $\mathcal{O}_{1-}^{b}$ | $\mathcal{O}_{1+}^{g}$ | $\mathcal{O}_{2-}^{g}$ | $\mathcal{O}_{1-}^{h}$ | $\mathcal{O}_{2-}^{h}$ |
| $(b,g,h):13$ | ${}^{s}R_{TT}^{z'0}$ | $R_{TT'}^{x'0}$ | ${}^{c}R_{LT'}^{x'0}$ | ${}^{c}R_{LT'}^{z'0}$ | ${}^{s}R_{LT'}^{x'x}$ | ${}^{c}R_{LT}^{x'x}$ |
| | $\mathcal{O}_{1+}^{b}$ | $\mathcal{O}_{1-}^{b}$ | $\mathcal{O}_{1-}^{g}$ | $\mathcal{O}_{2+}^{g}$ | $\mathcal{O}_{1+}^{h}$ | $\mathcal{O}_{2+}^{h}$ |
| $(b,g,h):14$ | ${}^{s}R_{TT}^{z'0}$ | $R_{TT'}^{x'0}$ | ${}^{c}R_{LT'}^{x'0}$ | ${}^{c}R_{LT'}^{z'0}$ | ${}^{c}R_{LT}^{z'x}$ | ${}^{s}R_{LT'}^{z'x}$ |
| | $\mathcal{O}_{1+}^{b}$ | $\mathcal{O}_{1-}^{b}$ | $\mathcal{O}_{1-}^{g}$ | $\mathcal{O}_{2+}^{g}$ | $\mathcal{O}_{1-}^{h}$ | $\mathcal{O}_{2-}^{h}$ |
| $(b,g,h):15$ | ${}^{s}R_{TT}^{z'0}$ | $R_{TT'}^{x'0}$ | ${}^{c}R_{LT'}^{x'0}$ | ${}^{s}R_{LT}^{x'0}$ | ${}^{s}R_{LT'}^{x'x}$ | ${}^{c}R_{LT}^{z'x}$ |
| | $\mathcal{O}_{1+}^{b}$ | $\mathcal{O}_{1-}^{b}$ | $\mathcal{O}_{1-}^{g}$ | $\mathcal{O}_{2-}^{g}$ | $\mathcal{O}_{1+}^{h}$ | $\mathcal{O}_{1-}^{h}$ |
| $(b,g,h):16$ | ${}^{s}R_{TT}^{z'0}$ | $R_{TT'}^{x'0}$ | ${}^{c}R_{LT'}^{x'0}$ | ${}^{s}R_{LT}^{x'0}$ | ${}^{c}R_{LT}^{x'x}$ | ${}^{s}R_{LT'}^{z'x}$ |
| | $\mathcal{O}_{1+}^{b}$ | $\mathcal{O}_{1-}^{b}$ | $\mathcal{O}_{1-}^{g}$ | $\mathcal{O}_{2-}^{g}$ | $\mathcal{O}_{2+}^{h}$ | $\mathcal{O}_{2-}^{h}$ |
| $(b,g,h):17$ | ${}^{s}R_{TT}^{z'0}$ | $R_{TT'}^{x'0}$ | ${}^{c}R_{LT'}^{x'0}$ | ${}^{s}R_{LT}^{x'0}$ | ${}^{s}R_{LT'}^{x'x}$ | ${}^{c}R_{LT}^{x'x}$ |
| | $\mathcal{O}_{1+}^{b}$ | $\mathcal{O}_{1-}^{b}$ | $\mathcal{O}_{1-}^{g}$ | $\mathcal{O}_{2-}^{g}$ | $\mathcal{O}_{1+}^{h}$ | $\mathcal{O}_{2+}^{h}$ |
| $(b,g,h):18$ | ${}^{s}R_{TT}^{z'0}$ | $R_{TT'}^{x'0}$ | ${}^{c}R_{LT'}^{x'0}$ | ${}^{s}R_{LT}^{x'0}$ | ${}^{s}R_{LT'}^{x'x}$ | ${}^{s}R_{LT'}^{z'x}$ |
| | $\mathcal{O}_{1+}^{b}$ | $\mathcal{O}_{1-}^{b}$ | $\mathcal{O}_{1-}^{g}$ | $\mathcal{O}_{2-}^{g}$ | $\mathcal{O}_{1+}^{h}$ | $\mathcal{O}_{2-}^{h}$ |
| $(b,g,h):19$ | ${}^{s}R_{TT}^{z'0}$ | $R_{TT'}^{x'0}$ | ${}^{c}R_{LT'}^{x'0}$ | ${}^{s}R_{LT}^{x'0}$ | ${}^{c}R_{LT}^{z'x}$ | ${}^{c}R_{LT}^{x'x}$ |
| | $\mathcal{O}_{1+}^{b}$ | $\mathcal{O}_{1-}^{b}$ | $\mathcal{O}_{1-}^{g}$ | $\mathcal{O}_{2-}^{g}$ | $\mathcal{O}_{1-}^{h}$ | $\mathcal{O}_{2+}^{h}$ |
| $(b,g,h):20$ | ${}^{s}R_{TT}^{z'0}$ | $R_{TT'}^{x'0}$ | ${}^{c}R_{LT'}^{x'0}$ | ${}^{s}R_{LT}^{x'0}$ | ${}^{c}R_{LT}^{z'x}$ | ${}^{s}R_{LT'}^{z'x}$ |
| | $\mathcal{O}_{1+}^{b}$ | $\mathcal{O}_{1-}^{b}$ | $\mathcal{O}_{1-}^{g}$ | $\mathcal{O}_{2-}^{g}$ | $\mathcal{O}_{1-}^{h}$ | $\mathcal{O}_{2-}^{h}$ |

| | | | | | | |
|---|---|---|---|---|---|---|
| $(b,g,h):21$ | $R^{z'0}_{TT'}$ | ${}^sR^{x'0}_{TT}$ | ${}^sR^{z'0}_{LT}$ | ${}^cR^{x'0}_{LT'}$ | ${}^sR^{x'x}_{LT'}$ | ${}^cR^{x'x}_{LT}$ |
| | $\mathcal{O}^b_{2+}$ | $\mathcal{O}^b_{2-}$ | $\mathcal{O}^g_{1+}$ | $\mathcal{O}^g_{1-}$ | $\mathcal{O}^h_{1+}$ | $\mathcal{O}^h_{2+}$ |
| $(b,g,h):22$ | $R^{z'0}_{TT'}$ | ${}^sR^{x'0}_{TT}$ | ${}^sR^{z'0}_{LT}$ | ${}^cR^{x'0}_{LT'}$ | ${}^cR^{z'x}_{LT}$ | ${}^sR^{z'x}_{LT'}$ |
| | $\mathcal{O}^b_{2+}$ | $\mathcal{O}^b_{2-}$ | $\mathcal{O}^g_{1+}$ | $\mathcal{O}^g_{1-}$ | $\mathcal{O}^h_{1-}$ | $\mathcal{O}^h_{2-}$ |
| $(b,g,h):23$ | $R^{z'0}_{TT'}$ | ${}^sR^{x'0}_{TT}$ | ${}^cR^{z'0}_{LT'}$ | ${}^sR^{x'0}_{LT}$ | ${}^sR^{x'x}_{LT'}$ | ${}^cR^{x'x}_{LT}$ |
| | $\mathcal{O}^b_{2+}$ | $\mathcal{O}^b_{2-}$ | $\mathcal{O}^g_{2+}$ | $\mathcal{O}^g_{2-}$ | $\mathcal{O}^h_{1+}$ | $\mathcal{O}^h_{2+}$ |
| $(b,g,h):24$ | $R^{z'0}_{TT'}$ | ${}^sR^{x'0}_{TT}$ | ${}^cR^{z'0}_{LT'}$ | ${}^sR^{x'0}_{LT}$ | ${}^cR^{z'x}_{LT}$ | ${}^sR^{z'x}_{LT'}$ |
| | $\mathcal{O}^b_{2+}$ | $\mathcal{O}^b_{2-}$ | $\mathcal{O}^g_{2+}$ | $\mathcal{O}^g_{2-}$ | $\mathcal{O}^h_{1-}$ | $\mathcal{O}^h_{2-}$ |
| $(b,g,h):25$ | $R^{z'0}_{TT'}$ | ${}^sR^{x'0}_{TT}$ | ${}^sR^{z'0}_{LT}$ | ${}^cR^{z'0}_{LT'}$ | ${}^sR^{x'x}_{LT'}$ | ${}^cR^{z'x}_{LT}$ |
| | $\mathcal{O}^b_{2+}$ | $\mathcal{O}^b_{2-}$ | $\mathcal{O}^g_{1+}$ | $\mathcal{O}^g_{2+}$ | $\mathcal{O}^h_{1+}$ | $\mathcal{O}^h_{1-}$ |
| $(b,g,h):26$ | $R^{z'0}_{TT'}$ | ${}^sR^{x'0}_{TT}$ | ${}^sR^{z'0}_{LT}$ | ${}^cR^{z'0}_{LT'}$ | ${}^cR^{x'x}_{LT}$ | ${}^sR^{z'x}_{LT'}$ |
| | $\mathcal{O}^b_{2+}$ | $\mathcal{O}^b_{2-}$ | $\mathcal{O}^g_{1+}$ | $\mathcal{O}^g_{2+}$ | $\mathcal{O}^h_{2+}$ | $\mathcal{O}^h_{2-}$ |
| $(b,g,h):27$ | $R^{z'0}_{TT'}$ | ${}^sR^{x'0}_{TT}$ | ${}^sR^{z'0}_{LT}$ | ${}^cR^{z'0}_{LT'}$ | ${}^sR^{x'x}_{LT'}$ | ${}^cR^{x'x}_{LT}$ |
| | $\mathcal{O}^b_{2+}$ | $\mathcal{O}^b_{2-}$ | $\mathcal{O}^g_{1+}$ | $\mathcal{O}^g_{2+}$ | $\mathcal{O}^h_{1+}$ | $\mathcal{O}^h_{2+}$ |
| $(b,g,h):28$ | $R^{z'0}_{TT'}$ | ${}^sR^{x'0}_{TT}$ | ${}^sR^{z'0}_{LT}$ | ${}^cR^{z'0}_{LT'}$ | ${}^sR^{x'x}_{LT'}$ | ${}^sR^{z'x}_{LT'}$ |
| | $\mathcal{O}^b_{2+}$ | $\mathcal{O}^b_{2-}$ | $\mathcal{O}^g_{1+}$ | $\mathcal{O}^g_{2+}$ | $\mathcal{O}^h_{1+}$ | $\mathcal{O}^h_{2-}$ |
| $(b,g,h):29$ | $R^{z'0}_{TT'}$ | ${}^sR^{x'0}_{TT}$ | ${}^sR^{z'0}_{LT}$ | ${}^cR^{z'0}_{LT'}$ | ${}^cR^{z'x}_{LT}$ | ${}^cR^{x'x}_{LT}$ |
| | $\mathcal{O}^b_{2+}$ | $\mathcal{O}^b_{2-}$ | $\mathcal{O}^g_{1+}$ | $\mathcal{O}^g_{2+}$ | $\mathcal{O}^h_{1-}$ | $\mathcal{O}^h_{2+}$ |
| $(b,g,h):30$ | $R^{z'0}_{TT'}$ | ${}^sR^{x'0}_{TT}$ | ${}^sR^{z'0}_{LT}$ | ${}^cR^{z'0}_{LT'}$ | ${}^cR^{z'x}_{LT}$ | ${}^sR^{z'x}_{LT'}$ |
| | $\mathcal{O}^b_{2+}$ | $\mathcal{O}^b_{2-}$ | $\mathcal{O}^g_{1+}$ | $\mathcal{O}^g_{2+}$ | $\mathcal{O}^h_{1-}$ | $\mathcal{O}^h_{2-}$ |
| $(b,g,h):31$ | $R^{z'0}_{TT'}$ | ${}^sR^{x'0}_{TT}$ | ${}^sR^{z'0}_{LT}$ | ${}^sR^{x'0}_{LT}$ | ${}^sR^{x'x}_{LT'}$ | ${}^cR^{x'x}_{LT}$ |
| | $\mathcal{O}^b_{2+}$ | $\mathcal{O}^b_{2-}$ | $\mathcal{O}^g_{1+}$ | $\mathcal{O}^g_{2-}$ | $\mathcal{O}^h_{1+}$ | $\mathcal{O}^h_{2+}$ |
| $(b,g,h):32$ | $R^{z'0}_{TT'}$ | ${}^sR^{x'0}_{TT}$ | ${}^sR^{z'0}_{LT}$ | ${}^sR^{x'0}_{LT}$ | ${}^cR^{z'x}_{LT}$ | ${}^sR^{z'x}_{LT'}$ |
| | $\mathcal{O}^b_{2+}$ | $\mathcal{O}^b_{2-}$ | $\mathcal{O}^g_{1+}$ | $\mathcal{O}^g_{2-}$ | $\mathcal{O}^h_{1-}$ | $\mathcal{O}^h_{2-}$ |
| $(b,g,h):33$ | $R^{z'0}_{TT'}$ | ${}^sR^{x'0}_{TT}$ | ${}^cR^{x'0}_{LT'}$ | ${}^cR^{z'0}_{LT'}$ | ${}^sR^{x'x}_{LT'}$ | ${}^cR^{x'x}_{LT}$ |
| | $\mathcal{O}^b_{2+}$ | $\mathcal{O}^b_{2-}$ | $\mathcal{O}^g_{1-}$ | $\mathcal{O}^g_{2+}$ | $\mathcal{O}^h_{1+}$ | $\mathcal{O}^h_{2+}$ |
| $(b,g,h):34$ | $R^{z'0}_{TT'}$ | ${}^sR^{x'0}_{TT}$ | ${}^cR^{x'0}_{LT'}$ | ${}^cR^{z'0}_{LT'}$ | ${}^cR^{z'x}_{LT}$ | ${}^sR^{z'x}_{LT'}$ |
| | $\mathcal{O}^b_{2+}$ | $\mathcal{O}^b_{2-}$ | $\mathcal{O}^g_{1-}$ | $\mathcal{O}^g_{2+}$ | $\mathcal{O}^h_{1-}$ | $\mathcal{O}^h_{2-}$ |
| $(b,g,h):35$ | $R^{z'0}_{TT'}$ | ${}^sR^{x'0}_{TT}$ | ${}^cR^{x'0}_{LT'}$ | ${}^sR^{x'0}_{LT}$ | ${}^sR^{x'x}_{LT'}$ | ${}^cR^{z'x}_{LT}$ |
| | $\mathcal{O}^b_{2+}$ | $\mathcal{O}^b_{2-}$ | $\mathcal{O}^g_{1-}$ | $\mathcal{O}^g_{2-}$ | $\mathcal{O}^h_{1+}$ | $\mathcal{O}^h_{1-}$ |
| $(b,g,h):36$ | $R^{z'0}_{TT'}$ | ${}^sR^{x'0}_{TT}$ | ${}^cR^{x'0}_{LT'}$ | ${}^sR^{x'0}_{LT}$ | ${}^cR^{x'x}_{LT}$ | ${}^sR^{z'x}_{LT'}$ |
| | $\mathcal{O}^b_{2+}$ | $\mathcal{O}^b_{2-}$ | $\mathcal{O}^g_{1-}$ | $\mathcal{O}^g_{2-}$ | $\mathcal{O}^h_{2+}$ | $\mathcal{O}^h_{2-}$ |
| $(b,g,h):37$ | $R^{z'0}_{TT'}$ | ${}^sR^{x'0}_{TT}$ | ${}^cR^{x'0}_{LT'}$ | ${}^sR^{x'0}_{LT}$ | ${}^sR^{x'x}_{LT'}$ | ${}^cR^{x'x}_{LT}$ |
| | $\mathcal{O}^b_{2+}$ | $\mathcal{O}^b_{2-}$ | $\mathcal{O}^g_{1-}$ | $\mathcal{O}^g_{2-}$ | $\mathcal{O}^h_{1+}$ | $\mathcal{O}^h_{2+}$ |
| $(b,g,h):38$ | $R^{z'0}_{TT'}$ | ${}^sR^{x'0}_{TT}$ | ${}^cR^{x'0}_{LT'}$ | ${}^sR^{x'0}_{LT}$ | ${}^sR^{x'x}_{LT'}$ | ${}^sR^{z'x}_{LT'}$ |
| | $\mathcal{O}^b_{2+}$ | $\mathcal{O}^b_{2-}$ | $\mathcal{O}^g_{1-}$ | $\mathcal{O}^g_{2-}$ | $\mathcal{O}^h_{1+}$ | $\mathcal{O}^h_{2-}$ |
| $(b,g,h):39$ | $R^{z'0}_{TT'}$ | ${}^sR^{x'0}_{TT}$ | ${}^cR^{x'0}_{LT'}$ | ${}^sR^{x'0}_{LT}$ | ${}^cR^{z'x}_{LT}$ | ${}^cR^{x'x}_{LT}$ |
| | $\mathcal{O}^b_{2+}$ | $\mathcal{O}^b_{2-}$ | $\mathcal{O}^g_{1-}$ | $\mathcal{O}^g_{2-}$ | $\mathcal{O}^h_{1-}$ | $\mathcal{O}^h_{2+}$ |
| $(b,g,h):40$ | $R^{z'0}_{TT'}$ | ${}^sR^{x'0}_{TT}$ | ${}^cR^{x'0}_{LT'}$ | ${}^sR^{x'0}_{LT}$ | ${}^cR^{z'x}_{LT}$ | ${}^sR^{z'x}_{LT'}$ |
| | $\mathcal{O}^b_{2+}$ | $\mathcal{O}^b_{2-}$ | $\mathcal{O}^g_{1-}$ | $\mathcal{O}^g_{2-}$ | $\mathcal{O}^h_{1-}$ | $\mathcal{O}^h_{2-}$ |
| $(b,g,h):41$ | ${}^sR^{z'0}_{TT}$ | $R^{z'0}_{TT'}$ | ${}^sR^{z'0}_{LT}$ | ${}^cR^{x'0}_{LT'}$ | ${}^sR^{x'x}_{LT'}$ | ${}^cR^{z'x}_{LT}$ |
| | $\mathcal{O}^b_{1+}$ | $\mathcal{O}^b_{2+}$ | $\mathcal{O}^g_{1+}$ | $\mathcal{O}^g_{1-}$ | $\mathcal{O}^h_{1+}$ | $\mathcal{O}^h_{1-}$ |
| $(b,g,h):42$ | ${}^sR^{z'0}_{TT}$ | $R^{z'0}_{TT'}$ | ${}^sR^{z'0}_{LT}$ | ${}^cR^{x'0}_{LT'}$ | ${}^cR^{x'x}_{LT}$ | ${}^sR^{z'x}_{LT'}$ |
| | $\mathcal{O}^b_{1+}$ | $\mathcal{O}^b_{2+}$ | $\mathcal{O}^g_{1+}$ | $\mathcal{O}^g_{1-}$ | $\mathcal{O}^h_{2+}$ | $\mathcal{O}^h_{2-}$ |
| $(b,g,h):43$ | ${}^sR^{z'0}_{TT}$ | $R^{z'0}_{TT'}$ | ${}^sR^{z'0}_{LT}$ | ${}^cR^{x'0}_{LT'}$ | ${}^sR^{x'x}_{LT'}$ | ${}^cR^{x'x}_{LT}$ |
| | $\mathcal{O}^b_{1+}$ | $\mathcal{O}^b_{2+}$ | $\mathcal{O}^g_{1+}$ | $\mathcal{O}^g_{1-}$ | $\mathcal{O}^h_{1+}$ | $\mathcal{O}^h_{2+}$ |
| $(b,g,h):44$ | ${}^sR^{z'0}_{TT}$ | $R^{z'0}_{TT'}$ | ${}^sR^{z'0}_{LT}$ | ${}^cR^{x'0}_{LT'}$ | ${}^sR^{x'x}_{LT'}$ | ${}^sR^{z'x}_{LT'}$ |
| | $\mathcal{O}^b_{1+}$ | $\mathcal{O}^b_{2+}$ | $\mathcal{O}^g_{1+}$ | $\mathcal{O}^g_{1-}$ | $\mathcal{O}^h_{1+}$ | $\mathcal{O}^h_{2-}$ |
| $(b,g,h):45$ | ${}^sR^{z'0}_{TT}$ | $R^{z'0}_{TT'}$ | ${}^sR^{z'0}_{LT}$ | ${}^cR^{x'0}_{LT'}$ | ${}^cR^{z'x}_{LT}$ | ${}^cR^{x'x}_{LT}$ |
| | $\mathcal{O}^b_{1+}$ | $\mathcal{O}^b_{2+}$ | $\mathcal{O}^g_{1+}$ | $\mathcal{O}^g_{1-}$ | $\mathcal{O}^h_{1-}$ | $\mathcal{O}^h_{2+}$ |
| $(b,g,h):46$ | ${}^sR^{z'0}_{TT}$ | $R^{z'0}_{TT'}$ | ${}^sR^{z'0}_{LT}$ | ${}^cR^{x'0}_{LT'}$ | ${}^cR^{z'x}_{LT}$ | ${}^sR^{z'x}_{LT'}$ |
| | $\mathcal{O}^b_{1+}$ | $\mathcal{O}^b_{2+}$ | $\mathcal{O}^g_{1+}$ | $\mathcal{O}^g_{1-}$ | $\mathcal{O}^h_{1-}$ | $\mathcal{O}^h_{2-}$ |
| $(b,g,h):47$ | ${}^sR^{z'0}_{TT}$ | $R^{z'0}_{TT'}$ | ${}^cR^{z'0}_{LT'}$ | ${}^sR^{x'0}_{LT}$ | ${}^sR^{x'x}_{LT'}$ | ${}^cR^{z'x}_{LT}$ |
| | $\mathcal{O}^b_{1+}$ | $\mathcal{O}^b_{2+}$ | $\mathcal{O}^g_{2+}$ | $\mathcal{O}^g_{2-}$ | $\mathcal{O}^h_{1+}$ | $\mathcal{O}^h_{1-}$ |
| $(b,g,h):48$ | ${}^sR^{z'0}_{TT}$ | $R^{z'0}_{TT'}$ | ${}^cR^{z'0}_{LT'}$ | ${}^sR^{x'0}_{LT}$ | ${}^cR^{x'x}_{LT}$ | ${}^sR^{z'x}_{LT'}$ |
| | $\mathcal{O}^b_{1+}$ | $\mathcal{O}^b_{2+}$ | $\mathcal{O}^g_{2+}$ | $\mathcal{O}^g_{2-}$ | $\mathcal{O}^h_{2+}$ | $\mathcal{O}^h_{2-}$ |

| | | | | | | |
|---|---|---|---|---|---|---|
| $(b,g,h):49$ | ${}^sR^{z'0}_{TT}$ | $R^{z'0}_{TT'}$ | ${}^cR^{z'0}_{LT'}$ | ${}^sR^{x'0}_{LT}$ | ${}^sR^{x'x}_{LT'}$ | ${}^cR^{x'x}_{LT}$ |
| | $\mathcal{O}^b_{1+}$ | $\mathcal{O}^b_{2+}$ | $\mathcal{O}^g_{2+}$ | $\mathcal{O}^g_{2-}$ | $\mathcal{O}^h_{1+}$ | $\mathcal{O}^h_{2+}$ |
| $(b,g,h):50$ | ${}^sR^{z'0}_{TT}$ | $R^{z'0}_{TT'}$ | ${}^cR^{z'0}_{LT'}$ | ${}^sR^{x'0}_{LT}$ | ${}^sR^{x'x}_{LT'}$ | ${}^sR^{z'x}_{LT'}$ |
| | $\mathcal{O}^b_{1+}$ | $\mathcal{O}^b_{2+}$ | $\mathcal{O}^g_{2+}$ | $\mathcal{O}^g_{2-}$ | $\mathcal{O}^h_{1+}$ | $\mathcal{O}^h_{2-}$ |
| $(b,g,h):51$ | ${}^sR^{z'0}_{TT}$ | $R^{z'0}_{TT'}$ | ${}^cR^{z'0}_{LT'}$ | ${}^sR^{x'0}_{LT}$ | ${}^cR^{z'x}_{LT}$ | ${}^cR^{x'x}_{LT}$ |
| | $\mathcal{O}^b_{1+}$ | $\mathcal{O}^b_{2+}$ | $\mathcal{O}^g_{2+}$ | $\mathcal{O}^g_{2-}$ | $\mathcal{O}^h_{1-}$ | $\mathcal{O}^h_{2+}$ |
| $(b,g,h):52$ | ${}^sR^{z'0}_{TT}$ | $R^{z'0}_{TT'}$ | ${}^cR^{z'0}_{LT'}$ | ${}^sR^{x'0}_{LT}$ | ${}^cR^{z'x}_{LT}$ | ${}^sR^{z'x}_{LT'}$ |
| | $\mathcal{O}^b_{1+}$ | $\mathcal{O}^b_{2+}$ | $\mathcal{O}^g_{2+}$ | $\mathcal{O}^g_{2-}$ | $\mathcal{O}^h_{1-}$ | $\mathcal{O}^h_{2-}$ |
| $(b,g,h):53$ | ${}^sR^{z'0}_{TT}$ | $R^{z'0}_{TT'}$ | ${}^sR^{z'0}_{LT}$ | ${}^cR^{z'0}_{LT'}$ | ${}^sR^{x'x}_{LT'}$ | ${}^cR^{z'x}_{LT}$ |
| | $\mathcal{O}^b_{1+}$ | $\mathcal{O}^b_{2+}$ | $\mathcal{O}^g_{1+}$ | $\mathcal{O}^g_{2+}$ | $\mathcal{O}^h_{1+}$ | $\mathcal{O}^h_{1-}$ |
| $(b,g,h):54$ | ${}^sR^{z'0}_{TT}$ | $R^{z'0}_{TT'}$ | ${}^sR^{z'0}_{LT}$ | ${}^cR^{z'0}_{LT'}$ | ${}^cR^{x'x}_{LT}$ | ${}^sR^{z'x}_{LT'}$ |
| | $\mathcal{O}^b_{1+}$ | $\mathcal{O}^b_{2+}$ | $\mathcal{O}^g_{1+}$ | $\mathcal{O}^g_{2+}$ | $\mathcal{O}^h_{2+}$ | $\mathcal{O}^h_{2-}$ |
| $(b,g,h):55$ | ${}^sR^{z'0}_{TT}$ | $R^{z'0}_{TT'}$ | ${}^sR^{z'0}_{LT}$ | ${}^cR^{z'0}_{LT'}$ | ${}^sR^{x'x}_{LT'}$ | ${}^cR^{x'x}_{LT}$ |
| | $\mathcal{O}^b_{1+}$ | $\mathcal{O}^b_{2+}$ | $\mathcal{O}^g_{1+}$ | $\mathcal{O}^g_{2+}$ | $\mathcal{O}^h_{1+}$ | $\mathcal{O}^h_{2+}$ |
| $(b,g,h):56$ | ${}^sR^{z'0}_{TT}$ | $R^{z'0}_{TT'}$ | ${}^sR^{z'0}_{LT}$ | ${}^cR^{z'0}_{LT'}$ | ${}^sR^{x'x}_{LT'}$ | ${}^sR^{z'x}_{LT'}$ |
| | $\mathcal{O}^b_{1+}$ | $\mathcal{O}^b_{2+}$ | $\mathcal{O}^g_{1+}$ | $\mathcal{O}^g_{2+}$ | $\mathcal{O}^h_{1+}$ | $\mathcal{O}^h_{2-}$ |
| $(b,g,h):57$ | ${}^sR^{z'0}_{TT}$ | $R^{z'0}_{TT'}$ | ${}^sR^{z'0}_{LT}$ | ${}^cR^{z'0}_{LT'}$ | ${}^cR^{z'x}_{LT}$ | ${}^cR^{x'x}_{LT}$ |
| | $\mathcal{O}^b_{1+}$ | $\mathcal{O}^b_{2+}$ | $\mathcal{O}^g_{1+}$ | $\mathcal{O}^g_{2+}$ | $\mathcal{O}^h_{1-}$ | $\mathcal{O}^h_{2+}$ |
| $(b,g,h):58$ | ${}^sR^{z'0}_{TT}$ | $R^{z'0}_{TT'}$ | ${}^sR^{z'0}_{LT}$ | ${}^cR^{z'0}_{LT'}$ | ${}^cR^{z'x}_{LT}$ | ${}^sR^{z'x}_{LT'}$ |
| | $\mathcal{O}^b_{1+}$ | $\mathcal{O}^b_{2+}$ | $\mathcal{O}^g_{1+}$ | $\mathcal{O}^g_{2+}$ | $\mathcal{O}^h_{1-}$ | $\mathcal{O}^h_{2-}$ |
| $(b,g,h):59$ | ${}^sR^{z'0}_{TT}$ | $R^{z'0}_{TT'}$ | ${}^sR^{z'0}_{LT}$ | ${}^sR^{x'0}_{LT}$ | ${}^sR^{x'x}_{LT'}$ | ${}^cR^{z'x}_{LT}$ |
| | $\mathcal{O}^b_{1+}$ | $\mathcal{O}^b_{2+}$ | $\mathcal{O}^g_{1+}$ | $\mathcal{O}^g_{2-}$ | $\mathcal{O}^h_{1+}$ | $\mathcal{O}^h_{1-}$ |
| $(b,g,h):60$ | ${}^sR^{z'0}_{TT}$ | $R^{z'0}_{TT'}$ | ${}^sR^{z'0}_{LT}$ | ${}^sR^{x'0}_{LT}$ | ${}^cR^{x'x}_{LT}$ | ${}^sR^{z'x}_{LT'}$ |
| | $\mathcal{O}^b_{1+}$ | $\mathcal{O}^b_{2+}$ | $\mathcal{O}^g_{1+}$ | $\mathcal{O}^g_{2-}$ | $\mathcal{O}^h_{2+}$ | $\mathcal{O}^h_{2-}$ |
| $(b,g,h):61$ | ${}^sR^{z'0}_{TT}$ | $R^{z'0}_{TT'}$ | ${}^sR^{z'0}_{LT}$ | ${}^sR^{x'0}_{LT}$ | ${}^sR^{x'x}_{LT'}$ | ${}^cR^{x'x}_{LT}$ |
| | $\mathcal{O}^b_{1+}$ | $\mathcal{O}^b_{2+}$ | $\mathcal{O}^g_{1+}$ | $\mathcal{O}^g_{2-}$ | $\mathcal{O}^h_{1+}$ | $\mathcal{O}^h_{2+}$ |
| $(b,g,h):62$ | ${}^sR^{z'0}_{TT}$ | $R^{z'0}_{TT'}$ | ${}^sR^{z'0}_{LT}$ | ${}^sR^{x'0}_{LT}$ | ${}^sR^{x'x}_{LT'}$ | ${}^sR^{z'x}_{LT'}$ |
| | $\mathcal{O}^b_{1+}$ | $\mathcal{O}^b_{2+}$ | $\mathcal{O}^g_{1+}$ | $\mathcal{O}^g_{2-}$ | $\mathcal{O}^h_{1+}$ | $\mathcal{O}^h_{2-}$ |
| $(b,g,h):63$ | ${}^sR^{z'0}_{TT}$ | $R^{z'0}_{TT'}$ | ${}^sR^{z'0}_{LT}$ | ${}^sR^{x'0}_{LT}$ | ${}^cR^{z'x}_{LT}$ | ${}^cR^{x'x}_{LT}$ |
| | $\mathcal{O}^b_{1+}$ | $\mathcal{O}^b_{2+}$ | $\mathcal{O}^g_{1+}$ | $\mathcal{O}^g_{2-}$ | $\mathcal{O}^h_{1-}$ | $\mathcal{O}^h_{2+}$ |
| $(b,g,h):64$ | ${}^sR^{z'0}_{TT}$ | $R^{z'0}_{TT'}$ | ${}^sR^{z'0}_{LT}$ | ${}^sR^{x'0}_{LT}$ | ${}^cR^{z'x}_{LT}$ | ${}^sR^{z'x}_{LT'}$ |
| | $\mathcal{O}^b_{1+}$ | $\mathcal{O}^b_{2+}$ | $\mathcal{O}^g_{1+}$ | $\mathcal{O}^g_{2-}$ | $\mathcal{O}^h_{1-}$ | $\mathcal{O}^h_{2-}$ |
| $(b,g,h):65$ | ${}^sR^{z'0}_{TT}$ | $R^{z'0}_{TT'}$ | ${}^cR^{x'0}_{LT'}$ | ${}^cR^{z'0}_{LT'}$ | ${}^sR^{x'x}_{LT'}$ | ${}^cR^{z'x}_{LT}$ |
| | $\mathcal{O}^b_{1+}$ | $\mathcal{O}^b_{2+}$ | $\mathcal{O}^g_{1-}$ | $\mathcal{O}^g_{2+}$ | $\mathcal{O}^h_{1+}$ | $\mathcal{O}^h_{1-}$ |
| $(b,g,h):66$ | ${}^sR^{z'0}_{TT}$ | $R^{z'0}_{TT'}$ | ${}^cR^{x'0}_{LT'}$ | ${}^cR^{z'0}_{LT'}$ | ${}^cR^{x'x}_{LT}$ | ${}^sR^{z'x}_{LT'}$ |
| | $\mathcal{O}^b_{1+}$ | $\mathcal{O}^b_{2+}$ | $\mathcal{O}^g_{1-}$ | $\mathcal{O}^g_{2+}$ | $\mathcal{O}^h_{2+}$ | $\mathcal{O}^h_{2-}$ |
| $(b,g,h):67$ | ${}^sR^{z'0}_{TT}$ | $R^{z'0}_{TT'}$ | ${}^cR^{x'0}_{LT'}$ | ${}^cR^{z'0}_{LT'}$ | ${}^sR^{x'x}_{LT'}$ | ${}^cR^{x'x}_{LT}$ |
| | $\mathcal{O}^b_{1+}$ | $\mathcal{O}^b_{2+}$ | $\mathcal{O}^g_{1-}$ | $\mathcal{O}^g_{2+}$ | $\mathcal{O}^h_{1+}$ | $\mathcal{O}^h_{2+}$ |
| $(b,g,h):68$ | ${}^sR^{z'0}_{TT}$ | $R^{z'0}_{TT'}$ | ${}^cR^{x'0}_{LT'}$ | ${}^cR^{z'0}_{LT'}$ | ${}^sR^{x'x}_{LT'}$ | ${}^sR^{z'x}_{LT'}$ |
| | $\mathcal{O}^b_{1+}$ | $\mathcal{O}^b_{2+}$ | $\mathcal{O}^g_{1-}$ | $\mathcal{O}^g_{2+}$ | $\mathcal{O}^h_{1+}$ | $\mathcal{O}^h_{2-}$ |
| $(b,g,h):69$ | ${}^sR^{z'0}_{TT}$ | $R^{z'0}_{TT'}$ | ${}^cR^{x'0}_{LT'}$ | ${}^cR^{z'0}_{LT'}$ | ${}^cR^{z'x}_{LT}$ | ${}^cR^{x'x}_{LT}$ |
| | $\mathcal{O}^b_{1+}$ | $\mathcal{O}^b_{2+}$ | $\mathcal{O}^g_{1-}$ | $\mathcal{O}^g_{2+}$ | $\mathcal{O}^h_{1-}$ | $\mathcal{O}^h_{2+}$ |
| $(b,g,h):70$ | ${}^sR^{z'0}_{TT}$ | $R^{z'0}_{TT'}$ | ${}^cR^{x'0}_{LT'}$ | ${}^cR^{z'0}_{LT'}$ | ${}^cR^{z'x}_{LT}$ | ${}^sR^{z'x}_{LT'}$ |
| | $\mathcal{O}^b_{1+}$ | $\mathcal{O}^b_{2+}$ | $\mathcal{O}^g_{1-}$ | $\mathcal{O}^g_{2+}$ | $\mathcal{O}^h_{1-}$ | $\mathcal{O}^h_{2-}$ |
| $(b,g,h):71$ | ${}^sR^{z'0}_{TT}$ | $R^{z'0}_{TT'}$ | ${}^cR^{x'0}_{LT'}$ | ${}^sR^{x'0}_{LT}$ | ${}^sR^{x'x}_{LT'}$ | ${}^cR^{z'x}_{LT}$ |
| | $\mathcal{O}^b_{1+}$ | $\mathcal{O}^b_{2+}$ | $\mathcal{O}^g_{1-}$ | $\mathcal{O}^g_{2-}$ | $\mathcal{O}^h_{1+}$ | $\mathcal{O}^h_{1-}$ |
| $(b,g,h):72$ | ${}^sR^{z'0}_{TT}$ | $R^{z'0}_{TT'}$ | ${}^cR^{x'0}_{LT'}$ | ${}^sR^{x'0}_{LT}$ | ${}^cR^{x'x}_{LT}$ | ${}^sR^{z'x}_{LT'}$ |
| | $\mathcal{O}^b_{1+}$ | $\mathcal{O}^b_{2+}$ | $\mathcal{O}^g_{1-}$ | $\mathcal{O}^g_{2-}$ | $\mathcal{O}^h_{2+}$ | $\mathcal{O}^h_{2-}$ |
| $(b,g,h):73$ | ${}^sR^{z'0}_{TT}$ | $R^{z'0}_{TT'}$ | ${}^cR^{x'0}_{LT'}$ | ${}^sR^{x'0}_{LT}$ | ${}^sR^{x'x}_{LT'}$ | ${}^cR^{x'x}_{LT}$ |
| | $\mathcal{O}^b_{1+}$ | $\mathcal{O}^b_{2+}$ | $\mathcal{O}^g_{1-}$ | $\mathcal{O}^g_{2-}$ | $\mathcal{O}^h_{1+}$ | $\mathcal{O}^h_{2+}$ |
| $(b,g,h):74$ | ${}^sR^{z'0}_{TT}$ | $R^{z'0}_{TT'}$ | ${}^cR^{x'0}_{LT'}$ | ${}^sR^{x'0}_{LT}$ | ${}^sR^{x'x}_{LT'}$ | ${}^sR^{z'x}_{LT'}$ |
| | $\mathcal{O}^b_{1+}$ | $\mathcal{O}^b_{2+}$ | $\mathcal{O}^g_{1-}$ | $\mathcal{O}^g_{2-}$ | $\mathcal{O}^h_{1+}$ | $\mathcal{O}^h_{2-}$ |
| $(b,g,h):75$ | ${}^sR^{z'0}_{TT}$ | $R^{z'0}_{TT'}$ | ${}^cR^{x'0}_{LT'}$ | ${}^sR^{x'0}_{LT}$ | ${}^cR^{z'x}_{LT}$ | ${}^cR^{x'x}_{LT}$ |
| | $\mathcal{O}^b_{1+}$ | $\mathcal{O}^b_{2+}$ | $\mathcal{O}^g_{1-}$ | $\mathcal{O}^g_{2-}$ | $\mathcal{O}^h_{1-}$ | $\mathcal{O}^h_{2+}$ |
| $(b,g,h):76$ | ${}^sR^{z'0}_{TT}$ | $R^{z'0}_{TT'}$ | ${}^cR^{x'0}_{LT'}$ | ${}^sR^{x'0}_{LT}$ | ${}^cR^{z'x}_{LT}$ | ${}^sR^{z'x}_{LT'}$ |
| | $\mathcal{O}^b_{1+}$ | $\mathcal{O}^b_{2+}$ | $\mathcal{O}^g_{1-}$ | $\mathcal{O}^g_{2-}$ | $\mathcal{O}^h_{1-}$ | $\mathcal{O}^h_{2-}$ |

| | | | | | | |
|---|---|---|---|---|---|---|
| $(b,g,h):77$ | ${}^{s}R^{z'0}_{TT}$ | ${}^{s}R^{x'0}_{TT}$ | ${}^{s}R^{z'0}_{LT}$ | ${}^{c}R^{x'0}_{LT'}$ | ${}^{s}R^{x'x}_{LT'}$ | ${}^{c}R^{x'x}_{LT}$ |
| | $\mathcal{O}^{b}_{1+}$ | $\mathcal{O}^{b}_{2-}$ | $\mathcal{O}^{g}_{1+}$ | $\mathcal{O}^{g}_{1-}$ | $\mathcal{O}^{h}_{1+}$ | $\mathcal{O}^{h}_{2+}$ |
| $(b,g,h):78$ | ${}^{s}R^{z'0}_{TT}$ | ${}^{s}R^{x'0}_{TT}$ | ${}^{s}R^{z'0}_{LT}$ | ${}^{c}R^{x'0}_{LT'}$ | ${}^{c}R^{z'x}_{LT}$ | ${}^{s}R^{z'x}_{LT'}$ |
| | $\mathcal{O}^{b}_{1+}$ | $\mathcal{O}^{b}_{2-}$ | $\mathcal{O}^{g}_{1+}$ | $\mathcal{O}^{g}_{1-}$ | $\mathcal{O}^{h}_{1-}$ | $\mathcal{O}^{h}_{2-}$ |
| $(b,g,h):79$ | ${}^{s}R^{z'0}_{TT}$ | ${}^{s}R^{x'0}_{TT}$ | ${}^{c}R^{z'0}_{LT'}$ | ${}^{s}R^{x'0}_{LT}$ | ${}^{s}R^{x'x}_{LT'}$ | ${}^{c}R^{x'x}_{LT}$ |
| | $\mathcal{O}^{b}_{1+}$ | $\mathcal{O}^{b}_{2-}$ | $\mathcal{O}^{g}_{2+}$ | $\mathcal{O}^{g}_{2-}$ | $\mathcal{O}^{h}_{1+}$ | $\mathcal{O}^{h}_{2+}$ |
| $(b,g,h):80$ | ${}^{s}R^{z'0}_{TT}$ | ${}^{s}R^{x'0}_{TT}$ | ${}^{c}R^{z'0}_{LT'}$ | ${}^{s}R^{x'0}_{LT}$ | ${}^{c}R^{z'x}_{LT}$ | ${}^{s}R^{z'x}_{LT'}$ |
| | $\mathcal{O}^{b}_{1+}$ | $\mathcal{O}^{b}_{2-}$ | $\mathcal{O}^{g}_{2+}$ | $\mathcal{O}^{g}_{2-}$ | $\mathcal{O}^{h}_{1-}$ | $\mathcal{O}^{h}_{2-}$ |
| $(b,g,h):81$ | ${}^{s}R^{z'0}_{TT}$ | ${}^{s}R^{x'0}_{TT}$ | ${}^{s}R^{z'0}_{LT}$ | ${}^{c}R^{z'0}_{LT'}$ | ${}^{s}R^{x'x}_{LT'}$ | ${}^{c}R^{z'x}_{LT}$ |
| | $\mathcal{O}^{b}_{1+}$ | $\mathcal{O}^{b}_{2-}$ | $\mathcal{O}^{g}_{1+}$ | $\mathcal{O}^{g}_{2+}$ | $\mathcal{O}^{h}_{1+}$ | $\mathcal{O}^{h}_{1-}$ |
| $(b,g,h):82$ | ${}^{s}R^{z'0}_{TT}$ | ${}^{s}R^{x'0}_{TT}$ | ${}^{s}R^{z'0}_{LT}$ | ${}^{c}R^{z'0}_{LT'}$ | ${}^{c}R^{x'x}_{LT}$ | ${}^{s}R^{z'x}_{LT'}$ |
| | $\mathcal{O}^{b}_{1+}$ | $\mathcal{O}^{b}_{2-}$ | $\mathcal{O}^{g}_{1+}$ | $\mathcal{O}^{g}_{2+}$ | $\mathcal{O}^{h}_{2+}$ | $\mathcal{O}^{h}_{2-}$ |
| $(b,g,h):83$ | ${}^{s}R^{z'0}_{TT}$ | ${}^{s}R^{x'0}_{TT}$ | ${}^{s}R^{z'0}_{LT}$ | ${}^{c}R^{z'0}_{LT'}$ | ${}^{s}R^{x'x}_{LT'}$ | ${}^{c}R^{x'x}_{LT}$ |
| | $\mathcal{O}^{b}_{1+}$ | $\mathcal{O}^{b}_{2-}$ | $\mathcal{O}^{g}_{1+}$ | $\mathcal{O}^{g}_{2+}$ | $\mathcal{O}^{h}_{1+}$ | $\mathcal{O}^{h}_{2+}$ |
| $(b,g,h):84$ | ${}^{s}R^{z'0}_{TT}$ | ${}^{s}R^{x'0}_{TT}$ | ${}^{s}R^{z'0}_{LT}$ | ${}^{c}R^{z'0}_{LT'}$ | ${}^{s}R^{x'x}_{LT'}$ | ${}^{s}R^{z'x}_{LT'}$ |
| | $\mathcal{O}^{b}_{1+}$ | $\mathcal{O}^{b}_{2-}$ | $\mathcal{O}^{g}_{1+}$ | $\mathcal{O}^{g}_{2+}$ | $\mathcal{O}^{h}_{1+}$ | $\mathcal{O}^{h}_{2-}$ |
| $(b,g,h):85$ | ${}^{s}R^{z'0}_{TT}$ | ${}^{s}R^{x'0}_{TT}$ | ${}^{s}R^{z'0}_{LT}$ | ${}^{c}R^{z'0}_{LT'}$ | ${}^{c}R^{z'x}_{LT}$ | ${}^{c}R^{x'x}_{LT}$ |
| | $\mathcal{O}^{b}_{1+}$ | $\mathcal{O}^{b}_{2-}$ | $\mathcal{O}^{g}_{1+}$ | $\mathcal{O}^{g}_{2+}$ | $\mathcal{O}^{h}_{1-}$ | $\mathcal{O}^{h}_{2+}$ |
| $(b,g,h):86$ | ${}^{s}R^{z'0}_{TT}$ | ${}^{s}R^{x'0}_{TT}$ | ${}^{s}R^{z'0}_{LT}$ | ${}^{c}R^{z'0}_{LT'}$ | ${}^{c}R^{z'x}_{LT}$ | ${}^{s}R^{z'x}_{LT'}$ |
| | $\mathcal{O}^{b}_{1+}$ | $\mathcal{O}^{b}_{2-}$ | $\mathcal{O}^{g}_{1+}$ | $\mathcal{O}^{g}_{2+}$ | $\mathcal{O}^{h}_{1-}$ | $\mathcal{O}^{h}_{2-}$ |
| $(b,g,h):87$ | ${}^{s}R^{z'0}_{TT}$ | ${}^{s}R^{x'0}_{TT}$ | ${}^{s}R^{z'0}_{LT}$ | ${}^{s}R^{x'0}_{LT}$ | ${}^{s}R^{x'x}_{LT'}$ | ${}^{c}R^{x'x}_{LT}$ |
| | $\mathcal{O}^{b}_{1+}$ | $\mathcal{O}^{b}_{2-}$ | $\mathcal{O}^{g}_{1+}$ | $\mathcal{O}^{g}_{2-}$ | $\mathcal{O}^{h}_{1+}$ | $\mathcal{O}^{h}_{2+}$ |
| $(b,g,h):88$ | ${}^{s}R^{z'0}_{TT}$ | ${}^{s}R^{x'0}_{TT}$ | ${}^{s}R^{z'0}_{LT}$ | ${}^{s}R^{x'0}_{LT}$ | ${}^{c}R^{z'x}_{LT}$ | ${}^{s}R^{z'x}_{LT'}$ |
| | $\mathcal{O}^{b}_{1+}$ | $\mathcal{O}^{b}_{2-}$ | $\mathcal{O}^{g}_{1+}$ | $\mathcal{O}^{g}_{2-}$ | $\mathcal{O}^{h}_{1-}$ | $\mathcal{O}^{h}_{2-}$ |
| $(b,g,h):89$ | ${}^{s}R^{z'0}_{TT}$ | ${}^{s}R^{x'0}_{TT}$ | ${}^{c}R^{x'0}_{LT'}$ | ${}^{c}R^{z'0}_{LT'}$ | ${}^{s}R^{x'x}_{LT'}$ | ${}^{c}R^{x'x}_{LT}$ |
| | $\mathcal{O}^{b}_{1+}$ | $\mathcal{O}^{b}_{2-}$ | $\mathcal{O}^{g}_{1-}$ | $\mathcal{O}^{g}_{2+}$ | $\mathcal{O}^{h}_{1+}$ | $\mathcal{O}^{h}_{2+}$ |
| $(b,g,h):90$ | ${}^{s}R^{z'0}_{TT}$ | ${}^{s}R^{x'0}_{TT}$ | ${}^{c}R^{x'0}_{LT'}$ | ${}^{c}R^{z'0}_{LT'}$ | ${}^{c}R^{z'x}_{LT}$ | ${}^{s}R^{z'x}_{LT'}$ |
| | $\mathcal{O}^{b}_{1+}$ | $\mathcal{O}^{b}_{2-}$ | $\mathcal{O}^{g}_{1-}$ | $\mathcal{O}^{g}_{2+}$ | $\mathcal{O}^{h}_{1-}$ | $\mathcal{O}^{h}_{2-}$ |
| $(b,g,h):91$ | ${}^{s}R^{z'0}_{TT}$ | ${}^{s}R^{x'0}_{TT}$ | ${}^{c}R^{x'0}_{LT'}$ | ${}^{s}R^{x'0}_{LT}$ | ${}^{s}R^{x'x}_{LT'}$ | ${}^{c}R^{z'x}_{LT}$ |
| | $\mathcal{O}^{b}_{1+}$ | $\mathcal{O}^{b}_{2-}$ | $\mathcal{O}^{g}_{1-}$ | $\mathcal{O}^{g}_{2-}$ | $\mathcal{O}^{h}_{1+}$ | $\mathcal{O}^{h}_{1-}$ |
| $(b,g,h):92$ | ${}^{s}R^{z'0}_{TT}$ | ${}^{s}R^{x'0}_{TT}$ | ${}^{c}R^{x'0}_{LT'}$ | ${}^{s}R^{x'0}_{LT}$ | ${}^{c}R^{x'x}_{LT}$ | ${}^{s}R^{z'x}_{LT'}$ |
| | $\mathcal{O}^{b}_{1+}$ | $\mathcal{O}^{b}_{2-}$ | $\mathcal{O}^{g}_{1-}$ | $\mathcal{O}^{g}_{2-}$ | $\mathcal{O}^{h}_{2+}$ | $\mathcal{O}^{h}_{2-}$ |
| $(b,g,h):93$ | ${}^{s}R^{z'0}_{TT}$ | ${}^{s}R^{x'0}_{TT}$ | ${}^{c}R^{x'0}_{LT'}$ | ${}^{s}R^{x'0}_{LT}$ | ${}^{s}R^{x'x}_{LT'}$ | ${}^{c}R^{x'x}_{LT}$ |
| | $\mathcal{O}^{b}_{1+}$ | $\mathcal{O}^{b}_{2-}$ | $\mathcal{O}^{g}_{1-}$ | $\mathcal{O}^{g}_{2-}$ | $\mathcal{O}^{h}_{1+}$ | $\mathcal{O}^{h}_{2+}$ |
| $(b,g,h):94$ | ${}^{s}R^{z'0}_{TT}$ | ${}^{s}R^{x'0}_{TT}$ | ${}^{c}R^{x'0}_{LT'}$ | ${}^{s}R^{x'0}_{LT}$ | ${}^{s}R^{x'x}_{LT'}$ | ${}^{s}R^{z'x}_{LT'}$ |
| | $\mathcal{O}^{b}_{1+}$ | $\mathcal{O}^{b}_{2-}$ | $\mathcal{O}^{g}_{1-}$ | $\mathcal{O}^{g}_{2-}$ | $\mathcal{O}^{h}_{1+}$ | $\mathcal{O}^{h}_{2-}$ |
| $(b,g,h):95$ | ${}^{s}R^{z'0}_{TT}$ | ${}^{s}R^{x'0}_{TT}$ | ${}^{c}R^{x'0}_{LT'}$ | ${}^{s}R^{x'0}_{LT}$ | ${}^{c}R^{z'x}_{LT}$ | ${}^{c}R^{x'x}_{LT}$ |
| | $\mathcal{O}^{b}_{1+}$ | $\mathcal{O}^{b}_{2-}$ | $\mathcal{O}^{g}_{1-}$ | $\mathcal{O}^{g}_{2-}$ | $\mathcal{O}^{h}_{1-}$ | $\mathcal{O}^{h}_{2+}$ |
| $(b,g,h):96$ | ${}^{s}R^{z'0}_{TT}$ | ${}^{s}R^{x'0}_{TT}$ | ${}^{c}R^{x'0}_{LT'}$ | ${}^{s}R^{x'0}_{LT}$ | ${}^{c}R^{z'x}_{LT}$ | ${}^{s}R^{z'x}_{LT'}$ |
| | $\mathcal{O}^{b}_{1+}$ | $\mathcal{O}^{b}_{2-}$ | $\mathcal{O}^{g}_{1-}$ | $\mathcal{O}^{g}_{2-}$ | $\mathcal{O}^{h}_{1-}$ | $\mathcal{O}^{h}_{2-}$ |
| $(b,g,h):97$ | $R^{x'0}_{TT'}$ | $R^{z'0}_{TT'}$ | ${}^{s}R^{z'0}_{LT}$ | ${}^{c}R^{x'0}_{LT'}$ | ${}^{s}R^{x'x}_{LT'}$ | ${}^{c}R^{x'x}_{LT}$ |
| | $\mathcal{O}^{b}_{1-}$ | $\mathcal{O}^{b}_{2+}$ | $\mathcal{O}^{g}_{1+}$ | $\mathcal{O}^{g}_{1-}$ | $\mathcal{O}^{h}_{1+}$ | $\mathcal{O}^{h}_{2+}$ |
| $(b,g,h):98$ | $R^{x'0}_{TT'}$ | $R^{z'0}_{TT'}$ | ${}^{s}R^{z'0}_{LT}$ | ${}^{c}R^{x'0}_{LT'}$ | ${}^{c}R^{z'x}_{LT}$ | ${}^{s}R^{z'x}_{LT'}$ |
| | $\mathcal{O}^{b}_{1-}$ | $\mathcal{O}^{b}_{2+}$ | $\mathcal{O}^{g}_{1+}$ | $\mathcal{O}^{g}_{1-}$ | $\mathcal{O}^{h}_{1-}$ | $\mathcal{O}^{h}_{2-}$ |
| $(b,g,h):99$ | $R^{x'0}_{TT'}$ | $R^{z'0}_{TT'}$ | ${}^{c}R^{z'0}_{LT'}$ | ${}^{s}R^{x'0}_{LT}$ | ${}^{s}R^{x'x}_{LT'}$ | ${}^{c}R^{x'x}_{LT}$ |
| | $\mathcal{O}^{b}_{1-}$ | $\mathcal{O}^{b}_{2+}$ | $\mathcal{O}^{g}_{2+}$ | $\mathcal{O}^{g}_{2-}$ | $\mathcal{O}^{h}_{1+}$ | $\mathcal{O}^{h}_{2+}$ |
| $(b,g,h):100$ | $R^{x'0}_{TT'}$ | $R^{z'0}_{TT'}$ | ${}^{c}R^{z'0}_{LT'}$ | ${}^{s}R^{x'0}_{LT}$ | ${}^{c}R^{z'x}_{LT}$ | ${}^{s}R^{z'x}_{LT'}$ |
| | $\mathcal{O}^{b}_{1-}$ | $\mathcal{O}^{b}_{2+}$ | $\mathcal{O}^{g}_{2+}$ | $\mathcal{O}^{g}_{2-}$ | $\mathcal{O}^{h}_{1-}$ | $\mathcal{O}^{h}_{2-}$ |
| $(b,g,h):101$ | $R^{x'0}_{TT'}$ | $R^{z'0}_{TT'}$ | ${}^{s}R^{z'0}_{LT}$ | ${}^{c}R^{z'0}_{LT'}$ | ${}^{s}R^{x'x}_{LT'}$ | ${}^{c}R^{z'x}_{LT}$ |
| | $\mathcal{O}^{b}_{1-}$ | $\mathcal{O}^{b}_{2+}$ | $\mathcal{O}^{g}_{1+}$ | $\mathcal{O}^{g}_{2+}$ | $\mathcal{O}^{h}_{1+}$ | $\mathcal{O}^{h}_{1-}$ |
| $(b,g,h):102$ | $R^{x'0}_{TT'}$ | $R^{z'0}_{TT'}$ | ${}^{s}R^{z'0}_{LT}$ | ${}^{c}R^{z'0}_{LT'}$ | ${}^{c}R^{x'x}_{LT}$ | ${}^{s}R^{z'x}_{LT'}$ |
| | $\mathcal{O}^{b}_{1-}$ | $\mathcal{O}^{b}_{2+}$ | $\mathcal{O}^{g}_{1+}$ | $\mathcal{O}^{g}_{2+}$ | $\mathcal{O}^{h}_{2+}$ | $\mathcal{O}^{h}_{2-}$ |
| $(b,g,h):103$ | $R^{x'0}_{TT'}$ | $R^{z'0}_{TT'}$ | ${}^{s}R^{z'0}_{LT}$ | ${}^{c}R^{z'0}_{LT'}$ | ${}^{s}R^{x'x}_{LT'}$ | ${}^{c}R^{x'x}_{LT}$ |
| | $\mathcal{O}^{b}_{1-}$ | $\mathcal{O}^{b}_{2+}$ | $\mathcal{O}^{g}_{1+}$ | $\mathcal{O}^{g}_{2+}$ | $\mathcal{O}^{h}_{1+}$ | $\mathcal{O}^{h}_{2+}$ |
| $(b,g,h):104$ | $R^{x'0}_{TT'}$ | $R^{z'0}_{TT'}$ | ${}^{s}R^{z'0}_{LT}$ | ${}^{c}R^{z'0}_{LT'}$ | ${}^{s}R^{x'x}_{LT'}$ | ${}^{s}R^{z'x}_{LT'}$ |
| | $\mathcal{O}^{b}_{1-}$ | $\mathcal{O}^{b}_{2+}$ | $\mathcal{O}^{g}_{1+}$ | $\mathcal{O}^{g}_{2+}$ | $\mathcal{O}^{h}_{1+}$ | $\mathcal{O}^{h}_{2-}$ |

| | | | | | | |
|---|---|---|---|---|---|---|
| $(b,g,h):105$ | $R^{x'0}_{TT'}$ | $R^{z'0}_{TT'}$ | ${}^{s}R^{z'0}_{LT}$ | ${}^{c}R^{z'0}_{LT'}$ | ${}^{c}R^{z'x}_{LT}$ | ${}^{c}R^{x'x}_{LT}$ |
| | $\mathcal{O}^{b}_{1-}$ | $\mathcal{O}^{b}_{2+}$ | $\mathcal{O}^{g}_{1+}$ | $\mathcal{O}^{g}_{2+}$ | $\mathcal{O}^{h}_{1-}$ | $\mathcal{O}^{h}_{2+}$ |
| $(b,g,h):106$ | $R^{x'0}_{TT'}$ | $R^{z'0}_{TT'}$ | ${}^{s}R^{z'0}_{LT}$ | ${}^{c}R^{z'0}_{LT'}$ | ${}^{c}R^{z'x}_{LT}$ | ${}^{s}R^{z'x}_{LT'}$ |
| | $\mathcal{O}^{b}_{1-}$ | $\mathcal{O}^{b}_{2+}$ | $\mathcal{O}^{g}_{1+}$ | $\mathcal{O}^{g}_{2+}$ | $\mathcal{O}^{h}_{1-}$ | $\mathcal{O}^{h}_{2-}$ |
| $(b,g,h):107$ | $R^{x'0}_{TT'}$ | $R^{z'0}_{TT'}$ | ${}^{s}R^{z'0}_{LT}$ | ${}^{s}R^{x'0}_{LT}$ | ${}^{s}R^{x'x}_{LT'}$ | ${}^{c}R^{x'x}_{LT}$ |
| | $\mathcal{O}^{b}_{1-}$ | $\mathcal{O}^{b}_{2+}$ | $\mathcal{O}^{g}_{1+}$ | $\mathcal{O}^{g}_{2-}$ | $\mathcal{O}^{h}_{1+}$ | $\mathcal{O}^{h}_{2+}$ |
| $(b,g,h):108$ | $R^{x'0}_{TT'}$ | $R^{z'0}_{TT'}$ | ${}^{s}R^{z'0}_{LT}$ | ${}^{s}R^{x'0}_{LT}$ | ${}^{c}R^{z'x}_{LT}$ | ${}^{s}R^{z'x}_{LT'}$ |
| | $\mathcal{O}^{b}_{1-}$ | $\mathcal{O}^{b}_{2+}$ | $\mathcal{O}^{g}_{1+}$ | $\mathcal{O}^{g}_{2-}$ | $\mathcal{O}^{h}_{1-}$ | $\mathcal{O}^{h}_{2-}$ |
| $(b,g,h):109$ | $R^{x'0}_{TT'}$ | $R^{z'0}_{TT'}$ | ${}^{c}R^{x'0}_{LT'}$ | ${}^{c}R^{z'0}_{LT'}$ | ${}^{s}R^{x'x}_{LT'}$ | ${}^{c}R^{x'x}_{LT}$ |
| | $\mathcal{O}^{b}_{1-}$ | $\mathcal{O}^{b}_{2+}$ | $\mathcal{O}^{g}_{1-}$ | $\mathcal{O}^{g}_{2+}$ | $\mathcal{O}^{h}_{1+}$ | $\mathcal{O}^{h}_{2+}$ |
| $(b,g,h):110$ | $R^{x'0}_{TT'}$ | $R^{z'0}_{TT'}$ | ${}^{c}R^{x'0}_{LT'}$ | ${}^{c}R^{z'0}_{LT'}$ | ${}^{c}R^{z'x}_{LT}$ | ${}^{s}R^{z'x}_{LT'}$ |
| | $\mathcal{O}^{b}_{1-}$ | $\mathcal{O}^{b}_{2+}$ | $\mathcal{O}^{g}_{1-}$ | $\mathcal{O}^{g}_{2+}$ | $\mathcal{O}^{h}_{1-}$ | $\mathcal{O}^{h}_{2-}$ |
| $(b,g,h):111$ | $R^{x'0}_{TT'}$ | $R^{z'0}_{TT'}$ | ${}^{c}R^{x'0}_{LT'}$ | ${}^{s}R^{x'0}_{LT}$ | ${}^{s}R^{x'x}_{LT'}$ | ${}^{c}R^{z'x}_{LT}$ |
| | $\mathcal{O}^{b}_{1-}$ | $\mathcal{O}^{b}_{2+}$ | $\mathcal{O}^{g}_{1-}$ | $\mathcal{O}^{g}_{2-}$ | $\mathcal{O}^{h}_{1+}$ | $\mathcal{O}^{h}_{1-}$ |
| $(b,g,h):112$ | $R^{x'0}_{TT'}$ | $R^{z'0}_{TT'}$ | ${}^{c}R^{x'0}_{LT'}$ | ${}^{s}R^{x'0}_{LT}$ | ${}^{c}R^{x'x}_{LT}$ | ${}^{s}R^{z'x}_{LT'}$ |
| | $\mathcal{O}^{b}_{1-}$ | $\mathcal{O}^{b}_{2+}$ | $\mathcal{O}^{g}_{1-}$ | $\mathcal{O}^{g}_{2-}$ | $\mathcal{O}^{h}_{2+}$ | $\mathcal{O}^{h}_{2-}$ |
| $(b,g,h):113$ | $R^{x'0}_{TT'}$ | $R^{z'0}_{TT'}$ | ${}^{c}R^{x'0}_{LT'}$ | ${}^{s}R^{x'0}_{LT}$ | ${}^{s}R^{x'x}_{LT'}$ | ${}^{c}R^{x'x}_{LT}$ |
| | $\mathcal{O}^{b}_{1-}$ | $\mathcal{O}^{b}_{2+}$ | $\mathcal{O}^{g}_{1-}$ | $\mathcal{O}^{g}_{2-}$ | $\mathcal{O}^{h}_{1+}$ | $\mathcal{O}^{h}_{2+}$ |
| $(b,g,h):114$ | $R^{x'0}_{TT'}$ | $R^{z'0}_{TT'}$ | ${}^{c}R^{x'0}_{LT'}$ | ${}^{s}R^{x'0}_{LT}$ | ${}^{s}R^{x'x}_{LT'}$ | ${}^{s}R^{z'x}_{LT'}$ |
| | $\mathcal{O}^{b}_{1-}$ | $\mathcal{O}^{b}_{2+}$ | $\mathcal{O}^{g}_{1-}$ | $\mathcal{O}^{g}_{2-}$ | $\mathcal{O}^{h}_{1+}$ | $\mathcal{O}^{h}_{2-}$ |
| $(b,g,h):115$ | $R^{x'0}_{TT'}$ | $R^{z'0}_{TT'}$ | ${}^{c}R^{x'0}_{LT'}$ | ${}^{s}R^{x'0}_{LT}$ | ${}^{c}R^{z'x}_{LT}$ | ${}^{c}R^{x'x}_{LT}$ |
| | $\mathcal{O}^{b}_{1-}$ | $\mathcal{O}^{b}_{2+}$ | $\mathcal{O}^{g}_{1-}$ | $\mathcal{O}^{g}_{2-}$ | $\mathcal{O}^{h}_{1-}$ | $\mathcal{O}^{h}_{2+}$ |
| $(b,g,h):116$ | $R^{x'0}_{TT'}$ | $R^{z'0}_{TT'}$ | ${}^{c}R^{x'0}_{LT'}$ | ${}^{s}R^{x'0}_{LT}$ | ${}^{c}R^{z'x}_{LT}$ | ${}^{s}R^{z'x}_{LT'}$ |
| | $\mathcal{O}^{b}_{1-}$ | $\mathcal{O}^{b}_{2+}$ | $\mathcal{O}^{g}_{1-}$ | $\mathcal{O}^{g}_{2-}$ | $\mathcal{O}^{h}_{1-}$ | $\mathcal{O}^{h}_{2-}$ |
| $(b,g,h):117$ | $R^{x'0}_{TT'}$ | ${}^{s}R^{x'0}_{TT}$ | ${}^{s}R^{z'0}_{LT}$ | ${}^{c}R^{x'0}_{LT'}$ | ${}^{s}R^{x'x}_{LT'}$ | ${}^{c}R^{z'x}_{LT}$ |
| | $\mathcal{O}^{b}_{1-}$ | $\mathcal{O}^{b}_{2-}$ | $\mathcal{O}^{g}_{1+}$ | $\mathcal{O}^{g}_{1-}$ | $\mathcal{O}^{h}_{1+}$ | $\mathcal{O}^{h}_{1-}$ |
| $(b,g,h):118$ | $R^{x'0}_{TT'}$ | ${}^{s}R^{x'0}_{TT}$ | ${}^{s}R^{z'0}_{LT}$ | ${}^{c}R^{x'0}_{LT'}$ | ${}^{c}R^{x'x}_{LT}$ | ${}^{s}R^{z'x}_{LT'}$ |
| | $\mathcal{O}^{b}_{1-}$ | $\mathcal{O}^{b}_{2-}$ | $\mathcal{O}^{g}_{1+}$ | $\mathcal{O}^{g}_{1-}$ | $\mathcal{O}^{h}_{2+}$ | $\mathcal{O}^{h}_{2-}$ |
| $(b,g,h):119$ | $R^{x'0}_{TT'}$ | ${}^{s}R^{x'0}_{TT}$ | ${}^{s}R^{z'0}_{LT}$ | ${}^{c}R^{x'0}_{LT'}$ | ${}^{s}R^{x'x}_{LT'}$ | ${}^{c}R^{x'x}_{LT}$ |
| | $\mathcal{O}^{b}_{1-}$ | $\mathcal{O}^{b}_{2-}$ | $\mathcal{O}^{g}_{1+}$ | $\mathcal{O}^{g}_{1-}$ | $\mathcal{O}^{h}_{1+}$ | $\mathcal{O}^{h}_{2+}$ |
| $(b,g,h):120$ | $R^{x'0}_{TT'}$ | ${}^{s}R^{x'0}_{TT}$ | ${}^{s}R^{z'0}_{LT}$ | ${}^{c}R^{x'0}_{LT'}$ | ${}^{s}R^{x'x}_{LT'}$ | ${}^{s}R^{z'x}_{LT'}$ |
| | $\mathcal{O}^{b}_{1-}$ | $\mathcal{O}^{b}_{2-}$ | $\mathcal{O}^{g}_{1+}$ | $\mathcal{O}^{g}_{1-}$ | $\mathcal{O}^{h}_{1+}$ | $\mathcal{O}^{h}_{2-}$ |
| $(b,g,h):121$ | $R^{x'0}_{TT'}$ | ${}^{s}R^{x'0}_{TT}$ | ${}^{s}R^{z'0}_{LT}$ | ${}^{c}R^{x'0}_{LT'}$ | ${}^{c}R^{z'x}_{LT}$ | ${}^{c}R^{x'x}_{LT}$ |
| | $\mathcal{O}^{b}_{1-}$ | $\mathcal{O}^{b}_{2-}$ | $\mathcal{O}^{g}_{1+}$ | $\mathcal{O}^{g}_{1-}$ | $\mathcal{O}^{h}_{1-}$ | $\mathcal{O}^{h}_{2+}$ |
| $(b,g,h):122$ | $R^{x'0}_{TT'}$ | ${}^{s}R^{x'0}_{TT}$ | ${}^{s}R^{z'0}_{LT}$ | ${}^{c}R^{x'0}_{LT'}$ | ${}^{c}R^{z'x}_{LT}$ | ${}^{s}R^{z'x}_{LT'}$ |
| | $\mathcal{O}^{b}_{1-}$ | $\mathcal{O}^{b}_{2-}$ | $\mathcal{O}^{g}_{1+}$ | $\mathcal{O}^{g}_{1-}$ | $\mathcal{O}^{h}_{1-}$ | $\mathcal{O}^{h}_{2-}$ |
| $(b,g,h):123$ | $R^{x'0}_{TT'}$ | ${}^{s}R^{x'0}_{TT}$ | ${}^{c}R^{z'0}_{LT'}$ | ${}^{s}R^{x'0}_{LT}$ | ${}^{s}R^{x'x}_{LT'}$ | ${}^{c}R^{z'x}_{LT}$ |
| | $\mathcal{O}^{b}_{1-}$ | $\mathcal{O}^{b}_{2-}$ | $\mathcal{O}^{g}_{2+}$ | $\mathcal{O}^{g}_{2-}$ | $\mathcal{O}^{h}_{1+}$ | $\mathcal{O}^{h}_{1-}$ |
| $(b,g,h):124$ | $R^{x'0}_{TT'}$ | ${}^{s}R^{x'0}_{TT}$ | ${}^{c}R^{z'0}_{LT'}$ | ${}^{s}R^{x'0}_{LT}$ | ${}^{c}R^{x'x}_{LT}$ | ${}^{s}R^{z'x}_{LT'}$ |
| | $\mathcal{O}^{b}_{1-}$ | $\mathcal{O}^{b}_{2-}$ | $\mathcal{O}^{g}_{2+}$ | $\mathcal{O}^{g}_{2-}$ | $\mathcal{O}^{h}_{2+}$ | $\mathcal{O}^{h}_{2-}$ |
| $(b,g,h):125$ | $R^{x'0}_{TT'}$ | ${}^{s}R^{x'0}_{TT}$ | ${}^{c}R^{z'0}_{LT'}$ | ${}^{s}R^{x'0}_{LT}$ | ${}^{s}R^{x'x}_{LT'}$ | ${}^{c}R^{x'x}_{LT}$ |
| | $\mathcal{O}^{b}_{1-}$ | $\mathcal{O}^{b}_{2-}$ | $\mathcal{O}^{g}_{2+}$ | $\mathcal{O}^{g}_{2-}$ | $\mathcal{O}^{h}_{1+}$ | $\mathcal{O}^{h}_{2+}$ |
| $(b,g,h):126$ | $R^{x'0}_{TT'}$ | ${}^{s}R^{x'0}_{TT}$ | ${}^{c}R^{z'0}_{LT'}$ | ${}^{s}R^{x'0}_{LT}$ | ${}^{s}R^{x'x}_{LT'}$ | ${}^{s}R^{z'x}_{LT'}$ |
| | $\mathcal{O}^{b}_{1-}$ | $\mathcal{O}^{b}_{2-}$ | $\mathcal{O}^{g}_{2+}$ | $\mathcal{O}^{g}_{2-}$ | $\mathcal{O}^{h}_{1+}$ | $\mathcal{O}^{h}_{2-}$ |
| $(b,g,h):127$ | $R^{x'0}_{TT'}$ | ${}^{s}R^{x'0}_{TT}$ | ${}^{c}R^{z'0}_{LT'}$ | ${}^{s}R^{x'0}_{LT}$ | ${}^{c}R^{z'x}_{LT}$ | ${}^{c}R^{x'x}_{LT}$ |
| | $\mathcal{O}^{b}_{1-}$ | $\mathcal{O}^{b}_{2-}$ | $\mathcal{O}^{g}_{2+}$ | $\mathcal{O}^{g}_{2-}$ | $\mathcal{O}^{h}_{1-}$ | $\mathcal{O}^{h}_{2+}$ |
| $(b,g,h):128$ | $R^{x'0}_{TT'}$ | ${}^{s}R^{x'0}_{TT}$ | ${}^{c}R^{z'0}_{LT'}$ | ${}^{s}R^{x'0}_{LT}$ | ${}^{c}R^{z'x}_{LT}$ | ${}^{s}R^{z'x}_{LT'}$ |
| | $\mathcal{O}^{b}_{1-}$ | $\mathcal{O}^{b}_{2-}$ | $\mathcal{O}^{g}_{2+}$ | $\mathcal{O}^{g}_{2-}$ | $\mathcal{O}^{h}_{1-}$ | $\mathcal{O}^{h}_{2-}$ |
| $(b,g,h):129$ | $R^{x'0}_{TT'}$ | ${}^{s}R^{x'0}_{TT}$ | ${}^{s}R^{z'0}_{LT}$ | ${}^{c}R^{z'0}_{LT'}$ | ${}^{s}R^{x'x}_{LT'}$ | ${}^{c}R^{z'x}_{LT}$ |
| | $\mathcal{O}^{b}_{1-}$ | $\mathcal{O}^{b}_{2-}$ | $\mathcal{O}^{g}_{1+}$ | $\mathcal{O}^{g}_{2+}$ | $\mathcal{O}^{h}_{1+}$ | $\mathcal{O}^{h}_{1-}$ |
| $(b,g,h):130$ | $R^{x'0}_{TT'}$ | ${}^{s}R^{x'0}_{TT}$ | ${}^{s}R^{z'0}_{LT}$ | ${}^{c}R^{z'0}_{LT'}$ | ${}^{c}R^{x'x}_{LT}$ | ${}^{s}R^{z'x}_{LT'}$ |
| | $\mathcal{O}^{b}_{1-}$ | $\mathcal{O}^{b}_{2-}$ | $\mathcal{O}^{g}_{1+}$ | $\mathcal{O}^{g}_{2+}$ | $\mathcal{O}^{h}_{2+}$ | $\mathcal{O}^{h}_{2-}$ |
| $(b,g,h):131$ | $R^{x'0}_{TT'}$ | ${}^{s}R^{x'0}_{TT}$ | ${}^{s}R^{z'0}_{LT}$ | ${}^{c}R^{z'0}_{LT'}$ | ${}^{s}R^{x'x}_{LT'}$ | ${}^{c}R^{x'x}_{LT}$ |
| | $\mathcal{O}^{b}_{1-}$ | $\mathcal{O}^{b}_{2-}$ | $\mathcal{O}^{g}_{1+}$ | $\mathcal{O}^{g}_{2+}$ | $\mathcal{O}^{h}_{1+}$ | $\mathcal{O}^{h}_{2+}$ |
| $(b,g,h):132$ | $R^{x'0}_{TT'}$ | ${}^{s}R^{x'0}_{TT}$ | ${}^{s}R^{z'0}_{LT}$ | ${}^{c}R^{z'0}_{LT'}$ | ${}^{s}R^{x'x}_{LT'}$ | ${}^{s}R^{z'x}_{LT'}$ |
| | $\mathcal{O}^{b}_{1-}$ | $\mathcal{O}^{b}_{2-}$ | $\mathcal{O}^{g}_{1+}$ | $\mathcal{O}^{g}_{2+}$ | $\mathcal{O}^{h}_{1+}$ | $\mathcal{O}^{h}_{2-}$ |

| | | | | | | |
|---|---|---|---|---|---|---|
| $(b,g,h):133$ | $R_{TT'}^{x'0}$ | ${}^{s}R_{TT}^{x'0}$ | ${}^{s}R_{LT}^{z'0}$ | ${}^{c}R_{LT'}^{z'0}$ | ${}^{c}R_{LT}^{z'x}$ | ${}^{c}R_{LT}^{x'x}$ |
| | $\mathcal{O}_{1-}^{b}$ | $\mathcal{O}_{2-}^{b}$ | $\mathcal{O}_{1+}^{g}$ | $\mathcal{O}_{2+}^{g}$ | $\mathcal{O}_{1-}^{h}$ | $\mathcal{O}_{2+}^{h}$ |
| $(b,g,h):134$ | $R_{TT'}^{x'0}$ | ${}^{s}R_{TT}^{x'0}$ | ${}^{s}R_{LT}^{z'0}$ | ${}^{c}R_{LT'}^{z'0}$ | ${}^{c}R_{LT}^{z'x}$ | ${}^{s}R_{LT'}^{z'x}$ |
| | $\mathcal{O}_{1-}^{b}$ | $\mathcal{O}_{2-}^{b}$ | $\mathcal{O}_{1+}^{g}$ | $\mathcal{O}_{2+}^{g}$ | $\mathcal{O}_{1-}^{h}$ | $\mathcal{O}_{2-}^{h}$ |
| $(b,g,h):135$ | $R_{TT'}^{x'0}$ | ${}^{s}R_{TT}^{x'0}$ | ${}^{s}R_{LT}^{z'0}$ | ${}^{s}R_{LT}^{x'0}$ | ${}^{s}R_{LT'}^{x'x}$ | ${}^{c}R_{LT}^{z'x}$ |
| | $\mathcal{O}_{1-}^{b}$ | $\mathcal{O}_{2-}^{b}$ | $\mathcal{O}_{1+}^{g}$ | $\mathcal{O}_{2-}^{g}$ | $\mathcal{O}_{1+}^{h}$ | $\mathcal{O}_{1-}^{h}$ |
| $(b,g,h):136$ | $R_{TT'}^{x'0}$ | ${}^{s}R_{TT}^{x'0}$ | ${}^{s}R_{LT}^{z'0}$ | ${}^{s}R_{LT}^{x'0}$ | ${}^{c}R_{LT}^{x'x}$ | ${}^{s}R_{LT'}^{z'x}$ |
| | $\mathcal{O}_{1-}^{b}$ | $\mathcal{O}_{2-}^{b}$ | $\mathcal{O}_{1+}^{g}$ | $\mathcal{O}_{2-}^{g}$ | $\mathcal{O}_{2+}^{h}$ | $\mathcal{O}_{2-}^{h}$ |
| $(b,g,h):137$ | $R_{TT'}^{x'0}$ | ${}^{s}R_{TT}^{x'0}$ | ${}^{s}R_{LT}^{z'0}$ | ${}^{s}R_{LT}^{x'0}$ | ${}^{s}R_{LT'}^{x'x}$ | ${}^{c}R_{LT}^{x'x}$ |
| | $\mathcal{O}_{1-}^{b}$ | $\mathcal{O}_{2-}^{b}$ | $\mathcal{O}_{1+}^{g}$ | $\mathcal{O}_{2-}^{g}$ | $\mathcal{O}_{1+}^{h}$ | $\mathcal{O}_{2+}^{h}$ |
| $(b,g,h):138$ | $R_{TT'}^{x'0}$ | ${}^{s}R_{TT}^{x'0}$ | ${}^{s}R_{LT}^{z'0}$ | ${}^{s}R_{LT}^{x'0}$ | ${}^{s}R_{LT'}^{x'x}$ | ${}^{s}R_{LT'}^{z'x}$ |
| | $\mathcal{O}_{1-}^{b}$ | $\mathcal{O}_{2-}^{b}$ | $\mathcal{O}_{1+}^{g}$ | $\mathcal{O}_{2-}^{g}$ | $\mathcal{O}_{1+}^{h}$ | $\mathcal{O}_{2-}^{h}$ |
| $(b,g,h):139$ | $R_{TT'}^{x'0}$ | ${}^{s}R_{TT}^{x'0}$ | ${}^{s}R_{LT}^{z'0}$ | ${}^{s}R_{LT}^{x'0}$ | ${}^{c}R_{LT}^{z'x}$ | ${}^{c}R_{LT}^{x'x}$ |
| | $\mathcal{O}_{1-}^{b}$ | $\mathcal{O}_{2-}^{b}$ | $\mathcal{O}_{1+}^{g}$ | $\mathcal{O}_{2-}^{g}$ | $\mathcal{O}_{1-}^{h}$ | $\mathcal{O}_{2+}^{h}$ |
| $(b,g,h):140$ | $R_{TT'}^{x'0}$ | ${}^{s}R_{TT}^{x'0}$ | ${}^{s}R_{LT}^{z'0}$ | ${}^{s}R_{LT}^{x'0}$ | ${}^{c}R_{LT}^{z'x}$ | ${}^{s}R_{LT'}^{z'x}$ |
| | $\mathcal{O}_{1-}^{b}$ | $\mathcal{O}_{2-}^{b}$ | $\mathcal{O}_{1+}^{g}$ | $\mathcal{O}_{2-}^{g}$ | $\mathcal{O}_{1-}^{h}$ | $\mathcal{O}_{2-}^{h}$ |
| $(b,g,h):141$ | $R_{TT'}^{x'0}$ | ${}^{s}R_{TT}^{x'0}$ | ${}^{c}R_{LT'}^{x'0}$ | ${}^{c}R_{LT'}^{z'0}$ | ${}^{s}R_{LT'}^{x'x}$ | ${}^{c}R_{LT}^{z'x}$ |
| | $\mathcal{O}_{1-}^{b}$ | $\mathcal{O}_{2-}^{b}$ | $\mathcal{O}_{1-}^{g}$ | $\mathcal{O}_{2+}^{g}$ | $\mathcal{O}_{1+}^{h}$ | $\mathcal{O}_{1-}^{h}$ |
| $(b,g,h):142$ | $R_{TT'}^{x'0}$ | ${}^{s}R_{TT}^{x'0}$ | ${}^{c}R_{LT'}^{x'0}$ | ${}^{c}R_{LT'}^{z'0}$ | ${}^{c}R_{LT}^{x'x}$ | ${}^{s}R_{LT'}^{z'x}$ |
| | $\mathcal{O}_{1-}^{b}$ | $\mathcal{O}_{2-}^{b}$ | $\mathcal{O}_{1-}^{g}$ | $\mathcal{O}_{2+}^{g}$ | $\mathcal{O}_{2+}^{h}$ | $\mathcal{O}_{2-}^{h}$ |
| $(b,g,h):143$ | $R_{TT'}^{x'0}$ | ${}^{s}R_{TT}^{x'0}$ | ${}^{c}R_{LT'}^{x'0}$ | ${}^{c}R_{LT'}^{z'0}$ | ${}^{s}R_{LT'}^{x'x}$ | ${}^{c}R_{LT}^{x'x}$ |
| | $\mathcal{O}_{1-}^{b}$ | $\mathcal{O}_{2-}^{b}$ | $\mathcal{O}_{1-}^{g}$ | $\mathcal{O}_{2+}^{g}$ | $\mathcal{O}_{1+}^{h}$ | $\mathcal{O}_{2+}^{h}$ |
| $(b,g,h):144$ | $R_{TT'}^{x'0}$ | ${}^{s}R_{TT}^{x'0}$ | ${}^{c}R_{LT'}^{x'0}$ | ${}^{c}R_{LT'}^{z'0}$ | ${}^{s}R_{LT'}^{x'x}$ | ${}^{s}R_{LT'}^{z'x}$ |
| | $\mathcal{O}_{1-}^{b}$ | $\mathcal{O}_{2-}^{b}$ | $\mathcal{O}_{1-}^{g}$ | $\mathcal{O}_{2+}^{g}$ | $\mathcal{O}_{1+}^{h}$ | $\mathcal{O}_{2-}^{h}$ |
| $(b,g,h):145$ | $R_{TT'}^{x'0}$ | ${}^{s}R_{TT}^{x'0}$ | ${}^{c}R_{LT'}^{x'0}$ | ${}^{c}R_{LT'}^{z'0}$ | ${}^{c}R_{LT}^{z'x}$ | ${}^{c}R_{LT}^{x'x}$ |
| | $\mathcal{O}_{1-}^{b}$ | $\mathcal{O}_{2-}^{b}$ | $\mathcal{O}_{1-}^{g}$ | $\mathcal{O}_{2+}^{g}$ | $\mathcal{O}_{1-}^{h}$ | $\mathcal{O}_{2+}^{h}$ |
| $(b,g,h):146$ | $R_{TT'}^{x'0}$ | ${}^{s}R_{TT}^{x'0}$ | ${}^{c}R_{LT'}^{x'0}$ | ${}^{c}R_{LT'}^{z'0}$ | ${}^{c}R_{LT}^{z'x}$ | ${}^{s}R_{LT'}^{z'x}$ |
| | $\mathcal{O}_{1-}^{b}$ | $\mathcal{O}_{2-}^{b}$ | $\mathcal{O}_{1-}^{g}$ | $\mathcal{O}_{2+}^{g}$ | $\mathcal{O}_{1-}^{h}$ | $\mathcal{O}_{2-}^{h}$ |
| $(b,g,h):147$ | $R_{TT'}^{x'0}$ | ${}^{s}R_{TT}^{x'0}$ | ${}^{c}R_{LT'}^{x'0}$ | ${}^{s}R_{LT}^{x'0}$ | ${}^{s}R_{LT'}^{x'x}$ | ${}^{c}R_{LT}^{z'x}$ |
| | $\mathcal{O}_{1-}^{b}$ | $\mathcal{O}_{2-}^{b}$ | $\mathcal{O}_{1-}^{g}$ | $\mathcal{O}_{2-}^{g}$ | $\mathcal{O}_{1+}^{h}$ | $\mathcal{O}_{1-}^{h}$ |
| $(b,g,h):148$ | $R_{TT'}^{x'0}$ | ${}^{s}R_{TT}^{x'0}$ | ${}^{c}R_{LT'}^{x'0}$ | ${}^{s}R_{LT}^{x'0}$ | ${}^{c}R_{LT}^{x'x}$ | ${}^{s}R_{LT'}^{z'x}$ |
| | $\mathcal{O}_{1-}^{b}$ | $\mathcal{O}_{2-}^{b}$ | $\mathcal{O}_{1-}^{g}$ | $\mathcal{O}_{2-}^{g}$ | $\mathcal{O}_{2+}^{h}$ | $\mathcal{O}_{2-}^{h}$ |
| $(b,g,h):149$ | $R_{TT'}^{x'0}$ | ${}^{s}R_{TT}^{x'0}$ | ${}^{c}R_{LT'}^{x'0}$ | ${}^{s}R_{LT}^{x'0}$ | ${}^{s}R_{LT'}^{x'x}$ | ${}^{c}R_{LT}^{x'x}$ |
| | $\mathcal{O}_{1-}^{b}$ | $\mathcal{O}_{2-}^{b}$ | $\mathcal{O}_{1-}^{g}$ | $\mathcal{O}_{2-}^{g}$ | $\mathcal{O}_{1+}^{h}$ | $\mathcal{O}_{2+}^{h}$ |
| $(b,g,h):150$ | $R_{TT'}^{x'0}$ | ${}^{s}R_{TT}^{x'0}$ | ${}^{c}R_{LT'}^{x'0}$ | ${}^{s}R_{LT}^{x'0}$ | ${}^{s}R_{LT'}^{x'x}$ | ${}^{s}R_{LT'}^{z'x}$ |
| | $\mathcal{O}_{1-}^{b}$ | $\mathcal{O}_{2-}^{b}$ | $\mathcal{O}_{1-}^{g}$ | $\mathcal{O}_{2-}^{g}$ | $\mathcal{O}_{1+}^{h}$ | $\mathcal{O}_{2-}^{h}$ |
| $(b,g,h):151$ | $R_{TT'}^{x'0}$ | ${}^{s}R_{TT}^{x'0}$ | ${}^{c}R_{LT'}^{x'0}$ | ${}^{s}R_{LT}^{x'0}$ | ${}^{c}R_{LT}^{z'x}$ | ${}^{c}R_{LT}^{x'x}$ |
| | $\mathcal{O}_{1-}^{b}$ | $\mathcal{O}_{2-}^{b}$ | $\mathcal{O}_{1-}^{g}$ | $\mathcal{O}_{2-}^{g}$ | $\mathcal{O}_{1-}^{h}$ | $\mathcal{O}_{2+}^{h}$ |
| $(b,g,h):152$ | $R_{TT'}^{x'0}$ | ${}^{s}R_{TT}^{x'0}$ | ${}^{c}R_{LT'}^{x'0}$ | ${}^{s}R_{LT}^{x'0}$ | ${}^{c}R_{LT}^{z'x}$ | ${}^{s}R_{LT'}^{z'x}$ |
| | $\mathcal{O}_{1-}^{b}$ | $\mathcal{O}_{2-}^{b}$ | $\mathcal{O}_{1-}^{g}$ | $\mathcal{O}_{2-}^{g}$ | $\mathcal{O}_{1-}^{h}$ | $\mathcal{O}_{2-}^{h}$ |

TABLE VIII: All the fully complete sets determined from the combination of shape-classes $(c, e, f)$ (i.e. graph-topology 'V') in the case of pseudoscalar meson electroproduction are listed here. The observables are written in the systematic symbolic notation $\mathcal{O}^{n}_{\nu\pm}$ by Nakayama [1], as well as in the more commonly used notation in terms of 'response-functions' $R_{i}^{\beta\alpha}$ (cf. references [4, 5]). The given sets of 6 observables have to be combined with the 6 'diagonal' observables $\left\{ R_{T}^{00}, {}^{c}R_{TT}^{00}, R_{T}^{0y}, R_{T}^{y'0}, R_{L}^{00}, R_{L}^{0y} \right\}$ in order to form a complete set of minimal length $2N = 12$. All of these sets have been verified to be complete using Mathematica [3].

| Set-Nr. | Observables | | | | | |
|---|---|---|---|---|---|---|
| $(c, e, f) : 1$ | $R_{T}^{x'z}$ | $R_{T}^{z'x}$ | ${}^{s}R_{LT'}^{00}$ | ${}^{s}R_{LT'}^{0y}$ | ${}^{s}R_{LT}^{0z}$ | ${}^{s}R_{LT}^{0x}$ |
| | $\mathcal{O}^{c}_{1+}$ | $\mathcal{O}^{c}_{1-}$ | $\mathcal{O}^{e}_{1+}$ | $\mathcal{O}^{e}_{1-}$ | $\mathcal{O}^{f}_{1+}$ | $\mathcal{O}^{f}_{2-}$ |
| $(c, e, f) : 2$ | $R_{T}^{x'z}$ | $R_{T}^{z'x}$ | ${}^{s}R_{LT'}^{00}$ | ${}^{s}R_{LT'}^{0y}$ | ${}^{c}R_{LT'}^{0x}$ | ${}^{c}R_{LT'}^{0z}$ |
| | $\mathcal{O}^{c}_{1+}$ | $\mathcal{O}^{c}_{1-}$ | $\mathcal{O}^{e}_{1+}$ | $\mathcal{O}^{e}_{1-}$ | $\mathcal{O}^{f}_{1-}$ | $\mathcal{O}^{f}_{2+}$ |
| $(c, e, f) : 3$ | $R_{T}^{x'z}$ | $R_{T}^{z'x}$ | ${}^{c}R_{LT}^{00}$ | ${}^{c}R_{LT}^{0y}$ | ${}^{s}R_{LT}^{0z}$ | ${}^{s}R_{LT}^{0x}$ |
| | $\mathcal{O}^{c}_{1+}$ | $\mathcal{O}^{c}_{1-}$ | $\mathcal{O}^{e}_{2+}$ | $\mathcal{O}^{e}_{2-}$ | $\mathcal{O}^{f}_{1+}$ | $\mathcal{O}^{f}_{2-}$ |
| $(c, e, f) : 4$ | $R_{T}^{x'z}$ | $R_{T}^{z'x}$ | ${}^{c}R_{LT}^{00}$ | ${}^{c}R_{LT}^{0y}$ | ${}^{c}R_{LT'}^{0x}$ | ${}^{c}R_{LT'}^{0z}$ |
| | $\mathcal{O}^{c}_{1+}$ | $\mathcal{O}^{c}_{1-}$ | $\mathcal{O}^{e}_{2+}$ | $\mathcal{O}^{e}_{2-}$ | $\mathcal{O}^{f}_{1-}$ | $\mathcal{O}^{f}_{2+}$ |
| $(c, e, f) : 5$ | $R_{T}^{x'z}$ | $R_{T}^{z'x}$ | ${}^{s}R_{LT'}^{00}$ | ${}^{c}R_{LT}^{00}$ | ${}^{s}R_{LT}^{0z}$ | ${}^{s}R_{LT}^{0x}$ |
| | $\mathcal{O}^{c}_{1+}$ | $\mathcal{O}^{c}_{1-}$ | $\mathcal{O}^{e}_{1+}$ | $\mathcal{O}^{e}_{2+}$ | $\mathcal{O}^{f}_{1+}$ | $\mathcal{O}^{f}_{2-}$ |
| $(c, e, f) : 6$ | $R_{T}^{x'z}$ | $R_{T}^{z'x}$ | ${}^{s}R_{LT'}^{00}$ | ${}^{c}R_{LT}^{00}$ | ${}^{c}R_{LT'}^{0x}$ | ${}^{c}R_{LT'}^{0z}$ |
| | $\mathcal{O}^{c}_{1+}$ | $\mathcal{O}^{c}_{1-}$ | $\mathcal{O}^{e}_{1+}$ | $\mathcal{O}^{e}_{2+}$ | $\mathcal{O}^{f}_{1-}$ | $\mathcal{O}^{f}_{2+}$ |
| $(c, e, f) : 7$ | $R_{T}^{x'z}$ | $R_{T}^{z'x}$ | ${}^{s}R_{LT'}^{00}$ | ${}^{c}R_{LT}^{0y}$ | ${}^{s}R_{LT}^{0z}$ | ${}^{c}R_{LT'}^{0x}$ |
| | $\mathcal{O}^{c}_{1+}$ | $\mathcal{O}^{c}_{1-}$ | $\mathcal{O}^{e}_{1+}$ | $\mathcal{O}^{e}_{2-}$ | $\mathcal{O}^{f}_{1+}$ | $\mathcal{O}^{f}_{1-}$ |
| $(c, e, f) : 8$ | $R_{T}^{x'z}$ | $R_{T}^{z'x}$ | ${}^{s}R_{LT'}^{00}$ | ${}^{c}R_{LT}^{0y}$ | ${}^{c}R_{LT'}^{0z}$ | ${}^{s}R_{LT}^{0x}$ |
| | $\mathcal{O}^{c}_{1+}$ | $\mathcal{O}^{c}_{1-}$ | $\mathcal{O}^{e}_{1+}$ | $\mathcal{O}^{e}_{2-}$ | $\mathcal{O}^{f}_{2+}$ | $\mathcal{O}^{f}_{2-}$ |
| $(c, e, f) : 9$ | $R_{T}^{x'z}$ | $R_{T}^{z'x}$ | ${}^{s}R_{LT'}^{00}$ | ${}^{c}R_{LT}^{0y}$ | ${}^{s}R_{LT}^{0z}$ | ${}^{c}R_{LT'}^{0z}$ |
| | $\mathcal{O}^{c}_{1+}$ | $\mathcal{O}^{c}_{1-}$ | $\mathcal{O}^{e}_{1+}$ | $\mathcal{O}^{e}_{2-}$ | $\mathcal{O}^{f}_{1+}$ | $\mathcal{O}^{f}_{2+}$ |
| $(c, e, f) : 10$ | $R_{T}^{x'z}$ | $R_{T}^{z'x}$ | ${}^{s}R_{LT'}^{00}$ | ${}^{c}R_{LT}^{0y}$ | ${}^{s}R_{LT}^{0z}$ | ${}^{s}R_{LT}^{0x}$ |
| | $\mathcal{O}^{c}_{1+}$ | $\mathcal{O}^{c}_{1-}$ | $\mathcal{O}^{e}_{1+}$ | $\mathcal{O}^{e}_{2-}$ | $\mathcal{O}^{f}_{1+}$ | $\mathcal{O}^{f}_{2-}$ |
| $(c, e, f) : 11$ | $R_{T}^{x'z}$ | $R_{T}^{z'x}$ | ${}^{s}R_{LT'}^{00}$ | ${}^{c}R_{LT}^{0y}$ | ${}^{c}R_{LT'}^{0x}$ | ${}^{c}R_{LT'}^{0z}$ |
| | $\mathcal{O}^{c}_{1+}$ | $\mathcal{O}^{c}_{1-}$ | $\mathcal{O}^{e}_{1+}$ | $\mathcal{O}^{e}_{2-}$ | $\mathcal{O}^{f}_{1-}$ | $\mathcal{O}^{f}_{2+}$ |
| $(c, e, f) : 12$ | $R_{T}^{x'z}$ | $R_{T}^{z'x}$ | ${}^{s}R_{LT'}^{00}$ | ${}^{c}R_{LT}^{0y}$ | ${}^{c}R_{LT'}^{0x}$ | ${}^{s}R_{LT}^{0x}$ |
| | $\mathcal{O}^{c}_{1+}$ | $\mathcal{O}^{c}_{1-}$ | $\mathcal{O}^{e}_{1+}$ | $\mathcal{O}^{e}_{2-}$ | $\mathcal{O}^{f}_{1-}$ | $\mathcal{O}^{f}_{2-}$ |
| $(c, e, f) : 13$ | $R_{T}^{x'z}$ | $R_{T}^{z'x}$ | ${}^{s}R_{LT'}^{0y}$ | ${}^{c}R_{LT}^{00}$ | ${}^{s}R_{LT}^{0z}$ | ${}^{c}R_{LT'}^{0x}$ |
| | $\mathcal{O}^{c}_{1+}$ | $\mathcal{O}^{c}_{1-}$ | $\mathcal{O}^{e}_{1-}$ | $\mathcal{O}^{e}_{2+}$ | $\mathcal{O}^{f}_{1+}$ | $\mathcal{O}^{f}_{1-}$ |
| $(c, e, f) : 14$ | $R_{T}^{x'z}$ | $R_{T}^{z'x}$ | ${}^{s}R_{LT'}^{0y}$ | ${}^{c}R_{LT}^{00}$ | ${}^{c}R_{LT'}^{0z}$ | ${}^{s}R_{LT}^{0x}$ |
| | $\mathcal{O}^{c}_{1+}$ | $\mathcal{O}^{c}_{1-}$ | $\mathcal{O}^{e}_{1-}$ | $\mathcal{O}^{e}_{2+}$ | $\mathcal{O}^{f}_{2+}$ | $\mathcal{O}^{f}_{2-}$ |
| $(c, e, f) : 15$ | $R_{T}^{x'z}$ | $R_{T}^{z'x}$ | ${}^{s}R_{LT'}^{0y}$ | ${}^{c}R_{LT}^{00}$ | ${}^{s}R_{LT}^{0z}$ | ${}^{c}R_{LT'}^{0z}$ |
| | $\mathcal{O}^{c}_{1+}$ | $\mathcal{O}^{c}_{1-}$ | $\mathcal{O}^{e}_{1-}$ | $\mathcal{O}^{e}_{2+}$ | $\mathcal{O}^{f}_{1+}$ | $\mathcal{O}^{f}_{2+}$ |
| $(c, e, f) : 16$ | $R_{T}^{x'z}$ | $R_{T}^{z'x}$ | ${}^{s}R_{LT'}^{0y}$ | ${}^{c}R_{LT}^{00}$ | ${}^{s}R_{LT}^{0z}$ | ${}^{s}R_{LT}^{0x}$ |
| | $\mathcal{O}^{c}_{1+}$ | $\mathcal{O}^{c}_{1-}$ | $\mathcal{O}^{e}_{1-}$ | $\mathcal{O}^{e}_{2+}$ | $\mathcal{O}^{f}_{1+}$ | $\mathcal{O}^{f}_{2-}$ |
| $(c, e, f) : 17$ | $R_{T}^{x'z}$ | $R_{T}^{z'x}$ | ${}^{s}R_{LT'}^{0y}$ | ${}^{c}R_{LT}^{00}$ | ${}^{c}R_{LT'}^{0x}$ | ${}^{c}R_{LT'}^{0z}$ |
| | $\mathcal{O}^{c}_{1+}$ | $\mathcal{O}^{c}_{1-}$ | $\mathcal{O}^{e}_{1-}$ | $\mathcal{O}^{e}_{2+}$ | $\mathcal{O}^{f}_{1-}$ | $\mathcal{O}^{f}_{2+}$ |
| $(c, e, f) : 18$ | $R_{T}^{x'z}$ | $R_{T}^{z'x}$ | ${}^{s}R_{LT'}^{0y}$ | ${}^{c}R_{LT}^{00}$ | ${}^{c}R_{LT'}^{0x}$ | ${}^{s}R_{LT}^{0x}$ |
| | $\mathcal{O}^{c}_{1+}$ | $\mathcal{O}^{c}_{1-}$ | $\mathcal{O}^{e}_{1-}$ | $\mathcal{O}^{e}_{2+}$ | $\mathcal{O}^{f}_{1-}$ | $\mathcal{O}^{f}_{2-}$ |
| $(c, e, f) : 19$ | $R_{T}^{x'z}$ | $R_{T}^{z'x}$ | ${}^{s}R_{LT'}^{0y}$ | ${}^{c}R_{LT}^{0y}$ | ${}^{s}R_{LT}^{0z}$ | ${}^{s}R_{LT}^{0x}$ |
| | $\mathcal{O}^{c}_{1+}$ | $\mathcal{O}^{c}_{1-}$ | $\mathcal{O}^{e}_{1-}$ | $\mathcal{O}^{e}_{2-}$ | $\mathcal{O}^{f}_{1+}$ | $\mathcal{O}^{f}_{2-}$ |
| $(c, e, f) : 20$ | $R_{T}^{x'z}$ | $R_{T}^{z'x}$ | ${}^{s}R_{LT'}^{0y}$ | ${}^{c}R_{LT}^{0y}$ | ${}^{c}R_{LT'}^{0x}$ | ${}^{c}R_{LT'}^{0z}$ |
| | $\mathcal{O}^{c}_{1+}$ | $\mathcal{O}^{c}_{1-}$ | $\mathcal{O}^{e}_{1-}$ | $\mathcal{O}^{e}_{2-}$ | $\mathcal{O}^{f}_{1-}$ | $\mathcal{O}^{f}_{2+}$ |
| $(c, e, f) : 21$ | $R_{T}^{z'z}$ | $R_{T}^{x'x}$ | ${}^{s}R_{LT'}^{00}$ | ${}^{s}R_{LT'}^{0y}$ | ${}^{s}R_{LT}^{0z}$ | ${}^{s}R_{LT}^{0x}$ |
| | $\mathcal{O}^{c}_{2+}$ | $\mathcal{O}^{c}_{2-}$ | $\mathcal{O}^{e}_{1+}$ | $\mathcal{O}^{e}_{1-}$ | $\mathcal{O}^{f}_{1+}$ | $\mathcal{O}^{f}_{2-}$ |
| $(c, e, f) : 22$ | $R_{T}^{z'z}$ | $R_{T}^{x'x}$ | ${}^{s}R_{LT'}^{00}$ | ${}^{s}R_{LT'}^{0y}$ | ${}^{c}R_{LT'}^{0x}$ | ${}^{c}R_{LT'}^{0z}$ |
| | $\mathcal{O}^{c}_{2+}$ | $\mathcal{O}^{c}_{2-}$ | $\mathcal{O}^{e}_{1+}$ | $\mathcal{O}^{e}_{1-}$ | $\mathcal{O}^{f}_{1-}$ | $\mathcal{O}^{f}_{2+}$ |
| $(c, e, f) : 23$ | $R_{T}^{z'z}$ | $R_{T}^{x'x}$ | ${}^{c}R_{LT}^{00}$ | ${}^{c}R_{LT}^{0y}$ | ${}^{s}R_{LT}^{0z}$ | ${}^{s}R_{LT}^{0x}$ |

| | | | | | | |
|---|---|---|---|---|---|---|
| | $\mathcal{O}^c_{2+}$ | $\mathcal{O}^c_{2-}$ | $\mathcal{O}^e_{2+}$ | $\mathcal{O}^e_{2-}$ | $\mathcal{O}^f_{1+}$ | $\mathcal{O}^f_{2-}$ |
| $(c,e,f):24$ | $R^{z'z}_T$ | $R^{x'x}_T$ | ${}^cR^{00}_{LT}$ | ${}^cR^{0y}_{LT}$ | ${}^cR^{0x}_{LT'}$ | ${}^cR^{0z}_{LT'}$ |
| | $\mathcal{O}^c_{2+}$ | $\mathcal{O}^c_{2-}$ | $\mathcal{O}^e_{2+}$ | $\mathcal{O}^e_{2-}$ | $\mathcal{O}^f_{1-}$ | $\mathcal{O}^f_{2+}$ |
| $(c,e,f):25$ | $R^{z'z}_T$ | $R^{x'x}_T$ | ${}^sR^{00}_{LT'}$ | ${}^cR^{00}_{LT}$ | ${}^sR^{0z}_{LT}$ | ${}^sR^{0x}_{LT}$ |
| | $\mathcal{O}^c_{2+}$ | $\mathcal{O}^c_{2-}$ | $\mathcal{O}^e_{1+}$ | $\mathcal{O}^e_{2+}$ | $\mathcal{O}^f_{1+}$ | $\mathcal{O}^f_{2-}$ |
| $(c,e,f):26$ | $R^{z'z}_T$ | $R^{x'x}_T$ | ${}^sR^{00}_{LT'}$ | ${}^cR^{00}_{LT}$ | ${}^cR^{0x}_{LT'}$ | ${}^cR^{0z}_{LT'}$ |
| | $\mathcal{O}^c_{2+}$ | $\mathcal{O}^c_{2-}$ | $\mathcal{O}^e_{1+}$ | $\mathcal{O}^e_{2+}$ | $\mathcal{O}^f_{1-}$ | $\mathcal{O}^f_{2+}$ |
| $(c,e,f):27$ | $R^{z'z}_T$ | $R^{x'x}_T$ | ${}^sR^{00}_{LT'}$ | ${}^cR^{0y}_{LT}$ | ${}^sR^{0z}_{LT}$ | ${}^cR^{0x}_{LT'}$ |
| | $\mathcal{O}^c_{2+}$ | $\mathcal{O}^c_{2-}$ | $\mathcal{O}^e_{1+}$ | $\mathcal{O}^e_{2-}$ | $\mathcal{O}^f_{1+}$ | $\mathcal{O}^f_{1-}$ |
| $(c,e,f):28$ | $R^{z'z}_T$ | $R^{x'x}_T$ | ${}^sR^{00}_{LT'}$ | ${}^cR^{0y}_{LT}$ | ${}^cR^{0z}_{LT'}$ | ${}^sR^{0x}_{LT}$ |
| | $\mathcal{O}^c_{2+}$ | $\mathcal{O}^c_{2-}$ | $\mathcal{O}^e_{1+}$ | $\mathcal{O}^e_{2-}$ | $\mathcal{O}^f_{2+}$ | $\mathcal{O}^f_{2-}$ |
| $(c,e,f):29$ | $R^{z'z}_T$ | $R^{x'x}_T$ | ${}^sR^{00}_{LT'}$ | ${}^cR^{0y}_{LT}$ | ${}^sR^{0z}_{LT}$ | ${}^cR^{0z}_{LT'}$ |
| | $\mathcal{O}^c_{2+}$ | $\mathcal{O}^c_{2-}$ | $\mathcal{O}^e_{1+}$ | $\mathcal{O}^e_{2-}$ | $\mathcal{O}^f_{1+}$ | $\mathcal{O}^f_{2+}$ |
| $(c,e,f):30$ | $R^{z'z}_T$ | $R^{x'x}_T$ | ${}^sR^{00}_{LT'}$ | ${}^cR^{0y}_{LT}$ | ${}^sR^{0z}_{LT}$ | ${}^sR^{0x}_{LT}$ |
| | $\mathcal{O}^c_{2+}$ | $\mathcal{O}^c_{2-}$ | $\mathcal{O}^e_{1+}$ | $\mathcal{O}^e_{2-}$ | $\mathcal{O}^f_{1+}$ | $\mathcal{O}^f_{2-}$ |
| $(c,e,f):31$ | $R^{z'z}_T$ | $R^{x'x}_T$ | ${}^sR^{00}_{LT'}$ | ${}^cR^{0y}_{LT}$ | ${}^cR^{0x}_{LT'}$ | ${}^cR^{0z}_{LT'}$ |
| | $\mathcal{O}^c_{2+}$ | $\mathcal{O}^c_{2-}$ | $\mathcal{O}^e_{1+}$ | $\mathcal{O}^e_{2-}$ | $\mathcal{O}^f_{1-}$ | $\mathcal{O}^f_{2+}$ |
| $(c,e,f):32$ | $R^{z'z}_T$ | $R^{x'x}_T$ | ${}^sR^{00}_{LT'}$ | ${}^cR^{0y}_{LT}$ | ${}^cR^{0x}_{LT'}$ | ${}^sR^{0x}_{LT}$ |
| | $\mathcal{O}^c_{2+}$ | $\mathcal{O}^c_{2-}$ | $\mathcal{O}^e_{1+}$ | $\mathcal{O}^e_{2-}$ | $\mathcal{O}^f_{1-}$ | $\mathcal{O}^f_{2-}$ |
| $(c,e,f):33$ | $R^{z'z}_T$ | $R^{x'x}_T$ | ${}^sR^{0y}_{LT'}$ | ${}^cR^{00}_{LT}$ | ${}^sR^{0z}_{LT}$ | ${}^cR^{0x}_{LT'}$ |
| | $\mathcal{O}^c_{2+}$ | $\mathcal{O}^c_{2-}$ | $\mathcal{O}^e_{1-}$ | $\mathcal{O}^e_{2+}$ | $\mathcal{O}^f_{1+}$ | $\mathcal{O}^f_{1-}$ |
| $(c,e,f):34$ | $R^{z'z}_T$ | $R^{x'x}_T$ | ${}^sR^{0y}_{LT'}$ | ${}^cR^{00}_{LT}$ | ${}^cR^{0z}_{LT'}$ | ${}^sR^{0x}_{LT}$ |
| | $\mathcal{O}^c_{2+}$ | $\mathcal{O}^c_{2-}$ | $\mathcal{O}^e_{1-}$ | $\mathcal{O}^e_{2+}$ | $\mathcal{O}^f_{2+}$ | $\mathcal{O}^f_{2-}$ |
| $(c,e,f):35$ | $R^{z'z}_T$ | $R^{x'x}_T$ | ${}^sR^{0y}_{LT'}$ | ${}^cR^{00}_{LT}$ | ${}^sR^{0z}_{LT}$ | ${}^cR^{0z}_{LT'}$ |
| | $\mathcal{O}^c_{2+}$ | $\mathcal{O}^c_{2-}$ | $\mathcal{O}^e_{1-}$ | $\mathcal{O}^e_{2+}$ | $\mathcal{O}^f_{1+}$ | $\mathcal{O}^f_{2+}$ |
| $(c,e,f):36$ | $R^{z'z}_T$ | $R^{x'x}_T$ | ${}^sR^{0y}_{LT'}$ | ${}^cR^{00}_{LT}$ | ${}^sR^{0z}_{LT}$ | ${}^sR^{0x}_{LT}$ |
| | $\mathcal{O}^c_{2+}$ | $\mathcal{O}^c_{2-}$ | $\mathcal{O}^e_{1-}$ | $\mathcal{O}^e_{2+}$ | $\mathcal{O}^f_{1+}$ | $\mathcal{O}^f_{2-}$ |
| $(c,e,f):37$ | $R^{z'z}_T$ | $R^{x'x}_T$ | ${}^sR^{0y}_{LT'}$ | ${}^cR^{00}_{LT}$ | ${}^cR^{0x}_{LT'}$ | ${}^cR^{0z}_{LT'}$ |
| | $\mathcal{O}^c_{2+}$ | $\mathcal{O}^c_{2-}$ | $\mathcal{O}^e_{1-}$ | $\mathcal{O}^e_{2+}$ | $\mathcal{O}^f_{1-}$ | $\mathcal{O}^f_{2+}$ |
| $(c,e,f):38$ | $R^{z'z}_T$ | $R^{x'x}_T$ | ${}^sR^{0y}_{LT'}$ | ${}^cR^{00}_{LT}$ | ${}^cR^{0x}_{LT'}$ | ${}^sR^{0x}_{LT}$ |
| | $\mathcal{O}^c_{2+}$ | $\mathcal{O}^c_{2-}$ | $\mathcal{O}^e_{1-}$ | $\mathcal{O}^e_{2+}$ | $\mathcal{O}^f_{1-}$ | $\mathcal{O}^f_{2-}$ |
| $(c,e,f):39$ | $R^{z'z}_T$ | $R^{x'x}_T$ | ${}^sR^{0y}_{LT'}$ | ${}^cR^{0y}_{LT}$ | ${}^sR^{0z}_{LT}$ | ${}^sR^{0x}_{LT}$ |
| | $\mathcal{O}^c_{2+}$ | $\mathcal{O}^c_{2-}$ | $\mathcal{O}^e_{1-}$ | $\mathcal{O}^e_{2-}$ | $\mathcal{O}^f_{1+}$ | $\mathcal{O}^f_{2-}$ |
| $(c,e,f):40$ | $R^{z'z}_T$ | $R^{x'x}_T$ | ${}^sR^{0y}_{LT'}$ | ${}^cR^{0y}_{LT}$ | ${}^cR^{0x}_{LT'}$ | ${}^cR^{0z}_{LT'}$ |
| | $\mathcal{O}^c_{2+}$ | $\mathcal{O}^c_{2-}$ | $\mathcal{O}^e_{1-}$ | $\mathcal{O}^e_{2-}$ | $\mathcal{O}^f_{1-}$ | $\mathcal{O}^f_{2+}$ |
| $(c,e,f):41$ | $R^{x'z}_T$ | $R^{z'z}_T$ | ${}^sR^{00}_{LT'}$ | ${}^sR^{0y}_{LT'}$ | ${}^sR^{0z}_{LT}$ | ${}^sR^{0x}_{LT}$ |
| | $\mathcal{O}^c_{1+}$ | $\mathcal{O}^c_{2+}$ | $\mathcal{O}^e_{1+}$ | $\mathcal{O}^e_{1-}$ | $\mathcal{O}^f_{1+}$ | $\mathcal{O}^f_{2-}$ |
| $(c,e,f):42$ | $R^{x'z}_T$ | $R^{z'z}_T$ | ${}^sR^{00}_{LT'}$ | ${}^sR^{0y}_{LT'}$ | ${}^cR^{0x}_{LT'}$ | ${}^cR^{0z}_{LT'}$ |
| | $\mathcal{O}^c_{1+}$ | $\mathcal{O}^c_{2+}$ | $\mathcal{O}^e_{1+}$ | $\mathcal{O}^e_{1-}$ | $\mathcal{O}^f_{1-}$ | $\mathcal{O}^f_{2+}$ |
| $(c,e,f):43$ | $R^{x'z}_T$ | $R^{z'z}_T$ | ${}^cR^{00}_{LT}$ | ${}^cR^{0y}_{LT}$ | ${}^sR^{0z}_{LT}$ | ${}^sR^{0x}_{LT}$ |
| | $\mathcal{O}^c_{1+}$ | $\mathcal{O}^c_{2+}$ | $\mathcal{O}^e_{2+}$ | $\mathcal{O}^e_{2-}$ | $\mathcal{O}^f_{1+}$ | $\mathcal{O}^f_{2-}$ |
| $(c,e,f):44$ | $R^{x'z}_T$ | $R^{z'z}_T$ | ${}^cR^{00}_{LT}$ | ${}^cR^{0y}_{LT}$ | ${}^cR^{0x}_{LT'}$ | ${}^cR^{0z}_{LT'}$ |
| | $\mathcal{O}^c_{1+}$ | $\mathcal{O}^c_{2+}$ | $\mathcal{O}^e_{2+}$ | $\mathcal{O}^e_{2-}$ | $\mathcal{O}^f_{1-}$ | $\mathcal{O}^f_{2+}$ |
| $(c,e,f):45$ | $R^{x'z}_T$ | $R^{z'z}_T$ | ${}^sR^{00}_{LT'}$ | ${}^cR^{00}_{LT}$ | ${}^sR^{0z}_{LT}$ | ${}^sR^{0x}_{LT}$ |
| | $\mathcal{O}^c_{1+}$ | $\mathcal{O}^c_{2+}$ | $\mathcal{O}^e_{1+}$ | $\mathcal{O}^e_{2+}$ | $\mathcal{O}^f_{1+}$ | $\mathcal{O}^f_{2-}$ |
| $(c,e,f):46$ | $R^{x'z}_T$ | $R^{z'z}_T$ | ${}^sR^{00}_{LT'}$ | ${}^cR^{00}_{LT}$ | ${}^cR^{0x}_{LT'}$ | ${}^cR^{0z}_{LT'}$ |
| | $\mathcal{O}^c_{1+}$ | $\mathcal{O}^c_{2+}$ | $\mathcal{O}^e_{1+}$ | $\mathcal{O}^e_{2+}$ | $\mathcal{O}^f_{1-}$ | $\mathcal{O}^f_{2+}$ |
| $(c,e,f):47$ | $R^{x'z}_T$ | $R^{z'z}_T$ | ${}^sR^{00}_{LT'}$ | ${}^cR^{0y}_{LT}$ | ${}^sR^{0z}_{LT}$ | ${}^cR^{0x}_{LT'}$ |
| | $\mathcal{O}^c_{1+}$ | $\mathcal{O}^c_{2+}$ | $\mathcal{O}^e_{1+}$ | $\mathcal{O}^e_{2-}$ | $\mathcal{O}^f_{1+}$ | $\mathcal{O}^f_{1-}$ |
| $(c,e,f):48$ | $R^{x'z}_T$ | $R^{z'z}_T$ | ${}^sR^{00}_{LT'}$ | ${}^cR^{0y}_{LT}$ | ${}^cR^{0z}_{LT'}$ | ${}^sR^{0x}_{LT}$ |
| | $\mathcal{O}^c_{1+}$ | $\mathcal{O}^c_{2+}$ | $\mathcal{O}^e_{1+}$ | $\mathcal{O}^e_{2-}$ | $\mathcal{O}^f_{2+}$ | $\mathcal{O}^f_{2-}$ |
| $(c,e,f):49$ | $R^{x'z}_T$ | $R^{z'z}_T$ | ${}^sR^{00}_{LT'}$ | ${}^cR^{0y}_{LT}$ | ${}^sR^{0z}_{LT}$ | ${}^cR^{0z}_{LT'}$ |
| | $\mathcal{O}^c_{1+}$ | $\mathcal{O}^c_{2+}$ | $\mathcal{O}^e_{1+}$ | $\mathcal{O}^e_{2-}$ | $\mathcal{O}^f_{1+}$ | $\mathcal{O}^f_{2+}$ |
| $(c,e,f):50$ | $R^{x'z}_T$ | $R^{z'z}_T$ | ${}^sR^{00}_{LT'}$ | ${}^cR^{0y}_{LT}$ | ${}^sR^{0z}_{LT}$ | ${}^sR^{0x}_{LT}$ |
| | $\mathcal{O}^c_{1+}$ | $\mathcal{O}^c_{2+}$ | $\mathcal{O}^e_{1+}$ | $\mathcal{O}^e_{2-}$ | $\mathcal{O}^f_{1+}$ | $\mathcal{O}^f_{2-}$ |

| | | | | | | |
|---|---|---|---|---|---|---|
| $(c,e,f):51$ | $R_T^{x'z}$ | $R_T^{z'z}$ | ${}^sR_{LT'}^{00}$ | ${}^cR_{LT}^{0y}$ | ${}^cR_{LT'}^{0x}$ | ${}^cR_{LT'}^{0z}$ |
| | $\mathcal{O}_{1+}^c$ | $\mathcal{O}_{2+}^c$ | $\mathcal{O}_{1+}^e$ | $\mathcal{O}_{2-}^e$ | $\mathcal{O}_{1-}^f$ | $\mathcal{O}_{2+}^f$ |
| $(c,e,f):52$ | $R_T^{x'z}$ | $R_T^{z'z}$ | ${}^sR_{LT'}^{00}$ | ${}^cR_{LT}^{0y}$ | ${}^cR_{LT'}^{0x}$ | ${}^sR_{LT}^{0x}$ |
| | $\mathcal{O}_{1+}^c$ | $\mathcal{O}_{2+}^c$ | $\mathcal{O}_{1+}^e$ | $\mathcal{O}_{2-}^e$ | $\mathcal{O}_{1-}^f$ | $\mathcal{O}_{2-}^f$ |
| $(c,e,f):53$ | $R_T^{x'z}$ | $R_T^{z'z}$ | ${}^sR_{LT'}^{0y}$ | ${}^cR_{LT}^{00}$ | ${}^sR_{LT}^{0z}$ | ${}^cR_{LT'}^{0x}$ |
| | $\mathcal{O}_{1+}^c$ | $\mathcal{O}_{2+}^c$ | $\mathcal{O}_{1-}^e$ | $\mathcal{O}_{2+}^e$ | $\mathcal{O}_{1+}^f$ | $\mathcal{O}_{1-}^f$ |
| $(c,e,f):54$ | $R_T^{x'z}$ | $R_T^{z'z}$ | ${}^sR_{LT'}^{0y}$ | ${}^cR_{LT}^{00}$ | ${}^cR_{LT'}^{0z}$ | ${}^sR_{LT}^{0x}$ |
| | $\mathcal{O}_{1+}^c$ | $\mathcal{O}_{2+}^c$ | $\mathcal{O}_{1-}^e$ | $\mathcal{O}_{2+}^e$ | $\mathcal{O}_{2+}^f$ | $\mathcal{O}_{2-}^f$ |
| $(c,e,f):55$ | $R_T^{x'z}$ | $R_T^{z'z}$ | ${}^sR_{LT'}^{0y}$ | ${}^cR_{LT}^{00}$ | ${}^sR_{LT}^{0z}$ | ${}^cR_{LT'}^{0z}$ |
| | $\mathcal{O}_{1+}^c$ | $\mathcal{O}_{2+}^c$ | $\mathcal{O}_{1-}^e$ | $\mathcal{O}_{2+}^e$ | $\mathcal{O}_{1+}^f$ | $\mathcal{O}_{2+}^f$ |
| $(c,e,f):56$ | $R_T^{x'z}$ | $R_T^{z'z}$ | ${}^sR_{LT'}^{0y}$ | ${}^cR_{LT}^{00}$ | ${}^sR_{LT}^{0z}$ | ${}^sR_{LT}^{0x}$ |
| | $\mathcal{O}_{1+}^c$ | $\mathcal{O}_{2+}^c$ | $\mathcal{O}_{1-}^e$ | $\mathcal{O}_{2+}^e$ | $\mathcal{O}_{1+}^f$ | $\mathcal{O}_{2-}^f$ |
| $(c,e,f):57$ | $R_T^{x'z}$ | $R_T^{z'z}$ | ${}^sR_{LT'}^{0y}$ | ${}^cR_{LT}^{00}$ | ${}^cR_{LT'}^{0x}$ | ${}^cR_{LT'}^{0z}$ |
| | $\mathcal{O}_{1+}^c$ | $\mathcal{O}_{2+}^c$ | $\mathcal{O}_{1-}^e$ | $\mathcal{O}_{2+}^e$ | $\mathcal{O}_{1-}^f$ | $\mathcal{O}_{2+}^f$ |
| $(c,e,f):58$ | $R_T^{x'z}$ | $R_T^{z'z}$ | ${}^sR_{LT'}^{0y}$ | ${}^cR_{LT}^{00}$ | ${}^cR_{LT'}^{0x}$ | ${}^sR_{LT}^{0x}$ |
| | $\mathcal{O}_{1+}^c$ | $\mathcal{O}_{2+}^c$ | $\mathcal{O}_{1-}^e$ | $\mathcal{O}_{2+}^e$ | $\mathcal{O}_{1-}^f$ | $\mathcal{O}_{2-}^f$ |
| $(c,e,f):59$ | $R_T^{x'z}$ | $R_T^{z'z}$ | ${}^sR_{LT'}^{0y}$ | ${}^cR_{LT}^{0y}$ | ${}^sR_{LT}^{0z}$ | ${}^sR_{LT}^{0x}$ |
| | $\mathcal{O}_{1+}^c$ | $\mathcal{O}_{2+}^c$ | $\mathcal{O}_{1-}^e$ | $\mathcal{O}_{2-}^e$ | $\mathcal{O}_{1+}^f$ | $\mathcal{O}_{2-}^f$ |
| $(c,e,f):60$ | $R_T^{x'z}$ | $R_T^{z'z}$ | ${}^sR_{LT'}^{0y}$ | ${}^cR_{LT}^{0y}$ | ${}^cR_{LT'}^{0x}$ | ${}^cR_{LT'}^{0z}$ |
| | $\mathcal{O}_{1+}^c$ | $\mathcal{O}_{2+}^c$ | $\mathcal{O}_{1-}^e$ | $\mathcal{O}_{2-}^e$ | $\mathcal{O}_{1-}^f$ | $\mathcal{O}_{2+}^f$ |
| $(c,e,f):61$ | $R_T^{x'z}$ | $R_T^{x'x}$ | ${}^sR_{LT'}^{00}$ | ${}^sR_{LT'}^{0y}$ | ${}^sR_{LT}^{0z}$ | ${}^cR_{LT'}^{0x}$ |
| | $\mathcal{O}_{1+}^c$ | $\mathcal{O}_{2-}^c$ | $\mathcal{O}_{1+}^e$ | $\mathcal{O}_{1-}^e$ | $\mathcal{O}_{1+}^f$ | $\mathcal{O}_{1-}^f$ |
| $(c,e,f):62$ | $R_T^{x'z}$ | $R_T^{x'x}$ | ${}^sR_{LT'}^{00}$ | ${}^sR_{LT'}^{0y}$ | ${}^cR_{LT'}^{0z}$ | ${}^sR_{LT}^{0x}$ |
| | $\mathcal{O}_{1+}^c$ | $\mathcal{O}_{2-}^c$ | $\mathcal{O}_{1+}^e$ | $\mathcal{O}_{1-}^e$ | $\mathcal{O}_{2+}^f$ | $\mathcal{O}_{2-}^f$ |
| $(c,e,f):63$ | $R_T^{x'z}$ | $R_T^{x'x}$ | ${}^sR_{LT'}^{00}$ | ${}^sR_{LT'}^{0y}$ | ${}^sR_{LT}^{0z}$ | ${}^cR_{LT'}^{0z}$ |
| | $\mathcal{O}_{1+}^c$ | $\mathcal{O}_{2-}^c$ | $\mathcal{O}_{1+}^e$ | $\mathcal{O}_{1-}^e$ | $\mathcal{O}_{1+}^f$ | $\mathcal{O}_{2+}^f$ |
| $(c,e,f):64$ | $R_T^{x'z}$ | $R_T^{x'x}$ | ${}^sR_{LT'}^{00}$ | ${}^sR_{LT'}^{0y}$ | ${}^sR_{LT}^{0z}$ | ${}^sR_{LT}^{0x}$ |
| | $\mathcal{O}_{1+}^c$ | $\mathcal{O}_{2-}^c$ | $\mathcal{O}_{1+}^e$ | $\mathcal{O}_{1-}^e$ | $\mathcal{O}_{1+}^f$ | $\mathcal{O}_{2-}^f$ |
| $(c,e,f):65$ | $R_T^{x'z}$ | $R_T^{x'x}$ | ${}^sR_{LT'}^{00}$ | ${}^sR_{LT'}^{0y}$ | ${}^cR_{LT'}^{0x}$ | ${}^cR_{LT'}^{0z}$ |
| | $\mathcal{O}_{1+}^c$ | $\mathcal{O}_{2-}^c$ | $\mathcal{O}_{1+}^e$ | $\mathcal{O}_{1-}^e$ | $\mathcal{O}_{1-}^f$ | $\mathcal{O}_{2+}^f$ |
| $(c,e,f):66$ | $R_T^{x'z}$ | $R_T^{x'x}$ | ${}^sR_{LT'}^{00}$ | ${}^sR_{LT'}^{0y}$ | ${}^cR_{LT'}^{0x}$ | ${}^sR_{LT}^{0x}$ |
| | $\mathcal{O}_{1+}^c$ | $\mathcal{O}_{2-}^c$ | $\mathcal{O}_{1+}^e$ | $\mathcal{O}_{1-}^e$ | $\mathcal{O}_{1-}^f$ | $\mathcal{O}_{2-}^f$ |
| $(c,e,f):67$ | $R_T^{x'z}$ | $R_T^{x'x}$ | ${}^cR_{LT}^{00}$ | ${}^cR_{LT}^{0y}$ | ${}^sR_{LT}^{0z}$ | ${}^cR_{LT'}^{0x}$ |
| | $\mathcal{O}_{1+}^c$ | $\mathcal{O}_{2-}^c$ | $\mathcal{O}_{2+}^e$ | $\mathcal{O}_{2-}^e$ | $\mathcal{O}_{1+}^f$ | $\mathcal{O}_{1-}^f$ |
| $(c,e,f):68$ | $R_T^{x'z}$ | $R_T^{x'x}$ | ${}^cR_{LT}^{00}$ | ${}^cR_{LT}^{0y}$ | ${}^cR_{LT'}^{0z}$ | ${}^sR_{LT}^{0x}$ |
| | $\mathcal{O}_{1+}^c$ | $\mathcal{O}_{2-}^c$ | $\mathcal{O}_{2+}^e$ | $\mathcal{O}_{2-}^e$ | $\mathcal{O}_{2+}^f$ | $\mathcal{O}_{2-}^f$ |
| $(c,e,f):69$ | $R_T^{x'z}$ | $R_T^{x'x}$ | ${}^cR_{LT}^{00}$ | ${}^cR_{LT}^{0y}$ | ${}^sR_{LT}^{0z}$ | ${}^cR_{LT'}^{0z}$ |
| | $\mathcal{O}_{1+}^c$ | $\mathcal{O}_{2-}^c$ | $\mathcal{O}_{2+}^e$ | $\mathcal{O}_{2-}^e$ | $\mathcal{O}_{1+}^f$ | $\mathcal{O}_{2+}^f$ |
| $(c,e,f):70$ | $R_T^{x'z}$ | $R_T^{x'x}$ | ${}^cR_{LT}^{00}$ | ${}^cR_{LT}^{0y}$ | ${}^sR_{LT}^{0z}$ | ${}^sR_{LT}^{0x}$ |
| | $\mathcal{O}_{1+}^c$ | $\mathcal{O}_{2-}^c$ | $\mathcal{O}_{2+}^e$ | $\mathcal{O}_{2-}^e$ | $\mathcal{O}_{1+}^f$ | $\mathcal{O}_{2-}^f$ |
| $(c,e,f):71$ | $R_T^{x'z}$ | $R_T^{x'x}$ | ${}^cR_{LT}^{00}$ | ${}^cR_{LT}^{0y}$ | ${}^cR_{LT'}^{0x}$ | ${}^cR_{LT'}^{0z}$ |
| | $\mathcal{O}_{1+}^c$ | $\mathcal{O}_{2-}^c$ | $\mathcal{O}_{2+}^e$ | $\mathcal{O}_{2-}^e$ | $\mathcal{O}_{1-}^f$ | $\mathcal{O}_{2+}^f$ |
| $(c,e,f):72$ | $R_T^{x'z}$ | $R_T^{x'x}$ | ${}^cR_{LT}^{00}$ | ${}^cR_{LT}^{0y}$ | ${}^cR_{LT'}^{0x}$ | ${}^sR_{LT}^{0x}$ |
| | $\mathcal{O}_{1+}^c$ | $\mathcal{O}_{2-}^c$ | $\mathcal{O}_{2+}^e$ | $\mathcal{O}_{2-}^e$ | $\mathcal{O}_{1-}^f$ | $\mathcal{O}_{2-}^f$ |
| $(c,e,f):73$ | $R_T^{x'z}$ | $R_T^{x'x}$ | ${}^sR_{LT'}^{00}$ | ${}^cR_{LT}^{00}$ | ${}^sR_{LT}^{0z}$ | ${}^cR_{LT'}^{0x}$ |
| | $\mathcal{O}_{1+}^c$ | $\mathcal{O}_{2-}^c$ | $\mathcal{O}_{1+}^e$ | $\mathcal{O}_{2+}^e$ | $\mathcal{O}_{1+}^f$ | $\mathcal{O}_{1-}^f$ |
| $(c,e,f):74$ | $R_T^{x'z}$ | $R_T^{x'x}$ | ${}^sR_{LT'}^{00}$ | ${}^cR_{LT}^{00}$ | ${}^cR_{LT'}^{0z}$ | ${}^sR_{LT}^{0x}$ |
| | $\mathcal{O}_{1+}^c$ | $\mathcal{O}_{2-}^c$ | $\mathcal{O}_{1+}^e$ | $\mathcal{O}_{2+}^e$ | $\mathcal{O}_{2+}^f$ | $\mathcal{O}_{2-}^f$ |
| $(c,e,f):75$ | $R_T^{x'z}$ | $R_T^{x'x}$ | ${}^sR_{LT'}^{00}$ | ${}^cR_{LT}^{00}$ | ${}^sR_{LT}^{0z}$ | ${}^cR_{LT'}^{0z}$ |
| | $\mathcal{O}_{1+}^c$ | $\mathcal{O}_{2-}^c$ | $\mathcal{O}_{1+}^e$ | $\mathcal{O}_{2+}^e$ | $\mathcal{O}_{1+}^f$ | $\mathcal{O}_{2+}^f$ |
| $(c,e,f):76$ | $R_T^{x'z}$ | $R_T^{x'x}$ | ${}^sR_{LT'}^{00}$ | ${}^cR_{LT}^{00}$ | ${}^sR_{LT}^{0z}$ | ${}^sR_{LT}^{0x}$ |
| | $\mathcal{O}_{1+}^c$ | $\mathcal{O}_{2-}^c$ | $\mathcal{O}_{1+}^e$ | $\mathcal{O}_{2+}^e$ | $\mathcal{O}_{1+}^f$ | $\mathcal{O}_{2-}^f$ |
| $(c,e,f):77$ | $R_T^{x'z}$ | $R_T^{x'x}$ | ${}^sR_{LT'}^{00}$ | ${}^cR_{LT}^{00}$ | ${}^cR_{LT'}^{0x}$ | ${}^cR_{LT'}^{0z}$ |
| | $\mathcal{O}_{1+}^c$ | $\mathcal{O}_{2-}^c$ | $\mathcal{O}_{1+}^e$ | $\mathcal{O}_{2+}^e$ | $\mathcal{O}_{1-}^f$ | $\mathcal{O}_{2+}^f$ |
| $(c,e,f):78$ | $R_T^{x'z}$ | $R_T^{x'x}$ | ${}^sR_{LT'}^{00}$ | ${}^cR_{LT}^{00}$ | ${}^cR_{LT'}^{0x}$ | ${}^sR_{LT}^{0x}$ |

| | | | | | | |
|---|---|---|---|---|---|---|
| | $\mathcal{O}^c_{1+}$ | $\mathcal{O}^c_{2-}$ | $\mathcal{O}^e_{1+}$ | $\mathcal{O}^e_{2+}$ | $\mathcal{O}^f_{1-}$ | $\mathcal{O}^f_{2-}$ |
| $(c,e,f):79$ | $R_T^{x'z}$ | $R_T^{x'x}$ | ${}^sR^{00}_{LT'}$ | ${}^cR^{0y}_{LT}$ | ${}^sR^{0z}_{LT}$ | ${}^cR^{0x}_{LT'}$ |
| | $\mathcal{O}^c_{1+}$ | $\mathcal{O}^c_{2-}$ | $\mathcal{O}^e_{1+}$ | $\mathcal{O}^e_{2-}$ | $\mathcal{O}^f_{1+}$ | $\mathcal{O}^f_{1-}$ |
| $(c,e,f):80$ | $R_T^{x'z}$ | $R_T^{x'x}$ | ${}^sR^{00}_{LT'}$ | ${}^cR^{0y}_{LT}$ | ${}^cR^{0z}_{LT'}$ | ${}^sR^{0x}_{LT}$ |
| | $\mathcal{O}^c_{1+}$ | $\mathcal{O}^c_{2-}$ | $\mathcal{O}^e_{1+}$ | $\mathcal{O}^e_{2-}$ | $\mathcal{O}^f_{2+}$ | $\mathcal{O}^f_{2-}$ |
| $(c,e,f):81$ | $R_T^{x'z}$ | $R_T^{x'x}$ | ${}^sR^{00}_{LT'}$ | ${}^cR^{0y}_{LT}$ | ${}^sR^{0z}_{LT}$ | ${}^cR^{0z}_{LT'}$ |
| | $\mathcal{O}^c_{1+}$ | $\mathcal{O}^c_{2-}$ | $\mathcal{O}^e_{1+}$ | $\mathcal{O}^e_{2-}$ | $\mathcal{O}^f_{1+}$ | $\mathcal{O}^f_{2+}$ |
| $(c,e,f):82$ | $R_T^{x'z}$ | $R_T^{x'x}$ | ${}^sR^{00}_{LT'}$ | ${}^cR^{0y}_{LT}$ | ${}^sR^{0z}_{LT}$ | ${}^sR^{0x}_{LT}$ |
| | $\mathcal{O}^c_{1+}$ | $\mathcal{O}^c_{2-}$ | $\mathcal{O}^e_{1+}$ | $\mathcal{O}^e_{2-}$ | $\mathcal{O}^f_{1+}$ | $\mathcal{O}^f_{2-}$ |
| $(c,e,f):83$ | $R_T^{x'z}$ | $R_T^{x'x}$ | ${}^sR^{00}_{LT'}$ | ${}^cR^{0y}_{LT}$ | ${}^cR^{0x}_{LT'}$ | ${}^cR^{0z}_{LT'}$ |
| | $\mathcal{O}^c_{1+}$ | $\mathcal{O}^c_{2-}$ | $\mathcal{O}^e_{1+}$ | $\mathcal{O}^e_{2-}$ | $\mathcal{O}^f_{1-}$ | $\mathcal{O}^f_{2+}$ |
| $(c,e,f):84$ | $R_T^{x'z}$ | $R_T^{x'x}$ | ${}^sR^{00}_{LT'}$ | ${}^cR^{0y}_{LT}$ | ${}^cR^{0x}_{LT'}$ | ${}^sR^{0x}_{LT}$ |
| | $\mathcal{O}^c_{1+}$ | $\mathcal{O}^c_{2-}$ | $\mathcal{O}^e_{1+}$ | $\mathcal{O}^e_{2-}$ | $\mathcal{O}^f_{1-}$ | $\mathcal{O}^f_{2-}$ |
| $(c,e,f):85$ | $R_T^{x'z}$ | $R_T^{x'x}$ | ${}^sR^{0y}_{LT'}$ | ${}^cR^{00}_{LT}$ | ${}^sR^{0z}_{LT}$ | ${}^cR^{0x}_{LT'}$ |
| | $\mathcal{O}^c_{1+}$ | $\mathcal{O}^c_{2-}$ | $\mathcal{O}^e_{1-}$ | $\mathcal{O}^e_{2+}$ | $\mathcal{O}^f_{1+}$ | $\mathcal{O}^f_{1-}$ |
| $(c,e,f):86$ | $R_T^{x'z}$ | $R_T^{x'x}$ | ${}^sR^{0y}_{LT'}$ | ${}^cR^{00}_{LT}$ | ${}^cR^{0z}_{LT'}$ | ${}^sR^{0x}_{LT}$ |
| | $\mathcal{O}^c_{1+}$ | $\mathcal{O}^c_{2-}$ | $\mathcal{O}^e_{1-}$ | $\mathcal{O}^e_{2+}$ | $\mathcal{O}^f_{2+}$ | $\mathcal{O}^f_{2-}$ |
| $(c,e,f):87$ | $R_T^{x'z}$ | $R_T^{x'x}$ | ${}^sR^{0y}_{LT'}$ | ${}^cR^{00}_{LT}$ | ${}^sR^{0z}_{LT}$ | ${}^cR^{0z}_{LT'}$ |
| | $\mathcal{O}^c_{1+}$ | $\mathcal{O}^c_{2-}$ | $\mathcal{O}^e_{1-}$ | $\mathcal{O}^e_{2+}$ | $\mathcal{O}^f_{1+}$ | $\mathcal{O}^f_{2+}$ |
| $(c,e,f):88$ | $R_T^{x'z}$ | $R_T^{x'x}$ | ${}^sR^{0y}_{LT'}$ | ${}^cR^{00}_{LT}$ | ${}^sR^{0z}_{LT}$ | ${}^sR^{0x}_{LT}$ |
| | $\mathcal{O}^c_{1+}$ | $\mathcal{O}^c_{2-}$ | $\mathcal{O}^e_{1-}$ | $\mathcal{O}^e_{2+}$ | $\mathcal{O}^f_{1+}$ | $\mathcal{O}^f_{2-}$ |
| $(c,e,f):89$ | $R_T^{x'z}$ | $R_T^{x'x}$ | ${}^sR^{0y}_{LT'}$ | ${}^cR^{00}_{LT}$ | ${}^cR^{0x}_{LT'}$ | ${}^cR^{0z}_{LT'}$ |
| | $\mathcal{O}^c_{1+}$ | $\mathcal{O}^c_{2-}$ | $\mathcal{O}^e_{1-}$ | $\mathcal{O}^e_{2+}$ | $\mathcal{O}^f_{1-}$ | $\mathcal{O}^f_{2+}$ |
| $(c,e,f):90$ | $R_T^{x'z}$ | $R_T^{x'x}$ | ${}^sR^{0y}_{LT'}$ | ${}^cR^{00}_{LT}$ | ${}^cR^{0x}_{LT'}$ | ${}^sR^{0x}_{LT}$ |
| | $\mathcal{O}^c_{1+}$ | $\mathcal{O}^c_{2-}$ | $\mathcal{O}^e_{1-}$ | $\mathcal{O}^e_{2+}$ | $\mathcal{O}^f_{1-}$ | $\mathcal{O}^f_{2-}$ |
| $(c,e,f):91$ | $R_T^{x'z}$ | $R_T^{x'x}$ | ${}^sR^{0y}_{LT'}$ | ${}^cR^{0y}_{LT}$ | ${}^sR^{0z}_{LT}$ | ${}^cR^{0x}_{LT'}$ |
| | $\mathcal{O}^c_{1+}$ | $\mathcal{O}^c_{2-}$ | $\mathcal{O}^e_{1-}$ | $\mathcal{O}^e_{2-}$ | $\mathcal{O}^f_{1+}$ | $\mathcal{O}^f_{1-}$ |
| $(c,e,f):92$ | $R_T^{x'z}$ | $R_T^{x'x}$ | ${}^sR^{0y}_{LT'}$ | ${}^cR^{0y}_{LT}$ | ${}^cR^{0z}_{LT'}$ | ${}^sR^{0x}_{LT}$ |
| | $\mathcal{O}^c_{1+}$ | $\mathcal{O}^c_{2-}$ | $\mathcal{O}^e_{1-}$ | $\mathcal{O}^e_{2-}$ | $\mathcal{O}^f_{2+}$ | $\mathcal{O}^f_{2-}$ |
| $(c,e,f):93$ | $R_T^{x'z}$ | $R_T^{x'x}$ | ${}^sR^{0y}_{LT'}$ | ${}^cR^{0y}_{LT}$ | ${}^sR^{0z}_{LT}$ | ${}^cR^{0z}_{LT'}$ |
| | $\mathcal{O}^c_{1+}$ | $\mathcal{O}^c_{2-}$ | $\mathcal{O}^e_{1-}$ | $\mathcal{O}^e_{2-}$ | $\mathcal{O}^f_{1+}$ | $\mathcal{O}^f_{2+}$ |
| $(c,e,f):94$ | $R_T^{x'z}$ | $R_T^{x'x}$ | ${}^sR^{0y}_{LT'}$ | ${}^cR^{0y}_{LT}$ | ${}^sR^{0z}_{LT}$ | ${}^sR^{0x}_{LT}$ |
| | $\mathcal{O}^c_{1+}$ | $\mathcal{O}^c_{2-}$ | $\mathcal{O}^e_{1-}$ | $\mathcal{O}^e_{2-}$ | $\mathcal{O}^f_{1+}$ | $\mathcal{O}^f_{2-}$ |
| $(c,e,f):95$ | $R_T^{x'z}$ | $R_T^{x'x}$ | ${}^sR^{0y}_{LT'}$ | ${}^cR^{0y}_{LT}$ | ${}^cR^{0x}_{LT'}$ | ${}^cR^{0z}_{LT'}$ |
| | $\mathcal{O}^c_{1+}$ | $\mathcal{O}^c_{2-}$ | $\mathcal{O}^e_{1-}$ | $\mathcal{O}^e_{2-}$ | $\mathcal{O}^f_{1-}$ | $\mathcal{O}^f_{2+}$ |
| $(c,e,f):96$ | $R_T^{x'z}$ | $R_T^{x'x}$ | ${}^sR^{0y}_{LT'}$ | ${}^cR^{0y}_{LT}$ | ${}^cR^{0x}_{LT'}$ | ${}^sR^{0x}_{LT}$ |
| | $\mathcal{O}^c_{1+}$ | $\mathcal{O}^c_{2-}$ | $\mathcal{O}^e_{1-}$ | $\mathcal{O}^e_{2-}$ | $\mathcal{O}^f_{1-}$ | $\mathcal{O}^f_{2-}$ |
| $(c,e,f):97$ | $R_T^{z'x}$ | $R_T^{z'z}$ | ${}^sR^{00}_{LT'}$ | ${}^sR^{0y}_{LT'}$ | ${}^sR^{0z}_{LT}$ | ${}^cR^{0x}_{LT'}$ |
| | $\mathcal{O}^c_{1-}$ | $\mathcal{O}^c_{2+}$ | $\mathcal{O}^e_{1+}$ | $\mathcal{O}^e_{1-}$ | $\mathcal{O}^f_{1+}$ | $\mathcal{O}^f_{1-}$ |
| $(c,e,f):98$ | $R_T^{z'x}$ | $R_T^{z'z}$ | ${}^sR^{00}_{LT'}$ | ${}^sR^{0y}_{LT'}$ | ${}^cR^{0z}_{LT'}$ | ${}^sR^{0x}_{LT}$ |
| | $\mathcal{O}^c_{1-}$ | $\mathcal{O}^c_{2+}$ | $\mathcal{O}^e_{1+}$ | $\mathcal{O}^e_{1-}$ | $\mathcal{O}^f_{2+}$ | $\mathcal{O}^f_{2-}$ |
| $(c,e,f):99$ | $R_T^{z'x}$ | $R_T^{z'z}$ | ${}^sR^{00}_{LT'}$ | ${}^sR^{0y}_{LT'}$ | ${}^sR^{0z}_{LT}$ | ${}^cR^{0z}_{LT'}$ |
| | $\mathcal{O}^c_{1-}$ | $\mathcal{O}^c_{2+}$ | $\mathcal{O}^e_{1+}$ | $\mathcal{O}^e_{1-}$ | $\mathcal{O}^f_{1+}$ | $\mathcal{O}^f_{2+}$ |
| $(c,e,f):100$ | $R_T^{z'x}$ | $R_T^{z'z}$ | ${}^sR^{00}_{LT'}$ | ${}^sR^{0y}_{LT'}$ | ${}^sR^{0z}_{LT}$ | ${}^sR^{0x}_{LT}$ |
| | $\mathcal{O}^c_{1-}$ | $\mathcal{O}^c_{2+}$ | $\mathcal{O}^e_{1+}$ | $\mathcal{O}^e_{1-}$ | $\mathcal{O}^f_{1+}$ | $\mathcal{O}^f_{2-}$ |
| $(c,e,f):101$ | $R_T^{z'x}$ | $R_T^{z'z}$ | ${}^sR^{00}_{LT'}$ | ${}^sR^{0y}_{LT'}$ | ${}^cR^{0x}_{LT'}$ | ${}^cR^{0z}_{LT'}$ |
| | $\mathcal{O}^c_{1-}$ | $\mathcal{O}^c_{2+}$ | $\mathcal{O}^e_{1+}$ | $\mathcal{O}^e_{1-}$ | $\mathcal{O}^f_{1-}$ | $\mathcal{O}^f_{2+}$ |
| $(c,e,f):102$ | $R_T^{z'x}$ | $R_T^{z'z}$ | ${}^sR^{00}_{LT'}$ | ${}^sR^{0y}_{LT'}$ | ${}^cR^{0x}_{LT'}$ | ${}^sR^{0x}_{LT}$ |
| | $\mathcal{O}^c_{1-}$ | $\mathcal{O}^c_{2+}$ | $\mathcal{O}^e_{1+}$ | $\mathcal{O}^e_{1-}$ | $\mathcal{O}^f_{1-}$ | $\mathcal{O}^f_{2-}$ |
| $(c,e,f):103$ | $R_T^{z'x}$ | $R_T^{z'z}$ | ${}^cR^{00}_{LT}$ | ${}^cR^{0y}_{LT}$ | ${}^sR^{0z}_{LT}$ | ${}^cR^{0x}_{LT'}$ |
| | $\mathcal{O}^c_{1-}$ | $\mathcal{O}^c_{2+}$ | $\mathcal{O}^e_{2+}$ | $\mathcal{O}^e_{2-}$ | $\mathcal{O}^f_{1+}$ | $\mathcal{O}^f_{1-}$ |
| $(c,e,f):104$ | $R_T^{z'x}$ | $R_T^{z'z}$ | ${}^cR^{00}_{LT}$ | ${}^cR^{0y}_{LT}$ | ${}^cR^{0z}_{LT'}$ | ${}^sR^{0x}_{LT}$ |
| | $\mathcal{O}^c_{1-}$ | $\mathcal{O}^c_{2+}$ | $\mathcal{O}^e_{2+}$ | $\mathcal{O}^e_{2-}$ | $\mathcal{O}^f_{2+}$ | $\mathcal{O}^f_{2-}$ |
| $(c,e,f):105$ | $R_T^{z'x}$ | $R_T^{z'z}$ | ${}^cR^{00}_{LT}$ | ${}^cR^{0y}_{LT}$ | ${}^sR^{0z}_{LT}$ | ${}^cR^{0z}_{LT'}$ |
| | $\mathcal{O}^c_{1-}$ | $\mathcal{O}^c_{2+}$ | $\mathcal{O}^e_{2+}$ | $\mathcal{O}^e_{2-}$ | $\mathcal{O}^f_{1+}$ | $\mathcal{O}^f_{2+}$ |

| | | | | | | |
|---|---|---|---|---|---|---|
| $(c,e,f):106$ | $R_T^{z'x}$ | $R_T^{z'z}$ | ${}^cR_{LT}^{00}$ | ${}^cR_{LT}^{0y}$ | ${}^sR_{LT}^{0z}$ | ${}^sR_{LT}^{0x}$ |
| | $\mathcal{O}_{1-}^c$ | $\mathcal{O}_{2+}^c$ | $\mathcal{O}_{2+}^e$ | $\mathcal{O}_{2-}^e$ | $\mathcal{O}_{1+}^f$ | $\mathcal{O}_{2-}^f$ |
| $(c,e,f):107$ | $R_T^{z'x}$ | $R_T^{z'z}$ | ${}^cR_{LT}^{00}$ | ${}^cR_{LT}^{0y}$ | ${}^cR_{LT'}^{0x}$ | ${}^cR_{LT'}^{0z}$ |
| | $\mathcal{O}_{1-}^c$ | $\mathcal{O}_{2+}^c$ | $\mathcal{O}_{2+}^e$ | $\mathcal{O}_{2-}^e$ | $\mathcal{O}_{1-}^f$ | $\mathcal{O}_{2+}^f$ |
| $(c,e,f):108$ | $R_T^{z'x}$ | $R_T^{z'z}$ | ${}^cR_{LT}^{00}$ | ${}^cR_{LT}^{0y}$ | ${}^cR_{LT'}^{0x}$ | ${}^sR_{LT}^{0x}$ |
| | $\mathcal{O}_{1-}^c$ | $\mathcal{O}_{2+}^c$ | $\mathcal{O}_{2+}^e$ | $\mathcal{O}_{2-}^e$ | $\mathcal{O}_{1-}^f$ | $\mathcal{O}_{2-}^f$ |
| $(c,e,f):109$ | $R_T^{z'x}$ | $R_T^{z'z}$ | ${}^sR_{LT'}^{00}$ | ${}^cR_{LT}^{00}$ | ${}^sR_{LT}^{0z}$ | ${}^cR_{LT'}^{0x}$ |
| | $\mathcal{O}_{1-}^c$ | $\mathcal{O}_{2+}^c$ | $\mathcal{O}_{1+}^e$ | $\mathcal{O}_{2+}^e$ | $\mathcal{O}_{1+}^f$ | $\mathcal{O}_{1-}^f$ |
| $(c,e,f):110$ | $R_T^{z'x}$ | $R_T^{z'z}$ | ${}^sR_{LT'}^{00}$ | ${}^cR_{LT}^{00}$ | ${}^cR_{LT'}^{0z}$ | ${}^sR_{LT}^{0x}$ |
| | $\mathcal{O}_{1-}^c$ | $\mathcal{O}_{2+}^c$ | $\mathcal{O}_{1+}^e$ | $\mathcal{O}_{2+}^e$ | $\mathcal{O}_{2+}^f$ | $\mathcal{O}_{2-}^f$ |
| $(c,e,f):111$ | $R_T^{z'x}$ | $R_T^{z'z}$ | ${}^sR_{LT'}^{00}$ | ${}^cR_{LT}^{00}$ | ${}^sR_{LT}^{0z}$ | ${}^cR_{LT'}^{0z}$ |
| | $\mathcal{O}_{1-}^c$ | $\mathcal{O}_{2+}^c$ | $\mathcal{O}_{1+}^e$ | $\mathcal{O}_{2+}^e$ | $\mathcal{O}_{1+}^f$ | $\mathcal{O}_{2+}^f$ |
| $(c,e,f):112$ | $R_T^{z'x}$ | $R_T^{z'z}$ | ${}^sR_{LT'}^{00}$ | ${}^cR_{LT}^{00}$ | ${}^sR_{LT}^{0z}$ | ${}^sR_{LT}^{0x}$ |
| | $\mathcal{O}_{1-}^c$ | $\mathcal{O}_{2+}^c$ | $\mathcal{O}_{1+}^e$ | $\mathcal{O}_{2+}^e$ | $\mathcal{O}_{1+}^f$ | $\mathcal{O}_{2-}^f$ |
| $(c,e,f):113$ | $R_T^{z'x}$ | $R_T^{z'z}$ | ${}^sR_{LT'}^{00}$ | ${}^cR_{LT}^{00}$ | ${}^cR_{LT'}^{0x}$ | ${}^cR_{LT'}^{0z}$ |
| | $\mathcal{O}_{1-}^c$ | $\mathcal{O}_{2+}^c$ | $\mathcal{O}_{1+}^e$ | $\mathcal{O}_{2+}^e$ | $\mathcal{O}_{1-}^f$ | $\mathcal{O}_{2+}^f$ |
| $(c,e,f):114$ | $R_T^{z'x}$ | $R_T^{z'z}$ | ${}^sR_{LT'}^{00}$ | ${}^cR_{LT}^{00}$ | ${}^cR_{LT'}^{0x}$ | ${}^sR_{LT}^{0x}$ |
| | $\mathcal{O}_{1-}^c$ | $\mathcal{O}_{2+}^c$ | $\mathcal{O}_{1+}^e$ | $\mathcal{O}_{2+}^e$ | $\mathcal{O}_{1-}^f$ | $\mathcal{O}_{2-}^f$ |
| $(c,e,f):115$ | $R_T^{z'x}$ | $R_T^{z'z}$ | ${}^sR_{LT'}^{00}$ | ${}^cR_{LT}^{0y}$ | ${}^sR_{LT}^{0z}$ | ${}^cR_{LT'}^{0x}$ |
| | $\mathcal{O}_{1-}^c$ | $\mathcal{O}_{2+}^c$ | $\mathcal{O}_{1+}^e$ | $\mathcal{O}_{2-}^e$ | $\mathcal{O}_{1+}^f$ | $\mathcal{O}_{1-}^f$ |
| $(c,e,f):116$ | $R_T^{z'x}$ | $R_T^{z'z}$ | ${}^sR_{LT'}^{00}$ | ${}^cR_{LT}^{0y}$ | ${}^cR_{LT'}^{0z}$ | ${}^sR_{LT}^{0x}$ |
| | $\mathcal{O}_{1-}^c$ | $\mathcal{O}_{2+}^c$ | $\mathcal{O}_{1+}^e$ | $\mathcal{O}_{2-}^e$ | $\mathcal{O}_{2+}^f$ | $\mathcal{O}_{2-}^f$ |
| $(c,e,f):117$ | $R_T^{z'x}$ | $R_T^{z'z}$ | ${}^sR_{LT'}^{00}$ | ${}^cR_{LT}^{0y}$ | ${}^sR_{LT}^{0z}$ | ${}^cR_{LT'}^{0z}$ |
| | $\mathcal{O}_{1-}^c$ | $\mathcal{O}_{2+}^c$ | $\mathcal{O}_{1+}^e$ | $\mathcal{O}_{2-}^e$ | $\mathcal{O}_{1+}^f$ | $\mathcal{O}_{2+}^f$ |
| $(c,e,f):118$ | $R_T^{z'x}$ | $R_T^{z'z}$ | ${}^sR_{LT'}^{00}$ | ${}^cR_{LT}^{0y}$ | ${}^sR_{LT}^{0z}$ | ${}^sR_{LT}^{0x}$ |
| | $\mathcal{O}_{1-}^c$ | $\mathcal{O}_{2+}^c$ | $\mathcal{O}_{1+}^e$ | $\mathcal{O}_{2-}^e$ | $\mathcal{O}_{1+}^f$ | $\mathcal{O}_{2-}^f$ |
| $(c,e,f):119$ | $R_T^{z'x}$ | $R_T^{z'z}$ | ${}^sR_{LT'}^{00}$ | ${}^cR_{LT}^{0y}$ | ${}^cR_{LT'}^{0x}$ | ${}^cR_{LT'}^{0z}$ |
| | $\mathcal{O}_{1-}^c$ | $\mathcal{O}_{2+}^c$ | $\mathcal{O}_{1+}^e$ | $\mathcal{O}_{2-}^e$ | $\mathcal{O}_{1-}^f$ | $\mathcal{O}_{2+}^f$ |
| $(c,e,f):120$ | $R_T^{z'x}$ | $R_T^{z'z}$ | ${}^sR_{LT'}^{00}$ | ${}^cR_{LT}^{0y}$ | ${}^cR_{LT'}^{0x}$ | ${}^sR_{LT}^{0x}$ |
| | $\mathcal{O}_{1-}^c$ | $\mathcal{O}_{2+}^c$ | $\mathcal{O}_{1+}^e$ | $\mathcal{O}_{2-}^e$ | $\mathcal{O}_{1-}^f$ | $\mathcal{O}_{2-}^f$ |
| $(c,e,f):121$ | $R_T^{z'x}$ | $R_T^{z'z}$ | ${}^sR_{LT'}^{0y}$ | ${}^cR_{LT}^{00}$ | ${}^sR_{LT}^{0z}$ | ${}^cR_{LT'}^{0x}$ |
| | $\mathcal{O}_{1-}^c$ | $\mathcal{O}_{2+}^c$ | $\mathcal{O}_{1-}^e$ | $\mathcal{O}_{2+}^e$ | $\mathcal{O}_{1+}^f$ | $\mathcal{O}_{1-}^f$ |
| $(c,e,f):122$ | $R_T^{z'x}$ | $R_T^{z'z}$ | ${}^sR_{LT'}^{0y}$ | ${}^cR_{LT}^{00}$ | ${}^cR_{LT'}^{0z}$ | ${}^sR_{LT}^{0x}$ |
| | $\mathcal{O}_{1-}^c$ | $\mathcal{O}_{2+}^c$ | $\mathcal{O}_{1-}^e$ | $\mathcal{O}_{2+}^e$ | $\mathcal{O}_{2+}^f$ | $\mathcal{O}_{2-}^f$ |
| $(c,e,f):123$ | $R_T^{z'x}$ | $R_T^{z'z}$ | ${}^sR_{LT'}^{0y}$ | ${}^cR_{LT}^{00}$ | ${}^sR_{LT}^{0z}$ | ${}^cR_{LT'}^{0z}$ |
| | $\mathcal{O}_{1-}^c$ | $\mathcal{O}_{2+}^c$ | $\mathcal{O}_{1-}^e$ | $\mathcal{O}_{2+}^e$ | $\mathcal{O}_{1+}^f$ | $\mathcal{O}_{2+}^f$ |
| $(c,e,f):124$ | $R_T^{z'x}$ | $R_T^{z'z}$ | ${}^sR_{LT'}^{0y}$ | ${}^cR_{LT}^{00}$ | ${}^sR_{LT}^{0z}$ | ${}^sR_{LT}^{0x}$ |
| | $\mathcal{O}_{1-}^c$ | $\mathcal{O}_{2+}^c$ | $\mathcal{O}_{1-}^e$ | $\mathcal{O}_{2+}^e$ | $\mathcal{O}_{1+}^f$ | $\mathcal{O}_{2-}^f$ |
| $(c,e,f):125$ | $R_T^{z'x}$ | $R_T^{z'z}$ | ${}^sR_{LT'}^{0y}$ | ${}^cR_{LT}^{00}$ | ${}^cR_{LT'}^{0x}$ | ${}^cR_{LT'}^{0z}$ |
| | $\mathcal{O}_{1-}^c$ | $\mathcal{O}_{2+}^c$ | $\mathcal{O}_{1-}^e$ | $\mathcal{O}_{2+}^e$ | $\mathcal{O}_{1-}^f$ | $\mathcal{O}_{2+}^f$ |
| $(c,e,f):126$ | $R_T^{z'x}$ | $R_T^{z'z}$ | ${}^sR_{LT'}^{0y}$ | ${}^cR_{LT}^{00}$ | ${}^cR_{LT'}^{0x}$ | ${}^sR_{LT}^{0x}$ |
| | $\mathcal{O}_{1-}^c$ | $\mathcal{O}_{2+}^c$ | $\mathcal{O}_{1-}^e$ | $\mathcal{O}_{2+}^e$ | $\mathcal{O}_{1-}^f$ | $\mathcal{O}_{2-}^f$ |
| $(c,e,f):127$ | $R_T^{z'x}$ | $R_T^{z'z}$ | ${}^sR_{LT'}^{0y}$ | ${}^cR_{LT}^{0y}$ | ${}^sR_{LT}^{0z}$ | ${}^cR_{LT'}^{0x}$ |
| | $\mathcal{O}_{1-}^c$ | $\mathcal{O}_{2+}^c$ | $\mathcal{O}_{1-}^e$ | $\mathcal{O}_{2-}^e$ | $\mathcal{O}_{1+}^f$ | $\mathcal{O}_{1-}^f$ |
| $(c,e,f):128$ | $R_T^{z'x}$ | $R_T^{z'z}$ | ${}^sR_{LT'}^{0y}$ | ${}^cR_{LT}^{0y}$ | ${}^cR_{LT'}^{0z}$ | ${}^sR_{LT}^{0x}$ |
| | $\mathcal{O}_{1-}^c$ | $\mathcal{O}_{2+}^c$ | $\mathcal{O}_{1-}^e$ | $\mathcal{O}_{2-}^e$ | $\mathcal{O}_{2+}^f$ | $\mathcal{O}_{2-}^f$ |
| $(c,e,f):129$ | $R_T^{z'x}$ | $R_T^{z'z}$ | ${}^sR_{LT'}^{0y}$ | ${}^cR_{LT}^{0y}$ | ${}^sR_{LT}^{0z}$ | ${}^cR_{LT'}^{0z}$ |
| | $\mathcal{O}_{1-}^c$ | $\mathcal{O}_{2+}^c$ | $\mathcal{O}_{1-}^e$ | $\mathcal{O}_{2-}^e$ | $\mathcal{O}_{1+}^f$ | $\mathcal{O}_{2+}^f$ |
| $(c,e,f):130$ | $R_T^{z'x}$ | $R_T^{z'z}$ | ${}^sR_{LT'}^{0y}$ | ${}^cR_{LT}^{0y}$ | ${}^sR_{LT}^{0z}$ | ${}^sR_{LT}^{0x}$ |
| | $\mathcal{O}_{1-}^c$ | $\mathcal{O}_{2+}^c$ | $\mathcal{O}_{1-}^e$ | $\mathcal{O}_{2-}^e$ | $\mathcal{O}_{1+}^f$ | $\mathcal{O}_{2-}^f$ |
| $(c,e,f):131$ | $R_T^{z'x}$ | $R_T^{z'z}$ | ${}^sR_{LT'}^{0y}$ | ${}^cR_{LT}^{0y}$ | ${}^cR_{LT'}^{0x}$ | ${}^cR_{LT'}^{0z}$ |
| | $\mathcal{O}_{1-}^c$ | $\mathcal{O}_{2+}^c$ | $\mathcal{O}_{1-}^e$ | $\mathcal{O}_{2-}^e$ | $\mathcal{O}_{1-}^f$ | $\mathcal{O}_{2+}^f$ |
| $(c,e,f):132$ | $R_T^{z'x}$ | $R_T^{z'z}$ | ${}^sR_{LT'}^{0y}$ | ${}^cR_{LT}^{0y}$ | ${}^cR_{LT'}^{0x}$ | ${}^sR_{LT}^{0x}$ |
| | $\mathcal{O}_{1-}^c$ | $\mathcal{O}_{2+}^c$ | $\mathcal{O}_{1-}^e$ | $\mathcal{O}_{2-}^e$ | $\mathcal{O}_{1-}^f$ | $\mathcal{O}_{2-}^f$ |
| $(c,e,f):133$ | $R_T^{z'x}$ | $R_T^{x'x}$ | ${}^sR_{LT'}^{00}$ | ${}^sR_{LT'}^{0y}$ | ${}^sR_{LT}^{0z}$ | ${}^sR_{LT}^{0x}$ |

| | | | | | | |
|---|---|---|---|---|---|---|
| | $\mathcal{O}^c_{1-}$ | $\mathcal{O}^c_{2-}$ | $\mathcal{O}^e_{1+}$ | $\mathcal{O}^e_{1-}$ | $\mathcal{O}^f_{1+}$ | $\mathcal{O}^f_{2-}$ |
| $(c,e,f):134$ | $R_T^{z'x}$ | $R_T^{x'x}$ | ${}^sR_{LT'}^{00}$ | ${}^sR_{LT'}^{0y}$ | ${}^cR_{LT'}^{0x}$ | ${}^cR_{LT'}^{0z}$ |
| | $\mathcal{O}^c_{1-}$ | $\mathcal{O}^c_{2-}$ | $\mathcal{O}^e_{1+}$ | $\mathcal{O}^e_{1-}$ | $\mathcal{O}^f_{1-}$ | $\mathcal{O}^f_{2+}$ |
| $(c,e,f):135$ | $R_T^{z'x}$ | $R_T^{x'x}$ | ${}^cR_{LT}^{00}$ | ${}^cR_{LT}^{0y}$ | ${}^sR_{LT}^{0z}$ | ${}^sR_{LT}^{0x}$ |
| | $\mathcal{O}^c_{1-}$ | $\mathcal{O}^c_{2-}$ | $\mathcal{O}^e_{2+}$ | $\mathcal{O}^e_{2-}$ | $\mathcal{O}^f_{1+}$ | $\mathcal{O}^f_{2-}$ |
| $(c,e,f):136$ | $R_T^{z'x}$ | $R_T^{x'x}$ | ${}^cR_{LT}^{00}$ | ${}^cR_{LT}^{0y}$ | ${}^cR_{LT'}^{0x}$ | ${}^cR_{LT'}^{0z}$ |
| | $\mathcal{O}^c_{1-}$ | $\mathcal{O}^c_{2-}$ | $\mathcal{O}^e_{2+}$ | $\mathcal{O}^e_{2-}$ | $\mathcal{O}^f_{1-}$ | $\mathcal{O}^f_{2+}$ |
| $(c,e,f):137$ | $R_T^{z'x}$ | $R_T^{x'x}$ | ${}^sR_{LT'}^{00}$ | ${}^cR_{LT}^{00}$ | ${}^sR_{LT}^{0z}$ | ${}^sR_{LT}^{0x}$ |
| | $\mathcal{O}^c_{1-}$ | $\mathcal{O}^c_{2-}$ | $\mathcal{O}^e_{1+}$ | $\mathcal{O}^e_{2+}$ | $\mathcal{O}^f_{1+}$ | $\mathcal{O}^f_{2-}$ |
| $(c,e,f):138$ | $R_T^{z'x}$ | $R_T^{x'x}$ | ${}^sR_{LT'}^{00}$ | ${}^cR_{LT}^{00}$ | ${}^cR_{LT'}^{0x}$ | ${}^cR_{LT'}^{0z}$ |
| | $\mathcal{O}^c_{1-}$ | $\mathcal{O}^c_{2-}$ | $\mathcal{O}^e_{1+}$ | $\mathcal{O}^e_{2+}$ | $\mathcal{O}^f_{1-}$ | $\mathcal{O}^f_{2+}$ |
| $(c,e,f):139$ | $R_T^{z'x}$ | $R_T^{x'x}$ | ${}^sR_{LT'}^{00}$ | ${}^cR_{LT}^{0y}$ | ${}^sR_{LT}^{0z}$ | ${}^cR_{LT'}^{0x}$ |
| | $\mathcal{O}^c_{1-}$ | $\mathcal{O}^c_{2-}$ | $\mathcal{O}^e_{1+}$ | $\mathcal{O}^e_{2-}$ | $\mathcal{O}^f_{1+}$ | $\mathcal{O}^f_{1-}$ |
| $(c,e,f):140$ | $R_T^{z'x}$ | $R_T^{x'x}$ | ${}^sR_{LT'}^{00}$ | ${}^cR_{LT}^{0y}$ | ${}^cR_{LT'}^{0z}$ | ${}^sR_{LT}^{0x}$ |
| | $\mathcal{O}^c_{1-}$ | $\mathcal{O}^c_{2-}$ | $\mathcal{O}^e_{1+}$ | $\mathcal{O}^e_{2-}$ | $\mathcal{O}^f_{2+}$ | $\mathcal{O}^f_{2-}$ |
| $(c,e,f):141$ | $R_T^{z'x}$ | $R_T^{x'x}$ | ${}^sR_{LT'}^{00}$ | ${}^cR_{LT}^{0y}$ | ${}^sR_{LT}^{0z}$ | ${}^cR_{LT'}^{0z}$ |
| | $\mathcal{O}^c_{1-}$ | $\mathcal{O}^c_{2-}$ | $\mathcal{O}^e_{1+}$ | $\mathcal{O}^e_{2-}$ | $\mathcal{O}^f_{1+}$ | $\mathcal{O}^f_{2+}$ |
| $(c,e,f):142$ | $R_T^{z'x}$ | $R_T^{x'x}$ | ${}^sR_{LT'}^{00}$ | ${}^cR_{LT}^{0y}$ | ${}^sR_{LT}^{0z}$ | ${}^sR_{LT}^{0x}$ |
| | $\mathcal{O}^c_{1-}$ | $\mathcal{O}^c_{2-}$ | $\mathcal{O}^e_{1+}$ | $\mathcal{O}^e_{2-}$ | $\mathcal{O}^f_{1+}$ | $\mathcal{O}^f_{2-}$ |
| $(c,e,f):143$ | $R_T^{z'x}$ | $R_T^{x'x}$ | ${}^sR_{LT'}^{00}$ | ${}^cR_{LT}^{0y}$ | ${}^cR_{LT'}^{0x}$ | ${}^cR_{LT'}^{0z}$ |
| | $\mathcal{O}^c_{1-}$ | $\mathcal{O}^c_{2-}$ | $\mathcal{O}^e_{1+}$ | $\mathcal{O}^e_{2-}$ | $\mathcal{O}^f_{1-}$ | $\mathcal{O}^f_{2+}$ |
| $(c,e,f):144$ | $R_T^{z'x}$ | $R_T^{x'x}$ | ${}^sR_{LT'}^{00}$ | ${}^cR_{LT}^{0y}$ | ${}^cR_{LT'}^{0x}$ | ${}^sR_{LT}^{0x}$ |
| | $\mathcal{O}^c_{1-}$ | $\mathcal{O}^c_{2-}$ | $\mathcal{O}^e_{1+}$ | $\mathcal{O}^e_{2-}$ | $\mathcal{O}^f_{1-}$ | $\mathcal{O}^f_{2-}$ |
| $(c,e,f):145$ | $R_T^{z'x}$ | $R_T^{x'x}$ | ${}^sR_{LT'}^{0y}$ | ${}^cR_{LT}^{00}$ | ${}^sR_{LT}^{0z}$ | ${}^cR_{LT'}^{0x}$ |
| | $\mathcal{O}^c_{1-}$ | $\mathcal{O}^c_{2-}$ | $\mathcal{O}^e_{1-}$ | $\mathcal{O}^e_{2+}$ | $\mathcal{O}^f_{1+}$ | $\mathcal{O}^f_{1-}$ |
| $(c,e,f):146$ | $R_T^{z'x}$ | $R_T^{x'x}$ | ${}^sR_{LT'}^{0y}$ | ${}^cR_{LT}^{00}$ | ${}^cR_{LT'}^{0z}$ | ${}^sR_{LT}^{0x}$ |
| | $\mathcal{O}^c_{1-}$ | $\mathcal{O}^c_{2-}$ | $\mathcal{O}^e_{1-}$ | $\mathcal{O}^e_{2+}$ | $\mathcal{O}^f_{2+}$ | $\mathcal{O}^f_{2-}$ |
| $(c,e,f):147$ | $R_T^{z'x}$ | $R_T^{x'x}$ | ${}^sR_{LT'}^{0y}$ | ${}^cR_{LT}^{00}$ | ${}^sR_{LT}^{0z}$ | ${}^cR_{LT'}^{0z}$ |
| | $\mathcal{O}^c_{1-}$ | $\mathcal{O}^c_{2-}$ | $\mathcal{O}^e_{1-}$ | $\mathcal{O}^e_{2+}$ | $\mathcal{O}^f_{1+}$ | $\mathcal{O}^f_{2+}$ |
| $(c,e,f):148$ | $R_T^{z'x}$ | $R_T^{x'x}$ | ${}^sR_{LT'}^{0y}$ | ${}^cR_{LT}^{00}$ | ${}^sR_{LT}^{0z}$ | ${}^sR_{LT}^{0x}$ |
| | $\mathcal{O}^c_{1-}$ | $\mathcal{O}^c_{2-}$ | $\mathcal{O}^e_{1-}$ | $\mathcal{O}^e_{2+}$ | $\mathcal{O}^f_{1+}$ | $\mathcal{O}^f_{2-}$ |
| $(c,e,f):149$ | $R_T^{z'x}$ | $R_T^{x'x}$ | ${}^sR_{LT'}^{0y}$ | ${}^cR_{LT}^{00}$ | ${}^cR_{LT'}^{0x}$ | ${}^cR_{LT'}^{0z}$ |
| | $\mathcal{O}^c_{1-}$ | $\mathcal{O}^c_{2-}$ | $\mathcal{O}^e_{1-}$ | $\mathcal{O}^e_{2+}$ | $\mathcal{O}^f_{1-}$ | $\mathcal{O}^f_{2+}$ |
| $(c,e,f):150$ | $R_T^{z'x}$ | $R_T^{x'x}$ | ${}^sR_{LT'}^{0y}$ | ${}^cR_{LT}^{00}$ | ${}^cR_{LT'}^{0x}$ | ${}^sR_{LT}^{0x}$ |
| | $\mathcal{O}^c_{1-}$ | $\mathcal{O}^c_{2-}$ | $\mathcal{O}^e_{1-}$ | $\mathcal{O}^e_{2+}$ | $\mathcal{O}^f_{1-}$ | $\mathcal{O}^f_{2-}$ |
| $(c,e,f):151$ | $R_T^{z'x}$ | $R_T^{x'x}$ | ${}^sR_{LT'}^{0y}$ | ${}^cR_{LT}^{0y}$ | ${}^sR_{LT}^{0z}$ | ${}^sR_{LT}^{0x}$ |
| | $\mathcal{O}^c_{1-}$ | $\mathcal{O}^c_{2-}$ | $\mathcal{O}^e_{1-}$ | $\mathcal{O}^e_{2-}$ | $\mathcal{O}^f_{1+}$ | $\mathcal{O}^f_{2-}$ |
| $(c,e,f):152$ | $R_T^{z'x}$ | $R_T^{x'x}$ | ${}^sR_{LT'}^{0y}$ | ${}^cR_{LT}^{0y}$ | ${}^cR_{LT'}^{0x}$ | ${}^cR_{LT'}^{0z}$ |
| | $\mathcal{O}^c_{1-}$ | $\mathcal{O}^c_{2-}$ | $\mathcal{O}^e_{1-}$ | $\mathcal{O}^e_{2-}$ | $\mathcal{O}^f_{1-}$ | $\mathcal{O}^f_{2+}$ |

TABLE IX: All the fully complete sets determined from the combination of shape-classes $(c, e, g)$ (i.e. graph-topology 'VI') in the case of pseudoscalar meson electroproduction are listed here. The observables are written in the systematic symbolic notation $\mathcal{O}^{n}_{\nu\pm}$ by Nakayama [1], as well as in the more commonly used notation in terms of 'response-functions' $R^{\beta\alpha}_{i}$ (cf. references [4, 5]). The given sets of 6 observables have to be combined with the 6 'diagonal' observables $\left\{ R^{00}_{T}, {}^{c}R^{00}_{TT}, R^{0y}_{T}, R^{y'0}_{T}, R^{00}_{L}, R^{0y}_{L} \right\}$ in order to form a complete set of minimal length $2N = 12$. All of these sets have been verified to be complete using Mathematica [3].

| Set-Nr. | Observables | | | | | |
|---|---|---|---|---|---|---|
| $(c, e, g) : 1$ | $R^{x'z}_{T}$ | $R^{z'x}_{T}$ | ${}^{s}R^{00}_{LT'}$ | ${}^{s}R^{0y}_{LT'}$ | ${}^{s}R^{z'0}_{LT}$ | ${}^{s}R^{x'0}_{LT}$ |
| | $\mathcal{O}^{c}_{1+}$ | $\mathcal{O}^{c}_{1-}$ | $\mathcal{O}^{e}_{1+}$ | $\mathcal{O}^{e}_{1-}$ | $\mathcal{O}^{g}_{1+}$ | $\mathcal{O}^{g}_{2-}$ |
| $(c, e, g) : 2$ | $R^{x'z}_{T}$ | $R^{z'x}_{T}$ | ${}^{s}R^{00}_{LT'}$ | ${}^{s}R^{0y}_{LT'}$ | ${}^{c}R^{x'0}_{LT'}$ | ${}^{c}R^{z'0}_{LT'}$ |
| | $\mathcal{O}^{c}_{1+}$ | $\mathcal{O}^{c}_{1-}$ | $\mathcal{O}^{e}_{1+}$ | $\mathcal{O}^{e}_{1-}$ | $\mathcal{O}^{g}_{1-}$ | $\mathcal{O}^{g}_{2+}$ |
| $(c, e, g) : 3$ | $R^{x'z}_{T}$ | $R^{z'x}_{T}$ | ${}^{c}R^{00}_{LT}$ | ${}^{c}R^{0y}_{LT}$ | ${}^{s}R^{z'0}_{LT}$ | ${}^{s}R^{x'0}_{LT}$ |
| | $\mathcal{O}^{c}_{1+}$ | $\mathcal{O}^{c}_{1-}$ | $\mathcal{O}^{e}_{2+}$ | $\mathcal{O}^{e}_{2-}$ | $\mathcal{O}^{g}_{1+}$ | $\mathcal{O}^{g}_{2-}$ |
| $(c, e, g) : 4$ | $R^{x'z}_{T}$ | $R^{z'x}_{T}$ | ${}^{c}R^{00}_{LT}$ | ${}^{c}R^{0y}_{LT}$ | ${}^{c}R^{x'0}_{LT'}$ | ${}^{c}R^{z'0}_{LT'}$ |
| | $\mathcal{O}^{c}_{1+}$ | $\mathcal{O}^{c}_{1-}$ | $\mathcal{O}^{e}_{2+}$ | $\mathcal{O}^{e}_{2-}$ | $\mathcal{O}^{g}_{1-}$ | $\mathcal{O}^{g}_{2+}$ |
| $(c, e, g) : 5$ | $R^{x'z}_{T}$ | $R^{z'x}_{T}$ | ${}^{s}R^{00}_{LT'}$ | ${}^{c}R^{00}_{LT}$ | ${}^{s}R^{z'0}_{LT}$ | ${}^{s}R^{x'0}_{LT}$ |
| | $\mathcal{O}^{c}_{1+}$ | $\mathcal{O}^{c}_{1-}$ | $\mathcal{O}^{e}_{1+}$ | $\mathcal{O}^{e}_{2+}$ | $\mathcal{O}^{g}_{1+}$ | $\mathcal{O}^{g}_{2-}$ |
| $(c, e, g) : 6$ | $R^{x'z}_{T}$ | $R^{z'x}_{T}$ | ${}^{s}R^{00}_{LT'}$ | ${}^{c}R^{00}_{LT}$ | ${}^{c}R^{x'0}_{LT'}$ | ${}^{c}R^{z'0}_{LT'}$ |
| | $\mathcal{O}^{c}_{1+}$ | $\mathcal{O}^{c}_{1-}$ | $\mathcal{O}^{e}_{1+}$ | $\mathcal{O}^{e}_{2+}$ | $\mathcal{O}^{g}_{1-}$ | $\mathcal{O}^{g}_{2+}$ |
| $(c, e, g) : 7$ | $R^{x'z}_{T}$ | $R^{z'x}_{T}$ | ${}^{s}R^{00}_{LT'}$ | ${}^{c}R^{0y}_{LT}$ | ${}^{s}R^{z'0}_{LT}$ | ${}^{c}R^{x'0}_{LT'}$ |
| | $\mathcal{O}^{c}_{1+}$ | $\mathcal{O}^{c}_{1-}$ | $\mathcal{O}^{e}_{1+}$ | $\mathcal{O}^{e}_{2-}$ | $\mathcal{O}^{g}_{1+}$ | $\mathcal{O}^{g}_{1-}$ |
| $(c, e, g) : 8$ | $R^{x'z}_{T}$ | $R^{z'x}_{T}$ | ${}^{s}R^{00}_{LT'}$ | ${}^{c}R^{0y}_{LT}$ | ${}^{c}R^{z'0}_{LT'}$ | ${}^{s}R^{x'0}_{LT}$ |
| | $\mathcal{O}^{c}_{1+}$ | $\mathcal{O}^{c}_{1-}$ | $\mathcal{O}^{e}_{1+}$ | $\mathcal{O}^{e}_{2-}$ | $\mathcal{O}^{g}_{2+}$ | $\mathcal{O}^{g}_{2-}$ |
| $(c, e, g) : 9$ | $R^{x'z}_{T}$ | $R^{z'x}_{T}$ | ${}^{s}R^{00}_{LT'}$ | ${}^{c}R^{0y}_{LT}$ | ${}^{s}R^{z'0}_{LT}$ | ${}^{c}R^{z'0}_{LT'}$ |
| | $\mathcal{O}^{c}_{1+}$ | $\mathcal{O}^{c}_{1-}$ | $\mathcal{O}^{e}_{1+}$ | $\mathcal{O}^{e}_{2-}$ | $\mathcal{O}^{g}_{1+}$ | $\mathcal{O}^{g}_{2+}$ |
| $(c, e, g) : 10$ | $R^{x'z}_{T}$ | $R^{z'x}_{T}$ | ${}^{s}R^{00}_{LT'}$ | ${}^{c}R^{0y}_{LT}$ | ${}^{s}R^{z'0}_{LT}$ | ${}^{s}R^{x'0}_{LT}$ |
| | $\mathcal{O}^{c}_{1+}$ | $\mathcal{O}^{c}_{1-}$ | $\mathcal{O}^{e}_{1+}$ | $\mathcal{O}^{e}_{2-}$ | $\mathcal{O}^{g}_{1+}$ | $\mathcal{O}^{g}_{2-}$ |
| $(c, e, g) : 11$ | $R^{x'z}_{T}$ | $R^{z'x}_{T}$ | ${}^{s}R^{00}_{LT'}$ | ${}^{c}R^{0y}_{LT}$ | ${}^{c}R^{x'0}_{LT'}$ | ${}^{c}R^{z'0}_{LT'}$ |
| | $\mathcal{O}^{c}_{1+}$ | $\mathcal{O}^{c}_{1-}$ | $\mathcal{O}^{e}_{1+}$ | $\mathcal{O}^{e}_{2-}$ | $\mathcal{O}^{g}_{1-}$ | $\mathcal{O}^{g}_{2+}$ |
| $(c, e, g) : 12$ | $R^{x'z}_{T}$ | $R^{z'x}_{T}$ | ${}^{s}R^{00}_{LT'}$ | ${}^{c}R^{0y}_{LT}$ | ${}^{c}R^{x'0}_{LT'}$ | ${}^{s}R^{x'0}_{LT}$ |
| | $\mathcal{O}^{c}_{1+}$ | $\mathcal{O}^{c}_{1-}$ | $\mathcal{O}^{e}_{1+}$ | $\mathcal{O}^{e}_{2-}$ | $\mathcal{O}^{g}_{1-}$ | $\mathcal{O}^{g}_{2-}$ |
| $(c, e, g) : 13$ | $R^{x'z}_{T}$ | $R^{z'x}_{T}$ | ${}^{s}R^{0y}_{LT'}$ | ${}^{c}R^{00}_{LT}$ | ${}^{s}R^{z'0}_{LT}$ | ${}^{c}R^{x'0}_{LT'}$ |
| | $\mathcal{O}^{c}_{1+}$ | $\mathcal{O}^{c}_{1-}$ | $\mathcal{O}^{e}_{1-}$ | $\mathcal{O}^{e}_{2+}$ | $\mathcal{O}^{g}_{1+}$ | $\mathcal{O}^{g}_{1-}$ |
| $(c, e, g) : 14$ | $R^{x'z}_{T}$ | $R^{z'x}_{T}$ | ${}^{s}R^{0y}_{LT'}$ | ${}^{c}R^{00}_{LT}$ | ${}^{c}R^{z'0}_{LT'}$ | ${}^{s}R^{x'0}_{LT}$ |
| | $\mathcal{O}^{c}_{1+}$ | $\mathcal{O}^{c}_{1-}$ | $\mathcal{O}^{e}_{1-}$ | $\mathcal{O}^{e}_{2+}$ | $\mathcal{O}^{g}_{2+}$ | $\mathcal{O}^{g}_{2-}$ |
| $(c, e, g) : 15$ | $R^{x'z}_{T}$ | $R^{z'x}_{T}$ | ${}^{s}R^{0y}_{LT'}$ | ${}^{c}R^{00}_{LT}$ | ${}^{s}R^{z'0}_{LT}$ | ${}^{c}R^{z'0}_{LT'}$ |
| | $\mathcal{O}^{c}_{1+}$ | $\mathcal{O}^{c}_{1-}$ | $\mathcal{O}^{e}_{1-}$ | $\mathcal{O}^{e}_{2+}$ | $\mathcal{O}^{g}_{1+}$ | $\mathcal{O}^{g}_{2+}$ |
| $(c, e, g) : 16$ | $R^{x'z}_{T}$ | $R^{z'x}_{T}$ | ${}^{s}R^{0y}_{LT'}$ | ${}^{c}R^{00}_{LT}$ | ${}^{s}R^{z'0}_{LT}$ | ${}^{s}R^{x'0}_{LT}$ |
| | $\mathcal{O}^{c}_{1+}$ | $\mathcal{O}^{c}_{1-}$ | $\mathcal{O}^{e}_{1-}$ | $\mathcal{O}^{e}_{2+}$ | $\mathcal{O}^{g}_{1+}$ | $\mathcal{O}^{g}_{2-}$ |
| $(c, e, g) : 17$ | $R^{x'z}_{T}$ | $R^{z'x}_{T}$ | ${}^{s}R^{0y}_{LT'}$ | ${}^{c}R^{00}_{LT}$ | ${}^{c}R^{x'0}_{LT'}$ | ${}^{c}R^{z'0}_{LT'}$ |
| | $\mathcal{O}^{c}_{1+}$ | $\mathcal{O}^{c}_{1-}$ | $\mathcal{O}^{e}_{1-}$ | $\mathcal{O}^{e}_{2+}$ | $\mathcal{O}^{g}_{1-}$ | $\mathcal{O}^{g}_{2+}$ |
| $(c, e, g) : 18$ | $R^{x'z}_{T}$ | $R^{z'x}_{T}$ | ${}^{s}R^{0y}_{LT'}$ | ${}^{c}R^{00}_{LT}$ | ${}^{c}R^{x'0}_{LT'}$ | ${}^{s}R^{x'0}_{LT}$ |
| | $\mathcal{O}^{c}_{1+}$ | $\mathcal{O}^{c}_{1-}$ | $\mathcal{O}^{e}_{1-}$ | $\mathcal{O}^{e}_{2+}$ | $\mathcal{O}^{g}_{1-}$ | $\mathcal{O}^{g}_{2-}$ |
| $(c, e, g) : 19$ | $R^{x'z}_{T}$ | $R^{z'x}_{T}$ | ${}^{s}R^{0y}_{LT'}$ | ${}^{c}R^{0y}_{LT}$ | ${}^{s}R^{z'0}_{LT}$ | ${}^{s}R^{x'0}_{LT}$ |
| | $\mathcal{O}^{c}_{1+}$ | $\mathcal{O}^{c}_{1-}$ | $\mathcal{O}^{e}_{1-}$ | $\mathcal{O}^{e}_{2-}$ | $\mathcal{O}^{g}_{1+}$ | $\mathcal{O}^{g}_{2-}$ |
| $(c, e, g) : 20$ | $R^{x'z}_{T}$ | $R^{z'x}_{T}$ | ${}^{s}R^{0y}_{LT'}$ | ${}^{c}R^{0y}_{LT}$ | ${}^{c}R^{x'0}_{LT'}$ | ${}^{c}R^{z'0}_{LT'}$ |
| | $\mathcal{O}^{c}_{1+}$ | $\mathcal{O}^{c}_{1-}$ | $\mathcal{O}^{e}_{1-}$ | $\mathcal{O}^{e}_{2-}$ | $\mathcal{O}^{g}_{1-}$ | $\mathcal{O}^{g}_{2+}$ |
| $(c, e, g) : 21$ | $R^{z'z}_{T}$ | $R^{x'x}_{T}$ | ${}^{s}R^{00}_{LT'}$ | ${}^{s}R^{0y}_{LT'}$ | ${}^{s}R^{z'0}_{LT}$ | ${}^{s}R^{x'0}_{LT}$ |
| | $\mathcal{O}^{c}_{2+}$ | $\mathcal{O}^{c}_{2-}$ | $\mathcal{O}^{e}_{1+}$ | $\mathcal{O}^{e}_{1-}$ | $\mathcal{O}^{g}_{1+}$ | $\mathcal{O}^{g}_{2-}$ |
| $(c, e, g) : 22$ | $R^{z'z}_{T}$ | $R^{x'x}_{T}$ | ${}^{s}R^{00}_{LT'}$ | ${}^{s}R^{0y}_{LT'}$ | ${}^{c}R^{x'0}_{LT'}$ | ${}^{c}R^{z'0}_{LT'}$ |
| | $\mathcal{O}^{c}_{2+}$ | $\mathcal{O}^{c}_{2-}$ | $\mathcal{O}^{e}_{1+}$ | $\mathcal{O}^{e}_{1-}$ | $\mathcal{O}^{g}_{1-}$ | $\mathcal{O}^{g}_{2+}$ |
| $(c, e, g) : 23$ | $R^{z'z}_{T}$ | $R^{x'x}_{T}$ | ${}^{c}R^{00}_{LT}$ | ${}^{c}R^{0y}_{LT}$ | ${}^{s}R^{z'0}_{LT}$ | ${}^{s}R^{x'0}_{LT}$ |
| | $\mathcal{O}^{c}_{2+}$ | $\mathcal{O}^{c}_{2-}$ | $\mathcal{O}^{e}_{2+}$ | $\mathcal{O}^{e}_{2-}$ | $\mathcal{O}^{g}_{1+}$ | $\mathcal{O}^{g}_{2-}$ |
| $(c, e, g) : 24$ | $R^{z'z}_{T}$ | $R^{x'x}_{T}$ | ${}^{c}R^{00}_{LT}$ | ${}^{c}R^{0y}_{LT}$ | ${}^{c}R^{x'0}_{LT'}$ | ${}^{c}R^{z'0}_{LT'}$ |

| | | | | | | |
|---|---|---|---|---|---|---|
| | $\mathcal{O}^c_{2+}$ | $\mathcal{O}^c_{2-}$ | $\mathcal{O}^e_{2+}$ | $\mathcal{O}^e_{2-}$ | $\mathcal{O}^g_{1-}$ | $\mathcal{O}^g_{2+}$ |
| $(c,e,g):25$ | $R_T^{z'z}$ | $R_T^{x'x}$ | ${}^sR_{LT'}^{00}$ | ${}^cR_{LT}^{00}$ | ${}^sR_{LT}^{z'0}$ | ${}^sR_{LT}^{x'0}$ |
| | $\mathcal{O}^c_{2+}$ | $\mathcal{O}^c_{2-}$ | $\mathcal{O}^e_{1+}$ | $\mathcal{O}^e_{2+}$ | $\mathcal{O}^g_{1+}$ | $\mathcal{O}^g_{2-}$ |
| $(c,e,g):26$ | $R_T^{z'z}$ | $R_T^{x'x}$ | ${}^sR_{LT'}^{00}$ | ${}^cR_{LT}^{00}$ | ${}^cR_{LT'}^{x'0}$ | ${}^cR_{LT'}^{z'0}$ |
| | $\mathcal{O}^c_{2+}$ | $\mathcal{O}^c_{2-}$ | $\mathcal{O}^e_{1+}$ | $\mathcal{O}^e_{2+}$ | $\mathcal{O}^g_{1-}$ | $\mathcal{O}^g_{2+}$ |
| $(c,e,g):27$ | $R_T^{z'z}$ | $R_T^{x'x}$ | ${}^sR_{LT'}^{00}$ | ${}^cR_{LT}^{0y}$ | ${}^sR_{LT}^{z'0}$ | ${}^cR_{LT'}^{x'0}$ |
| | $\mathcal{O}^c_{2+}$ | $\mathcal{O}^c_{2-}$ | $\mathcal{O}^e_{1+}$ | $\mathcal{O}^e_{2-}$ | $\mathcal{O}^g_{1+}$ | $\mathcal{O}^g_{1-}$ |
| $(c,e,g):28$ | $R_T^{z'z}$ | $R_T^{x'x}$ | ${}^sR_{LT'}^{00}$ | ${}^cR_{LT}^{0y}$ | ${}^cR_{LT'}^{z'0}$ | ${}^sR_{LT}^{x'0}$ |
| | $\mathcal{O}^c_{2+}$ | $\mathcal{O}^c_{2-}$ | $\mathcal{O}^e_{1+}$ | $\mathcal{O}^e_{2-}$ | $\mathcal{O}^g_{2+}$ | $\mathcal{O}^g_{2-}$ |
| $(c,e,g):29$ | $R_T^{z'z}$ | $R_T^{x'x}$ | ${}^sR_{LT'}^{00}$ | ${}^cR_{LT}^{0y}$ | ${}^sR_{LT}^{z'0}$ | ${}^cR_{LT'}^{z'0}$ |
| | $\mathcal{O}^c_{2+}$ | $\mathcal{O}^c_{2-}$ | $\mathcal{O}^e_{1+}$ | $\mathcal{O}^e_{2-}$ | $\mathcal{O}^g_{1+}$ | $\mathcal{O}^g_{2+}$ |
| $(c,e,g):30$ | $R_T^{z'z}$ | $R_T^{x'x}$ | ${}^sR_{LT'}^{00}$ | ${}^cR_{LT}^{0y}$ | ${}^sR_{LT}^{z'0}$ | ${}^sR_{LT}^{x'0}$ |
| | $\mathcal{O}^c_{2+}$ | $\mathcal{O}^c_{2-}$ | $\mathcal{O}^e_{1+}$ | $\mathcal{O}^e_{2-}$ | $\mathcal{O}^g_{1+}$ | $\mathcal{O}^g_{2-}$ |
| $(c,e,g):31$ | $R_T^{z'z}$ | $R_T^{x'x}$ | ${}^sR_{LT'}^{00}$ | ${}^cR_{LT}^{0y}$ | ${}^cR_{LT'}^{x'0}$ | ${}^cR_{LT'}^{z'0}$ |
| | $\mathcal{O}^c_{2+}$ | $\mathcal{O}^c_{2-}$ | $\mathcal{O}^e_{1+}$ | $\mathcal{O}^e_{2-}$ | $\mathcal{O}^g_{1-}$ | $\mathcal{O}^g_{2+}$ |
| $(c,e,g):32$ | $R_T^{z'z}$ | $R_T^{x'x}$ | ${}^sR_{LT'}^{00}$ | ${}^cR_{LT}^{0y}$ | ${}^cR_{LT'}^{x'0}$ | ${}^sR_{LT}^{x'0}$ |
| | $\mathcal{O}^c_{2+}$ | $\mathcal{O}^c_{2-}$ | $\mathcal{O}^e_{1+}$ | $\mathcal{O}^e_{2-}$ | $\mathcal{O}^g_{1-}$ | $\mathcal{O}^g_{2-}$ |
| $(c,e,g):33$ | $R_T^{z'z}$ | $R_T^{x'x}$ | ${}^sR_{LT'}^{0y}$ | ${}^cR_{LT}^{00}$ | ${}^sR_{LT}^{z'0}$ | ${}^cR_{LT'}^{x'0}$ |
| | $\mathcal{O}^c_{2+}$ | $\mathcal{O}^c_{2-}$ | $\mathcal{O}^e_{1-}$ | $\mathcal{O}^e_{2+}$ | $\mathcal{O}^g_{1+}$ | $\mathcal{O}^g_{1-}$ |
| $(c,e,g):34$ | $R_T^{z'z}$ | $R_T^{x'x}$ | ${}^sR_{LT'}^{0y}$ | ${}^cR_{LT}^{00}$ | ${}^cR_{LT'}^{z'0}$ | ${}^sR_{LT}^{x'0}$ |
| | $\mathcal{O}^c_{2+}$ | $\mathcal{O}^c_{2-}$ | $\mathcal{O}^e_{1-}$ | $\mathcal{O}^e_{2+}$ | $\mathcal{O}^g_{2+}$ | $\mathcal{O}^g_{2-}$ |
| $(c,e,g):35$ | $R_T^{z'z}$ | $R_T^{x'x}$ | ${}^sR_{LT'}^{0y}$ | ${}^cR_{LT}^{00}$ | ${}^sR_{LT}^{z'0}$ | ${}^cR_{LT'}^{z'0}$ |
| | $\mathcal{O}^c_{2+}$ | $\mathcal{O}^c_{2-}$ | $\mathcal{O}^e_{1-}$ | $\mathcal{O}^e_{2+}$ | $\mathcal{O}^g_{1+}$ | $\mathcal{O}^g_{2+}$ |
| $(c,e,g):36$ | $R_T^{z'z}$ | $R_T^{x'x}$ | ${}^sR_{LT'}^{0y}$ | ${}^cR_{LT}^{00}$ | ${}^sR_{LT}^{z'0}$ | ${}^sR_{LT}^{x'0}$ |
| | $\mathcal{O}^c_{2+}$ | $\mathcal{O}^c_{2-}$ | $\mathcal{O}^e_{1-}$ | $\mathcal{O}^e_{2+}$ | $\mathcal{O}^g_{1+}$ | $\mathcal{O}^g_{2-}$ |
| $(c,e,g):37$ | $R_T^{z'z}$ | $R_T^{x'x}$ | ${}^sR_{LT'}^{0y}$ | ${}^cR_{LT}^{00}$ | ${}^cR_{LT'}^{x'0}$ | ${}^cR_{LT'}^{z'0}$ |
| | $\mathcal{O}^c_{2+}$ | $\mathcal{O}^c_{2-}$ | $\mathcal{O}^e_{1-}$ | $\mathcal{O}^e_{2+}$ | $\mathcal{O}^g_{1-}$ | $\mathcal{O}^g_{2+}$ |
| $(c,e,g):38$ | $R_T^{z'z}$ | $R_T^{x'x}$ | ${}^sR_{LT'}^{0y}$ | ${}^cR_{LT}^{00}$ | ${}^cR_{LT'}^{x'0}$ | ${}^sR_{LT}^{x'0}$ |
| | $\mathcal{O}^c_{2+}$ | $\mathcal{O}^c_{2-}$ | $\mathcal{O}^e_{1-}$ | $\mathcal{O}^e_{2+}$ | $\mathcal{O}^g_{1-}$ | $\mathcal{O}^g_{2-}$ |
| $(c,e,g):39$ | $R_T^{z'z}$ | $R_T^{x'x}$ | ${}^sR_{LT'}^{0y}$ | ${}^cR_{LT}^{0y}$ | ${}^sR_{LT}^{z'0}$ | ${}^sR_{LT}^{x'0}$ |
| | $\mathcal{O}^c_{2+}$ | $\mathcal{O}^c_{2-}$ | $\mathcal{O}^e_{1-}$ | $\mathcal{O}^e_{2-}$ | $\mathcal{O}^g_{1+}$ | $\mathcal{O}^g_{2-}$ |
| $(c,e,g):40$ | $R_T^{z'z}$ | $R_T^{x'x}$ | ${}^sR_{LT'}^{0y}$ | ${}^cR_{LT}^{0y}$ | ${}^cR_{LT'}^{x'0}$ | ${}^cR_{LT'}^{z'0}$ |
| | $\mathcal{O}^c_{2+}$ | $\mathcal{O}^c_{2-}$ | $\mathcal{O}^e_{1-}$ | $\mathcal{O}^e_{2-}$ | $\mathcal{O}^g_{1-}$ | $\mathcal{O}^g_{2+}$ |
| $(c,e,g):41$ | $R_T^{x'z}$ | $R_T^{z'z}$ | ${}^sR_{LT'}^{00}$ | ${}^sR_{LT'}^{0y}$ | ${}^sR_{LT}^{z'0}$ | ${}^cR_{LT'}^{x'0}$ |
| | $\mathcal{O}^c_{1+}$ | $\mathcal{O}^c_{2+}$ | $\mathcal{O}^e_{1+}$ | $\mathcal{O}^e_{1-}$ | $\mathcal{O}^g_{1+}$ | $\mathcal{O}^g_{1-}$ |
| $(c,e,g):42$ | $R_T^{x'z}$ | $R_T^{z'z}$ | ${}^sR_{LT'}^{00}$ | ${}^sR_{LT'}^{0y}$ | ${}^cR_{LT'}^{z'0}$ | ${}^sR_{LT}^{x'0}$ |
| | $\mathcal{O}^c_{1+}$ | $\mathcal{O}^c_{2+}$ | $\mathcal{O}^e_{1+}$ | $\mathcal{O}^e_{1-}$ | $\mathcal{O}^g_{2+}$ | $\mathcal{O}^g_{2-}$ |
| $(c,e,g):43$ | $R_T^{x'z}$ | $R_T^{z'z}$ | ${}^sR_{LT'}^{00}$ | ${}^sR_{LT'}^{0y}$ | ${}^sR_{LT}^{z'0}$ | ${}^cR_{LT'}^{z'0}$ |
| | $\mathcal{O}^c_{1+}$ | $\mathcal{O}^c_{2+}$ | $\mathcal{O}^e_{1+}$ | $\mathcal{O}^e_{1-}$ | $\mathcal{O}^g_{1+}$ | $\mathcal{O}^g_{2+}$ |
| $(c,e,g):44$ | $R_T^{x'z}$ | $R_T^{z'z}$ | ${}^sR_{LT'}^{00}$ | ${}^sR_{LT'}^{0y}$ | ${}^sR_{LT}^{z'0}$ | ${}^sR_{LT}^{x'0}$ |
| | $\mathcal{O}^c_{1+}$ | $\mathcal{O}^c_{2+}$ | $\mathcal{O}^e_{1+}$ | $\mathcal{O}^e_{1-}$ | $\mathcal{O}^g_{1+}$ | $\mathcal{O}^g_{2-}$ |
| $(c,e,g):45$ | $R_T^{x'z}$ | $R_T^{z'z}$ | ${}^sR_{LT'}^{00}$ | ${}^sR_{LT'}^{0y}$ | ${}^cR_{LT'}^{x'0}$ | ${}^cR_{LT'}^{z'0}$ |
| | $\mathcal{O}^c_{1+}$ | $\mathcal{O}^c_{2+}$ | $\mathcal{O}^e_{1+}$ | $\mathcal{O}^e_{1-}$ | $\mathcal{O}^g_{1-}$ | $\mathcal{O}^g_{2+}$ |
| $(c,e,g):46$ | $R_T^{x'z}$ | $R_T^{z'z}$ | ${}^sR_{LT'}^{00}$ | ${}^sR_{LT'}^{0y}$ | ${}^cR_{LT'}^{x'0}$ | ${}^sR_{LT}^{x'0}$ |
| | $\mathcal{O}^c_{1+}$ | $\mathcal{O}^c_{2+}$ | $\mathcal{O}^e_{1+}$ | $\mathcal{O}^e_{1-}$ | $\mathcal{O}^g_{1-}$ | $\mathcal{O}^g_{2-}$ |
| $(c,e,g):47$ | $R_T^{x'z}$ | $R_T^{z'z}$ | ${}^cR_{LT}^{00}$ | ${}^cR_{LT}^{0y}$ | ${}^sR_{LT}^{z'0}$ | ${}^cR_{LT'}^{x'0}$ |
| | $\mathcal{O}^c_{1+}$ | $\mathcal{O}^c_{2+}$ | $\mathcal{O}^e_{2+}$ | $\mathcal{O}^e_{2-}$ | $\mathcal{O}^g_{1+}$ | $\mathcal{O}^g_{1-}$ |
| $(c,e,g):48$ | $R_T^{x'z}$ | $R_T^{z'z}$ | ${}^cR_{LT}^{00}$ | ${}^cR_{LT}^{0y}$ | ${}^cR_{LT'}^{z'0}$ | ${}^sR_{LT}^{x'0}$ |
| | $\mathcal{O}^c_{1+}$ | $\mathcal{O}^c_{2+}$ | $\mathcal{O}^e_{2+}$ | $\mathcal{O}^e_{2-}$ | $\mathcal{O}^g_{2+}$ | $\mathcal{O}^g_{2-}$ |
| $(c,e,g):49$ | $R_T^{x'z}$ | $R_T^{z'z}$ | ${}^cR_{LT}^{00}$ | ${}^cR_{LT}^{0y}$ | ${}^sR_{LT}^{z'0}$ | ${}^cR_{LT'}^{z'0}$ |
| | $\mathcal{O}^c_{1+}$ | $\mathcal{O}^c_{2+}$ | $\mathcal{O}^e_{2+}$ | $\mathcal{O}^e_{2-}$ | $\mathcal{O}^g_{1+}$ | $\mathcal{O}^g_{2+}$ |
| $(c,e,g):50$ | $R_T^{x'z}$ | $R_T^{z'z}$ | ${}^cR_{LT}^{00}$ | ${}^cR_{LT}^{0y}$ | ${}^sR_{LT}^{z'0}$ | ${}^sR_{LT}^{x'0}$ |
| | $\mathcal{O}^c_{1+}$ | $\mathcal{O}^c_{2+}$ | $\mathcal{O}^e_{2+}$ | $\mathcal{O}^e_{2-}$ | $\mathcal{O}^g_{1+}$ | $\mathcal{O}^g_{2-}$ |
| $(c,e,g):51$ | $R_T^{x'z}$ | $R_T^{z'z}$ | ${}^cR_{LT}^{00}$ | ${}^cR_{LT}^{0y}$ | ${}^cR_{LT'}^{x'0}$ | ${}^cR_{LT'}^{z'0}$ |
| | $\mathcal{O}^c_{1+}$ | $\mathcal{O}^c_{2+}$ | $\mathcal{O}^e_{2+}$ | $\mathcal{O}^e_{2-}$ | $\mathcal{O}^g_{1-}$ | $\mathcal{O}^g_{2+}$ |
| $(c,e,g):52$ | $R_T^{x'z}$ | $R_T^{z'z}$ | ${}^cR_{LT}^{00}$ | ${}^cR_{LT}^{0y}$ | ${}^cR_{LT'}^{x'0}$ | ${}^sR_{LT}^{x'0}$ |
| | $\mathcal{O}^c_{1+}$ | $\mathcal{O}^c_{2+}$ | $\mathcal{O}^e_{2+}$ | $\mathcal{O}^e_{2-}$ | $\mathcal{O}^g_{1-}$ | $\mathcal{O}^g_{2-}$ |
| $(c,e,g):53$ | $R_T^{x'z}$ | $R_T^{z'z}$ | ${}^sR_{LT'}^{00}$ | ${}^cR_{LT}^{00}$ | ${}^sR_{LT}^{z'0}$ | ${}^cR_{LT'}^{x'0}$ |

| | | | | | | |
|---|---|---|---|---|---|---|
| | $\mathcal{O}^c_{1+}$ | $\mathcal{O}^c_{2+}$ | $\mathcal{O}^e_{1+}$ | $\mathcal{O}^e_{2+}$ | $\mathcal{O}^g_{1+}$ | $\mathcal{O}^g_{1-}$ |
| $(c,e,g):54$ | $R^{x'z}_T$ | $R^{z'z}_T$ | ${}^sR^{00}_{LT'}$ | ${}^cR^{00}_{LT}$ | ${}^cR^{z'0}_{LT'}$ | ${}^sR^{x'0}_{LT}$ |
| | $\mathcal{O}^c_{1+}$ | $\mathcal{O}^c_{2+}$ | $\mathcal{O}^e_{1+}$ | $\mathcal{O}^e_{2+}$ | $\mathcal{O}^g_{2+}$ | $\mathcal{O}^g_{2-}$ |
| $(c,e,g):55$ | $R^{x'z}_T$ | $R^{z'z}_T$ | ${}^sR^{00}_{LT'}$ | ${}^cR^{00}_{LT}$ | ${}^sR^{z'0}_{LT}$ | ${}^cR^{z'0}_{LT'}$ |
| | $\mathcal{O}^c_{1+}$ | $\mathcal{O}^c_{2+}$ | $\mathcal{O}^e_{1+}$ | $\mathcal{O}^e_{2+}$ | $\mathcal{O}^g_{1+}$ | $\mathcal{O}^g_{2+}$ |
| $(c,e,g):56$ | $R^{x'z}_T$ | $R^{z'z}_T$ | ${}^sR^{00}_{LT'}$ | ${}^cR^{00}_{LT}$ | ${}^sR^{z'0}_{LT}$ | ${}^sR^{x'0}_{LT}$ |
| | $\mathcal{O}^c_{1+}$ | $\mathcal{O}^c_{2+}$ | $\mathcal{O}^e_{1+}$ | $\mathcal{O}^e_{2+}$ | $\mathcal{O}^g_{1+}$ | $\mathcal{O}^g_{2-}$ |
| $(c,e,g):57$ | $R^{x'z}_T$ | $R^{z'z}_T$ | ${}^sR^{00}_{LT'}$ | ${}^cR^{00}_{LT}$ | ${}^cR^{x'0}_{LT'}$ | ${}^cR^{z'0}_{LT'}$ |
| | $\mathcal{O}^c_{1+}$ | $\mathcal{O}^c_{2+}$ | $\mathcal{O}^e_{1+}$ | $\mathcal{O}^e_{2+}$ | $\mathcal{O}^g_{1-}$ | $\mathcal{O}^g_{2+}$ |
| $(c,e,g):58$ | $R^{x'z}_T$ | $R^{z'z}_T$ | ${}^sR^{00}_{LT'}$ | ${}^cR^{00}_{LT}$ | ${}^cR^{x'0}_{LT'}$ | ${}^sR^{x'0}_{LT}$ |
| | $\mathcal{O}^c_{1+}$ | $\mathcal{O}^c_{2+}$ | $\mathcal{O}^e_{1+}$ | $\mathcal{O}^e_{2+}$ | $\mathcal{O}^g_{1-}$ | $\mathcal{O}^g_{2-}$ |
| $(c,e,g):59$ | $R^{x'z}_T$ | $R^{z'z}_T$ | ${}^sR^{00}_{LT'}$ | ${}^cR^{0y}_{LT}$ | ${}^sR^{z'0}_{LT}$ | ${}^cR^{x'0}_{LT'}$ |
| | $\mathcal{O}^c_{1+}$ | $\mathcal{O}^c_{2+}$ | $\mathcal{O}^e_{1+}$ | $\mathcal{O}^e_{2-}$ | $\mathcal{O}^g_{1+}$ | $\mathcal{O}^g_{1-}$ |
| $(c,e,g):60$ | $R^{x'z}_T$ | $R^{z'z}_T$ | ${}^sR^{00}_{LT'}$ | ${}^cR^{0y}_{LT}$ | ${}^cR^{z'0}_{LT'}$ | ${}^sR^{x'0}_{LT}$ |
| | $\mathcal{O}^c_{1+}$ | $\mathcal{O}^c_{2+}$ | $\mathcal{O}^e_{1+}$ | $\mathcal{O}^e_{2-}$ | $\mathcal{O}^g_{2+}$ | $\mathcal{O}^g_{2-}$ |
| $(c,e,g):61$ | $R^{x'z}_T$ | $R^{z'z}_T$ | ${}^sR^{00}_{LT'}$ | ${}^cR^{0y}_{LT}$ | ${}^sR^{z'0}_{LT}$ | ${}^cR^{z'0}_{LT'}$ |
| | $\mathcal{O}^c_{1+}$ | $\mathcal{O}^c_{2+}$ | $\mathcal{O}^e_{1+}$ | $\mathcal{O}^e_{2-}$ | $\mathcal{O}^g_{1+}$ | $\mathcal{O}^g_{2+}$ |
| $(c,e,g):62$ | $R^{x'z}_T$ | $R^{z'z}_T$ | ${}^sR^{00}_{LT'}$ | ${}^cR^{0y}_{LT}$ | ${}^sR^{z'0}_{LT}$ | ${}^sR^{x'0}_{LT}$ |
| | $\mathcal{O}^c_{1+}$ | $\mathcal{O}^c_{2+}$ | $\mathcal{O}^e_{1+}$ | $\mathcal{O}^e_{2-}$ | $\mathcal{O}^g_{1+}$ | $\mathcal{O}^g_{2-}$ |
| $(c,e,g):63$ | $R^{x'z}_T$ | $R^{z'z}_T$ | ${}^sR^{00}_{LT'}$ | ${}^cR^{0y}_{LT}$ | ${}^cR^{x'0}_{LT'}$ | ${}^cR^{z'0}_{LT'}$ |
| | $\mathcal{O}^c_{1+}$ | $\mathcal{O}^c_{2+}$ | $\mathcal{O}^e_{1+}$ | $\mathcal{O}^e_{2-}$ | $\mathcal{O}^g_{1-}$ | $\mathcal{O}^g_{2+}$ |
| $(c,e,g):64$ | $R^{x'z}_T$ | $R^{z'z}_T$ | ${}^sR^{00}_{LT'}$ | ${}^cR^{0y}_{LT}$ | ${}^cR^{x'0}_{LT'}$ | ${}^sR^{x'0}_{LT}$ |
| | $\mathcal{O}^c_{1+}$ | $\mathcal{O}^c_{2+}$ | $\mathcal{O}^e_{1+}$ | $\mathcal{O}^e_{2-}$ | $\mathcal{O}^g_{1-}$ | $\mathcal{O}^g_{2-}$ |
| $(c,e,g):65$ | $R^{x'z}_T$ | $R^{z'z}_T$ | ${}^sR^{0y}_{LT'}$ | ${}^cR^{00}_{LT}$ | ${}^sR^{z'0}_{LT}$ | ${}^cR^{x'0}_{LT'}$ |
| | $\mathcal{O}^c_{1+}$ | $\mathcal{O}^c_{2+}$ | $\mathcal{O}^e_{1-}$ | $\mathcal{O}^e_{2+}$ | $\mathcal{O}^g_{1+}$ | $\mathcal{O}^g_{1-}$ |
| $(c,e,g):66$ | $R^{x'z}_T$ | $R^{z'z}_T$ | ${}^sR^{0y}_{LT'}$ | ${}^cR^{00}_{LT}$ | ${}^cR^{z'0}_{LT'}$ | ${}^sR^{x'0}_{LT}$ |
| | $\mathcal{O}^c_{1+}$ | $\mathcal{O}^c_{2+}$ | $\mathcal{O}^e_{1-}$ | $\mathcal{O}^e_{2+}$ | $\mathcal{O}^g_{2+}$ | $\mathcal{O}^g_{2-}$ |
| $(c,e,g):67$ | $R^{x'z}_T$ | $R^{z'z}_T$ | ${}^sR^{0y}_{LT'}$ | ${}^cR^{00}_{LT}$ | ${}^sR^{z'0}_{LT}$ | ${}^cR^{z'0}_{LT'}$ |
| | $\mathcal{O}^c_{1+}$ | $\mathcal{O}^c_{2+}$ | $\mathcal{O}^e_{1-}$ | $\mathcal{O}^e_{2+}$ | $\mathcal{O}^g_{1+}$ | $\mathcal{O}^g_{2+}$ |
| $(c,e,g):68$ | $R^{x'z}_T$ | $R^{z'z}_T$ | ${}^sR^{0y}_{LT'}$ | ${}^cR^{00}_{LT}$ | ${}^sR^{z'0}_{LT}$ | ${}^sR^{x'0}_{LT}$ |
| | $\mathcal{O}^c_{1+}$ | $\mathcal{O}^c_{2+}$ | $\mathcal{O}^e_{1-}$ | $\mathcal{O}^e_{2+}$ | $\mathcal{O}^g_{1+}$ | $\mathcal{O}^g_{2-}$ |
| $(c,e,g):69$ | $R^{x'z}_T$ | $R^{z'z}_T$ | ${}^sR^{0y}_{LT'}$ | ${}^cR^{00}_{LT}$ | ${}^cR^{x'0}_{LT'}$ | ${}^cR^{z'0}_{LT'}$ |
| | $\mathcal{O}^c_{1+}$ | $\mathcal{O}^c_{2+}$ | $\mathcal{O}^e_{1-}$ | $\mathcal{O}^e_{2+}$ | $\mathcal{O}^g_{1-}$ | $\mathcal{O}^g_{2+}$ |
| $(c,e,g):70$ | $R^{x'z}_T$ | $R^{z'z}_T$ | ${}^sR^{0y}_{LT'}$ | ${}^cR^{00}_{LT}$ | ${}^cR^{x'0}_{LT'}$ | ${}^sR^{x'0}_{LT}$ |
| | $\mathcal{O}^c_{1+}$ | $\mathcal{O}^c_{2+}$ | $\mathcal{O}^e_{1-}$ | $\mathcal{O}^e_{2+}$ | $\mathcal{O}^g_{1-}$ | $\mathcal{O}^g_{2-}$ |
| $(c,e,g):71$ | $R^{x'z}_T$ | $R^{z'z}_T$ | ${}^sR^{0y}_{LT'}$ | ${}^cR^{0y}_{LT}$ | ${}^sR^{z'0}_{LT}$ | ${}^cR^{x'0}_{LT'}$ |
| | $\mathcal{O}^c_{1+}$ | $\mathcal{O}^c_{2+}$ | $\mathcal{O}^e_{1-}$ | $\mathcal{O}^e_{2-}$ | $\mathcal{O}^g_{1+}$ | $\mathcal{O}^g_{1-}$ |
| $(c,e,g):72$ | $R^{x'z}_T$ | $R^{z'z}_T$ | ${}^sR^{0y}_{LT'}$ | ${}^cR^{0y}_{LT}$ | ${}^cR^{z'0}_{LT'}$ | ${}^sR^{x'0}_{LT}$ |
| | $\mathcal{O}^c_{1+}$ | $\mathcal{O}^c_{2+}$ | $\mathcal{O}^e_{1-}$ | $\mathcal{O}^e_{2-}$ | $\mathcal{O}^g_{2+}$ | $\mathcal{O}^g_{2-}$ |
| $(c,e,g):73$ | $R^{x'z}_T$ | $R^{z'z}_T$ | ${}^sR^{0y}_{LT'}$ | ${}^cR^{0y}_{LT}$ | ${}^sR^{z'0}_{LT}$ | ${}^cR^{z'0}_{LT'}$ |
| | $\mathcal{O}^c_{1+}$ | $\mathcal{O}^c_{2+}$ | $\mathcal{O}^e_{1-}$ | $\mathcal{O}^e_{2-}$ | $\mathcal{O}^g_{1+}$ | $\mathcal{O}^g_{2+}$ |
| $(c,e,g):74$ | $R^{x'z}_T$ | $R^{z'z}_T$ | ${}^sR^{0y}_{LT'}$ | ${}^cR^{0y}_{LT}$ | ${}^sR^{z'0}_{LT}$ | ${}^sR^{x'0}_{LT}$ |
| | $\mathcal{O}^c_{1+}$ | $\mathcal{O}^c_{2+}$ | $\mathcal{O}^e_{1-}$ | $\mathcal{O}^e_{2-}$ | $\mathcal{O}^g_{1+}$ | $\mathcal{O}^g_{2-}$ |
| $(c,e,g):75$ | $R^{x'z}_T$ | $R^{z'z}_T$ | ${}^sR^{0y}_{LT'}$ | ${}^cR^{0y}_{LT}$ | ${}^cR^{x'0}_{LT'}$ | ${}^cR^{z'0}_{LT'}$ |
| | $\mathcal{O}^c_{1+}$ | $\mathcal{O}^c_{2+}$ | $\mathcal{O}^e_{1-}$ | $\mathcal{O}^e_{2-}$ | $\mathcal{O}^g_{1-}$ | $\mathcal{O}^g_{2+}$ |
| $(c,e,g):76$ | $R^{x'z}_T$ | $R^{z'z}_T$ | ${}^sR^{0y}_{LT'}$ | ${}^cR^{0y}_{LT}$ | ${}^cR^{x'0}_{LT'}$ | ${}^sR^{x'0}_{LT}$ |
| | $\mathcal{O}^c_{1+}$ | $\mathcal{O}^c_{2+}$ | $\mathcal{O}^e_{1-}$ | $\mathcal{O}^e_{2-}$ | $\mathcal{O}^g_{1-}$ | $\mathcal{O}^g_{2-}$ |
| $(c,e,g):77$ | $R^{x'z}_T$ | $R^{x'x}_T$ | ${}^sR^{00}_{LT'}$ | ${}^sR^{0y}_{LT'}$ | ${}^sR^{z'0}_{LT}$ | ${}^sR^{x'0}_{LT}$ |
| | $\mathcal{O}^c_{1+}$ | $\mathcal{O}^c_{2-}$ | $\mathcal{O}^e_{1+}$ | $\mathcal{O}^e_{1-}$ | $\mathcal{O}^g_{1+}$ | $\mathcal{O}^g_{2-}$ |
| $(c,e,g):78$ | $R^{x'z}_T$ | $R^{x'x}_T$ | ${}^sR^{00}_{LT'}$ | ${}^sR^{0y}_{LT'}$ | ${}^cR^{x'0}_{LT'}$ | ${}^cR^{z'0}_{LT'}$ |
| | $\mathcal{O}^c_{1+}$ | $\mathcal{O}^c_{2-}$ | $\mathcal{O}^e_{1+}$ | $\mathcal{O}^e_{1-}$ | $\mathcal{O}^g_{1-}$ | $\mathcal{O}^g_{2+}$ |
| $(c,e,g):79$ | $R^{x'z}_T$ | $R^{x'x}_T$ | ${}^cR^{00}_{LT}$ | ${}^cR^{0y}_{LT}$ | ${}^sR^{z'0}_{LT}$ | ${}^sR^{x'0}_{LT}$ |
| | $\mathcal{O}^c_{1+}$ | $\mathcal{O}^c_{2-}$ | $\mathcal{O}^e_{2+}$ | $\mathcal{O}^e_{2-}$ | $\mathcal{O}^g_{1+}$ | $\mathcal{O}^g_{2-}$ |
| $(c,e,g):80$ | $R^{x'z}_T$ | $R^{x'x}_T$ | ${}^cR^{00}_{LT}$ | ${}^cR^{0y}_{LT}$ | ${}^cR^{x'0}_{LT'}$ | ${}^cR^{z'0}_{LT'}$ |
| | $\mathcal{O}^c_{1+}$ | $\mathcal{O}^c_{2-}$ | $\mathcal{O}^e_{2+}$ | $\mathcal{O}^e_{2-}$ | $\mathcal{O}^g_{1-}$ | $\mathcal{O}^g_{2+}$ |
| $(c,e,g):81$ | $R^{x'z}_T$ | $R^{x'x}_T$ | ${}^sR^{00}_{LT'}$ | ${}^cR^{00}_{LT}$ | ${}^sR^{z'0}_{LT}$ | ${}^sR^{x'0}_{LT}$ |
| | $\mathcal{O}^c_{1+}$ | $\mathcal{O}^c_{2-}$ | $\mathcal{O}^e_{1+}$ | $\mathcal{O}^e_{2+}$ | $\mathcal{O}^g_{1+}$ | $\mathcal{O}^g_{2-}$ |
| $(c,e,g):82$ | $R^{x'z}_T$ | $R^{x'x}_T$ | ${}^sR^{00}_{LT'}$ | ${}^cR^{00}_{LT}$ | ${}^cR^{x'0}_{LT'}$ | ${}^cR^{z'0}_{LT'}$ |

| | | | | | | |
|---|---|---|---|---|---|---|
| | $\mathcal{O}^c_{1+}$ | $\mathcal{O}^c_{2-}$ | $\mathcal{O}^e_{1+}$ | $\mathcal{O}^e_{2+}$ | $\mathcal{O}^g_{1-}$ | $\mathcal{O}^g_{2+}$ |
| $(c,e,g):83$ | $R^{x'z}_T$ | $R^{x'x}_T$ | ${}^sR^{00}_{LT'}$ | ${}^cR^{0y}_{LT}$ | ${}^sR^{z'0}_{LT}$ | ${}^cR^{x'0}_{LT'}$ |
| | $\mathcal{O}^c_{1+}$ | $\mathcal{O}^c_{2-}$ | $\mathcal{O}^e_{1+}$ | $\mathcal{O}^e_{2-}$ | $\mathcal{O}^g_{1+}$ | $\mathcal{O}^g_{1-}$ |
| $(c,e,g):84$ | $R^{x'z}_T$ | $R^{x'x}_T$ | ${}^sR^{00}_{LT'}$ | ${}^cR^{0y}_{LT}$ | ${}^cR^{z'0}_{LT'}$ | ${}^sR^{x'0}_{LT}$ |
| | $\mathcal{O}^c_{1+}$ | $\mathcal{O}^c_{2-}$ | $\mathcal{O}^e_{1+}$ | $\mathcal{O}^e_{2-}$ | $\mathcal{O}^g_{2+}$ | $\mathcal{O}^g_{2-}$ |
| $(c,e,g):85$ | $R^{x'z}_T$ | $R^{x'x}_T$ | ${}^sR^{00}_{LT'}$ | ${}^cR^{0y}_{LT}$ | ${}^sR^{z'0}_{LT}$ | ${}^cR^{z'0}_{LT'}$ |
| | $\mathcal{O}^c_{1+}$ | $\mathcal{O}^c_{2-}$ | $\mathcal{O}^e_{1+}$ | $\mathcal{O}^e_{2-}$ | $\mathcal{O}^g_{1+}$ | $\mathcal{O}^g_{2+}$ |
| $(c,e,g):86$ | $R^{x'z}_T$ | $R^{x'x}_T$ | ${}^sR^{00}_{LT'}$ | ${}^cR^{0y}_{LT}$ | ${}^sR^{z'0}_{LT}$ | ${}^sR^{x'0}_{LT}$ |
| | $\mathcal{O}^c_{1+}$ | $\mathcal{O}^c_{2-}$ | $\mathcal{O}^e_{1+}$ | $\mathcal{O}^e_{2-}$ | $\mathcal{O}^g_{1+}$ | $\mathcal{O}^g_{2-}$ |
| $(c,e,g):87$ | $R^{x'z}_T$ | $R^{x'x}_T$ | ${}^sR^{00}_{LT'}$ | ${}^cR^{0y}_{LT}$ | ${}^cR^{x'0}_{LT'}$ | ${}^cR^{z'0}_{LT'}$ |
| | $\mathcal{O}^c_{1+}$ | $\mathcal{O}^c_{2-}$ | $\mathcal{O}^e_{1+}$ | $\mathcal{O}^e_{2-}$ | $\mathcal{O}^g_{1-}$ | $\mathcal{O}^g_{2+}$ |
| $(c,e,g):88$ | $R^{x'z}_T$ | $R^{x'x}_T$ | ${}^sR^{00}_{LT'}$ | ${}^cR^{0y}_{LT}$ | ${}^cR^{x'0}_{LT'}$ | ${}^sR^{x'0}_{LT}$ |
| | $\mathcal{O}^c_{1+}$ | $\mathcal{O}^c_{2-}$ | $\mathcal{O}^e_{1+}$ | $\mathcal{O}^e_{2-}$ | $\mathcal{O}^g_{1-}$ | $\mathcal{O}^g_{2-}$ |
| $(c,e,g):89$ | $R^{x'z}_T$ | $R^{x'x}_T$ | ${}^sR^{0y}_{LT'}$ | ${}^cR^{00}_{LT}$ | ${}^sR^{z'0}_{LT}$ | ${}^cR^{x'0}_{LT'}$ |
| | $\mathcal{O}^c_{1+}$ | $\mathcal{O}^c_{2-}$ | $\mathcal{O}^e_{1-}$ | $\mathcal{O}^e_{2+}$ | $\mathcal{O}^g_{1+}$ | $\mathcal{O}^g_{1-}$ |
| $(c,e,g):90$ | $R^{x'z}_T$ | $R^{x'x}_T$ | ${}^sR^{0y}_{LT'}$ | ${}^cR^{00}_{LT}$ | ${}^cR^{z'0}_{LT'}$ | ${}^sR^{x'0}_{LT}$ |
| | $\mathcal{O}^c_{1+}$ | $\mathcal{O}^c_{2-}$ | $\mathcal{O}^e_{1-}$ | $\mathcal{O}^e_{2+}$ | $\mathcal{O}^g_{2+}$ | $\mathcal{O}^g_{2-}$ |
| $(c,e,g):91$ | $R^{x'z}_T$ | $R^{x'x}_T$ | ${}^sR^{0y}_{LT'}$ | ${}^cR^{00}_{LT}$ | ${}^sR^{z'0}_{LT}$ | ${}^cR^{z'0}_{LT'}$ |
| | $\mathcal{O}^c_{1+}$ | $\mathcal{O}^c_{2-}$ | $\mathcal{O}^e_{1-}$ | $\mathcal{O}^e_{2+}$ | $\mathcal{O}^g_{1+}$ | $\mathcal{O}^g_{2+}$ |
| $(c,e,g):92$ | $R^{x'z}_T$ | $R^{x'x}_T$ | ${}^sR^{0y}_{LT'}$ | ${}^cR^{00}_{LT}$ | ${}^sR^{z'0}_{LT}$ | ${}^sR^{x'0}_{LT}$ |
| | $\mathcal{O}^c_{1+}$ | $\mathcal{O}^c_{2-}$ | $\mathcal{O}^e_{1-}$ | $\mathcal{O}^e_{2+}$ | $\mathcal{O}^g_{1+}$ | $\mathcal{O}^g_{2-}$ |
| $(c,e,g):93$ | $R^{x'z}_T$ | $R^{x'x}_T$ | ${}^sR^{0y}_{LT'}$ | ${}^cR^{00}_{LT}$ | ${}^cR^{x'0}_{LT'}$ | ${}^cR^{z'0}_{LT'}$ |
| | $\mathcal{O}^c_{1+}$ | $\mathcal{O}^c_{2-}$ | $\mathcal{O}^e_{1-}$ | $\mathcal{O}^e_{2+}$ | $\mathcal{O}^g_{1-}$ | $\mathcal{O}^g_{2+}$ |
| $(c,e,g):94$ | $R^{x'z}_T$ | $R^{x'x}_T$ | ${}^sR^{0y}_{LT'}$ | ${}^cR^{00}_{LT}$ | ${}^cR^{x'0}_{LT'}$ | ${}^sR^{x'0}_{LT}$ |
| | $\mathcal{O}^c_{1+}$ | $\mathcal{O}^c_{2-}$ | $\mathcal{O}^e_{1-}$ | $\mathcal{O}^e_{2+}$ | $\mathcal{O}^g_{1-}$ | $\mathcal{O}^g_{2-}$ |
| $(c,e,g):95$ | $R^{x'z}_T$ | $R^{x'x}_T$ | ${}^sR^{0y}_{LT'}$ | ${}^cR^{0y}_{LT}$ | ${}^sR^{z'0}_{LT}$ | ${}^sR^{x'0}_{LT}$ |
| | $\mathcal{O}^c_{1+}$ | $\mathcal{O}^c_{2-}$ | $\mathcal{O}^e_{1-}$ | $\mathcal{O}^e_{2-}$ | $\mathcal{O}^g_{1+}$ | $\mathcal{O}^g_{2-}$ |
| $(c,e,g):96$ | $R^{x'z}_T$ | $R^{x'x}_T$ | ${}^sR^{0y}_{LT'}$ | ${}^cR^{0y}_{LT}$ | ${}^cR^{x'0}_{LT'}$ | ${}^cR^{z'0}_{LT'}$ |
| | $\mathcal{O}^c_{1+}$ | $\mathcal{O}^c_{2-}$ | $\mathcal{O}^e_{1-}$ | $\mathcal{O}^e_{2-}$ | $\mathcal{O}^g_{1-}$ | $\mathcal{O}^g_{2+}$ |
| $(c,e,g):97$ | $R^{z'x}_T$ | $R^{z'z}_T$ | ${}^sR^{00}_{LT'}$ | ${}^sR^{0y}_{LT'}$ | ${}^sR^{z'0}_{LT}$ | ${}^sR^{x'0}_{LT}$ |
| | $\mathcal{O}^c_{1-}$ | $\mathcal{O}^c_{2+}$ | $\mathcal{O}^e_{1+}$ | $\mathcal{O}^e_{1-}$ | $\mathcal{O}^g_{1+}$ | $\mathcal{O}^g_{2-}$ |
| $(c,e,g):98$ | $R^{z'x}_T$ | $R^{z'z}_T$ | ${}^sR^{00}_{LT'}$ | ${}^sR^{0y}_{LT'}$ | ${}^cR^{x'0}_{LT'}$ | ${}^cR^{z'0}_{LT'}$ |
| | $\mathcal{O}^c_{1-}$ | $\mathcal{O}^c_{2+}$ | $\mathcal{O}^e_{1+}$ | $\mathcal{O}^e_{1-}$ | $\mathcal{O}^g_{1-}$ | $\mathcal{O}^g_{2+}$ |
| $(c,e,g):99$ | $R^{z'x}_T$ | $R^{z'z}_T$ | ${}^cR^{00}_{LT}$ | ${}^cR^{0y}_{LT}$ | ${}^sR^{z'0}_{LT}$ | ${}^sR^{x'0}_{LT}$ |
| | $\mathcal{O}^c_{1-}$ | $\mathcal{O}^c_{2+}$ | $\mathcal{O}^e_{2+}$ | $\mathcal{O}^e_{2-}$ | $\mathcal{O}^g_{1+}$ | $\mathcal{O}^g_{2-}$ |
| $(c,e,g):100$ | $R^{z'x}_T$ | $R^{z'z}_T$ | ${}^cR^{00}_{LT}$ | ${}^cR^{0y}_{LT}$ | ${}^cR^{x'0}_{LT'}$ | ${}^cR^{z'0}_{LT'}$ |
| | $\mathcal{O}^c_{1-}$ | $\mathcal{O}^c_{2+}$ | $\mathcal{O}^e_{2+}$ | $\mathcal{O}^e_{2-}$ | $\mathcal{O}^g_{1-}$ | $\mathcal{O}^g_{2+}$ |
| $(c,e,g):101$ | $R^{z'x}_T$ | $R^{z'z}_T$ | ${}^sR^{00}_{LT'}$ | ${}^cR^{00}_{LT}$ | ${}^sR^{z'0}_{LT}$ | ${}^sR^{x'0}_{LT}$ |
| | $\mathcal{O}^c_{1-}$ | $\mathcal{O}^c_{2+}$ | $\mathcal{O}^e_{1+}$ | $\mathcal{O}^e_{2+}$ | $\mathcal{O}^g_{1+}$ | $\mathcal{O}^g_{2-}$ |
| $(c,e,g):102$ | $R^{z'x}_T$ | $R^{z'z}_T$ | ${}^sR^{00}_{LT'}$ | ${}^cR^{00}_{LT}$ | ${}^cR^{x'0}_{LT'}$ | ${}^cR^{z'0}_{LT'}$ |
| | $\mathcal{O}^c_{1-}$ | $\mathcal{O}^c_{2+}$ | $\mathcal{O}^e_{1+}$ | $\mathcal{O}^e_{2+}$ | $\mathcal{O}^g_{1-}$ | $\mathcal{O}^g_{2+}$ |
| $(c,e,g):103$ | $R^{z'x}_T$ | $R^{z'z}_T$ | ${}^sR^{00}_{LT'}$ | ${}^cR^{0y}_{LT}$ | ${}^sR^{z'0}_{LT}$ | ${}^cR^{x'0}_{LT'}$ |
| | $\mathcal{O}^c_{1-}$ | $\mathcal{O}^c_{2+}$ | $\mathcal{O}^e_{1+}$ | $\mathcal{O}^e_{2-}$ | $\mathcal{O}^g_{1+}$ | $\mathcal{O}^g_{1-}$ |
| $(c,e,g):104$ | $R^{z'x}_T$ | $R^{z'z}_T$ | ${}^sR^{00}_{LT'}$ | ${}^cR^{0y}_{LT}$ | ${}^cR^{z'0}_{LT'}$ | ${}^sR^{x'0}_{LT}$ |
| | $\mathcal{O}^c_{1-}$ | $\mathcal{O}^c_{2+}$ | $\mathcal{O}^e_{1+}$ | $\mathcal{O}^e_{2-}$ | $\mathcal{O}^g_{2+}$ | $\mathcal{O}^g_{2-}$ |
| $(c,e,g):105$ | $R^{z'x}_T$ | $R^{z'z}_T$ | ${}^sR^{00}_{LT'}$ | ${}^cR^{0y}_{LT}$ | ${}^sR^{z'0}_{LT}$ | ${}^cR^{z'0}_{LT'}$ |
| | $\mathcal{O}^c_{1-}$ | $\mathcal{O}^c_{2+}$ | $\mathcal{O}^e_{1+}$ | $\mathcal{O}^e_{2-}$ | $\mathcal{O}^g_{1+}$ | $\mathcal{O}^g_{2+}$ |
| $(c,e,g):106$ | $R^{z'x}_T$ | $R^{z'z}_T$ | ${}^sR^{00}_{LT'}$ | ${}^cR^{0y}_{LT}$ | ${}^sR^{z'0}_{LT}$ | ${}^sR^{x'0}_{LT}$ |
| | $\mathcal{O}^c_{1-}$ | $\mathcal{O}^c_{2+}$ | $\mathcal{O}^e_{1+}$ | $\mathcal{O}^e_{2-}$ | $\mathcal{O}^g_{1+}$ | $\mathcal{O}^g_{2-}$ |
| $(c,e,g):107$ | $R^{z'x}_T$ | $R^{z'z}_T$ | ${}^sR^{00}_{LT'}$ | ${}^cR^{0y}_{LT}$ | ${}^cR^{x'0}_{LT'}$ | ${}^cR^{z'0}_{LT'}$ |
| | $\mathcal{O}^c_{1-}$ | $\mathcal{O}^c_{2+}$ | $\mathcal{O}^e_{1+}$ | $\mathcal{O}^e_{2-}$ | $\mathcal{O}^g_{1-}$ | $\mathcal{O}^g_{2+}$ |
| $(c,e,g):108$ | $R^{z'x}_T$ | $R^{z'z}_T$ | ${}^sR^{00}_{LT'}$ | ${}^cR^{0y}_{LT}$ | ${}^cR^{x'0}_{LT'}$ | ${}^sR^{x'0}_{LT}$ |
| | $\mathcal{O}^c_{1-}$ | $\mathcal{O}^c_{2+}$ | $\mathcal{O}^e_{1+}$ | $\mathcal{O}^e_{2-}$ | $\mathcal{O}^g_{1-}$ | $\mathcal{O}^g_{2-}$ |
| $(c,e,g):109$ | $R^{z'x}_T$ | $R^{z'z}_T$ | ${}^sR^{0y}_{LT'}$ | ${}^cR^{00}_{LT}$ | ${}^sR^{z'0}_{LT}$ | ${}^cR^{x'0}_{LT'}$ |
| | $\mathcal{O}^c_{1-}$ | $\mathcal{O}^c_{2+}$ | $\mathcal{O}^e_{1-}$ | $\mathcal{O}^e_{2+}$ | $\mathcal{O}^g_{1+}$ | $\mathcal{O}^g_{1-}$ |
| $(c,e,g):110$ | $R^{z'x}_T$ | $R^{z'z}_T$ | ${}^sR^{0y}_{LT'}$ | ${}^cR^{00}_{LT}$ | ${}^cR^{z'0}_{LT'}$ | ${}^sR^{x'0}_{LT}$ |
| | $\mathcal{O}^c_{1-}$ | $\mathcal{O}^c_{2+}$ | $\mathcal{O}^e_{1-}$ | $\mathcal{O}^e_{2+}$ | $\mathcal{O}^g_{2+}$ | $\mathcal{O}^g_{2-}$ |
| $(c,e,g):111$ | $R^{z'x}_T$ | $R^{z'z}_T$ | ${}^sR^{0y}_{LT'}$ | ${}^cR^{00}_{LT}$ | ${}^sR^{z'0}_{LT}$ | ${}^cR^{z'0}_{LT'}$ |

| | | | | | | |
|---|---|---|---|---|---|---|
| | $\mathcal{O}^{c}_{1-}$ | $\mathcal{O}^{c}_{2+}$ | $\mathcal{O}^{e}_{1-}$ | $\mathcal{O}^{e}_{2+}$ | $\mathcal{O}^{g}_{1+}$ | $\mathcal{O}^{g}_{2+}$ |
| $(c,e,g):112$ | $R_T^{z'x}$ | $R_T^{z'z}$ | ${}^sR_{LT'}^{0y}$ | ${}^cR_{LT}^{00}$ | ${}^sR_{LT}^{z'0}$ | ${}^sR_{LT}^{x'0}$ |
| | $\mathcal{O}^{c}_{1-}$ | $\mathcal{O}^{c}_{2+}$ | $\mathcal{O}^{e}_{1-}$ | $\mathcal{O}^{e}_{2+}$ | $\mathcal{O}^{g}_{1+}$ | $\mathcal{O}^{g}_{2-}$ |
| $(c,e,g):113$ | $R_T^{z'x}$ | $R_T^{z'z}$ | ${}^sR_{LT'}^{0y}$ | ${}^cR_{LT}^{00}$ | ${}^cR_{LT'}^{x'0}$ | ${}^cR_{LT'}^{z'0}$ |
| | $\mathcal{O}^{c}_{1-}$ | $\mathcal{O}^{c}_{2+}$ | $\mathcal{O}^{e}_{1-}$ | $\mathcal{O}^{e}_{2+}$ | $\mathcal{O}^{g}_{1-}$ | $\mathcal{O}^{g}_{2+}$ |
| $(c,e,g):114$ | $R_T^{z'x}$ | $R_T^{z'z}$ | ${}^sR_{LT'}^{0y}$ | ${}^cR_{LT}^{00}$ | ${}^cR_{LT'}^{x'0}$ | ${}^sR_{LT}^{x'0}$ |
| | $\mathcal{O}^{c}_{1-}$ | $\mathcal{O}^{c}_{2+}$ | $\mathcal{O}^{e}_{1-}$ | $\mathcal{O}^{e}_{2+}$ | $\mathcal{O}^{g}_{1-}$ | $\mathcal{O}^{g}_{2-}$ |
| $(c,e,g):115$ | $R_T^{z'x}$ | $R_T^{z'z}$ | ${}^sR_{LT'}^{0y}$ | ${}^cR_{LT}^{0y}$ | ${}^sR_{LT}^{z'0}$ | ${}^sR_{LT}^{x'0}$ |
| | $\mathcal{O}^{c}_{1-}$ | $\mathcal{O}^{c}_{2+}$ | $\mathcal{O}^{e}_{1-}$ | $\mathcal{O}^{e}_{2-}$ | $\mathcal{O}^{g}_{1+}$ | $\mathcal{O}^{g}_{2-}$ |
| $(c,e,g):116$ | $R_T^{z'x}$ | $R_T^{z'z}$ | ${}^sR_{LT'}^{0y}$ | ${}^cR_{LT}^{0y}$ | ${}^cR_{LT'}^{x'0}$ | ${}^cR_{LT'}^{z'0}$ |
| | $\mathcal{O}^{c}_{1-}$ | $\mathcal{O}^{c}_{2+}$ | $\mathcal{O}^{e}_{1-}$ | $\mathcal{O}^{e}_{2-}$ | $\mathcal{O}^{g}_{1-}$ | $\mathcal{O}^{g}_{2+}$ |
| $(c,e,g):117$ | $R_T^{z'x}$ | $R_T^{x'x}$ | ${}^sR_{LT'}^{00}$ | ${}^sR_{LT'}^{0y}$ | ${}^sR_{LT}^{z'0}$ | ${}^cR_{LT'}^{x'0}$ |
| | $\mathcal{O}^{c}_{1-}$ | $\mathcal{O}^{c}_{2-}$ | $\mathcal{O}^{e}_{1+}$ | $\mathcal{O}^{e}_{1-}$ | $\mathcal{O}^{g}_{1+}$ | $\mathcal{O}^{g}_{1-}$ |
| $(c,e,g):118$ | $R_T^{z'x}$ | $R_T^{x'x}$ | ${}^sR_{LT'}^{00}$ | ${}^sR_{LT'}^{0y}$ | ${}^cR_{LT'}^{z'0}$ | ${}^sR_{LT}^{x'0}$ |
| | $\mathcal{O}^{c}_{1-}$ | $\mathcal{O}^{c}_{2-}$ | $\mathcal{O}^{e}_{1+}$ | $\mathcal{O}^{e}_{1-}$ | $\mathcal{O}^{g}_{2+}$ | $\mathcal{O}^{g}_{2-}$ |
| $(c,e,g):119$ | $R_T^{z'x}$ | $R_T^{x'x}$ | ${}^sR_{LT'}^{00}$ | ${}^sR_{LT'}^{0y}$ | ${}^sR_{LT}^{z'0}$ | ${}^cR_{LT'}^{z'0}$ |
| | $\mathcal{O}^{c}_{1-}$ | $\mathcal{O}^{c}_{2-}$ | $\mathcal{O}^{e}_{1+}$ | $\mathcal{O}^{e}_{1-}$ | $\mathcal{O}^{g}_{1+}$ | $\mathcal{O}^{g}_{2+}$ |
| $(c,e,g):120$ | $R_T^{z'x}$ | $R_T^{x'x}$ | ${}^sR_{LT'}^{00}$ | ${}^sR_{LT'}^{0y}$ | ${}^sR_{LT}^{z'0}$ | ${}^sR_{LT}^{x'0}$ |
| | $\mathcal{O}^{c}_{1-}$ | $\mathcal{O}^{c}_{2-}$ | $\mathcal{O}^{e}_{1+}$ | $\mathcal{O}^{e}_{1-}$ | $\mathcal{O}^{g}_{1+}$ | $\mathcal{O}^{g}_{2-}$ |
| $(c,e,g):121$ | $R_T^{z'x}$ | $R_T^{x'x}$ | ${}^sR_{LT'}^{00}$ | ${}^sR_{LT'}^{0y}$ | ${}^cR_{LT'}^{x'0}$ | ${}^cR_{LT'}^{z'0}$ |
| | $\mathcal{O}^{c}_{1-}$ | $\mathcal{O}^{c}_{2-}$ | $\mathcal{O}^{e}_{1+}$ | $\mathcal{O}^{e}_{1-}$ | $\mathcal{O}^{g}_{1-}$ | $\mathcal{O}^{g}_{2+}$ |
| $(c,e,g):122$ | $R_T^{z'x}$ | $R_T^{x'x}$ | ${}^sR_{LT'}^{00}$ | ${}^sR_{LT'}^{0y}$ | ${}^cR_{LT'}^{x'0}$ | ${}^sR_{LT}^{x'0}$ |
| | $\mathcal{O}^{c}_{1-}$ | $\mathcal{O}^{c}_{2-}$ | $\mathcal{O}^{e}_{1+}$ | $\mathcal{O}^{e}_{1-}$ | $\mathcal{O}^{g}_{1-}$ | $\mathcal{O}^{g}_{2-}$ |
| $(c,e,g):123$ | $R_T^{z'x}$ | $R_T^{x'x}$ | ${}^cR_{LT}^{00}$ | ${}^cR_{LT}^{0y}$ | ${}^sR_{LT}^{z'0}$ | ${}^cR_{LT'}^{x'0}$ |
| | $\mathcal{O}^{c}_{1-}$ | $\mathcal{O}^{c}_{2-}$ | $\mathcal{O}^{e}_{2+}$ | $\mathcal{O}^{e}_{2-}$ | $\mathcal{O}^{g}_{1+}$ | $\mathcal{O}^{g}_{1-}$ |
| $(c,e,g):124$ | $R_T^{z'x}$ | $R_T^{x'x}$ | ${}^cR_{LT}^{00}$ | ${}^cR_{LT}^{0y}$ | ${}^cR_{LT'}^{z'0}$ | ${}^sR_{LT}^{x'0}$ |
| | $\mathcal{O}^{c}_{1-}$ | $\mathcal{O}^{c}_{2-}$ | $\mathcal{O}^{e}_{2+}$ | $\mathcal{O}^{e}_{2-}$ | $\mathcal{O}^{g}_{2+}$ | $\mathcal{O}^{g}_{2-}$ |
| $(c,e,g):125$ | $R_T^{z'x}$ | $R_T^{x'x}$ | ${}^cR_{LT}^{00}$ | ${}^cR_{LT}^{0y}$ | ${}^sR_{LT}^{z'0}$ | ${}^cR_{LT'}^{z'0}$ |
| | $\mathcal{O}^{c}_{1-}$ | $\mathcal{O}^{c}_{2-}$ | $\mathcal{O}^{e}_{2+}$ | $\mathcal{O}^{e}_{2-}$ | $\mathcal{O}^{g}_{1+}$ | $\mathcal{O}^{g}_{2+}$ |
| $(c,e,g):126$ | $R_T^{z'x}$ | $R_T^{x'x}$ | ${}^cR_{LT}^{00}$ | ${}^cR_{LT}^{0y}$ | ${}^sR_{LT}^{z'0}$ | ${}^sR_{LT}^{x'0}$ |
| | $\mathcal{O}^{c}_{1-}$ | $\mathcal{O}^{c}_{2-}$ | $\mathcal{O}^{e}_{2+}$ | $\mathcal{O}^{e}_{2-}$ | $\mathcal{O}^{g}_{1+}$ | $\mathcal{O}^{g}_{2-}$ |
| $(c,e,g):127$ | $R_T^{z'x}$ | $R_T^{x'x}$ | ${}^cR_{LT}^{00}$ | ${}^cR_{LT}^{0y}$ | ${}^cR_{LT'}^{x'0}$ | ${}^cR_{LT'}^{z'0}$ |
| | $\mathcal{O}^{c}_{1-}$ | $\mathcal{O}^{c}_{2-}$ | $\mathcal{O}^{e}_{2+}$ | $\mathcal{O}^{e}_{2-}$ | $\mathcal{O}^{g}_{1-}$ | $\mathcal{O}^{g}_{2+}$ |
| $(c,e,g):128$ | $R_T^{z'x}$ | $R_T^{x'x}$ | ${}^cR_{LT}^{00}$ | ${}^cR_{LT}^{0y}$ | ${}^cR_{LT'}^{x'0}$ | ${}^sR_{LT}^{x'0}$ |
| | $\mathcal{O}^{c}_{1-}$ | $\mathcal{O}^{c}_{2-}$ | $\mathcal{O}^{e}_{2+}$ | $\mathcal{O}^{e}_{2-}$ | $\mathcal{O}^{g}_{1-}$ | $\mathcal{O}^{g}_{2-}$ |
| $(c,e,g):129$ | $R_T^{z'x}$ | $R_T^{x'x}$ | ${}^sR_{LT'}^{00}$ | ${}^cR_{LT}^{00}$ | ${}^sR_{LT}^{z'0}$ | ${}^cR_{LT'}^{x'0}$ |
| | $\mathcal{O}^{c}_{1-}$ | $\mathcal{O}^{c}_{2-}$ | $\mathcal{O}^{e}_{1+}$ | $\mathcal{O}^{e}_{2+}$ | $\mathcal{O}^{g}_{1+}$ | $\mathcal{O}^{g}_{1-}$ |
| $(c,e,g):130$ | $R_T^{z'x}$ | $R_T^{x'x}$ | ${}^sR_{LT'}^{00}$ | ${}^cR_{LT}^{00}$ | ${}^cR_{LT'}^{z'0}$ | ${}^sR_{LT}^{x'0}$ |
| | $\mathcal{O}^{c}_{1-}$ | $\mathcal{O}^{c}_{2-}$ | $\mathcal{O}^{e}_{1+}$ | $\mathcal{O}^{e}_{2+}$ | $\mathcal{O}^{g}_{2+}$ | $\mathcal{O}^{g}_{2-}$ |
| $(c,e,g):131$ | $R_T^{z'x}$ | $R_T^{x'x}$ | ${}^sR_{LT'}^{00}$ | ${}^cR_{LT}^{00}$ | ${}^sR_{LT}^{z'0}$ | ${}^cR_{LT'}^{z'0}$ |
| | $\mathcal{O}^{c}_{1-}$ | $\mathcal{O}^{c}_{2-}$ | $\mathcal{O}^{e}_{1+}$ | $\mathcal{O}^{e}_{2+}$ | $\mathcal{O}^{g}_{1+}$ | $\mathcal{O}^{g}_{2+}$ |
| $(c,e,g):132$ | $R_T^{z'x}$ | $R_T^{x'x}$ | ${}^sR_{LT'}^{00}$ | ${}^cR_{LT}^{00}$ | ${}^sR_{LT}^{z'0}$ | ${}^sR_{LT}^{x'0}$ |
| | $\mathcal{O}^{c}_{1-}$ | $\mathcal{O}^{c}_{2-}$ | $\mathcal{O}^{e}_{1+}$ | $\mathcal{O}^{e}_{2+}$ | $\mathcal{O}^{g}_{1+}$ | $\mathcal{O}^{g}_{2-}$ |
| $(c,e,g):133$ | $R_T^{z'x}$ | $R_T^{x'x}$ | ${}^sR_{LT'}^{00}$ | ${}^cR_{LT}^{00}$ | ${}^cR_{LT'}^{x'0}$ | ${}^cR_{LT'}^{z'0}$ |
| | $\mathcal{O}^{c}_{1-}$ | $\mathcal{O}^{c}_{2-}$ | $\mathcal{O}^{e}_{1+}$ | $\mathcal{O}^{e}_{2+}$ | $\mathcal{O}^{g}_{1-}$ | $\mathcal{O}^{g}_{2+}$ |
| $(c,e,g):134$ | $R_T^{z'x}$ | $R_T^{x'x}$ | ${}^sR_{LT'}^{00}$ | ${}^cR_{LT}^{00}$ | ${}^cR_{LT'}^{x'0}$ | ${}^sR_{LT}^{x'0}$ |
| | $\mathcal{O}^{c}_{1-}$ | $\mathcal{O}^{c}_{2-}$ | $\mathcal{O}^{e}_{1+}$ | $\mathcal{O}^{e}_{2+}$ | $\mathcal{O}^{g}_{1-}$ | $\mathcal{O}^{g}_{2-}$ |
| $(c,e,g):135$ | $R_T^{z'x}$ | $R_T^{x'x}$ | ${}^sR_{LT'}^{00}$ | ${}^cR_{LT}^{0y}$ | ${}^sR_{LT}^{z'0}$ | ${}^cR_{LT'}^{x'0}$ |
| | $\mathcal{O}^{c}_{1-}$ | $\mathcal{O}^{c}_{2-}$ | $\mathcal{O}^{e}_{1+}$ | $\mathcal{O}^{e}_{2-}$ | $\mathcal{O}^{g}_{1+}$ | $\mathcal{O}^{g}_{1-}$ |
| $(c,e,g):136$ | $R_T^{z'x}$ | $R_T^{x'x}$ | ${}^sR_{LT'}^{00}$ | ${}^cR_{LT}^{0y}$ | ${}^cR_{LT'}^{z'0}$ | ${}^sR_{LT}^{x'0}$ |
| | $\mathcal{O}^{c}_{1-}$ | $\mathcal{O}^{c}_{2-}$ | $\mathcal{O}^{e}_{1+}$ | $\mathcal{O}^{e}_{2-}$ | $\mathcal{O}^{g}_{2+}$ | $\mathcal{O}^{g}_{2-}$ |
| $(c,e,g):137$ | $R_T^{z'x}$ | $R_T^{x'x}$ | ${}^sR_{LT'}^{00}$ | ${}^cR_{LT}^{0y}$ | ${}^sR_{LT}^{z'0}$ | ${}^cR_{LT'}^{z'0}$ |
| | $\mathcal{O}^{c}_{1-}$ | $\mathcal{O}^{c}_{2-}$ | $\mathcal{O}^{e}_{1+}$ | $\mathcal{O}^{e}_{2-}$ | $\mathcal{O}^{g}_{1+}$ | $\mathcal{O}^{g}_{2+}$ |
| $(c,e,g):138$ | $R_T^{z'x}$ | $R_T^{x'x}$ | ${}^sR_{LT'}^{00}$ | ${}^cR_{LT}^{0y}$ | ${}^sR_{LT}^{z'0}$ | ${}^sR_{LT}^{x'0}$ |
| | $\mathcal{O}^{c}_{1-}$ | $\mathcal{O}^{c}_{2-}$ | $\mathcal{O}^{e}_{1+}$ | $\mathcal{O}^{e}_{2-}$ | $\mathcal{O}^{g}_{1+}$ | $\mathcal{O}^{g}_{2-}$ |
| $(c,e,g):139$ | $R_T^{z'x}$ | $R_T^{x'x}$ | ${}^sR_{LT'}^{00}$ | ${}^cR_{LT}^{0y}$ | ${}^cR_{LT'}^{x'0}$ | ${}^cR_{LT'}^{z'0}$ |
| | $\mathcal{O}^{c}_{1-}$ | $\mathcal{O}^{c}_{2-}$ | $\mathcal{O}^{e}_{1+}$ | $\mathcal{O}^{e}_{2-}$ | $\mathcal{O}^{g}_{1-}$ | $\mathcal{O}^{g}_{2+}$ |
| $(c,e,g):140$ | $R_T^{z'x}$ | $R_T^{x'x}$ | ${}^sR_{LT'}^{00}$ | ${}^cR_{LT}^{0y}$ | ${}^cR_{LT'}^{x'0}$ | ${}^sR_{LT}^{x'0}$ |

| | | | | | | |
|---|---|---|---|---|---|---|
| | $\mathcal{O}^{c}_{1-}$ | $\mathcal{O}^{c}_{2-}$ | $\mathcal{O}^{e}_{1+}$ | $\mathcal{O}^{e}_{2-}$ | $\mathcal{O}^{g}_{1-}$ | $\mathcal{O}^{g}_{2-}$ |
| $(c,e,g):141$ | $R^{z'x}_{T}$ | $R^{x'x}_{T}$ | ${}^{s}R^{0y}_{LT'}$ | ${}^{c}R^{00}_{LT}$ | ${}^{s}R^{z'0}_{LT}$ | ${}^{c}R^{x'0}_{LT'}$ |
| | $\mathcal{O}^{c}_{1-}$ | $\mathcal{O}^{c}_{2-}$ | $\mathcal{O}^{e}_{1-}$ | $\mathcal{O}^{e}_{2+}$ | $\mathcal{O}^{g}_{1+}$ | $\mathcal{O}^{g}_{1-}$ |
| $(c,e,g):142$ | $R^{z'x}_{T}$ | $R^{x'x}_{T}$ | ${}^{s}R^{0y}_{LT'}$ | ${}^{c}R^{00}_{LT}$ | ${}^{c}R^{z'0}_{LT'}$ | ${}^{s}R^{x'0}_{LT}$ |
| | $\mathcal{O}^{c}_{1-}$ | $\mathcal{O}^{c}_{2-}$ | $\mathcal{O}^{e}_{1-}$ | $\mathcal{O}^{e}_{2+}$ | $\mathcal{O}^{g}_{2+}$ | $\mathcal{O}^{g}_{2-}$ |
| $(c,e,g):143$ | $R^{z'x}_{T}$ | $R^{x'x}_{T}$ | ${}^{s}R^{0y}_{LT'}$ | ${}^{c}R^{00}_{LT}$ | ${}^{s}R^{z'0}_{LT}$ | ${}^{c}R^{z'0}_{LT'}$ |
| | $\mathcal{O}^{c}_{1-}$ | $\mathcal{O}^{c}_{2-}$ | $\mathcal{O}^{e}_{1-}$ | $\mathcal{O}^{e}_{2+}$ | $\mathcal{O}^{g}_{1+}$ | $\mathcal{O}^{g}_{2+}$ |
| $(c,e,g):144$ | $R^{z'x}_{T}$ | $R^{x'x}_{T}$ | ${}^{s}R^{0y}_{LT'}$ | ${}^{c}R^{00}_{LT}$ | ${}^{s}R^{z'0}_{LT}$ | ${}^{s}R^{x'0}_{LT}$ |
| | $\mathcal{O}^{c}_{1-}$ | $\mathcal{O}^{c}_{2-}$ | $\mathcal{O}^{e}_{1-}$ | $\mathcal{O}^{e}_{2+}$ | $\mathcal{O}^{g}_{1+}$ | $\mathcal{O}^{g}_{2-}$ |
| $(c,e,g):145$ | $R^{z'x}_{T}$ | $R^{x'x}_{T}$ | ${}^{s}R^{0y}_{LT'}$ | ${}^{c}R^{00}_{LT}$ | ${}^{c}R^{x'0}_{LT'}$ | ${}^{c}R^{z'0}_{LT'}$ |
| | $\mathcal{O}^{c}_{1-}$ | $\mathcal{O}^{c}_{2-}$ | $\mathcal{O}^{e}_{1-}$ | $\mathcal{O}^{e}_{2+}$ | $\mathcal{O}^{g}_{1-}$ | $\mathcal{O}^{g}_{2+}$ |
| $(c,e,g):146$ | $R^{z'x}_{T}$ | $R^{x'x}_{T}$ | ${}^{s}R^{0y}_{LT'}$ | ${}^{c}R^{00}_{LT}$ | ${}^{c}R^{x'0}_{LT'}$ | ${}^{s}R^{x'0}_{LT}$ |
| | $\mathcal{O}^{c}_{1-}$ | $\mathcal{O}^{c}_{2-}$ | $\mathcal{O}^{e}_{1-}$ | $\mathcal{O}^{e}_{2+}$ | $\mathcal{O}^{g}_{1-}$ | $\mathcal{O}^{g}_{2-}$ |
| $(c,e,g):147$ | $R^{z'x}_{T}$ | $R^{x'x}_{T}$ | ${}^{s}R^{0y}_{LT'}$ | ${}^{c}R^{0y}_{LT}$ | ${}^{s}R^{z'0}_{LT}$ | ${}^{c}R^{x'0}_{LT'}$ |
| | $\mathcal{O}^{c}_{1-}$ | $\mathcal{O}^{c}_{2-}$ | $\mathcal{O}^{e}_{1-}$ | $\mathcal{O}^{e}_{2-}$ | $\mathcal{O}^{g}_{1+}$ | $\mathcal{O}^{g}_{1-}$ |
| $(c,e,g):148$ | $R^{z'x}_{T}$ | $R^{x'x}_{T}$ | ${}^{s}R^{0y}_{LT'}$ | ${}^{c}R^{0y}_{LT}$ | ${}^{c}R^{z'0}_{LT'}$ | ${}^{s}R^{x'0}_{LT}$ |
| | $\mathcal{O}^{c}_{1-}$ | $\mathcal{O}^{c}_{2-}$ | $\mathcal{O}^{e}_{1-}$ | $\mathcal{O}^{e}_{2-}$ | $\mathcal{O}^{g}_{2+}$ | $\mathcal{O}^{g}_{2-}$ |
| $(c,e,g):149$ | $R^{z'x}_{T}$ | $R^{x'x}_{T}$ | ${}^{s}R^{0y}_{LT'}$ | ${}^{c}R^{0y}_{LT}$ | ${}^{s}R^{z'0}_{LT}$ | ${}^{c}R^{z'0}_{LT'}$ |
| | $\mathcal{O}^{c}_{1-}$ | $\mathcal{O}^{c}_{2-}$ | $\mathcal{O}^{e}_{1-}$ | $\mathcal{O}^{e}_{2-}$ | $\mathcal{O}^{g}_{1+}$ | $\mathcal{O}^{g}_{2+}$ |
| $(c,e,g):150$ | $R^{z'x}_{T}$ | $R^{x'x}_{T}$ | ${}^{s}R^{0y}_{LT'}$ | ${}^{c}R^{0y}_{LT}$ | ${}^{s}R^{z'0}_{LT}$ | ${}^{s}R^{x'0}_{LT}$ |
| | $\mathcal{O}^{c}_{1-}$ | $\mathcal{O}^{c}_{2-}$ | $\mathcal{O}^{e}_{1-}$ | $\mathcal{O}^{e}_{2-}$ | $\mathcal{O}^{g}_{1+}$ | $\mathcal{O}^{g}_{2-}$ |
| $(c,e,g):151$ | $R^{z'x}_{T}$ | $R^{x'x}_{T}$ | ${}^{s}R^{0y}_{LT'}$ | ${}^{c}R^{0y}_{LT}$ | ${}^{c}R^{x'0}_{LT'}$ | ${}^{c}R^{z'0}_{LT'}$ |
| | $\mathcal{O}^{c}_{1-}$ | $\mathcal{O}^{c}_{2-}$ | $\mathcal{O}^{e}_{1-}$ | $\mathcal{O}^{e}_{2-}$ | $\mathcal{O}^{g}_{1-}$ | $\mathcal{O}^{g}_{2+}$ |
| $(c,e,g):152$ | $R^{z'x}_{T}$ | $R^{x'x}_{T}$ | ${}^{s}R^{0y}_{LT'}$ | ${}^{c}R^{0y}_{LT}$ | ${}^{c}R^{x'0}_{LT'}$ | ${}^{s}R^{x'0}_{LT}$ |
| | $\mathcal{O}^{c}_{1-}$ | $\mathcal{O}^{c}_{2-}$ | $\mathcal{O}^{e}_{1-}$ | $\mathcal{O}^{e}_{2-}$ | $\mathcal{O}^{g}_{1-}$ | $\mathcal{O}^{g}_{2-}$ |

TABLE X: All the fully complete sets determined from the combination of shape-classes $(c,f,h)$ (i.e. graph-topology 'VII') in the case of pseudoscalar meson electroproduction are listed here. The observables are written in the systematic symbolic notation $\mathcal{O}^{n}_{\nu\pm}$ by Nakayama [1], as well as in the more commonly used notation in terms of 'response-functions' $R^{\beta\alpha}_{i}$ (cf. references [4, 5]). The given sets of 6 observables have to be combined with the 6 'diagonal' observables $\left\{R^{00}_{T}, {}^{c}R^{00}_{TT}, R^{0y}_{T}, R^{y'0}_{T}, R^{00}_{L}, R^{0y}_{L}\right\}$ in order to form a complete set of minimal length $2N = 12$. All of these sets have been verified to be complete using Mathematica [3].

| Set-Nr. | Observables | | | | | |
|---|---|---|---|---|---|---|
| $(c,f,h):1$ | $R^{x'z}_{T}$ | $R^{z'x}_{T}$ | ${}^{s}R^{0z}_{LT}$ | ${}^{c}R^{0x}_{LT'}$ | ${}^{s}R^{x'x}_{LT'}$ | ${}^{s}R^{z'x}_{LT'}$ |
| | $\mathcal{O}^{c}_{1+}$ | $\mathcal{O}^{c}_{1-}$ | $\mathcal{O}^{f}_{1+}$ | $\mathcal{O}^{f}_{1-}$ | $\mathcal{O}^{h}_{1+}$ | $\mathcal{O}^{h}_{2-}$ |
| $(c,f,h):2$ | $R^{x'z}_{T}$ | $R^{z'x}_{T}$ | ${}^{s}R^{0z}_{LT}$ | ${}^{c}R^{0x}_{LT'}$ | ${}^{c}R^{z'x}_{LT}$ | ${}^{c}R^{x'x}_{LT}$ |
| | $\mathcal{O}^{c}_{1+}$ | $\mathcal{O}^{c}_{1-}$ | $\mathcal{O}^{f}_{1+}$ | $\mathcal{O}^{f}_{1-}$ | $\mathcal{O}^{h}_{1-}$ | $\mathcal{O}^{h}_{2+}$ |
| $(c,f,h):3$ | $R^{x'z}_{T}$ | $R^{z'x}_{T}$ | ${}^{c}R^{0z}_{LT'}$ | ${}^{s}R^{0x}_{LT}$ | ${}^{s}R^{x'x}_{LT'}$ | ${}^{s}R^{z'x}_{LT'}$ |
| | $\mathcal{O}^{c}_{1+}$ | $\mathcal{O}^{c}_{1-}$ | $\mathcal{O}^{f}_{2+}$ | $\mathcal{O}^{f}_{2-}$ | $\mathcal{O}^{h}_{1+}$ | $\mathcal{O}^{h}_{2-}$ |
| $(c,f,h):4$ | $R^{x'z}_{T}$ | $R^{z'x}_{T}$ | ${}^{c}R^{0z}_{LT'}$ | ${}^{s}R^{0x}_{LT}$ | ${}^{c}R^{z'x}_{LT}$ | ${}^{c}R^{x'x}_{LT}$ |
| | $\mathcal{O}^{c}_{1+}$ | $\mathcal{O}^{c}_{1-}$ | $\mathcal{O}^{f}_{2+}$ | $\mathcal{O}^{f}_{2-}$ | $\mathcal{O}^{h}_{1-}$ | $\mathcal{O}^{h}_{2+}$ |
| $(c,f,h):5$ | $R^{x'z}_{T}$ | $R^{z'x}_{T}$ | ${}^{s}R^{0z}_{LT}$ | ${}^{c}R^{0z}_{LT'}$ | ${}^{s}R^{x'x}_{LT'}$ | ${}^{s}R^{z'x}_{LT'}$ |
| | $\mathcal{O}^{c}_{1+}$ | $\mathcal{O}^{c}_{1-}$ | $\mathcal{O}^{f}_{1+}$ | $\mathcal{O}^{f}_{2+}$ | $\mathcal{O}^{h}_{1+}$ | $\mathcal{O}^{h}_{2-}$ |
| $(c,f,h):6$ | $R^{x'z}_{T}$ | $R^{z'x}_{T}$ | ${}^{s}R^{0z}_{LT}$ | ${}^{c}R^{0z}_{LT'}$ | ${}^{c}R^{z'x}_{LT}$ | ${}^{c}R^{x'x}_{LT}$ |
| | $\mathcal{O}^{c}_{1+}$ | $\mathcal{O}^{c}_{1-}$ | $\mathcal{O}^{f}_{1+}$ | $\mathcal{O}^{f}_{2+}$ | $\mathcal{O}^{h}_{1-}$ | $\mathcal{O}^{h}_{2+}$ |
| $(c,f,h):7$ | $R^{x'z}_{T}$ | $R^{z'x}_{T}$ | ${}^{s}R^{0z}_{LT}$ | ${}^{s}R^{0x}_{LT}$ | ${}^{s}R^{x'x}_{LT'}$ | ${}^{c}R^{z'x}_{LT}$ |
| | $\mathcal{O}^{c}_{1+}$ | $\mathcal{O}^{c}_{1-}$ | $\mathcal{O}^{f}_{1+}$ | $\mathcal{O}^{f}_{2-}$ | $\mathcal{O}^{h}_{1+}$ | $\mathcal{O}^{h}_{1-}$ |
| $(c,f,h):8$ | $R^{x'z}_{T}$ | $R^{z'x}_{T}$ | ${}^{s}R^{0z}_{LT}$ | ${}^{s}R^{0x}_{LT}$ | ${}^{c}R^{x'x}_{LT}$ | ${}^{s}R^{z'x}_{LT'}$ |
| | $\mathcal{O}^{c}_{1+}$ | $\mathcal{O}^{c}_{1-}$ | $\mathcal{O}^{f}_{1+}$ | $\mathcal{O}^{f}_{2-}$ | $\mathcal{O}^{h}_{2+}$ | $\mathcal{O}^{h}_{2-}$ |
| $(c,f,h):9$ | $R^{x'z}_{T}$ | $R^{z'x}_{T}$ | ${}^{s}R^{0z}_{LT}$ | ${}^{s}R^{0x}_{LT}$ | ${}^{s}R^{x'x}_{LT'}$ | ${}^{c}R^{x'x}_{LT}$ |

| | | | | | | |
|---|---|---|---|---|---|---|
| | $\mathcal{O}^c_{1+}$ | $\mathcal{O}^c_{1-}$ | $\mathcal{O}^f_{1+}$ | $\mathcal{O}^f_{2-}$ | $\mathcal{O}^h_{1+}$ | $\mathcal{O}^h_{2+}$ |
| $(c,f,h):10$ | $R_T^{x'z}$ | $R_T^{z'x}$ | ${}^sR_{LT}^{0z}$ | ${}^sR_{LT}^{0x}$ | ${}^sR_{LT'}^{x'x}$ | ${}^sR_{LT'}^{z'x}$ |
| | $\mathcal{O}^c_{1+}$ | $\mathcal{O}^c_{1-}$ | $\mathcal{O}^f_{1+}$ | $\mathcal{O}^f_{2-}$ | $\mathcal{O}^h_{1+}$ | $\mathcal{O}^h_{2-}$ |
| $(c,f,h):11$ | $R_T^{x'z}$ | $R_T^{z'x}$ | ${}^sR_{LT}^{0z}$ | ${}^sR_{LT}^{0x}$ | ${}^cR_{LT}^{z'x}$ | ${}^cR_{LT}^{x'x}$ |
| | $\mathcal{O}^c_{1+}$ | $\mathcal{O}^c_{1-}$ | $\mathcal{O}^f_{1+}$ | $\mathcal{O}^f_{2-}$ | $\mathcal{O}^h_{1-}$ | $\mathcal{O}^h_{2+}$ |
| $(c,f,h):12$ | $R_T^{x'z}$ | $R_T^{z'x}$ | ${}^sR_{LT}^{0z}$ | ${}^sR_{LT}^{0x}$ | ${}^cR_{LT}^{z'x}$ | ${}^sR_{LT'}^{z'x}$ |
| | $\mathcal{O}^c_{1+}$ | $\mathcal{O}^c_{1-}$ | $\mathcal{O}^f_{1+}$ | $\mathcal{O}^f_{2-}$ | $\mathcal{O}^h_{1-}$ | $\mathcal{O}^h_{2-}$ |
| $(c,f,h):13$ | $R_T^{x'z}$ | $R_T^{z'x}$ | ${}^cR_{LT'}^{0x}$ | ${}^cR_{LT'}^{0z}$ | ${}^sR_{LT'}^{x'x}$ | ${}^cR_{LT}^{z'x}$ |
| | $\mathcal{O}^c_{1+}$ | $\mathcal{O}^c_{1-}$ | $\mathcal{O}^f_{1-}$ | $\mathcal{O}^f_{2+}$ | $\mathcal{O}^h_{1+}$ | $\mathcal{O}^h_{1-}$ |
| $(c,f,h):14$ | $R_T^{x'z}$ | $R_T^{z'x}$ | ${}^cR_{LT'}^{0x}$ | ${}^cR_{LT'}^{0z}$ | ${}^cR_{LT}^{x'x}$ | ${}^sR_{LT'}^{z'x}$ |
| | $\mathcal{O}^c_{1+}$ | $\mathcal{O}^c_{1-}$ | $\mathcal{O}^f_{1-}$ | $\mathcal{O}^f_{2+}$ | $\mathcal{O}^h_{2+}$ | $\mathcal{O}^h_{2-}$ |
| $(c,f,h):15$ | $R_T^{x'z}$ | $R_T^{z'x}$ | ${}^cR_{LT'}^{0x}$ | ${}^cR_{LT'}^{0z}$ | ${}^sR_{LT'}^{x'x}$ | ${}^cR_{LT}^{x'x}$ |
| | $\mathcal{O}^c_{1+}$ | $\mathcal{O}^c_{1-}$ | $\mathcal{O}^f_{1-}$ | $\mathcal{O}^f_{2+}$ | $\mathcal{O}^h_{1+}$ | $\mathcal{O}^h_{2+}$ |
| $(c,f,h):16$ | $R_T^{x'z}$ | $R_T^{z'x}$ | ${}^cR_{LT'}^{0x}$ | ${}^cR_{LT'}^{0z}$ | ${}^sR_{LT'}^{x'x}$ | ${}^sR_{LT'}^{z'x}$ |
| | $\mathcal{O}^c_{1+}$ | $\mathcal{O}^c_{1-}$ | $\mathcal{O}^f_{1-}$ | $\mathcal{O}^f_{2+}$ | $\mathcal{O}^h_{1+}$ | $\mathcal{O}^h_{2-}$ |
| $(c,f,h):17$ | $R_T^{x'z}$ | $R_T^{z'x}$ | ${}^cR_{LT'}^{0x}$ | ${}^cR_{LT'}^{0z}$ | ${}^cR_{LT}^{z'x}$ | ${}^cR_{LT}^{x'x}$ |
| | $\mathcal{O}^c_{1+}$ | $\mathcal{O}^c_{1-}$ | $\mathcal{O}^f_{1-}$ | $\mathcal{O}^f_{2+}$ | $\mathcal{O}^h_{1-}$ | $\mathcal{O}^h_{2+}$ |
| $(c,f,h):18$ | $R_T^{x'z}$ | $R_T^{z'x}$ | ${}^cR_{LT'}^{0x}$ | ${}^cR_{LT'}^{0z}$ | ${}^cR_{LT}^{z'x}$ | ${}^sR_{LT'}^{z'x}$ |
| | $\mathcal{O}^c_{1+}$ | $\mathcal{O}^c_{1-}$ | $\mathcal{O}^f_{1-}$ | $\mathcal{O}^f_{2+}$ | $\mathcal{O}^h_{1-}$ | $\mathcal{O}^h_{2-}$ |
| $(c,f,h):19$ | $R_T^{x'z}$ | $R_T^{z'x}$ | ${}^cR_{LT'}^{0x}$ | ${}^sR_{LT}^{0x}$ | ${}^sR_{LT'}^{x'x}$ | ${}^sR_{LT'}^{z'x}$ |
| | $\mathcal{O}^c_{1+}$ | $\mathcal{O}^c_{1-}$ | $\mathcal{O}^f_{1-}$ | $\mathcal{O}^f_{2-}$ | $\mathcal{O}^h_{1+}$ | $\mathcal{O}^h_{2-}$ |
| $(c,f,h):20$ | $R_T^{x'z}$ | $R_T^{z'x}$ | ${}^cR_{LT'}^{0x}$ | ${}^sR_{LT}^{0x}$ | ${}^cR_{LT}^{z'x}$ | ${}^cR_{LT}^{x'x}$ |
| | $\mathcal{O}^c_{1+}$ | $\mathcal{O}^c_{1-}$ | $\mathcal{O}^f_{1-}$ | $\mathcal{O}^f_{2-}$ | $\mathcal{O}^h_{1-}$ | $\mathcal{O}^h_{2+}$ |
| $(c,f,h):21$ | $R_T^{z'z}$ | $R_T^{x'x}$ | ${}^sR_{LT}^{0z}$ | ${}^cR_{LT'}^{0x}$ | ${}^sR_{LT'}^{x'x}$ | ${}^sR_{LT'}^{z'x}$ |
| | $\mathcal{O}^c_{2+}$ | $\mathcal{O}^c_{2-}$ | $\mathcal{O}^f_{1+}$ | $\mathcal{O}^f_{1-}$ | $\mathcal{O}^h_{1+}$ | $\mathcal{O}^h_{2-}$ |
| $(c,f,h):22$ | $R_T^{z'z}$ | $R_T^{x'x}$ | ${}^sR_{LT}^{0z}$ | ${}^cR_{LT'}^{0x}$ | ${}^cR_{LT}^{z'x}$ | ${}^cR_{LT}^{x'x}$ |
| | $\mathcal{O}^c_{2+}$ | $\mathcal{O}^c_{2-}$ | $\mathcal{O}^f_{1+}$ | $\mathcal{O}^f_{1-}$ | $\mathcal{O}^h_{1-}$ | $\mathcal{O}^h_{2+}$ |
| $(c,f,h):23$ | $R_T^{z'z}$ | $R_T^{x'x}$ | ${}^cR_{LT'}^{0z}$ | ${}^sR_{LT}^{0x}$ | ${}^sR_{LT'}^{x'x}$ | ${}^sR_{LT'}^{z'x}$ |
| | $\mathcal{O}^c_{2+}$ | $\mathcal{O}^c_{2-}$ | $\mathcal{O}^f_{2+}$ | $\mathcal{O}^f_{2-}$ | $\mathcal{O}^h_{1+}$ | $\mathcal{O}^h_{2-}$ |
| $(c,f,h):24$ | $R_T^{z'z}$ | $R_T^{x'x}$ | ${}^cR_{LT'}^{0z}$ | ${}^sR_{LT}^{0x}$ | ${}^cR_{LT}^{z'x}$ | ${}^cR_{LT}^{x'x}$ |
| | $\mathcal{O}^c_{2+}$ | $\mathcal{O}^c_{2-}$ | $\mathcal{O}^f_{2+}$ | $\mathcal{O}^f_{2-}$ | $\mathcal{O}^h_{1-}$ | $\mathcal{O}^h_{2+}$ |
| $(c,f,h):25$ | $R_T^{z'z}$ | $R_T^{x'x}$ | ${}^sR_{LT}^{0z}$ | ${}^cR_{LT'}^{0z}$ | ${}^sR_{LT'}^{x'x}$ | ${}^sR_{LT'}^{z'x}$ |
| | $\mathcal{O}^c_{2+}$ | $\mathcal{O}^c_{2-}$ | $\mathcal{O}^f_{1+}$ | $\mathcal{O}^f_{2+}$ | $\mathcal{O}^h_{1+}$ | $\mathcal{O}^h_{2-}$ |
| $(c,f,h):26$ | $R_T^{z'z}$ | $R_T^{x'x}$ | ${}^sR_{LT}^{0z}$ | ${}^cR_{LT'}^{0z}$ | ${}^cR_{LT}^{z'x}$ | ${}^cR_{LT}^{x'x}$ |
| | $\mathcal{O}^c_{2+}$ | $\mathcal{O}^c_{2-}$ | $\mathcal{O}^f_{1+}$ | $\mathcal{O}^f_{2+}$ | $\mathcal{O}^h_{1-}$ | $\mathcal{O}^h_{2+}$ |
| $(c,f,h):27$ | $R_T^{z'z}$ | $R_T^{x'x}$ | ${}^sR_{LT}^{0z}$ | ${}^sR_{LT}^{0x}$ | ${}^sR_{LT'}^{x'x}$ | ${}^cR_{LT}^{z'x}$ |
| | $\mathcal{O}^c_{2+}$ | $\mathcal{O}^c_{2-}$ | $\mathcal{O}^f_{1+}$ | $\mathcal{O}^f_{2-}$ | $\mathcal{O}^h_{1+}$ | $\mathcal{O}^h_{1-}$ |
| $(c,f,h):28$ | $R_T^{z'z}$ | $R_T^{x'x}$ | ${}^sR_{LT}^{0z}$ | ${}^sR_{LT}^{0x}$ | ${}^cR_{LT}^{x'x}$ | ${}^sR_{LT'}^{z'x}$ |
| | $\mathcal{O}^c_{2+}$ | $\mathcal{O}^c_{2-}$ | $\mathcal{O}^f_{1+}$ | $\mathcal{O}^f_{2-}$ | $\mathcal{O}^h_{2+}$ | $\mathcal{O}^h_{2-}$ |
| $(c,f,h):29$ | $R_T^{z'z}$ | $R_T^{x'x}$ | ${}^sR_{LT}^{0z}$ | ${}^sR_{LT}^{0x}$ | ${}^sR_{LT'}^{x'x}$ | ${}^cR_{LT}^{x'x}$ |
| | $\mathcal{O}^c_{2+}$ | $\mathcal{O}^c_{2-}$ | $\mathcal{O}^f_{1+}$ | $\mathcal{O}^f_{2-}$ | $\mathcal{O}^h_{1+}$ | $\mathcal{O}^h_{2+}$ |
| $(c,f,h):30$ | $R_T^{z'z}$ | $R_T^{x'x}$ | ${}^sR_{LT}^{0z}$ | ${}^sR_{LT}^{0x}$ | ${}^sR_{LT'}^{x'x}$ | ${}^sR_{LT'}^{z'x}$ |
| | $\mathcal{O}^c_{2+}$ | $\mathcal{O}^c_{2-}$ | $\mathcal{O}^f_{1+}$ | $\mathcal{O}^f_{2-}$ | $\mathcal{O}^h_{1+}$ | $\mathcal{O}^h_{2-}$ |
| $(c,f,h):31$ | $R_T^{z'z}$ | $R_T^{x'x}$ | ${}^sR_{LT}^{0z}$ | ${}^sR_{LT}^{0x}$ | ${}^cR_{LT}^{z'x}$ | ${}^cR_{LT}^{x'x}$ |
| | $\mathcal{O}^c_{2+}$ | $\mathcal{O}^c_{2-}$ | $\mathcal{O}^f_{1+}$ | $\mathcal{O}^f_{2-}$ | $\mathcal{O}^h_{1-}$ | $\mathcal{O}^h_{2+}$ |
| $(c,f,h):32$ | $R_T^{z'z}$ | $R_T^{x'x}$ | ${}^sR_{LT}^{0z}$ | ${}^sR_{LT}^{0x}$ | ${}^cR_{LT}^{z'x}$ | ${}^sR_{LT'}^{z'x}$ |
| | $\mathcal{O}^c_{2+}$ | $\mathcal{O}^c_{2-}$ | $\mathcal{O}^f_{1+}$ | $\mathcal{O}^f_{2-}$ | $\mathcal{O}^h_{1-}$ | $\mathcal{O}^h_{2-}$ |
| $(c,f,h):33$ | $R_T^{z'z}$ | $R_T^{x'x}$ | ${}^cR_{LT'}^{0x}$ | ${}^cR_{LT'}^{0z}$ | ${}^sR_{LT'}^{x'x}$ | ${}^cR_{LT}^{z'x}$ |
| | $\mathcal{O}^c_{2+}$ | $\mathcal{O}^c_{2-}$ | $\mathcal{O}^f_{1-}$ | $\mathcal{O}^f_{2+}$ | $\mathcal{O}^h_{1+}$ | $\mathcal{O}^h_{1-}$ |
| $(c,f,h):34$ | $R_T^{z'z}$ | $R_T^{x'x}$ | ${}^cR_{LT'}^{0x}$ | ${}^cR_{LT'}^{0z}$ | ${}^cR_{LT}^{x'x}$ | ${}^sR_{LT'}^{z'x}$ |
| | $\mathcal{O}^c_{2+}$ | $\mathcal{O}^c_{2-}$ | $\mathcal{O}^f_{1-}$ | $\mathcal{O}^f_{2+}$ | $\mathcal{O}^h_{2+}$ | $\mathcal{O}^h_{2-}$ |
| $(c,f,h):35$ | $R_T^{z'z}$ | $R_T^{x'x}$ | ${}^cR_{LT'}^{0x}$ | ${}^cR_{LT'}^{0z}$ | ${}^sR_{LT'}^{x'x}$ | ${}^cR_{LT}^{x'x}$ |
| | $\mathcal{O}^c_{2+}$ | $\mathcal{O}^c_{2-}$ | $\mathcal{O}^f_{1-}$ | $\mathcal{O}^f_{2+}$ | $\mathcal{O}^h_{1+}$ | $\mathcal{O}^h_{2+}$ |
| $(c,f,h):36$ | $R_T^{z'z}$ | $R_T^{x'x}$ | ${}^cR_{LT'}^{0x}$ | ${}^cR_{LT'}^{0z}$ | ${}^sR_{LT'}^{x'x}$ | ${}^sR_{LT'}^{z'x}$ |
| | $\mathcal{O}^c_{2+}$ | $\mathcal{O}^c_{2-}$ | $\mathcal{O}^f_{1-}$ | $\mathcal{O}^f_{2+}$ | $\mathcal{O}^h_{1+}$ | $\mathcal{O}^h_{2-}$ |

| | | | | | | |
|---|---|---|---|---|---|---|
| $(c,f,h):37$ | $R_T^{z'z}$ | $R_T^{x'x}$ | ${}^cR_{LT'}^{0x}$ | ${}^cR_{LT'}^{0z}$ | ${}^cR_{LT}^{z'x}$ | ${}^cR_{LT}^{x'x}$ |
| | $\mathcal{O}_{2+}^c$ | $\mathcal{O}_{2-}^c$ | $\mathcal{O}_{1-}^f$ | $\mathcal{O}_{2+}^f$ | $\mathcal{O}_{1-}^h$ | $\mathcal{O}_{2+}^h$ |
| $(c,f,h):38$ | $R_T^{z'z}$ | $R_T^{x'x}$ | ${}^cR_{LT'}^{0x}$ | ${}^cR_{LT'}^{0z}$ | ${}^cR_{LT}^{z'x}$ | ${}^sR_{LT'}^{z'x}$ |
| | $\mathcal{O}_{2+}^c$ | $\mathcal{O}_{2-}^c$ | $\mathcal{O}_{1-}^f$ | $\mathcal{O}_{2+}^f$ | $\mathcal{O}_{1-}^h$ | $\mathcal{O}_{2-}^h$ |
| $(c,f,h):39$ | $R_T^{z'z}$ | $R_T^{x'x}$ | ${}^cR_{LT'}^{0x}$ | ${}^sR_{LT}^{0x}$ | ${}^sR_{LT'}^{x'x}$ | ${}^sR_{LT'}^{z'x}$ |
| | $\mathcal{O}_{2+}^c$ | $\mathcal{O}_{2-}^c$ | $\mathcal{O}_{1-}^f$ | $\mathcal{O}_{2-}^f$ | $\mathcal{O}_{1+}^h$ | $\mathcal{O}_{2-}^h$ |
| $(c,f,h):40$ | $R_T^{z'z}$ | $R_T^{x'x}$ | ${}^cR_{LT'}^{0x}$ | ${}^sR_{LT}^{0x}$ | ${}^cR_{LT}^{z'x}$ | ${}^cR_{LT}^{x'x}$ |
| | $\mathcal{O}_{2+}^c$ | $\mathcal{O}_{2-}^c$ | $\mathcal{O}_{1-}^f$ | $\mathcal{O}_{2-}^f$ | $\mathcal{O}_{1-}^h$ | $\mathcal{O}_{2+}^h$ |
| $(c,f,h):41$ | $R_T^{x'z}$ | $R_T^{z'z}$ | ${}^sR_{LT}^{0z}$ | ${}^cR_{LT'}^{0x}$ | ${}^sR_{LT'}^{x'x}$ | ${}^cR_{LT}^{z'x}$ |
| | $\mathcal{O}_{1+}^c$ | $\mathcal{O}_{2+}^c$ | $\mathcal{O}_{1+}^f$ | $\mathcal{O}_{1-}^f$ | $\mathcal{O}_{1+}^h$ | $\mathcal{O}_{1-}^h$ |
| $(c,f,h):42$ | $R_T^{x'z}$ | $R_T^{z'z}$ | ${}^sR_{LT}^{0z}$ | ${}^cR_{LT'}^{0x}$ | ${}^cR_{LT}^{x'x}$ | ${}^sR_{LT'}^{z'x}$ |
| | $\mathcal{O}_{1+}^c$ | $\mathcal{O}_{2+}^c$ | $\mathcal{O}_{1+}^f$ | $\mathcal{O}_{1-}^f$ | $\mathcal{O}_{2+}^h$ | $\mathcal{O}_{2-}^h$ |
| $(c,f,h):43$ | $R_T^{x'z}$ | $R_T^{z'z}$ | ${}^sR_{LT}^{0z}$ | ${}^cR_{LT'}^{0x}$ | ${}^sR_{LT'}^{x'x}$ | ${}^cR_{LT}^{x'x}$ |
| | $\mathcal{O}_{1+}^c$ | $\mathcal{O}_{2+}^c$ | $\mathcal{O}_{1+}^f$ | $\mathcal{O}_{1-}^f$ | $\mathcal{O}_{1+}^h$ | $\mathcal{O}_{2+}^h$ |
| $(c,f,h):44$ | $R_T^{x'z}$ | $R_T^{z'z}$ | ${}^sR_{LT}^{0z}$ | ${}^cR_{LT'}^{0x}$ | ${}^sR_{LT'}^{x'x}$ | ${}^sR_{LT'}^{z'x}$ |
| | $\mathcal{O}_{1+}^c$ | $\mathcal{O}_{2+}^c$ | $\mathcal{O}_{1+}^f$ | $\mathcal{O}_{1-}^f$ | $\mathcal{O}_{1+}^h$ | $\mathcal{O}_{2-}^h$ |
| $(c,f,h):45$ | $R_T^{x'z}$ | $R_T^{z'z}$ | ${}^sR_{LT}^{0z}$ | ${}^cR_{LT'}^{0x}$ | ${}^cR_{LT}^{z'x}$ | ${}^cR_{LT}^{x'x}$ |
| | $\mathcal{O}_{1+}^c$ | $\mathcal{O}_{2+}^c$ | $\mathcal{O}_{1+}^f$ | $\mathcal{O}_{1-}^f$ | $\mathcal{O}_{1-}^h$ | $\mathcal{O}_{2+}^h$ |
| $(c,f,h):46$ | $R_T^{x'z}$ | $R_T^{z'z}$ | ${}^sR_{LT}^{0z}$ | ${}^cR_{LT'}^{0x}$ | ${}^cR_{LT}^{z'x}$ | ${}^sR_{LT'}^{z'x}$ |
| | $\mathcal{O}_{1+}^c$ | $\mathcal{O}_{2+}^c$ | $\mathcal{O}_{1+}^f$ | $\mathcal{O}_{1-}^f$ | $\mathcal{O}_{1-}^h$ | $\mathcal{O}_{2-}^h$ |
| $(c,f,h):47$ | $R_T^{x'z}$ | $R_T^{z'z}$ | ${}^cR_{LT'}^{0z}$ | ${}^sR_{LT}^{0x}$ | ${}^sR_{LT'}^{x'x}$ | ${}^cR_{LT}^{z'x}$ |
| | $\mathcal{O}_{1+}^c$ | $\mathcal{O}_{2+}^c$ | $\mathcal{O}_{2+}^f$ | $\mathcal{O}_{2-}^f$ | $\mathcal{O}_{1+}^h$ | $\mathcal{O}_{1-}^h$ |
| $(c,f,h):48$ | $R_T^{x'z}$ | $R_T^{z'z}$ | ${}^cR_{LT'}^{0z}$ | ${}^sR_{LT}^{0x}$ | ${}^cR_{LT}^{x'x}$ | ${}^sR_{LT'}^{z'x}$ |
| | $\mathcal{O}_{1+}^c$ | $\mathcal{O}_{2+}^c$ | $\mathcal{O}_{2+}^f$ | $\mathcal{O}_{2-}^f$ | $\mathcal{O}_{2+}^h$ | $\mathcal{O}_{2-}^h$ |
| $(c,f,h):49$ | $R_T^{x'z}$ | $R_T^{z'z}$ | ${}^cR_{LT'}^{0z}$ | ${}^sR_{LT}^{0x}$ | ${}^sR_{LT'}^{x'x}$ | ${}^cR_{LT}^{x'x}$ |
| | $\mathcal{O}_{1+}^c$ | $\mathcal{O}_{2+}^c$ | $\mathcal{O}_{2+}^f$ | $\mathcal{O}_{2-}^f$ | $\mathcal{O}_{1+}^h$ | $\mathcal{O}_{2+}^h$ |
| $(c,f,h):50$ | $R_T^{x'z}$ | $R_T^{z'z}$ | ${}^cR_{LT'}^{0z}$ | ${}^sR_{LT}^{0x}$ | ${}^sR_{LT'}^{x'x}$ | ${}^sR_{LT'}^{z'x}$ |
| | $\mathcal{O}_{1+}^c$ | $\mathcal{O}_{2+}^c$ | $\mathcal{O}_{2+}^f$ | $\mathcal{O}_{2-}^f$ | $\mathcal{O}_{1+}^h$ | $\mathcal{O}_{2-}^h$ |
| $(c,f,h):51$ | $R_T^{x'z}$ | $R_T^{z'z}$ | ${}^cR_{LT'}^{0z}$ | ${}^sR_{LT}^{0x}$ | ${}^cR_{LT}^{z'x}$ | ${}^cR_{LT}^{x'x}$ |
| | $\mathcal{O}_{1+}^c$ | $\mathcal{O}_{2+}^c$ | $\mathcal{O}_{2+}^f$ | $\mathcal{O}_{2-}^f$ | $\mathcal{O}_{1-}^h$ | $\mathcal{O}_{2+}^h$ |
| $(c,f,h):52$ | $R_T^{x'z}$ | $R_T^{z'z}$ | ${}^cR_{LT'}^{0z}$ | ${}^sR_{LT}^{0x}$ | ${}^cR_{LT}^{z'x}$ | ${}^sR_{LT'}^{z'x}$ |
| | $\mathcal{O}_{1+}^c$ | $\mathcal{O}_{2+}^c$ | $\mathcal{O}_{2+}^f$ | $\mathcal{O}_{2-}^f$ | $\mathcal{O}_{1-}^h$ | $\mathcal{O}_{2-}^h$ |
| $(c,f,h):53$ | $R_T^{x'z}$ | $R_T^{z'z}$ | ${}^sR_{LT}^{0z}$ | ${}^cR_{LT'}^{0z}$ | ${}^sR_{LT'}^{x'x}$ | ${}^cR_{LT}^{z'x}$ |
| | $\mathcal{O}_{1+}^c$ | $\mathcal{O}_{2+}^c$ | $\mathcal{O}_{1+}^f$ | $\mathcal{O}_{2+}^f$ | $\mathcal{O}_{1+}^h$ | $\mathcal{O}_{1-}^h$ |
| $(c,f,h):54$ | $R_T^{x'z}$ | $R_T^{z'z}$ | ${}^sR_{LT}^{0z}$ | ${}^cR_{LT'}^{0z}$ | ${}^cR_{LT}^{x'x}$ | ${}^sR_{LT'}^{z'x}$ |
| | $\mathcal{O}_{1+}^c$ | $\mathcal{O}_{2+}^c$ | $\mathcal{O}_{1+}^f$ | $\mathcal{O}_{2+}^f$ | $\mathcal{O}_{2+}^h$ | $\mathcal{O}_{2-}^h$ |
| $(c,f,h):55$ | $R_T^{x'z}$ | $R_T^{z'z}$ | ${}^sR_{LT}^{0z}$ | ${}^cR_{LT'}^{0z}$ | ${}^sR_{LT'}^{x'x}$ | ${}^cR_{LT}^{x'x}$ |
| | $\mathcal{O}_{1+}^c$ | $\mathcal{O}_{2+}^c$ | $\mathcal{O}_{1+}^f$ | $\mathcal{O}_{2+}^f$ | $\mathcal{O}_{1+}^h$ | $\mathcal{O}_{2+}^h$ |
| $(c,f,h):56$ | $R_T^{x'z}$ | $R_T^{z'z}$ | ${}^sR_{LT}^{0z}$ | ${}^cR_{LT'}^{0z}$ | ${}^sR_{LT'}^{x'x}$ | ${}^sR_{LT'}^{z'x}$ |
| | $\mathcal{O}_{1+}^c$ | $\mathcal{O}_{2+}^c$ | $\mathcal{O}_{1+}^f$ | $\mathcal{O}_{2+}^f$ | $\mathcal{O}_{1+}^h$ | $\mathcal{O}_{2-}^h$ |
| $(c,f,h):57$ | $R_T^{x'z}$ | $R_T^{z'z}$ | ${}^sR_{LT}^{0z}$ | ${}^cR_{LT'}^{0z}$ | ${}^cR_{LT}^{z'x}$ | ${}^cR_{LT}^{x'x}$ |
| | $\mathcal{O}_{1+}^c$ | $\mathcal{O}_{2+}^c$ | $\mathcal{O}_{1+}^f$ | $\mathcal{O}_{2+}^f$ | $\mathcal{O}_{1-}^h$ | $\mathcal{O}_{2+}^h$ |
| $(c,f,h):58$ | $R_T^{x'z}$ | $R_T^{z'z}$ | ${}^sR_{LT}^{0z}$ | ${}^cR_{LT'}^{0z}$ | ${}^cR_{LT}^{z'x}$ | ${}^sR_{LT'}^{z'x}$ |
| | $\mathcal{O}_{1+}^c$ | $\mathcal{O}_{2+}^c$ | $\mathcal{O}_{1+}^f$ | $\mathcal{O}_{2+}^f$ | $\mathcal{O}_{1-}^h$ | $\mathcal{O}_{2-}^h$ |
| $(c,f,h):59$ | $R_T^{x'z}$ | $R_T^{z'z}$ | ${}^sR_{LT}^{0z}$ | ${}^sR_{LT}^{0x}$ | ${}^sR_{LT'}^{x'x}$ | ${}^cR_{LT}^{z'x}$ |
| | $\mathcal{O}_{1+}^c$ | $\mathcal{O}_{2+}^c$ | $\mathcal{O}_{1+}^f$ | $\mathcal{O}_{2-}^f$ | $\mathcal{O}_{1+}^h$ | $\mathcal{O}_{1-}^h$ |
| $(c,f,h):60$ | $R_T^{x'z}$ | $R_T^{z'z}$ | ${}^sR_{LT}^{0z}$ | ${}^sR_{LT}^{0x}$ | ${}^cR_{LT}^{x'x}$ | ${}^sR_{LT'}^{z'x}$ |
| | $\mathcal{O}_{1+}^c$ | $\mathcal{O}_{2+}^c$ | $\mathcal{O}_{1+}^f$ | $\mathcal{O}_{2-}^f$ | $\mathcal{O}_{2+}^h$ | $\mathcal{O}_{2-}^h$ |
| $(c,f,h):61$ | $R_T^{x'z}$ | $R_T^{z'z}$ | ${}^sR_{LT}^{0z}$ | ${}^sR_{LT}^{0x}$ | ${}^sR_{LT'}^{x'x}$ | ${}^cR_{LT}^{x'x}$ |
| | $\mathcal{O}_{1+}^c$ | $\mathcal{O}_{2+}^c$ | $\mathcal{O}_{1+}^f$ | $\mathcal{O}_{2-}^f$ | $\mathcal{O}_{1+}^h$ | $\mathcal{O}_{2+}^h$ |
| $(c,f,h):62$ | $R_T^{x'z}$ | $R_T^{z'z}$ | ${}^sR_{LT}^{0z}$ | ${}^sR_{LT}^{0x}$ | ${}^sR_{LT'}^{x'x}$ | ${}^sR_{LT'}^{z'x}$ |
| | $\mathcal{O}_{1+}^c$ | $\mathcal{O}_{2+}^c$ | $\mathcal{O}_{1+}^f$ | $\mathcal{O}_{2-}^f$ | $\mathcal{O}_{1+}^h$ | $\mathcal{O}_{2-}^h$ |
| $(c,f,h):63$ | $R_T^{x'z}$ | $R_T^{z'z}$ | ${}^sR_{LT}^{0z}$ | ${}^sR_{LT}^{0x}$ | ${}^cR_{LT}^{z'x}$ | ${}^cR_{LT}^{x'x}$ |
| | $\mathcal{O}_{1+}^c$ | $\mathcal{O}_{2+}^c$ | $\mathcal{O}_{1+}^f$ | $\mathcal{O}_{2-}^f$ | $\mathcal{O}_{1-}^h$ | $\mathcal{O}_{2+}^h$ |
| $(c,f,h):64$ | $R_T^{x'z}$ | $R_T^{z'z}$ | ${}^sR_{LT}^{0z}$ | ${}^sR_{LT}^{0x}$ | ${}^cR_{LT}^{z'x}$ | ${}^sR_{LT'}^{z'x}$ |

| | | | | | | |
|---|---|---|---|---|---|---|
| | $\mathcal{O}^c_{1+}$ | $\mathcal{O}^c_{2+}$ | $\mathcal{O}^f_{1+}$ | $\mathcal{O}^f_{2-}$ | $\mathcal{O}^h_{1-}$ | $\mathcal{O}^h_{2-}$ |
| $(c,f,h):65$ | $R_T^{x'z}$ | $R_T^{z'z}$ | ${}^cR_{LT'}^{0x}$ | ${}^cR_{LT'}^{0z}$ | ${}^sR_{LT'}^{x'x}$ | ${}^cR_{LT}^{z'x}$ |
| | $\mathcal{O}^c_{1+}$ | $\mathcal{O}^c_{2+}$ | $\mathcal{O}^f_{1-}$ | $\mathcal{O}^f_{2+}$ | $\mathcal{O}^h_{1+}$ | $\mathcal{O}^h_{1-}$ |
| $(c,f,h):66$ | $R_T^{x'z}$ | $R_T^{z'z}$ | ${}^cR_{LT'}^{0x}$ | ${}^cR_{LT'}^{0z}$ | ${}^cR_{LT}^{x'x}$ | ${}^sR_{LT'}^{z'x}$ |
| | $\mathcal{O}^c_{1+}$ | $\mathcal{O}^c_{2+}$ | $\mathcal{O}^f_{1-}$ | $\mathcal{O}^f_{2+}$ | $\mathcal{O}^h_{2+}$ | $\mathcal{O}^h_{2-}$ |
| $(c,f,h):67$ | $R_T^{x'z}$ | $R_T^{z'z}$ | ${}^cR_{LT'}^{0x}$ | ${}^cR_{LT'}^{0z}$ | ${}^sR_{LT'}^{x'x}$ | ${}^cR_{LT}^{x'x}$ |
| | $\mathcal{O}^c_{1+}$ | $\mathcal{O}^c_{2+}$ | $\mathcal{O}^f_{1-}$ | $\mathcal{O}^f_{2+}$ | $\mathcal{O}^h_{1+}$ | $\mathcal{O}^h_{2+}$ |
| $(c,f,h):68$ | $R_T^{x'z}$ | $R_T^{z'z}$ | ${}^cR_{LT'}^{0x}$ | ${}^cR_{LT'}^{0z}$ | ${}^sR_{LT'}^{x'x}$ | ${}^sR_{LT'}^{z'x}$ |
| | $\mathcal{O}^c_{1+}$ | $\mathcal{O}^c_{2+}$ | $\mathcal{O}^f_{1-}$ | $\mathcal{O}^f_{2+}$ | $\mathcal{O}^h_{1+}$ | $\mathcal{O}^h_{2-}$ |
| $(c,f,h):69$ | $R_T^{x'z}$ | $R_T^{z'z}$ | ${}^cR_{LT'}^{0x}$ | ${}^cR_{LT'}^{0z}$ | ${}^cR_{LT}^{z'x}$ | ${}^cR_{LT}^{x'x}$ |
| | $\mathcal{O}^c_{1+}$ | $\mathcal{O}^c_{2+}$ | $\mathcal{O}^f_{1-}$ | $\mathcal{O}^f_{2+}$ | $\mathcal{O}^h_{1-}$ | $\mathcal{O}^h_{2+}$ |
| $(c,f,h):70$ | $R_T^{x'z}$ | $R_T^{z'z}$ | ${}^cR_{LT'}^{0x}$ | ${}^cR_{LT'}^{0z}$ | ${}^cR_{LT}^{z'x}$ | ${}^sR_{LT'}^{z'x}$ |
| | $\mathcal{O}^c_{1+}$ | $\mathcal{O}^c_{2+}$ | $\mathcal{O}^f_{1-}$ | $\mathcal{O}^f_{2+}$ | $\mathcal{O}^h_{1-}$ | $\mathcal{O}^h_{2-}$ |
| $(c,f,h):71$ | $R_T^{x'z}$ | $R_T^{z'z}$ | ${}^cR_{LT'}^{0x}$ | ${}^sR_{LT}^{0x}$ | ${}^sR_{LT'}^{x'x}$ | ${}^cR_{LT}^{z'x}$ |
| | $\mathcal{O}^c_{1+}$ | $\mathcal{O}^c_{2+}$ | $\mathcal{O}^f_{1-}$ | $\mathcal{O}^f_{2-}$ | $\mathcal{O}^h_{1+}$ | $\mathcal{O}^h_{1-}$ |
| $(c,f,h):72$ | $R_T^{x'z}$ | $R_T^{z'z}$ | ${}^cR_{LT'}^{0x}$ | ${}^sR_{LT}^{0x}$ | ${}^cR_{LT}^{x'x}$ | ${}^sR_{LT'}^{z'x}$ |
| | $\mathcal{O}^c_{1+}$ | $\mathcal{O}^c_{2+}$ | $\mathcal{O}^f_{1-}$ | $\mathcal{O}^f_{2-}$ | $\mathcal{O}^h_{2+}$ | $\mathcal{O}^h_{2-}$ |
| $(c,f,h):73$ | $R_T^{x'z}$ | $R_T^{z'z}$ | ${}^cR_{LT'}^{0x}$ | ${}^sR_{LT}^{0x}$ | ${}^sR_{LT'}^{x'x}$ | ${}^cR_{LT}^{x'x}$ |
| | $\mathcal{O}^c_{1+}$ | $\mathcal{O}^c_{2+}$ | $\mathcal{O}^f_{1-}$ | $\mathcal{O}^f_{2-}$ | $\mathcal{O}^h_{1+}$ | $\mathcal{O}^h_{2+}$ |
| $(c,f,h):74$ | $R_T^{x'z}$ | $R_T^{z'z}$ | ${}^cR_{LT'}^{0x}$ | ${}^sR_{LT}^{0x}$ | ${}^sR_{LT'}^{x'x}$ | ${}^sR_{LT'}^{z'x}$ |
| | $\mathcal{O}^c_{1+}$ | $\mathcal{O}^c_{2+}$ | $\mathcal{O}^f_{1-}$ | $\mathcal{O}^f_{2-}$ | $\mathcal{O}^h_{1+}$ | $\mathcal{O}^h_{2-}$ |
| $(c,f,h):75$ | $R_T^{x'z}$ | $R_T^{z'z}$ | ${}^cR_{LT'}^{0x}$ | ${}^sR_{LT}^{0x}$ | ${}^cR_{LT}^{z'x}$ | ${}^cR_{LT}^{x'x}$ |
| | $\mathcal{O}^c_{1+}$ | $\mathcal{O}^c_{2+}$ | $\mathcal{O}^f_{1-}$ | $\mathcal{O}^f_{2-}$ | $\mathcal{O}^h_{1-}$ | $\mathcal{O}^h_{2+}$ |
| $(c,f,h):76$ | $R_T^{x'z}$ | $R_T^{z'z}$ | ${}^cR_{LT'}^{0x}$ | ${}^sR_{LT}^{0x}$ | ${}^cR_{LT}^{z'x}$ | ${}^sR_{LT'}^{z'x}$ |
| | $\mathcal{O}^c_{1+}$ | $\mathcal{O}^c_{2+}$ | $\mathcal{O}^f_{1-}$ | $\mathcal{O}^f_{2-}$ | $\mathcal{O}^h_{1-}$ | $\mathcal{O}^h_{2-}$ |
| $(c,f,h):77$ | $R_T^{x'z}$ | $R_T^{x'x}$ | ${}^sR_{LT}^{0z}$ | ${}^cR_{LT'}^{0x}$ | ${}^sR_{LT'}^{x'x}$ | ${}^sR_{LT'}^{z'x}$ |
| | $\mathcal{O}^c_{1+}$ | $\mathcal{O}^c_{2-}$ | $\mathcal{O}^f_{1+}$ | $\mathcal{O}^f_{1-}$ | $\mathcal{O}^h_{1+}$ | $\mathcal{O}^h_{2-}$ |
| $(c,f,h):78$ | $R_T^{x'z}$ | $R_T^{x'x}$ | ${}^sR_{LT}^{0z}$ | ${}^cR_{LT'}^{0x}$ | ${}^cR_{LT}^{z'x}$ | ${}^cR_{LT}^{x'x}$ |
| | $\mathcal{O}^c_{1+}$ | $\mathcal{O}^c_{2-}$ | $\mathcal{O}^f_{1+}$ | $\mathcal{O}^f_{1-}$ | $\mathcal{O}^h_{1-}$ | $\mathcal{O}^h_{2+}$ |
| $(c,f,h):79$ | $R_T^{x'z}$ | $R_T^{x'x}$ | ${}^cR_{LT'}^{0z}$ | ${}^sR_{LT}^{0x}$ | ${}^sR_{LT'}^{x'x}$ | ${}^sR_{LT'}^{z'x}$ |
| | $\mathcal{O}^c_{1+}$ | $\mathcal{O}^c_{2-}$ | $\mathcal{O}^f_{2+}$ | $\mathcal{O}^f_{2-}$ | $\mathcal{O}^h_{1+}$ | $\mathcal{O}^h_{2-}$ |
| $(c,f,h):80$ | $R_T^{x'z}$ | $R_T^{x'x}$ | ${}^cR_{LT'}^{0z}$ | ${}^sR_{LT}^{0x}$ | ${}^cR_{LT}^{z'x}$ | ${}^cR_{LT}^{x'x}$ |
| | $\mathcal{O}^c_{1+}$ | $\mathcal{O}^c_{2-}$ | $\mathcal{O}^f_{2+}$ | $\mathcal{O}^f_{2-}$ | $\mathcal{O}^h_{1-}$ | $\mathcal{O}^h_{2+}$ |
| $(c,f,h):81$ | $R_T^{x'z}$ | $R_T^{x'x}$ | ${}^sR_{LT}^{0z}$ | ${}^cR_{LT'}^{0z}$ | ${}^sR_{LT'}^{x'x}$ | ${}^sR_{LT'}^{z'x}$ |
| | $\mathcal{O}^c_{1+}$ | $\mathcal{O}^c_{2-}$ | $\mathcal{O}^f_{1+}$ | $\mathcal{O}^f_{2+}$ | $\mathcal{O}^h_{1+}$ | $\mathcal{O}^h_{2-}$ |
| $(c,f,h):82$ | $R_T^{x'z}$ | $R_T^{x'x}$ | ${}^sR_{LT}^{0z}$ | ${}^cR_{LT'}^{0z}$ | ${}^cR_{LT}^{z'x}$ | ${}^cR_{LT}^{x'x}$ |
| | $\mathcal{O}^c_{1+}$ | $\mathcal{O}^c_{2-}$ | $\mathcal{O}^f_{1+}$ | $\mathcal{O}^f_{2+}$ | $\mathcal{O}^h_{1-}$ | $\mathcal{O}^h_{2+}$ |
| $(c,f,h):83$ | $R_T^{x'z}$ | $R_T^{x'x}$ | ${}^sR_{LT}^{0z}$ | ${}^sR_{LT}^{0x}$ | ${}^sR_{LT'}^{x'x}$ | ${}^cR_{LT}^{z'x}$ |
| | $\mathcal{O}^c_{1+}$ | $\mathcal{O}^c_{2-}$ | $\mathcal{O}^f_{1+}$ | $\mathcal{O}^f_{2-}$ | $\mathcal{O}^h_{1+}$ | $\mathcal{O}^h_{1-}$ |
| $(c,f,h):84$ | $R_T^{x'z}$ | $R_T^{x'x}$ | ${}^sR_{LT}^{0z}$ | ${}^sR_{LT}^{0x}$ | ${}^cR_{LT}^{x'x}$ | ${}^sR_{LT'}^{z'x}$ |
| | $\mathcal{O}^c_{1+}$ | $\mathcal{O}^c_{2-}$ | $\mathcal{O}^f_{1+}$ | $\mathcal{O}^f_{2-}$ | $\mathcal{O}^h_{2+}$ | $\mathcal{O}^h_{2-}$ |
| $(c,f,h):85$ | $R_T^{x'z}$ | $R_T^{x'x}$ | ${}^sR_{LT}^{0z}$ | ${}^sR_{LT}^{0x}$ | ${}^sR_{LT'}^{x'x}$ | ${}^cR_{LT}^{x'x}$ |
| | $\mathcal{O}^c_{1+}$ | $\mathcal{O}^c_{2-}$ | $\mathcal{O}^f_{1+}$ | $\mathcal{O}^f_{2-}$ | $\mathcal{O}^h_{1+}$ | $\mathcal{O}^h_{2+}$ |
| $(c,f,h):86$ | $R_T^{x'z}$ | $R_T^{x'x}$ | ${}^sR_{LT}^{0z}$ | ${}^sR_{LT}^{0x}$ | ${}^sR_{LT'}^{x'x}$ | ${}^sR_{LT'}^{z'x}$ |
| | $\mathcal{O}^c_{1+}$ | $\mathcal{O}^c_{2-}$ | $\mathcal{O}^f_{1+}$ | $\mathcal{O}^f_{2-}$ | $\mathcal{O}^h_{1+}$ | $\mathcal{O}^h_{2-}$ |
| $(c,f,h):87$ | $R_T^{x'z}$ | $R_T^{x'x}$ | ${}^sR_{LT}^{0z}$ | ${}^sR_{LT}^{0x}$ | ${}^cR_{LT}^{z'x}$ | ${}^cR_{LT}^{x'x}$ |
| | $\mathcal{O}^c_{1+}$ | $\mathcal{O}^c_{2-}$ | $\mathcal{O}^f_{1+}$ | $\mathcal{O}^f_{2-}$ | $\mathcal{O}^h_{1-}$ | $\mathcal{O}^h_{2+}$ |
| $(c,f,h):88$ | $R_T^{x'z}$ | $R_T^{x'x}$ | ${}^sR_{LT}^{0z}$ | ${}^sR_{LT}^{0x}$ | ${}^cR_{LT}^{z'x}$ | ${}^sR_{LT'}^{z'x}$ |
| | $\mathcal{O}^c_{1+}$ | $\mathcal{O}^c_{2-}$ | $\mathcal{O}^f_{1+}$ | $\mathcal{O}^f_{2-}$ | $\mathcal{O}^h_{1-}$ | $\mathcal{O}^h_{2-}$ |
| $(c,f,h):89$ | $R_T^{x'z}$ | $R_T^{x'x}$ | ${}^cR_{LT'}^{0x}$ | ${}^cR_{LT'}^{0z}$ | ${}^sR_{LT'}^{x'x}$ | ${}^cR_{LT}^{z'x}$ |
| | $\mathcal{O}^c_{1+}$ | $\mathcal{O}^c_{2-}$ | $\mathcal{O}^f_{1-}$ | $\mathcal{O}^f_{2+}$ | $\mathcal{O}^h_{1+}$ | $\mathcal{O}^h_{1-}$ |
| $(c,f,h):90$ | $R_T^{x'z}$ | $R_T^{x'x}$ | ${}^cR_{LT'}^{0x}$ | ${}^cR_{LT'}^{0z}$ | ${}^cR_{LT}^{x'x}$ | ${}^sR_{LT'}^{z'x}$ |
| | $\mathcal{O}^c_{1+}$ | $\mathcal{O}^c_{2-}$ | $\mathcal{O}^f_{1-}$ | $\mathcal{O}^f_{2+}$ | $\mathcal{O}^h_{2+}$ | $\mathcal{O}^h_{2-}$ |
| $(c,f,h):91$ | $R_T^{x'z}$ | $R_T^{x'x}$ | ${}^cR_{LT'}^{0x}$ | ${}^cR_{LT'}^{0z}$ | ${}^sR_{LT'}^{x'x}$ | ${}^cR_{LT}^{x'x}$ |
| | $\mathcal{O}^c_{1+}$ | $\mathcal{O}^c_{2-}$ | $\mathcal{O}^f_{1-}$ | $\mathcal{O}^f_{2+}$ | $\mathcal{O}^h_{1+}$ | $\mathcal{O}^h_{2+}$ |

| | | | | | | |
|---|---|---|---|---|---|---|
| $(c,f,h):92$ | $R_T^{x'z}$ | $R_T^{x'x}$ | ${}^cR_{LT'}^{0x}$ | ${}^cR_{LT'}^{0z}$ | ${}^sR_{LT'}^{x'x}$ | ${}^sR_{LT'}^{z'x}$ |
| | $\mathcal{O}_{1+}^c$ | $\mathcal{O}_{2-}^c$ | $\mathcal{O}_{1-}^f$ | $\mathcal{O}_{2+}^f$ | $\mathcal{O}_{1+}^h$ | $\mathcal{O}_{2-}^h$ |
| $(c,f,h):93$ | $R_T^{x'z}$ | $R_T^{x'x}$ | ${}^cR_{LT'}^{0x}$ | ${}^cR_{LT'}^{0z}$ | ${}^cR_{LT}^{z'x}$ | ${}^cR_{LT}^{x'x}$ |
| | $\mathcal{O}_{1+}^c$ | $\mathcal{O}_{2-}^c$ | $\mathcal{O}_{1-}^f$ | $\mathcal{O}_{2+}^f$ | $\mathcal{O}_{1-}^h$ | $\mathcal{O}_{2+}^h$ |
| $(c,f,h):94$ | $R_T^{x'z}$ | $R_T^{x'x}$ | ${}^cR_{LT'}^{0x}$ | ${}^cR_{LT'}^{0z}$ | ${}^cR_{LT}^{z'x}$ | ${}^sR_{LT'}^{z'x}$ |
| | $\mathcal{O}_{1+}^c$ | $\mathcal{O}_{2-}^c$ | $\mathcal{O}_{1-}^f$ | $\mathcal{O}_{2+}^f$ | $\mathcal{O}_{1-}^h$ | $\mathcal{O}_{2-}^h$ |
| $(c,f,h):95$ | $R_T^{x'z}$ | $R_T^{x'x}$ | ${}^cR_{LT'}^{0x}$ | ${}^sR_{LT}^{0x}$ | ${}^sR_{LT'}^{x'x}$ | ${}^sR_{LT'}^{z'x}$ |
| | $\mathcal{O}_{1+}^c$ | $\mathcal{O}_{2-}^c$ | $\mathcal{O}_{1-}^f$ | $\mathcal{O}_{2-}^f$ | $\mathcal{O}_{1+}^h$ | $\mathcal{O}_{2-}^h$ |
| $(c,f,h):96$ | $R_T^{x'z}$ | $R_T^{x'x}$ | ${}^cR_{LT'}^{0x}$ | ${}^sR_{LT}^{0x}$ | ${}^cR_{LT}^{z'x}$ | ${}^cR_{LT}^{x'x}$ |
| | $\mathcal{O}_{1+}^c$ | $\mathcal{O}_{2-}^c$ | $\mathcal{O}_{1-}^f$ | $\mathcal{O}_{2-}^f$ | $\mathcal{O}_{1-}^h$ | $\mathcal{O}_{2+}^h$ |
| $(c,f,h):97$ | $R_T^{z'x}$ | $R_T^{z'z}$ | ${}^sR_{LT}^{0z}$ | ${}^cR_{LT'}^{0x}$ | ${}^sR_{LT'}^{x'x}$ | ${}^sR_{LT'}^{z'x}$ |
| | $\mathcal{O}_{1-}^c$ | $\mathcal{O}_{2+}^c$ | $\mathcal{O}_{1+}^f$ | $\mathcal{O}_{1-}^f$ | $\mathcal{O}_{1+}^h$ | $\mathcal{O}_{2-}^h$ |
| $(c,f,h):98$ | $R_T^{z'x}$ | $R_T^{z'z}$ | ${}^sR_{LT}^{0z}$ | ${}^cR_{LT'}^{0x}$ | ${}^cR_{LT}^{z'x}$ | ${}^cR_{LT}^{x'x}$ |
| | $\mathcal{O}_{1-}^c$ | $\mathcal{O}_{2+}^c$ | $\mathcal{O}_{1+}^f$ | $\mathcal{O}_{1-}^f$ | $\mathcal{O}_{1-}^h$ | $\mathcal{O}_{2+}^h$ |
| $(c,f,h):99$ | $R_T^{z'x}$ | $R_T^{z'z}$ | ${}^cR_{LT'}^{0z}$ | ${}^sR_{LT}^{0x}$ | ${}^sR_{LT'}^{x'x}$ | ${}^sR_{LT'}^{z'x}$ |
| | $\mathcal{O}_{1-}^c$ | $\mathcal{O}_{2+}^c$ | $\mathcal{O}_{2+}^f$ | $\mathcal{O}_{2-}^f$ | $\mathcal{O}_{1+}^h$ | $\mathcal{O}_{2-}^h$ |
| $(c,f,h):100$ | $R_T^{z'x}$ | $R_T^{z'z}$ | ${}^cR_{LT'}^{0z}$ | ${}^sR_{LT}^{0x}$ | ${}^cR_{LT}^{z'x}$ | ${}^cR_{LT}^{x'x}$ |
| | $\mathcal{O}_{1-}^c$ | $\mathcal{O}_{2+}^c$ | $\mathcal{O}_{2+}^f$ | $\mathcal{O}_{2-}^f$ | $\mathcal{O}_{1-}^h$ | $\mathcal{O}_{2+}^h$ |
| $(c,f,h):101$ | $R_T^{z'x}$ | $R_T^{z'z}$ | ${}^sR_{LT}^{0z}$ | ${}^cR_{LT'}^{0z}$ | ${}^sR_{LT'}^{x'x}$ | ${}^sR_{LT'}^{z'x}$ |
| | $\mathcal{O}_{1-}^c$ | $\mathcal{O}_{2+}^c$ | $\mathcal{O}_{1+}^f$ | $\mathcal{O}_{2+}^f$ | $\mathcal{O}_{1+}^h$ | $\mathcal{O}_{2-}^h$ |
| $(c,f,h):102$ | $R_T^{z'x}$ | $R_T^{z'z}$ | ${}^sR_{LT}^{0z}$ | ${}^cR_{LT'}^{0z}$ | ${}^cR_{LT}^{z'x}$ | ${}^cR_{LT}^{x'x}$ |
| | $\mathcal{O}_{1-}^c$ | $\mathcal{O}_{2+}^c$ | $\mathcal{O}_{1+}^f$ | $\mathcal{O}_{2+}^f$ | $\mathcal{O}_{1-}^h$ | $\mathcal{O}_{2+}^h$ |
| $(c,f,h):103$ | $R_T^{z'x}$ | $R_T^{z'z}$ | ${}^sR_{LT}^{0z}$ | ${}^sR_{LT}^{0x}$ | ${}^sR_{LT'}^{x'x}$ | ${}^cR_{LT}^{z'x}$ |
| | $\mathcal{O}_{1-}^c$ | $\mathcal{O}_{2+}^c$ | $\mathcal{O}_{1+}^f$ | $\mathcal{O}_{2-}^f$ | $\mathcal{O}_{1+}^h$ | $\mathcal{O}_{1-}^h$ |
| $(c,f,h):104$ | $R_T^{z'x}$ | $R_T^{z'z}$ | ${}^sR_{LT}^{0z}$ | ${}^sR_{LT}^{0x}$ | ${}^cR_{LT}^{x'x}$ | ${}^sR_{LT'}^{z'x}$ |
| | $\mathcal{O}_{1-}^c$ | $\mathcal{O}_{2+}^c$ | $\mathcal{O}_{1+}^f$ | $\mathcal{O}_{2-}^f$ | $\mathcal{O}_{2+}^h$ | $\mathcal{O}_{2-}^h$ |
| $(c,f,h):105$ | $R_T^{z'x}$ | $R_T^{z'z}$ | ${}^sR_{LT}^{0z}$ | ${}^sR_{LT}^{0x}$ | ${}^sR_{LT'}^{x'x}$ | ${}^cR_{LT}^{x'x}$ |
| | $\mathcal{O}_{1-}^c$ | $\mathcal{O}_{2+}^c$ | $\mathcal{O}_{1+}^f$ | $\mathcal{O}_{2-}^f$ | $\mathcal{O}_{1+}^h$ | $\mathcal{O}_{2+}^h$ |
| $(c,f,h):106$ | $R_T^{z'x}$ | $R_T^{z'z}$ | ${}^sR_{LT}^{0z}$ | ${}^sR_{LT}^{0x}$ | ${}^sR_{LT'}^{x'x}$ | ${}^sR_{LT'}^{z'x}$ |
| | $\mathcal{O}_{1-}^c$ | $\mathcal{O}_{2+}^c$ | $\mathcal{O}_{1+}^f$ | $\mathcal{O}_{2-}^f$ | $\mathcal{O}_{1+}^h$ | $\mathcal{O}_{2-}^h$ |
| $(c,f,h):107$ | $R_T^{z'x}$ | $R_T^{z'z}$ | ${}^sR_{LT}^{0z}$ | ${}^sR_{LT}^{0x}$ | ${}^cR_{LT}^{z'x}$ | ${}^cR_{LT}^{x'x}$ |
| | $\mathcal{O}_{1-}^c$ | $\mathcal{O}_{2+}^c$ | $\mathcal{O}_{1+}^f$ | $\mathcal{O}_{2-}^f$ | $\mathcal{O}_{1-}^h$ | $\mathcal{O}_{2+}^h$ |
| $(c,f,h):108$ | $R_T^{z'x}$ | $R_T^{z'z}$ | ${}^sR_{LT}^{0z}$ | ${}^sR_{LT}^{0x}$ | ${}^cR_{LT}^{z'x}$ | ${}^sR_{LT'}^{z'x}$ |
| | $\mathcal{O}_{1-}^c$ | $\mathcal{O}_{2+}^c$ | $\mathcal{O}_{1+}^f$ | $\mathcal{O}_{2-}^f$ | $\mathcal{O}_{1-}^h$ | $\mathcal{O}_{2-}^h$ |
| $(c,f,h):109$ | $R_T^{z'x}$ | $R_T^{z'z}$ | ${}^cR_{LT'}^{0x}$ | ${}^cR_{LT'}^{0z}$ | ${}^sR_{LT'}^{x'x}$ | ${}^cR_{LT}^{z'x}$ |
| | $\mathcal{O}_{1-}^c$ | $\mathcal{O}_{2+}^c$ | $\mathcal{O}_{1-}^f$ | $\mathcal{O}_{2+}^f$ | $\mathcal{O}_{1+}^h$ | $\mathcal{O}_{1-}^h$ |
| $(c,f,h):110$ | $R_T^{z'x}$ | $R_T^{z'z}$ | ${}^cR_{LT'}^{0x}$ | ${}^cR_{LT'}^{0z}$ | ${}^cR_{LT}^{x'x}$ | ${}^sR_{LT'}^{z'x}$ |
| | $\mathcal{O}_{1-}^c$ | $\mathcal{O}_{2+}^c$ | $\mathcal{O}_{1-}^f$ | $\mathcal{O}_{2+}^f$ | $\mathcal{O}_{2+}^h$ | $\mathcal{O}_{2-}^h$ |
| $(c,f,h):111$ | $R_T^{z'x}$ | $R_T^{z'z}$ | ${}^cR_{LT'}^{0x}$ | ${}^cR_{LT'}^{0z}$ | ${}^sR_{LT'}^{x'x}$ | ${}^cR_{LT}^{x'x}$ |
| | $\mathcal{O}_{1-}^c$ | $\mathcal{O}_{2+}^c$ | $\mathcal{O}_{1-}^f$ | $\mathcal{O}_{2+}^f$ | $\mathcal{O}_{1+}^h$ | $\mathcal{O}_{2+}^h$ |
| $(c,f,h):112$ | $R_T^{z'x}$ | $R_T^{z'z}$ | ${}^cR_{LT'}^{0x}$ | ${}^cR_{LT'}^{0z}$ | ${}^sR_{LT'}^{x'x}$ | ${}^sR_{LT'}^{z'x}$ |
| | $\mathcal{O}_{1-}^c$ | $\mathcal{O}_{2+}^c$ | $\mathcal{O}_{1-}^f$ | $\mathcal{O}_{2+}^f$ | $\mathcal{O}_{1+}^h$ | $\mathcal{O}_{2-}^h$ |
| $(c,f,h):113$ | $R_T^{z'x}$ | $R_T^{z'z}$ | ${}^cR_{LT'}^{0x}$ | ${}^cR_{LT'}^{0z}$ | ${}^cR_{LT}^{z'x}$ | ${}^cR_{LT}^{x'x}$ |
| | $\mathcal{O}_{1-}^c$ | $\mathcal{O}_{2+}^c$ | $\mathcal{O}_{1-}^f$ | $\mathcal{O}_{2+}^f$ | $\mathcal{O}_{1-}^h$ | $\mathcal{O}_{2+}^h$ |
| $(c,f,h):114$ | $R_T^{z'x}$ | $R_T^{z'z}$ | ${}^cR_{LT'}^{0x}$ | ${}^cR_{LT'}^{0z}$ | ${}^cR_{LT}^{z'x}$ | ${}^sR_{LT'}^{z'x}$ |
| | $\mathcal{O}_{1-}^c$ | $\mathcal{O}_{2+}^c$ | $\mathcal{O}_{1-}^f$ | $\mathcal{O}_{2+}^f$ | $\mathcal{O}_{1-}^h$ | $\mathcal{O}_{2-}^h$ |
| $(c,f,h):115$ | $R_T^{z'x}$ | $R_T^{z'z}$ | ${}^cR_{LT'}^{0x}$ | ${}^sR_{LT}^{0x}$ | ${}^sR_{LT'}^{x'x}$ | ${}^sR_{LT'}^{z'x}$ |
| | $\mathcal{O}_{1-}^c$ | $\mathcal{O}_{2+}^c$ | $\mathcal{O}_{1-}^f$ | $\mathcal{O}_{2-}^f$ | $\mathcal{O}_{1+}^h$ | $\mathcal{O}_{2-}^h$ |
| $(c,f,h):116$ | $R_T^{z'x}$ | $R_T^{z'z}$ | ${}^cR_{LT'}^{0x}$ | ${}^sR_{LT}^{0x}$ | ${}^cR_{LT}^{z'x}$ | ${}^cR_{LT}^{x'x}$ |
| | $\mathcal{O}_{1-}^c$ | $\mathcal{O}_{2+}^c$ | $\mathcal{O}_{1-}^f$ | $\mathcal{O}_{2-}^f$ | $\mathcal{O}_{1-}^h$ | $\mathcal{O}_{2+}^h$ |
| $(c,f,h):117$ | $R_T^{z'x}$ | $R_T^{x'x}$ | ${}^sR_{LT}^{0z}$ | ${}^cR_{LT'}^{0x}$ | ${}^sR_{LT'}^{x'x}$ | ${}^cR_{LT}^{z'x}$ |
| | $\mathcal{O}_{1-}^c$ | $\mathcal{O}_{2-}^c$ | $\mathcal{O}_{1+}^f$ | $\mathcal{O}_{1-}^f$ | $\mathcal{O}_{1+}^h$ | $\mathcal{O}_{1-}^h$ |
| $(c,f,h):118$ | $R_T^{z'x}$ | $R_T^{x'x}$ | ${}^sR_{LT}^{0z}$ | ${}^cR_{LT'}^{0x}$ | ${}^cR_{LT}^{x'x}$ | ${}^sR_{LT'}^{z'x}$ |
| | $\mathcal{O}_{1-}^c$ | $\mathcal{O}_{2-}^c$ | $\mathcal{O}_{1+}^f$ | $\mathcal{O}_{1-}^f$ | $\mathcal{O}_{2+}^h$ | $\mathcal{O}_{2-}^h$ |
| $(c,f,h):119$ | $R_T^{z'x}$ | $R_T^{x'x}$ | ${}^sR_{LT}^{0z}$ | ${}^cR_{LT'}^{0x}$ | ${}^sR_{LT'}^{x'x}$ | ${}^cR_{LT}^{x'x}$ |

| | | | | | | |
|---|---|---|---|---|---|---|
| | $\mathcal{O}^c_{1-}$ | $\mathcal{O}^c_{2-}$ | $\mathcal{O}^f_{1+}$ | $\mathcal{O}^f_{1-}$ | $\mathcal{O}^h_{1+}$ | $\mathcal{O}^h_{2+}$ |
| $(c,f,h):120$ | $R_T^{z'x}$ | $R_T^{x'x}$ | ${}^sR^{0z}_{LT}$ | ${}^cR^{0x}_{LT'}$ | ${}^sR^{x'x}_{LT'}$ | ${}^sR^{z'x}_{LT'}$ |
| | $\mathcal{O}^c_{1-}$ | $\mathcal{O}^c_{2-}$ | $\mathcal{O}^f_{1+}$ | $\mathcal{O}^f_{1-}$ | $\mathcal{O}^h_{1+}$ | $\mathcal{O}^h_{2-}$ |
| $(c,f,h):121$ | $R_T^{z'x}$ | $R_T^{x'x}$ | ${}^sR^{0z}_{LT}$ | ${}^cR^{0x}_{LT'}$ | ${}^cR^{z'x}_{LT}$ | ${}^cR^{x'x}_{LT}$ |
| | $\mathcal{O}^c_{1-}$ | $\mathcal{O}^c_{2-}$ | $\mathcal{O}^f_{1+}$ | $\mathcal{O}^f_{1-}$ | $\mathcal{O}^h_{1-}$ | $\mathcal{O}^h_{2+}$ |
| $(c,f,h):122$ | $R_T^{z'x}$ | $R_T^{x'x}$ | ${}^sR^{0z}_{LT}$ | ${}^cR^{0x}_{LT'}$ | ${}^cR^{z'x}_{LT}$ | ${}^sR^{z'x}_{LT'}$ |
| | $\mathcal{O}^c_{1-}$ | $\mathcal{O}^c_{2-}$ | $\mathcal{O}^f_{1+}$ | $\mathcal{O}^f_{1-}$ | $\mathcal{O}^h_{1-}$ | $\mathcal{O}^h_{2-}$ |
| $(c,f,h):123$ | $R_T^{z'x}$ | $R_T^{x'x}$ | ${}^cR^{0z}_{LT'}$ | ${}^sR^{0x}_{LT}$ | ${}^sR^{x'x}_{LT'}$ | ${}^cR^{z'x}_{LT}$ |
| | $\mathcal{O}^c_{1-}$ | $\mathcal{O}^c_{2-}$ | $\mathcal{O}^f_{2+}$ | $\mathcal{O}^f_{2-}$ | $\mathcal{O}^h_{1+}$ | $\mathcal{O}^h_{1-}$ |
| $(c,f,h):124$ | $R_T^{z'x}$ | $R_T^{x'x}$ | ${}^cR^{0z}_{LT'}$ | ${}^sR^{0x}_{LT}$ | ${}^cR^{x'x}_{LT}$ | ${}^sR^{z'x}_{LT'}$ |
| | $\mathcal{O}^c_{1-}$ | $\mathcal{O}^c_{2-}$ | $\mathcal{O}^f_{2+}$ | $\mathcal{O}^f_{2-}$ | $\mathcal{O}^h_{2+}$ | $\mathcal{O}^h_{2-}$ |
| $(c,f,h):125$ | $R_T^{z'x}$ | $R_T^{x'x}$ | ${}^cR^{0z}_{LT'}$ | ${}^sR^{0x}_{LT}$ | ${}^sR^{x'x}_{LT'}$ | ${}^cR^{x'x}_{LT}$ |
| | $\mathcal{O}^c_{1-}$ | $\mathcal{O}^c_{2-}$ | $\mathcal{O}^f_{2+}$ | $\mathcal{O}^f_{2-}$ | $\mathcal{O}^h_{1+}$ | $\mathcal{O}^h_{2+}$ |
| $(c,f,h):126$ | $R_T^{z'x}$ | $R_T^{x'x}$ | ${}^cR^{0z}_{LT'}$ | ${}^sR^{0x}_{LT}$ | ${}^sR^{x'x}_{LT'}$ | ${}^sR^{z'x}_{LT'}$ |
| | $\mathcal{O}^c_{1-}$ | $\mathcal{O}^c_{2-}$ | $\mathcal{O}^f_{2+}$ | $\mathcal{O}^f_{2-}$ | $\mathcal{O}^h_{1+}$ | $\mathcal{O}^h_{2-}$ |
| $(c,f,h):127$ | $R_T^{z'x}$ | $R_T^{x'x}$ | ${}^cR^{0z}_{LT'}$ | ${}^sR^{0x}_{LT}$ | ${}^cR^{z'x}_{LT}$ | ${}^cR^{x'x}_{LT}$ |
| | $\mathcal{O}^c_{1-}$ | $\mathcal{O}^c_{2-}$ | $\mathcal{O}^f_{2+}$ | $\mathcal{O}^f_{2-}$ | $\mathcal{O}^h_{1-}$ | $\mathcal{O}^h_{2+}$ |
| $(c,f,h):128$ | $R_T^{z'x}$ | $R_T^{x'x}$ | ${}^cR^{0z}_{LT'}$ | ${}^sR^{0x}_{LT}$ | ${}^cR^{z'x}_{LT}$ | ${}^sR^{z'x}_{LT'}$ |
| | $\mathcal{O}^c_{1-}$ | $\mathcal{O}^c_{2-}$ | $\mathcal{O}^f_{2+}$ | $\mathcal{O}^f_{2-}$ | $\mathcal{O}^h_{1-}$ | $\mathcal{O}^h_{2-}$ |
| $(c,f,h):129$ | $R_T^{z'x}$ | $R_T^{x'x}$ | ${}^sR^{0z}_{LT}$ | ${}^cR^{0z}_{LT'}$ | ${}^sR^{x'x}_{LT'}$ | ${}^cR^{z'x}_{LT}$ |
| | $\mathcal{O}^c_{1-}$ | $\mathcal{O}^c_{2-}$ | $\mathcal{O}^f_{1+}$ | $\mathcal{O}^f_{2+}$ | $\mathcal{O}^h_{1+}$ | $\mathcal{O}^h_{1-}$ |
| $(c,f,h):130$ | $R_T^{z'x}$ | $R_T^{x'x}$ | ${}^sR^{0z}_{LT}$ | ${}^cR^{0z}_{LT'}$ | ${}^cR^{x'x}_{LT}$ | ${}^sR^{z'x}_{LT'}$ |
| | $\mathcal{O}^c_{1-}$ | $\mathcal{O}^c_{2-}$ | $\mathcal{O}^f_{1+}$ | $\mathcal{O}^f_{2+}$ | $\mathcal{O}^h_{2+}$ | $\mathcal{O}^h_{2-}$ |
| $(c,f,h):131$ | $R_T^{z'x}$ | $R_T^{x'x}$ | ${}^sR^{0z}_{LT}$ | ${}^cR^{0z}_{LT'}$ | ${}^sR^{x'x}_{LT'}$ | ${}^cR^{x'x}_{LT}$ |
| | $\mathcal{O}^c_{1-}$ | $\mathcal{O}^c_{2-}$ | $\mathcal{O}^f_{1+}$ | $\mathcal{O}^f_{2+}$ | $\mathcal{O}^h_{1+}$ | $\mathcal{O}^h_{2+}$ |
| $(c,f,h):132$ | $R_T^{z'x}$ | $R_T^{x'x}$ | ${}^sR^{0z}_{LT}$ | ${}^cR^{0z}_{LT'}$ | ${}^sR^{x'x}_{LT'}$ | ${}^sR^{z'x}_{LT'}$ |
| | $\mathcal{O}^c_{1-}$ | $\mathcal{O}^c_{2-}$ | $\mathcal{O}^f_{1+}$ | $\mathcal{O}^f_{2+}$ | $\mathcal{O}^h_{1+}$ | $\mathcal{O}^h_{2-}$ |
| $(c,f,h):133$ | $R_T^{z'x}$ | $R_T^{x'x}$ | ${}^sR^{0z}_{LT}$ | ${}^cR^{0z}_{LT'}$ | ${}^cR^{z'x}_{LT}$ | ${}^cR^{x'x}_{LT}$ |
| | $\mathcal{O}^c_{1-}$ | $\mathcal{O}^c_{2-}$ | $\mathcal{O}^f_{1+}$ | $\mathcal{O}^f_{2+}$ | $\mathcal{O}^h_{1-}$ | $\mathcal{O}^h_{2+}$ |
| $(c,f,h):134$ | $R_T^{z'x}$ | $R_T^{x'x}$ | ${}^sR^{0z}_{LT}$ | ${}^cR^{0z}_{LT'}$ | ${}^cR^{z'x}_{LT}$ | ${}^sR^{z'x}_{LT'}$ |
| | $\mathcal{O}^c_{1-}$ | $\mathcal{O}^c_{2-}$ | $\mathcal{O}^f_{1+}$ | $\mathcal{O}^f_{2+}$ | $\mathcal{O}^h_{1-}$ | $\mathcal{O}^h_{2-}$ |
| $(c,f,h):135$ | $R_T^{z'x}$ | $R_T^{x'x}$ | ${}^sR^{0z}_{LT}$ | ${}^sR^{0x}_{LT}$ | ${}^sR^{x'x}_{LT'}$ | ${}^cR^{z'x}_{LT}$ |
| | $\mathcal{O}^c_{1-}$ | $\mathcal{O}^c_{2-}$ | $\mathcal{O}^f_{1+}$ | $\mathcal{O}^f_{2-}$ | $\mathcal{O}^h_{1+}$ | $\mathcal{O}^h_{1-}$ |
| $(c,f,h):136$ | $R_T^{z'x}$ | $R_T^{x'x}$ | ${}^sR^{0z}_{LT}$ | ${}^sR^{0x}_{LT}$ | ${}^cR^{x'x}_{LT}$ | ${}^sR^{z'x}_{LT'}$ |
| | $\mathcal{O}^c_{1-}$ | $\mathcal{O}^c_{2-}$ | $\mathcal{O}^f_{1+}$ | $\mathcal{O}^f_{2-}$ | $\mathcal{O}^h_{2+}$ | $\mathcal{O}^h_{2-}$ |
| $(c,f,h):137$ | $R_T^{z'x}$ | $R_T^{x'x}$ | ${}^sR^{0z}_{LT}$ | ${}^sR^{0x}_{LT}$ | ${}^sR^{x'x}_{LT'}$ | ${}^cR^{x'x}_{LT}$ |
| | $\mathcal{O}^c_{1-}$ | $\mathcal{O}^c_{2-}$ | $\mathcal{O}^f_{1+}$ | $\mathcal{O}^f_{2-}$ | $\mathcal{O}^h_{1+}$ | $\mathcal{O}^h_{2+}$ |
| $(c,f,h):138$ | $R_T^{z'x}$ | $R_T^{x'x}$ | ${}^sR^{0z}_{LT}$ | ${}^sR^{0x}_{LT}$ | ${}^sR^{x'x}_{LT'}$ | ${}^sR^{z'x}_{LT'}$ |
| | $\mathcal{O}^c_{1-}$ | $\mathcal{O}^c_{2-}$ | $\mathcal{O}^f_{1+}$ | $\mathcal{O}^f_{2-}$ | $\mathcal{O}^h_{1+}$ | $\mathcal{O}^h_{2-}$ |
| $(c,f,h):139$ | $R_T^{z'x}$ | $R_T^{x'x}$ | ${}^sR^{0z}_{LT}$ | ${}^sR^{0x}_{LT}$ | ${}^cR^{z'x}_{LT}$ | ${}^cR^{x'x}_{LT}$ |
| | $\mathcal{O}^c_{1-}$ | $\mathcal{O}^c_{2-}$ | $\mathcal{O}^f_{1+}$ | $\mathcal{O}^f_{2-}$ | $\mathcal{O}^h_{1-}$ | $\mathcal{O}^h_{2+}$ |
| $(c,f,h):140$ | $R_T^{z'x}$ | $R_T^{x'x}$ | ${}^sR^{0z}_{LT}$ | ${}^sR^{0x}_{LT}$ | ${}^cR^{z'x}_{LT}$ | ${}^sR^{z'x}_{LT'}$ |
| | $\mathcal{O}^c_{1-}$ | $\mathcal{O}^c_{2-}$ | $\mathcal{O}^f_{1+}$ | $\mathcal{O}^f_{2-}$ | $\mathcal{O}^h_{1-}$ | $\mathcal{O}^h_{2-}$ |
| $(c,f,h):141$ | $R_T^{z'x}$ | $R_T^{x'x}$ | ${}^cR^{0x}_{LT'}$ | ${}^cR^{0z}_{LT'}$ | ${}^sR^{x'x}_{LT'}$ | ${}^cR^{z'x}_{LT}$ |
| | $\mathcal{O}^c_{1-}$ | $\mathcal{O}^c_{2-}$ | $\mathcal{O}^f_{1-}$ | $\mathcal{O}^f_{2+}$ | $\mathcal{O}^h_{1+}$ | $\mathcal{O}^h_{1-}$ |
| $(c,f,h):142$ | $R_T^{z'x}$ | $R_T^{x'x}$ | ${}^cR^{0x}_{LT'}$ | ${}^cR^{0z}_{LT'}$ | ${}^cR^{x'x}_{LT}$ | ${}^sR^{z'x}_{LT'}$ |
| | $\mathcal{O}^c_{1-}$ | $\mathcal{O}^c_{2-}$ | $\mathcal{O}^f_{1-}$ | $\mathcal{O}^f_{2+}$ | $\mathcal{O}^h_{2+}$ | $\mathcal{O}^h_{2-}$ |
| $(c,f,h):143$ | $R_T^{z'x}$ | $R_T^{x'x}$ | ${}^cR^{0x}_{LT'}$ | ${}^cR^{0z}_{LT'}$ | ${}^sR^{x'x}_{LT'}$ | ${}^cR^{x'x}_{LT}$ |
| | $\mathcal{O}^c_{1-}$ | $\mathcal{O}^c_{2-}$ | $\mathcal{O}^f_{1-}$ | $\mathcal{O}^f_{2+}$ | $\mathcal{O}^h_{1+}$ | $\mathcal{O}^h_{2+}$ |
| $(c,f,h):144$ | $R_T^{z'x}$ | $R_T^{x'x}$ | ${}^cR^{0x}_{LT'}$ | ${}^cR^{0z}_{LT'}$ | ${}^sR^{x'x}_{LT'}$ | ${}^sR^{z'x}_{LT'}$ |
| | $\mathcal{O}^c_{1-}$ | $\mathcal{O}^c_{2-}$ | $\mathcal{O}^f_{1-}$ | $\mathcal{O}^f_{2+}$ | $\mathcal{O}^h_{1+}$ | $\mathcal{O}^h_{2-}$ |
| $(c,f,h):145$ | $R_T^{z'x}$ | $R_T^{x'x}$ | ${}^cR^{0x}_{LT'}$ | ${}^cR^{0z}_{LT'}$ | ${}^cR^{z'x}_{LT}$ | ${}^cR^{x'x}_{LT}$ |
| | $\mathcal{O}^c_{1-}$ | $\mathcal{O}^c_{2-}$ | $\mathcal{O}^f_{1-}$ | $\mathcal{O}^f_{2+}$ | $\mathcal{O}^h_{1-}$ | $\mathcal{O}^h_{2+}$ |
| $(c,f,h):146$ | $R_T^{z'x}$ | $R_T^{x'x}$ | ${}^cR^{0x}_{LT'}$ | ${}^cR^{0z}_{LT'}$ | ${}^cR^{z'x}_{LT}$ | ${}^sR^{z'x}_{LT'}$ |
| | $\mathcal{O}^c_{1-}$ | $\mathcal{O}^c_{2-}$ | $\mathcal{O}^f_{1-}$ | $\mathcal{O}^f_{2+}$ | $\mathcal{O}^h_{1-}$ | $\mathcal{O}^h_{2-}$ |

| | | | | | | |
|---|---|---|---|---|---|---|
| $(c,f,h):147$ | $R_T^{z'x}$ | $R_T^{x'x}$ | ${}^cR_{LT'}^{0x}$ | ${}^sR_{LT}^{0x}$ | ${}^sR_{LT'}^{x'x}$ | ${}^cR_{LT}^{z'x}$ |
| | $\mathcal{O}_{1-}^c$ | $\mathcal{O}_{2-}^c$ | $\mathcal{O}_{1-}^f$ | $\mathcal{O}_{2-}^f$ | $\mathcal{O}_{1+}^h$ | $\mathcal{O}_{1-}^h$ |
| $(c,f,h):148$ | $R_T^{z'x}$ | $R_T^{x'x}$ | ${}^cR_{LT'}^{0x}$ | ${}^sR_{LT}^{0x}$ | ${}^cR_{LT}^{x'x}$ | ${}^sR_{LT'}^{z'x}$ |
| | $\mathcal{O}_{1-}^c$ | $\mathcal{O}_{2-}^c$ | $\mathcal{O}_{1-}^f$ | $\mathcal{O}_{2-}^f$ | $\mathcal{O}_{2+}^h$ | $\mathcal{O}_{2-}^h$ |
| $(c,f,h):149$ | $R_T^{z'x}$ | $R_T^{x'x}$ | ${}^cR_{LT'}^{0x}$ | ${}^sR_{LT}^{0x}$ | ${}^sR_{LT'}^{x'x}$ | ${}^cR_{LT}^{x'x}$ |
| | $\mathcal{O}_{1-}^c$ | $\mathcal{O}_{2-}^c$ | $\mathcal{O}_{1-}^f$ | $\mathcal{O}_{2-}^f$ | $\mathcal{O}_{1+}^h$ | $\mathcal{O}_{2+}^h$ |
| $(c,f,h):150$ | $R_T^{z'x}$ | $R_T^{x'x}$ | ${}^cR_{LT'}^{0x}$ | ${}^sR_{LT}^{0x}$ | ${}^sR_{LT'}^{x'x}$ | ${}^sR_{LT'}^{z'x}$ |
| | $\mathcal{O}_{1-}^c$ | $\mathcal{O}_{2-}^c$ | $\mathcal{O}_{1-}^f$ | $\mathcal{O}_{2-}^f$ | $\mathcal{O}_{1+}^h$ | $\mathcal{O}_{2-}^h$ |
| $(c,f,h):151$ | $R_T^{z'x}$ | $R_T^{x'x}$ | ${}^cR_{LT'}^{0x}$ | ${}^sR_{LT}^{0x}$ | ${}^cR_{LT}^{z'x}$ | ${}^cR_{LT}^{x'x}$ |
| | $\mathcal{O}_{1-}^c$ | $\mathcal{O}_{2-}^c$ | $\mathcal{O}_{1-}^f$ | $\mathcal{O}_{2-}^f$ | $\mathcal{O}_{1-}^h$ | $\mathcal{O}_{2+}^h$ |
| $(c,f,h):152$ | $R_T^{z'x}$ | $R_T^{x'x}$ | ${}^cR_{LT'}^{0x}$ | ${}^sR_{LT}^{0x}$ | ${}^cR_{LT}^{z'x}$ | ${}^sR_{LT'}^{z'x}$ |
| | $\mathcal{O}_{1-}^c$ | $\mathcal{O}_{2-}^c$ | $\mathcal{O}_{1-}^f$ | $\mathcal{O}_{2-}^f$ | $\mathcal{O}_{1-}^h$ | $\mathcal{O}_{2-}^h$ |

TABLE XI: All the fully complete sets determined from the combination of shape-classes $(c,g,h)$ (i.e. graph-topology 'VIII') in the case of pseudoscalar meson electroproduction are listed here. The observables are written in the systematic symbolic notation $\mathcal{O}_{\nu\pm}^{n}$ by Nakayama [1], as well as in the more commonly used notation in terms of 'response-functions' $R_i^{\beta\alpha}$ (cf. references [4, 5]). The given sets of 6 observables have to be combined with the 6 'diagonal' observables $\left\{R_T^{00}, {}^cR_{TT}^{00}, R_T^{0y}, R_T^{y'0}, R_L^{00}, R_L^{0y}\right\}$ in order to form a complete set of minimal length $2N=12$. All of these sets have been verified to be complete using Mathematica [3].

| Set-Nr. | Observables | | | | | |
|---|---|---|---|---|---|---|
| $(c,g,h):1$ | $R_T^{x'z}$ | $R_T^{z'x}$ | ${}^sR_{LT}^{z'0}$ | ${}^cR_{LT'}^{x'0}$ | ${}^sR_{LT'}^{x'x}$ | ${}^sR_{LT'}^{z'x}$ |
| | $\mathcal{O}_{1+}^c$ | $\mathcal{O}_{1-}^c$ | $\mathcal{O}_{1+}^g$ | $\mathcal{O}_{1-}^g$ | $\mathcal{O}_{1+}^h$ | $\mathcal{O}_{2-}^h$ |
| $(c,g,h):2$ | $R_T^{x'z}$ | $R_T^{z'x}$ | ${}^sR_{LT}^{z'0}$ | ${}^cR_{LT'}^{x'0}$ | ${}^cR_{LT}^{z'x}$ | ${}^cR_{LT}^{x'x}$ |
| | $\mathcal{O}_{1+}^c$ | $\mathcal{O}_{1-}^c$ | $\mathcal{O}_{1+}^g$ | $\mathcal{O}_{1-}^g$ | $\mathcal{O}_{1-}^h$ | $\mathcal{O}_{2+}^h$ |
| $(c,g,h):3$ | $R_T^{x'z}$ | $R_T^{z'x}$ | ${}^cR_{LT'}^{z'0}$ | ${}^sR_{LT}^{x'0}$ | ${}^sR_{LT'}^{x'x}$ | ${}^sR_{LT'}^{z'x}$ |
| | $\mathcal{O}_{1+}^c$ | $\mathcal{O}_{1-}^c$ | $\mathcal{O}_{2+}^g$ | $\mathcal{O}_{2-}^g$ | $\mathcal{O}_{1+}^h$ | $\mathcal{O}_{2-}^h$ |
| $(c,g,h):4$ | $R_T^{x'z}$ | $R_T^{z'x}$ | ${}^cR_{LT'}^{z'0}$ | ${}^sR_{LT}^{x'0}$ | ${}^cR_{LT}^{z'x}$ | ${}^cR_{LT}^{x'x}$ |
| | $\mathcal{O}_{1+}^c$ | $\mathcal{O}_{1-}^c$ | $\mathcal{O}_{2+}^g$ | $\mathcal{O}_{2-}^g$ | $\mathcal{O}_{1-}^h$ | $\mathcal{O}_{2+}^h$ |
| $(c,g,h):5$ | $R_T^{x'z}$ | $R_T^{z'x}$ | ${}^sR_{LT}^{z'0}$ | ${}^cR_{LT'}^{z'0}$ | ${}^sR_{LT'}^{x'x}$ | ${}^sR_{LT'}^{z'x}$ |
| | $\mathcal{O}_{1+}^c$ | $\mathcal{O}_{1-}^c$ | $\mathcal{O}_{1+}^g$ | $\mathcal{O}_{2+}^g$ | $\mathcal{O}_{1+}^h$ | $\mathcal{O}_{2-}^h$ |
| $(c,g,h):6$ | $R_T^{x'z}$ | $R_T^{z'x}$ | ${}^sR_{LT}^{z'0}$ | ${}^cR_{LT'}^{z'0}$ | ${}^cR_{LT}^{z'x}$ | ${}^cR_{LT}^{x'x}$ |
| | $\mathcal{O}_{1+}^c$ | $\mathcal{O}_{1-}^c$ | $\mathcal{O}_{1+}^g$ | $\mathcal{O}_{2+}^g$ | $\mathcal{O}_{1-}^h$ | $\mathcal{O}_{2+}^h$ |
| $(c,g,h):7$ | $R_T^{x'z}$ | $R_T^{z'x}$ | ${}^sR_{LT}^{z'0}$ | ${}^sR_{LT}^{x'0}$ | ${}^sR_{LT'}^{x'x}$ | ${}^cR_{LT}^{z'x}$ |
| | $\mathcal{O}_{1+}^c$ | $\mathcal{O}_{1-}^c$ | $\mathcal{O}_{1+}^g$ | $\mathcal{O}_{2-}^g$ | $\mathcal{O}_{1+}^h$ | $\mathcal{O}_{1-}^h$ |
| $(c,g,h):8$ | $R_T^{x'z}$ | $R_T^{z'x}$ | ${}^sR_{LT}^{z'0}$ | ${}^sR_{LT}^{x'0}$ | ${}^cR_{LT}^{x'x}$ | ${}^sR_{LT'}^{z'x}$ |
| | $\mathcal{O}_{1+}^c$ | $\mathcal{O}_{1-}^c$ | $\mathcal{O}_{1+}^g$ | $\mathcal{O}_{2-}^g$ | $\mathcal{O}_{2+}^h$ | $\mathcal{O}_{2-}^h$ |
| $(c,g,h):9$ | $R_T^{x'z}$ | $R_T^{z'x}$ | ${}^sR_{LT}^{z'0}$ | ${}^sR_{LT}^{x'0}$ | ${}^sR_{LT'}^{x'x}$ | ${}^cR_{LT}^{x'x}$ |
| | $\mathcal{O}_{1+}^c$ | $\mathcal{O}_{1-}^c$ | $\mathcal{O}_{1+}^g$ | $\mathcal{O}_{2-}^g$ | $\mathcal{O}_{1+}^h$ | $\mathcal{O}_{2+}^h$ |
| $(c,g,h):10$ | $R_T^{x'z}$ | $R_T^{z'x}$ | ${}^sR_{LT}^{z'0}$ | ${}^sR_{LT}^{x'0}$ | ${}^sR_{LT'}^{x'x}$ | ${}^sR_{LT'}^{z'x}$ |
| | $\mathcal{O}_{1+}^c$ | $\mathcal{O}_{1-}^c$ | $\mathcal{O}_{1+}^g$ | $\mathcal{O}_{2-}^g$ | $\mathcal{O}_{1+}^h$ | $\mathcal{O}_{2-}^h$ |
| $(c,g,h):11$ | $R_T^{x'z}$ | $R_T^{z'x}$ | ${}^sR_{LT}^{z'0}$ | ${}^sR_{LT}^{x'0}$ | ${}^cR_{LT}^{z'x}$ | ${}^cR_{LT}^{x'x}$ |
| | $\mathcal{O}_{1+}^c$ | $\mathcal{O}_{1-}^c$ | $\mathcal{O}_{1+}^g$ | $\mathcal{O}_{2-}^g$ | $\mathcal{O}_{1-}^h$ | $\mathcal{O}_{2+}^h$ |
| $(c,g,h):12$ | $R_T^{x'z}$ | $R_T^{z'x}$ | ${}^sR_{LT}^{z'0}$ | ${}^sR_{LT}^{x'0}$ | ${}^cR_{LT}^{z'x}$ | ${}^sR_{LT'}^{z'x}$ |
| | $\mathcal{O}_{1+}^c$ | $\mathcal{O}_{1-}^c$ | $\mathcal{O}_{1+}^g$ | $\mathcal{O}_{2-}^g$ | $\mathcal{O}_{1-}^h$ | $\mathcal{O}_{2-}^h$ |
| $(c,g,h):13$ | $R_T^{x'z}$ | $R_T^{z'x}$ | ${}^cR_{LT'}^{x'0}$ | ${}^cR_{LT'}^{z'0}$ | ${}^sR_{LT'}^{x'x}$ | ${}^cR_{LT}^{z'x}$ |
| | $\mathcal{O}_{1+}^c$ | $\mathcal{O}_{1-}^c$ | $\mathcal{O}_{1-}^g$ | $\mathcal{O}_{2+}^g$ | $\mathcal{O}_{1+}^h$ | $\mathcal{O}_{1-}^h$ |
| $(c,g,h):14$ | $R_T^{x'z}$ | $R_T^{z'x}$ | ${}^cR_{LT'}^{x'0}$ | ${}^cR_{LT'}^{z'0}$ | ${}^cR_{LT}^{x'x}$ | ${}^sR_{LT'}^{z'x}$ |
| | $\mathcal{O}_{1+}^c$ | $\mathcal{O}_{1-}^c$ | $\mathcal{O}_{1-}^g$ | $\mathcal{O}_{2+}^g$ | $\mathcal{O}_{2+}^h$ | $\mathcal{O}_{2-}^h$ |
| $(c,g,h):15$ | $R_T^{x'z}$ | $R_T^{z'x}$ | ${}^cR_{LT'}^{x'0}$ | ${}^cR_{LT'}^{z'0}$ | ${}^sR_{LT'}^{x'x}$ | ${}^cR_{LT}^{x'x}$ |
| | $\mathcal{O}_{1+}^c$ | $\mathcal{O}_{1-}^c$ | $\mathcal{O}_{1-}^g$ | $\mathcal{O}_{2+}^g$ | $\mathcal{O}_{1+}^h$ | $\mathcal{O}_{2+}^h$ |

| | | | | | | |
|---|---|---|---|---|---|---|
| $(c,g,h):16$ | $R_T^{x'z}$ | $R_T^{z'x}$ | ${}^cR_{LT'}^{x'0}$ | ${}^cR_{LT'}^{z'0}$ | ${}^sR_{LT'}^{x'x}$ | ${}^sR_{LT'}^{z'x}$ |
| | $\mathcal{O}_{1+}^c$ | $\mathcal{O}_{1-}^c$ | $\mathcal{O}_{1-}^g$ | $\mathcal{O}_{2+}^g$ | $\mathcal{O}_{1+}^h$ | $\mathcal{O}_{2-}^h$ |
| $(c,g,h):17$ | $R_T^{x'z}$ | $R_T^{z'x}$ | ${}^cR_{LT'}^{x'0}$ | ${}^cR_{LT'}^{z'0}$ | ${}^cR_{LT}^{z'x}$ | ${}^cR_{LT}^{x'x}$ |
| | $\mathcal{O}_{1+}^c$ | $\mathcal{O}_{1-}^c$ | $\mathcal{O}_{1-}^g$ | $\mathcal{O}_{2+}^g$ | $\mathcal{O}_{1-}^h$ | $\mathcal{O}_{2+}^h$ |
| $(c,g,h):18$ | $R_T^{x'z}$ | $R_T^{z'x}$ | ${}^cR_{LT'}^{x'0}$ | ${}^cR_{LT'}^{z'0}$ | ${}^cR_{LT}^{z'x}$ | ${}^sR_{LT'}^{z'x}$ |
| | $\mathcal{O}_{1+}^c$ | $\mathcal{O}_{1-}^c$ | $\mathcal{O}_{1-}^g$ | $\mathcal{O}_{2+}^g$ | $\mathcal{O}_{1-}^h$ | $\mathcal{O}_{2-}^h$ |
| $(c,g,h):19$ | $R_T^{x'z}$ | $R_T^{z'x}$ | ${}^cR_{LT'}^{x'0}$ | ${}^sR_{LT}^{x'0}$ | ${}^sR_{LT'}^{x'x}$ | ${}^sR_{LT'}^{z'x}$ |
| | $\mathcal{O}_{1+}^c$ | $\mathcal{O}_{1-}^c$ | $\mathcal{O}_{1-}^g$ | $\mathcal{O}_{2-}^g$ | $\mathcal{O}_{1+}^h$ | $\mathcal{O}_{2-}^h$ |
| $(c,g,h):20$ | $R_T^{x'z}$ | $R_T^{z'x}$ | ${}^cR_{LT'}^{x'0}$ | ${}^sR_{LT}^{x'0}$ | ${}^cR_{LT}^{z'x}$ | ${}^cR_{LT}^{x'x}$ |
| | $\mathcal{O}_{1+}^c$ | $\mathcal{O}_{1-}^c$ | $\mathcal{O}_{1-}^g$ | $\mathcal{O}_{2-}^g$ | $\mathcal{O}_{1-}^h$ | $\mathcal{O}_{2+}^h$ |
| $(c,g,h):21$ | $R_T^{z'z}$ | $R_T^{x'x}$ | ${}^sR_{LT}^{z'0}$ | ${}^cR_{LT'}^{x'0}$ | ${}^sR_{LT'}^{x'x}$ | ${}^sR_{LT'}^{z'x}$ |
| | $\mathcal{O}_{2+}^c$ | $\mathcal{O}_{2-}^c$ | $\mathcal{O}_{1+}^g$ | $\mathcal{O}_{1-}^g$ | $\mathcal{O}_{1+}^h$ | $\mathcal{O}_{2-}^h$ |
| $(c,g,h):22$ | $R_T^{z'z}$ | $R_T^{x'x}$ | ${}^sR_{LT}^{z'0}$ | ${}^cR_{LT'}^{x'0}$ | ${}^cR_{LT}^{z'x}$ | ${}^cR_{LT}^{x'x}$ |
| | $\mathcal{O}_{2+}^c$ | $\mathcal{O}_{2-}^c$ | $\mathcal{O}_{1+}^g$ | $\mathcal{O}_{1-}^g$ | $\mathcal{O}_{1-}^h$ | $\mathcal{O}_{2+}^h$ |
| $(c,g,h):23$ | $R_T^{z'z}$ | $R_T^{x'x}$ | ${}^cR_{LT'}^{z'0}$ | ${}^sR_{LT}^{x'0}$ | ${}^sR_{LT'}^{x'x}$ | ${}^sR_{LT'}^{z'x}$ |
| | $\mathcal{O}_{2+}^c$ | $\mathcal{O}_{2-}^c$ | $\mathcal{O}_{2+}^g$ | $\mathcal{O}_{2-}^g$ | $\mathcal{O}_{1+}^h$ | $\mathcal{O}_{2-}^h$ |
| $(c,g,h):24$ | $R_T^{z'z}$ | $R_T^{x'x}$ | ${}^cR_{LT'}^{z'0}$ | ${}^sR_{LT}^{x'0}$ | ${}^cR_{LT}^{z'x}$ | ${}^cR_{LT}^{x'x}$ |
| | $\mathcal{O}_{2+}^c$ | $\mathcal{O}_{2-}^c$ | $\mathcal{O}_{2+}^g$ | $\mathcal{O}_{2-}^g$ | $\mathcal{O}_{1-}^h$ | $\mathcal{O}_{2+}^h$ |
| $(c,g,h):25$ | $R_T^{z'z}$ | $R_T^{x'x}$ | ${}^sR_{LT}^{z'0}$ | ${}^cR_{LT'}^{z'0}$ | ${}^sR_{LT'}^{x'x}$ | ${}^sR_{LT'}^{z'x}$ |
| | $\mathcal{O}_{2+}^c$ | $\mathcal{O}_{2-}^c$ | $\mathcal{O}_{1+}^g$ | $\mathcal{O}_{2+}^g$ | $\mathcal{O}_{1+}^h$ | $\mathcal{O}_{2-}^h$ |
| $(c,g,h):26$ | $R_T^{z'z}$ | $R_T^{x'x}$ | ${}^sR_{LT}^{z'0}$ | ${}^cR_{LT'}^{z'0}$ | ${}^cR_{LT}^{z'x}$ | ${}^cR_{LT}^{x'x}$ |
| | $\mathcal{O}_{2+}^c$ | $\mathcal{O}_{2-}^c$ | $\mathcal{O}_{1+}^g$ | $\mathcal{O}_{2+}^g$ | $\mathcal{O}_{1-}^h$ | $\mathcal{O}_{2+}^h$ |
| $(c,g,h):27$ | $R_T^{z'z}$ | $R_T^{x'x}$ | ${}^sR_{LT}^{z'0}$ | ${}^sR_{LT}^{x'0}$ | ${}^sR_{LT'}^{x'x}$ | ${}^cR_{LT}^{z'x}$ |
| | $\mathcal{O}_{2+}^c$ | $\mathcal{O}_{2-}^c$ | $\mathcal{O}_{1+}^g$ | $\mathcal{O}_{2-}^g$ | $\mathcal{O}_{1+}^h$ | $\mathcal{O}_{1-}^h$ |
| $(c,g,h):28$ | $R_T^{z'z}$ | $R_T^{x'x}$ | ${}^sR_{LT}^{z'0}$ | ${}^sR_{LT}^{x'0}$ | ${}^cR_{LT}^{x'x}$ | ${}^sR_{LT'}^{z'x}$ |
| | $\mathcal{O}_{2+}^c$ | $\mathcal{O}_{2-}^c$ | $\mathcal{O}_{1+}^g$ | $\mathcal{O}_{2-}^g$ | $\mathcal{O}_{2+}^h$ | $\mathcal{O}_{2-}^h$ |
| $(c,g,h):29$ | $R_T^{z'z}$ | $R_T^{x'x}$ | ${}^sR_{LT}^{z'0}$ | ${}^sR_{LT}^{x'0}$ | ${}^sR_{LT'}^{x'x}$ | ${}^cR_{LT}^{x'x}$ |
| | $\mathcal{O}_{2+}^c$ | $\mathcal{O}_{2-}^c$ | $\mathcal{O}_{1+}^g$ | $\mathcal{O}_{2-}^g$ | $\mathcal{O}_{1+}^h$ | $\mathcal{O}_{2+}^h$ |
| $(c,g,h):30$ | $R_T^{z'z}$ | $R_T^{x'x}$ | ${}^sR_{LT}^{z'0}$ | ${}^sR_{LT}^{x'0}$ | ${}^sR_{LT'}^{x'x}$ | ${}^sR_{LT'}^{z'x}$ |
| | $\mathcal{O}_{2+}^c$ | $\mathcal{O}_{2-}^c$ | $\mathcal{O}_{1+}^g$ | $\mathcal{O}_{2-}^g$ | $\mathcal{O}_{1+}^h$ | $\mathcal{O}_{2-}^h$ |
| $(c,g,h):31$ | $R_T^{z'z}$ | $R_T^{x'x}$ | ${}^sR_{LT}^{z'0}$ | ${}^sR_{LT}^{x'0}$ | ${}^cR_{LT}^{z'x}$ | ${}^cR_{LT}^{x'x}$ |
| | $\mathcal{O}_{2+}^c$ | $\mathcal{O}_{2-}^c$ | $\mathcal{O}_{1+}^g$ | $\mathcal{O}_{2-}^g$ | $\mathcal{O}_{1-}^h$ | $\mathcal{O}_{2+}^h$ |
| $(c,g,h):32$ | $R_T^{z'z}$ | $R_T^{x'x}$ | ${}^sR_{LT}^{z'0}$ | ${}^sR_{LT}^{x'0}$ | ${}^cR_{LT}^{z'x}$ | ${}^sR_{LT'}^{z'x}$ |
| | $\mathcal{O}_{2+}^c$ | $\mathcal{O}_{2-}^c$ | $\mathcal{O}_{1+}^g$ | $\mathcal{O}_{2-}^g$ | $\mathcal{O}_{1-}^h$ | $\mathcal{O}_{2-}^h$ |
| $(c,g,h):33$ | $R_T^{z'z}$ | $R_T^{x'x}$ | ${}^cR_{LT'}^{x'0}$ | ${}^cR_{LT'}^{z'0}$ | ${}^sR_{LT'}^{x'x}$ | ${}^cR_{LT}^{z'x}$ |
| | $\mathcal{O}_{2+}^c$ | $\mathcal{O}_{2-}^c$ | $\mathcal{O}_{1-}^g$ | $\mathcal{O}_{2+}^g$ | $\mathcal{O}_{1+}^h$ | $\mathcal{O}_{1-}^h$ |
| $(c,g,h):34$ | $R_T^{z'z}$ | $R_T^{x'x}$ | ${}^cR_{LT'}^{x'0}$ | ${}^cR_{LT'}^{z'0}$ | ${}^cR_{LT}^{x'x}$ | ${}^sR_{LT'}^{z'x}$ |
| | $\mathcal{O}_{2+}^c$ | $\mathcal{O}_{2-}^c$ | $\mathcal{O}_{1-}^g$ | $\mathcal{O}_{2+}^g$ | $\mathcal{O}_{2+}^h$ | $\mathcal{O}_{2-}^h$ |
| $(c,g,h):35$ | $R_T^{z'z}$ | $R_T^{x'x}$ | ${}^cR_{LT'}^{x'0}$ | ${}^cR_{LT'}^{z'0}$ | ${}^sR_{LT'}^{x'x}$ | ${}^cR_{LT}^{x'x}$ |
| | $\mathcal{O}_{2+}^c$ | $\mathcal{O}_{2-}^c$ | $\mathcal{O}_{1-}^g$ | $\mathcal{O}_{2+}^g$ | $\mathcal{O}_{1+}^h$ | $\mathcal{O}_{2+}^h$ |
| $(c,g,h):36$ | $R_T^{z'z}$ | $R_T^{x'x}$ | ${}^cR_{LT'}^{x'0}$ | ${}^cR_{LT'}^{z'0}$ | ${}^sR_{LT'}^{x'x}$ | ${}^sR_{LT'}^{z'x}$ |
| | $\mathcal{O}_{2+}^c$ | $\mathcal{O}_{2-}^c$ | $\mathcal{O}_{1-}^g$ | $\mathcal{O}_{2+}^g$ | $\mathcal{O}_{1+}^h$ | $\mathcal{O}_{2-}^h$ |
| $(c,g,h):37$ | $R_T^{z'z}$ | $R_T^{x'x}$ | ${}^cR_{LT'}^{x'0}$ | ${}^cR_{LT'}^{z'0}$ | ${}^cR_{LT}^{z'x}$ | ${}^cR_{LT}^{x'x}$ |
| | $\mathcal{O}_{2+}^c$ | $\mathcal{O}_{2-}^c$ | $\mathcal{O}_{1-}^g$ | $\mathcal{O}_{2+}^g$ | $\mathcal{O}_{1-}^h$ | $\mathcal{O}_{2+}^h$ |
| $(c,g,h):38$ | $R_T^{z'z}$ | $R_T^{x'x}$ | ${}^cR_{LT'}^{x'0}$ | ${}^cR_{LT'}^{z'0}$ | ${}^cR_{LT}^{z'x}$ | ${}^sR_{LT'}^{z'x}$ |
| | $\mathcal{O}_{2+}^c$ | $\mathcal{O}_{2-}^c$ | $\mathcal{O}_{1-}^g$ | $\mathcal{O}_{2+}^g$ | $\mathcal{O}_{1-}^h$ | $\mathcal{O}_{2-}^h$ |
| $(c,g,h):39$ | $R_T^{z'z}$ | $R_T^{x'x}$ | ${}^cR_{LT'}^{x'0}$ | ${}^sR_{LT}^{x'0}$ | ${}^sR_{LT'}^{x'x}$ | ${}^sR_{LT'}^{z'x}$ |
| | $\mathcal{O}_{2+}^c$ | $\mathcal{O}_{2-}^c$ | $\mathcal{O}_{1-}^g$ | $\mathcal{O}_{2-}^g$ | $\mathcal{O}_{1+}^h$ | $\mathcal{O}_{2-}^h$ |
| $(c,g,h):40$ | $R_T^{z'z}$ | $R_T^{x'x}$ | ${}^cR_{LT'}^{x'0}$ | ${}^sR_{LT}^{x'0}$ | ${}^cR_{LT}^{z'x}$ | ${}^cR_{LT}^{x'x}$ |
| | $\mathcal{O}_{2+}^c$ | $\mathcal{O}_{2-}^c$ | $\mathcal{O}_{1-}^g$ | $\mathcal{O}_{2-}^g$ | $\mathcal{O}_{1-}^h$ | $\mathcal{O}_{2+}^h$ |
| $(c,g,h):41$ | $R_T^{x'z}$ | $R_T^{z'z}$ | ${}^sR_{LT}^{z'0}$ | ${}^cR_{LT'}^{x'0}$ | ${}^sR_{LT'}^{x'x}$ | ${}^sR_{LT'}^{z'x}$ |
| | $\mathcal{O}_{1+}^c$ | $\mathcal{O}_{2+}^c$ | $\mathcal{O}_{1+}^g$ | $\mathcal{O}_{1-}^g$ | $\mathcal{O}_{1+}^h$ | $\mathcal{O}_{2-}^h$ |
| $(c,g,h):42$ | $R_T^{x'z}$ | $R_T^{z'z}$ | ${}^sR_{LT}^{z'0}$ | ${}^cR_{LT'}^{x'0}$ | ${}^cR_{LT}^{z'x}$ | ${}^cR_{LT}^{x'x}$ |
| | $\mathcal{O}_{1+}^c$ | $\mathcal{O}_{2+}^c$ | $\mathcal{O}_{1+}^g$ | $\mathcal{O}_{1-}^g$ | $\mathcal{O}_{1-}^h$ | $\mathcal{O}_{2+}^h$ |
| $(c,g,h):43$ | $R_T^{x'z}$ | $R_T^{z'z}$ | ${}^cR_{LT'}^{z'0}$ | ${}^sR_{LT}^{x'0}$ | ${}^sR_{LT'}^{x'x}$ | ${}^sR_{LT'}^{z'x}$ |
| | $\mathcal{O}_{1+}^c$ | $\mathcal{O}_{2+}^c$ | $\mathcal{O}_{2+}^g$ | $\mathcal{O}_{2-}^g$ | $\mathcal{O}_{1+}^h$ | $\mathcal{O}_{2-}^h$ |

| | | | | | | |
|---|---|---|---|---|---|---|
| $(c,g,h):44$ | $R_T^{x'z}$ | $R_T^{z'z}$ | ${}^cR_{LT'}^{z'0}$ | ${}^sR_{LT}^{x'0}$ | ${}^cR_{LT}^{z'x}$ | ${}^cR_{LT}^{x'x}$ |
| | $\mathcal{O}_{1+}^c$ | $\mathcal{O}_{2+}^c$ | $\mathcal{O}_{2+}^g$ | $\mathcal{O}_{2-}^g$ | $\mathcal{O}_{1-}^h$ | $\mathcal{O}_{2+}^h$ |
| $(c,g,h):45$ | $R_T^{x'z}$ | $R_T^{z'z}$ | ${}^sR_{LT}^{z'0}$ | ${}^cR_{LT'}^{z'0}$ | ${}^sR_{LT'}^{x'x}$ | ${}^sR_{LT'}^{z'x}$ |
| | $\mathcal{O}_{1+}^c$ | $\mathcal{O}_{2+}^c$ | $\mathcal{O}_{1+}^g$ | $\mathcal{O}_{2+}^g$ | $\mathcal{O}_{1+}^h$ | $\mathcal{O}_{2-}^h$ |
| $(c,g,h):46$ | $R_T^{x'z}$ | $R_T^{z'z}$ | ${}^sR_{LT}^{z'0}$ | ${}^cR_{LT'}^{z'0}$ | ${}^cR_{LT}^{z'x}$ | ${}^cR_{LT}^{x'x}$ |
| | $\mathcal{O}_{1+}^c$ | $\mathcal{O}_{2+}^c$ | $\mathcal{O}_{1+}^g$ | $\mathcal{O}_{2+}^g$ | $\mathcal{O}_{1-}^h$ | $\mathcal{O}_{2+}^h$ |
| $(c,g,h):47$ | $R_T^{x'z}$ | $R_T^{z'z}$ | ${}^sR_{LT}^{z'0}$ | ${}^sR_{LT}^{x'0}$ | ${}^sR_{LT'}^{x'x}$ | ${}^cR_{LT}^{z'x}$ |
| | $\mathcal{O}_{1+}^c$ | $\mathcal{O}_{2+}^c$ | $\mathcal{O}_{1+}^g$ | $\mathcal{O}_{2-}^g$ | $\mathcal{O}_{1+}^h$ | $\mathcal{O}_{1-}^h$ |
| $(c,g,h):48$ | $R_T^{x'z}$ | $R_T^{z'z}$ | ${}^sR_{LT}^{z'0}$ | ${}^sR_{LT}^{x'0}$ | ${}^cR_{LT}^{x'x}$ | ${}^sR_{LT'}^{z'x}$ |
| | $\mathcal{O}_{1+}^c$ | $\mathcal{O}_{2+}^c$ | $\mathcal{O}_{1+}^g$ | $\mathcal{O}_{2-}^g$ | $\mathcal{O}_{2+}^h$ | $\mathcal{O}_{2-}^h$ |
| $(c,g,h):49$ | $R_T^{x'z}$ | $R_T^{z'z}$ | ${}^sR_{LT}^{z'0}$ | ${}^sR_{LT}^{x'0}$ | ${}^sR_{LT'}^{x'x}$ | ${}^cR_{LT}^{x'x}$ |
| | $\mathcal{O}_{1+}^c$ | $\mathcal{O}_{2+}^c$ | $\mathcal{O}_{1+}^g$ | $\mathcal{O}_{2-}^g$ | $\mathcal{O}_{1+}^h$ | $\mathcal{O}_{2+}^h$ |
| $(c,g,h):50$ | $R_T^{x'z}$ | $R_T^{z'z}$ | ${}^sR_{LT}^{z'0}$ | ${}^sR_{LT}^{x'0}$ | ${}^sR_{LT'}^{x'x}$ | ${}^sR_{LT'}^{z'x}$ |
| | $\mathcal{O}_{1+}^c$ | $\mathcal{O}_{2+}^c$ | $\mathcal{O}_{1+}^g$ | $\mathcal{O}_{2-}^g$ | $\mathcal{O}_{1+}^h$ | $\mathcal{O}_{2-}^h$ |
| $(c,g,h):51$ | $R_T^{x'z}$ | $R_T^{z'z}$ | ${}^sR_{LT}^{z'0}$ | ${}^sR_{LT}^{x'0}$ | ${}^cR_{LT}^{z'x}$ | ${}^cR_{LT}^{x'x}$ |
| | $\mathcal{O}_{1+}^c$ | $\mathcal{O}_{2+}^c$ | $\mathcal{O}_{1+}^g$ | $\mathcal{O}_{2-}^g$ | $\mathcal{O}_{1-}^h$ | $\mathcal{O}_{2+}^h$ |
| $(c,g,h):52$ | $R_T^{x'z}$ | $R_T^{z'z}$ | ${}^sR_{LT}^{z'0}$ | ${}^sR_{LT}^{x'0}$ | ${}^cR_{LT}^{z'x}$ | ${}^sR_{LT'}^{z'x}$ |
| | $\mathcal{O}_{1+}^c$ | $\mathcal{O}_{2+}^c$ | $\mathcal{O}_{1+}^g$ | $\mathcal{O}_{2-}^g$ | $\mathcal{O}_{1-}^h$ | $\mathcal{O}_{2-}^h$ |
| $(c,g,h):53$ | $R_T^{x'z}$ | $R_T^{z'z}$ | ${}^cR_{LT'}^{x'0}$ | ${}^cR_{LT'}^{z'0}$ | ${}^sR_{LT'}^{x'x}$ | ${}^cR_{LT}^{z'x}$ |
| | $\mathcal{O}_{1+}^c$ | $\mathcal{O}_{2+}^c$ | $\mathcal{O}_{1-}^g$ | $\mathcal{O}_{2+}^g$ | $\mathcal{O}_{1+}^h$ | $\mathcal{O}_{1-}^h$ |
| $(c,g,h):54$ | $R_T^{x'z}$ | $R_T^{z'z}$ | ${}^cR_{LT'}^{x'0}$ | ${}^cR_{LT'}^{z'0}$ | ${}^cR_{LT}^{x'x}$ | ${}^sR_{LT'}^{z'x}$ |
| | $\mathcal{O}_{1+}^c$ | $\mathcal{O}_{2+}^c$ | $\mathcal{O}_{1-}^g$ | $\mathcal{O}_{2+}^g$ | $\mathcal{O}_{2+}^h$ | $\mathcal{O}_{2-}^h$ |
| $(c,g,h):55$ | $R_T^{x'z}$ | $R_T^{z'z}$ | ${}^cR_{LT'}^{x'0}$ | ${}^cR_{LT'}^{z'0}$ | ${}^sR_{LT'}^{x'x}$ | ${}^cR_{LT}^{x'x}$ |
| | $\mathcal{O}_{1+}^c$ | $\mathcal{O}_{2+}^c$ | $\mathcal{O}_{1-}^g$ | $\mathcal{O}_{2+}^g$ | $\mathcal{O}_{1+}^h$ | $\mathcal{O}_{2+}^h$ |
| $(c,g,h):56$ | $R_T^{x'z}$ | $R_T^{z'z}$ | ${}^cR_{LT'}^{x'0}$ | ${}^cR_{LT'}^{z'0}$ | ${}^sR_{LT'}^{x'x}$ | ${}^sR_{LT'}^{z'x}$ |
| | $\mathcal{O}_{1+}^c$ | $\mathcal{O}_{2+}^c$ | $\mathcal{O}_{1-}^g$ | $\mathcal{O}_{2+}^g$ | $\mathcal{O}_{1+}^h$ | $\mathcal{O}_{2-}^h$ |
| $(c,g,h):57$ | $R_T^{x'z}$ | $R_T^{z'z}$ | ${}^cR_{LT'}^{x'0}$ | ${}^cR_{LT'}^{z'0}$ | ${}^cR_{LT}^{z'x}$ | ${}^cR_{LT}^{x'x}$ |
| | $\mathcal{O}_{1+}^c$ | $\mathcal{O}_{2+}^c$ | $\mathcal{O}_{1-}^g$ | $\mathcal{O}_{2+}^g$ | $\mathcal{O}_{1-}^h$ | $\mathcal{O}_{2+}^h$ |
| $(c,g,h):58$ | $R_T^{x'z}$ | $R_T^{z'z}$ | ${}^cR_{LT'}^{x'0}$ | ${}^cR_{LT'}^{z'0}$ | ${}^cR_{LT}^{z'x}$ | ${}^sR_{LT'}^{z'x}$ |
| | $\mathcal{O}_{1+}^c$ | $\mathcal{O}_{2+}^c$ | $\mathcal{O}_{1-}^g$ | $\mathcal{O}_{2+}^g$ | $\mathcal{O}_{1-}^h$ | $\mathcal{O}_{2-}^h$ |
| $(c,g,h):59$ | $R_T^{x'z}$ | $R_T^{z'z}$ | ${}^cR_{LT'}^{x'0}$ | ${}^sR_{LT}^{x'0}$ | ${}^sR_{LT'}^{x'x}$ | ${}^sR_{LT'}^{z'x}$ |
| | $\mathcal{O}_{1+}^c$ | $\mathcal{O}_{2+}^c$ | $\mathcal{O}_{1-}^g$ | $\mathcal{O}_{2-}^g$ | $\mathcal{O}_{1+}^h$ | $\mathcal{O}_{2-}^h$ |
| $(c,g,h):60$ | $R_T^{x'z}$ | $R_T^{z'z}$ | ${}^cR_{LT'}^{x'0}$ | ${}^sR_{LT}^{x'0}$ | ${}^cR_{LT}^{z'x}$ | ${}^cR_{LT}^{x'x}$ |
| | $\mathcal{O}_{1+}^c$ | $\mathcal{O}_{2+}^c$ | $\mathcal{O}_{1-}^g$ | $\mathcal{O}_{2-}^g$ | $\mathcal{O}_{1-}^h$ | $\mathcal{O}_{2+}^h$ |
| $(c,g,h):61$ | $R_T^{x'z}$ | $R_T^{x'x}$ | ${}^sR_{LT}^{z'0}$ | ${}^cR_{LT'}^{x'0}$ | ${}^sR_{LT'}^{x'x}$ | ${}^cR_{LT}^{z'x}$ |
| | $\mathcal{O}_{1+}^c$ | $\mathcal{O}_{2-}^c$ | $\mathcal{O}_{1+}^g$ | $\mathcal{O}_{1-}^g$ | $\mathcal{O}_{1+}^h$ | $\mathcal{O}_{1-}^h$ |
| $(c,g,h):62$ | $R_T^{x'z}$ | $R_T^{x'x}$ | ${}^sR_{LT}^{z'0}$ | ${}^cR_{LT'}^{x'0}$ | ${}^cR_{LT}^{x'x}$ | ${}^sR_{LT'}^{z'x}$ |
| | $\mathcal{O}_{1+}^c$ | $\mathcal{O}_{2-}^c$ | $\mathcal{O}_{1+}^g$ | $\mathcal{O}_{1-}^g$ | $\mathcal{O}_{2+}^h$ | $\mathcal{O}_{2-}^h$ |
| $(c,g,h):63$ | $R_T^{x'z}$ | $R_T^{x'x}$ | ${}^sR_{LT}^{z'0}$ | ${}^cR_{LT'}^{x'0}$ | ${}^sR_{LT'}^{x'x}$ | ${}^cR_{LT}^{x'x}$ |
| | $\mathcal{O}_{1+}^c$ | $\mathcal{O}_{2-}^c$ | $\mathcal{O}_{1+}^g$ | $\mathcal{O}_{1-}^g$ | $\mathcal{O}_{1+}^h$ | $\mathcal{O}_{2+}^h$ |
| $(c,g,h):64$ | $R_T^{x'z}$ | $R_T^{x'x}$ | ${}^sR_{LT}^{z'0}$ | ${}^cR_{LT'}^{x'0}$ | ${}^sR_{LT'}^{x'x}$ | ${}^sR_{LT'}^{z'x}$ |
| | $\mathcal{O}_{1+}^c$ | $\mathcal{O}_{2-}^c$ | $\mathcal{O}_{1+}^g$ | $\mathcal{O}_{1-}^g$ | $\mathcal{O}_{1+}^h$ | $\mathcal{O}_{2-}^h$ |
| $(c,g,h):65$ | $R_T^{x'z}$ | $R_T^{x'x}$ | ${}^sR_{LT}^{z'0}$ | ${}^cR_{LT'}^{x'0}$ | ${}^cR_{LT}^{z'x}$ | ${}^cR_{LT}^{x'x}$ |
| | $\mathcal{O}_{1+}^c$ | $\mathcal{O}_{2-}^c$ | $\mathcal{O}_{1+}^g$ | $\mathcal{O}_{1-}^g$ | $\mathcal{O}_{1-}^h$ | $\mathcal{O}_{2+}^h$ |
| $(c,g,h):66$ | $R_T^{x'z}$ | $R_T^{x'x}$ | ${}^sR_{LT}^{z'0}$ | ${}^cR_{LT'}^{x'0}$ | ${}^cR_{LT}^{z'x}$ | ${}^sR_{LT'}^{z'x}$ |
| | $\mathcal{O}_{1+}^c$ | $\mathcal{O}_{2-}^c$ | $\mathcal{O}_{1+}^g$ | $\mathcal{O}_{1-}^g$ | $\mathcal{O}_{1-}^h$ | $\mathcal{O}_{2-}^h$ |
| $(c,g,h):67$ | $R_T^{x'z}$ | $R_T^{x'x}$ | ${}^cR_{LT'}^{z'0}$ | ${}^sR_{LT}^{x'0}$ | ${}^sR_{LT'}^{x'x}$ | ${}^cR_{LT}^{z'x}$ |
| | $\mathcal{O}_{1+}^c$ | $\mathcal{O}_{2-}^c$ | $\mathcal{O}_{2+}^g$ | $\mathcal{O}_{2-}^g$ | $\mathcal{O}_{1+}^h$ | $\mathcal{O}_{1-}^h$ |
| $(c,g,h):68$ | $R_T^{x'z}$ | $R_T^{x'x}$ | ${}^cR_{LT'}^{z'0}$ | ${}^sR_{LT}^{x'0}$ | ${}^cR_{LT}^{x'x}$ | ${}^sR_{LT'}^{z'x}$ |
| | $\mathcal{O}_{1+}^c$ | $\mathcal{O}_{2-}^c$ | $\mathcal{O}_{2+}^g$ | $\mathcal{O}_{2-}^g$ | $\mathcal{O}_{2+}^h$ | $\mathcal{O}_{2-}^h$ |
| $(c,g,h):69$ | $R_T^{x'z}$ | $R_T^{x'x}$ | ${}^cR_{LT'}^{z'0}$ | ${}^sR_{LT}^{x'0}$ | ${}^sR_{LT'}^{x'x}$ | ${}^cR_{LT}^{x'x}$ |
| | $\mathcal{O}_{1+}^c$ | $\mathcal{O}_{2-}^c$ | $\mathcal{O}_{2+}^g$ | $\mathcal{O}_{2-}^g$ | $\mathcal{O}_{1+}^h$ | $\mathcal{O}_{2+}^h$ |
| $(c,g,h):70$ | $R_T^{x'z}$ | $R_T^{x'x}$ | ${}^cR_{LT'}^{z'0}$ | ${}^sR_{LT}^{x'0}$ | ${}^sR_{LT'}^{x'x}$ | ${}^sR_{LT'}^{z'x}$ |
| | $\mathcal{O}_{1+}^c$ | $\mathcal{O}_{2-}^c$ | $\mathcal{O}_{2+}^g$ | $\mathcal{O}_{2-}^g$ | $\mathcal{O}_{1+}^h$ | $\mathcal{O}_{2-}^h$ |
| $(c,g,h):71$ | $R_T^{x'z}$ | $R_T^{x'x}$ | ${}^cR_{LT'}^{z'0}$ | ${}^sR_{LT}^{x'0}$ | ${}^cR_{LT}^{z'x}$ | ${}^cR_{LT}^{x'x}$ |
| | $\mathcal{O}_{1+}^c$ | $\mathcal{O}_{2-}^c$ | $\mathcal{O}_{2+}^g$ | $\mathcal{O}_{2-}^g$ | $\mathcal{O}_{1-}^h$ | $\mathcal{O}_{2+}^h$ |

| | | | | | | |
|---|---|---|---|---|---|---|
| $(c,g,h):72$ | $R_T^{x'z}$ | $R_T^{x'x}$ | ${}^cR_{LT'}^{z'0}$ | ${}^sR_{LT}^{x'0}$ | ${}^cR_{LT}^{z'x}$ | ${}^sR_{LT'}^{z'x}$ |
| | $\mathcal{O}_{1+}^c$ | $\mathcal{O}_{2-}^c$ | $\mathcal{O}_{2+}^g$ | $\mathcal{O}_{2-}^g$ | $\mathcal{O}_{1-}^h$ | $\mathcal{O}_{2-}^h$ |
| $(c,g,h):73$ | $R_T^{x'z}$ | $R_T^{x'x}$ | ${}^sR_{LT}^{z'0}$ | ${}^cR_{LT'}^{z'0}$ | ${}^sR_{LT'}^{x'x}$ | ${}^cR_{LT}^{z'x}$ |
| | $\mathcal{O}_{1+}^c$ | $\mathcal{O}_{2-}^c$ | $\mathcal{O}_{1+}^g$ | $\mathcal{O}_{2+}^g$ | $\mathcal{O}_{1+}^h$ | $\mathcal{O}_{1-}^h$ |
| $(c,g,h):74$ | $R_T^{x'z}$ | $R_T^{x'x}$ | ${}^sR_{LT}^{z'0}$ | ${}^cR_{LT'}^{z'0}$ | ${}^cR_{LT}^{x'x}$ | ${}^sR_{LT'}^{z'x}$ |
| | $\mathcal{O}_{1+}^c$ | $\mathcal{O}_{2-}^c$ | $\mathcal{O}_{1+}^g$ | $\mathcal{O}_{2+}^g$ | $\mathcal{O}_{2+}^h$ | $\mathcal{O}_{2-}^h$ |
| $(c,g,h):75$ | $R_T^{x'z}$ | $R_T^{x'x}$ | ${}^sR_{LT}^{z'0}$ | ${}^cR_{LT'}^{z'0}$ | ${}^sR_{LT'}^{x'x}$ | ${}^cR_{LT}^{x'x}$ |
| | $\mathcal{O}_{1+}^c$ | $\mathcal{O}_{2-}^c$ | $\mathcal{O}_{1+}^g$ | $\mathcal{O}_{2+}^g$ | $\mathcal{O}_{1+}^h$ | $\mathcal{O}_{2+}^h$ |
| $(c,g,h):76$ | $R_T^{x'z}$ | $R_T^{x'x}$ | ${}^sR_{LT}^{z'0}$ | ${}^cR_{LT'}^{z'0}$ | ${}^sR_{LT'}^{x'x}$ | ${}^sR_{LT'}^{z'x}$ |
| | $\mathcal{O}_{1+}^c$ | $\mathcal{O}_{2-}^c$ | $\mathcal{O}_{1+}^g$ | $\mathcal{O}_{2+}^g$ | $\mathcal{O}_{1+}^h$ | $\mathcal{O}_{2-}^h$ |
| $(c,g,h):77$ | $R_T^{x'z}$ | $R_T^{x'x}$ | ${}^sR_{LT}^{z'0}$ | ${}^cR_{LT'}^{z'0}$ | ${}^cR_{LT}^{z'x}$ | ${}^cR_{LT}^{x'x}$ |
| | $\mathcal{O}_{1+}^c$ | $\mathcal{O}_{2-}^c$ | $\mathcal{O}_{1+}^g$ | $\mathcal{O}_{2+}^g$ | $\mathcal{O}_{1-}^h$ | $\mathcal{O}_{2+}^h$ |
| $(c,g,h):78$ | $R_T^{x'z}$ | $R_T^{x'x}$ | ${}^sR_{LT}^{z'0}$ | ${}^cR_{LT'}^{z'0}$ | ${}^cR_{LT}^{z'x}$ | ${}^sR_{LT'}^{z'x}$ |
| | $\mathcal{O}_{1+}^c$ | $\mathcal{O}_{2-}^c$ | $\mathcal{O}_{1+}^g$ | $\mathcal{O}_{2+}^g$ | $\mathcal{O}_{1-}^h$ | $\mathcal{O}_{2-}^h$ |
| $(c,g,h):79$ | $R_T^{x'z}$ | $R_T^{x'x}$ | ${}^sR_{LT}^{z'0}$ | ${}^sR_{LT}^{x'0}$ | ${}^sR_{LT'}^{x'x}$ | ${}^cR_{LT}^{z'x}$ |
| | $\mathcal{O}_{1+}^c$ | $\mathcal{O}_{2-}^c$ | $\mathcal{O}_{1+}^g$ | $\mathcal{O}_{2-}^g$ | $\mathcal{O}_{1+}^h$ | $\mathcal{O}_{1-}^h$ |
| $(c,g,h):80$ | $R_T^{x'z}$ | $R_T^{x'x}$ | ${}^sR_{LT}^{z'0}$ | ${}^sR_{LT}^{x'0}$ | ${}^cR_{LT}^{x'x}$ | ${}^sR_{LT'}^{z'x}$ |
| | $\mathcal{O}_{1+}^c$ | $\mathcal{O}_{2-}^c$ | $\mathcal{O}_{1+}^g$ | $\mathcal{O}_{2-}^g$ | $\mathcal{O}_{2+}^h$ | $\mathcal{O}_{2-}^h$ |
| $(c,g,h):81$ | $R_T^{x'z}$ | $R_T^{x'x}$ | ${}^sR_{LT}^{z'0}$ | ${}^sR_{LT}^{x'0}$ | ${}^sR_{LT'}^{x'x}$ | ${}^cR_{LT}^{x'x}$ |
| | $\mathcal{O}_{1+}^c$ | $\mathcal{O}_{2-}^c$ | $\mathcal{O}_{1+}^g$ | $\mathcal{O}_{2-}^g$ | $\mathcal{O}_{1+}^h$ | $\mathcal{O}_{2+}^h$ |
| $(c,g,h):82$ | $R_T^{x'z}$ | $R_T^{x'x}$ | ${}^sR_{LT}^{z'0}$ | ${}^sR_{LT}^{x'0}$ | ${}^sR_{LT'}^{x'x}$ | ${}^sR_{LT'}^{z'x}$ |
| | $\mathcal{O}_{1+}^c$ | $\mathcal{O}_{2-}^c$ | $\mathcal{O}_{1+}^g$ | $\mathcal{O}_{2-}^g$ | $\mathcal{O}_{1+}^h$ | $\mathcal{O}_{2-}^h$ |
| $(c,g,h):83$ | $R_T^{x'z}$ | $R_T^{x'x}$ | ${}^sR_{LT}^{z'0}$ | ${}^sR_{LT}^{x'0}$ | ${}^cR_{LT}^{z'x}$ | ${}^cR_{LT}^{x'x}$ |
| | $\mathcal{O}_{1+}^c$ | $\mathcal{O}_{2-}^c$ | $\mathcal{O}_{1+}^g$ | $\mathcal{O}_{2-}^g$ | $\mathcal{O}_{1-}^h$ | $\mathcal{O}_{2+}^h$ |
| $(c,g,h):84$ | $R_T^{x'z}$ | $R_T^{x'x}$ | ${}^sR_{LT}^{z'0}$ | ${}^sR_{LT}^{x'0}$ | ${}^cR_{LT}^{z'x}$ | ${}^sR_{LT'}^{z'x}$ |
| | $\mathcal{O}_{1+}^c$ | $\mathcal{O}_{2-}^c$ | $\mathcal{O}_{1+}^g$ | $\mathcal{O}_{2-}^g$ | $\mathcal{O}_{1-}^h$ | $\mathcal{O}_{2-}^h$ |
| $(c,g,h):85$ | $R_T^{x'z}$ | $R_T^{x'x}$ | ${}^cR_{LT'}^{x'0}$ | ${}^cR_{LT'}^{z'0}$ | ${}^sR_{LT'}^{x'x}$ | ${}^cR_{LT}^{z'x}$ |
| | $\mathcal{O}_{1+}^c$ | $\mathcal{O}_{2-}^c$ | $\mathcal{O}_{1-}^g$ | $\mathcal{O}_{2+}^g$ | $\mathcal{O}_{1+}^h$ | $\mathcal{O}_{1-}^h$ |
| $(c,g,h):86$ | $R_T^{x'z}$ | $R_T^{x'x}$ | ${}^cR_{LT'}^{x'0}$ | ${}^cR_{LT'}^{z'0}$ | ${}^cR_{LT}^{x'x}$ | ${}^sR_{LT'}^{z'x}$ |
| | $\mathcal{O}_{1+}^c$ | $\mathcal{O}_{2-}^c$ | $\mathcal{O}_{1-}^g$ | $\mathcal{O}_{2+}^g$ | $\mathcal{O}_{2+}^h$ | $\mathcal{O}_{2-}^h$ |
| $(c,g,h):87$ | $R_T^{x'z}$ | $R_T^{x'x}$ | ${}^cR_{LT'}^{x'0}$ | ${}^cR_{LT'}^{z'0}$ | ${}^sR_{LT'}^{x'x}$ | ${}^cR_{LT}^{x'x}$ |
| | $\mathcal{O}_{1+}^c$ | $\mathcal{O}_{2-}^c$ | $\mathcal{O}_{1-}^g$ | $\mathcal{O}_{2+}^g$ | $\mathcal{O}_{1+}^h$ | $\mathcal{O}_{2+}^h$ |
| $(c,g,h):88$ | $R_T^{x'z}$ | $R_T^{x'x}$ | ${}^cR_{LT'}^{x'0}$ | ${}^cR_{LT'}^{z'0}$ | ${}^sR_{LT'}^{x'x}$ | ${}^sR_{LT'}^{z'x}$ |
| | $\mathcal{O}_{1+}^c$ | $\mathcal{O}_{2-}^c$ | $\mathcal{O}_{1-}^g$ | $\mathcal{O}_{2+}^g$ | $\mathcal{O}_{1+}^h$ | $\mathcal{O}_{2-}^h$ |
| $(c,g,h):89$ | $R_T^{x'z}$ | $R_T^{x'x}$ | ${}^cR_{LT'}^{x'0}$ | ${}^cR_{LT'}^{z'0}$ | ${}^cR_{LT}^{z'x}$ | ${}^cR_{LT}^{x'x}$ |
| | $\mathcal{O}_{1+}^c$ | $\mathcal{O}_{2-}^c$ | $\mathcal{O}_{1-}^g$ | $\mathcal{O}_{2+}^g$ | $\mathcal{O}_{1-}^h$ | $\mathcal{O}_{2+}^h$ |
| $(c,g,h):90$ | $R_T^{x'z}$ | $R_T^{x'x}$ | ${}^cR_{LT'}^{x'0}$ | ${}^cR_{LT'}^{z'0}$ | ${}^cR_{LT}^{z'x}$ | ${}^sR_{LT'}^{z'x}$ |
| | $\mathcal{O}_{1+}^c$ | $\mathcal{O}_{2-}^c$ | $\mathcal{O}_{1-}^g$ | $\mathcal{O}_{2+}^g$ | $\mathcal{O}_{1-}^h$ | $\mathcal{O}_{2-}^h$ |
| $(c,g,h):91$ | $R_T^{x'z}$ | $R_T^{x'x}$ | ${}^cR_{LT'}^{x'0}$ | ${}^sR_{LT}^{x'0}$ | ${}^sR_{LT'}^{x'x}$ | ${}^cR_{LT}^{z'x}$ |
| | $\mathcal{O}_{1+}^c$ | $\mathcal{O}_{2-}^c$ | $\mathcal{O}_{1-}^g$ | $\mathcal{O}_{2-}^g$ | $\mathcal{O}_{1+}^h$ | $\mathcal{O}_{1-}^h$ |
| $(c,g,h):92$ | $R_T^{x'z}$ | $R_T^{x'x}$ | ${}^cR_{LT'}^{x'0}$ | ${}^sR_{LT}^{x'0}$ | ${}^cR_{LT}^{x'x}$ | ${}^sR_{LT'}^{z'x}$ |
| | $\mathcal{O}_{1+}^c$ | $\mathcal{O}_{2-}^c$ | $\mathcal{O}_{1-}^g$ | $\mathcal{O}_{2-}^g$ | $\mathcal{O}_{2+}^h$ | $\mathcal{O}_{2-}^h$ |
| $(c,g,h):93$ | $R_T^{x'z}$ | $R_T^{x'x}$ | ${}^cR_{LT'}^{x'0}$ | ${}^sR_{LT}^{x'0}$ | ${}^sR_{LT'}^{x'x}$ | ${}^cR_{LT}^{x'x}$ |
| | $\mathcal{O}_{1+}^c$ | $\mathcal{O}_{2-}^c$ | $\mathcal{O}_{1-}^g$ | $\mathcal{O}_{2-}^g$ | $\mathcal{O}_{1+}^h$ | $\mathcal{O}_{2+}^h$ |
| $(c,g,h):94$ | $R_T^{x'z}$ | $R_T^{x'x}$ | ${}^cR_{LT'}^{x'0}$ | ${}^sR_{LT}^{x'0}$ | ${}^sR_{LT'}^{x'x}$ | ${}^sR_{LT'}^{z'x}$ |
| | $\mathcal{O}_{1+}^c$ | $\mathcal{O}_{2-}^c$ | $\mathcal{O}_{1-}^g$ | $\mathcal{O}_{2-}^g$ | $\mathcal{O}_{1+}^h$ | $\mathcal{O}_{2-}^h$ |
| $(c,g,h):95$ | $R_T^{x'z}$ | $R_T^{x'x}$ | ${}^cR_{LT'}^{x'0}$ | ${}^sR_{LT}^{x'0}$ | ${}^cR_{LT}^{z'x}$ | ${}^cR_{LT}^{x'x}$ |
| | $\mathcal{O}_{1+}^c$ | $\mathcal{O}_{2-}^c$ | $\mathcal{O}_{1-}^g$ | $\mathcal{O}_{2-}^g$ | $\mathcal{O}_{1-}^h$ | $\mathcal{O}_{2+}^h$ |
| $(c,g,h):96$ | $R_T^{x'z}$ | $R_T^{x'x}$ | ${}^cR_{LT'}^{x'0}$ | ${}^sR_{LT}^{x'0}$ | ${}^cR_{LT}^{z'x}$ | ${}^sR_{LT'}^{z'x}$ |
| | $\mathcal{O}_{1+}^c$ | $\mathcal{O}_{2-}^c$ | $\mathcal{O}_{1-}^g$ | $\mathcal{O}_{2-}^g$ | $\mathcal{O}_{1-}^h$ | $\mathcal{O}_{2-}^h$ |
| $(c,g,h):97$ | $R_T^{z'x}$ | $R_T^{z'z}$ | ${}^sR_{LT}^{z'0}$ | ${}^cR_{LT'}^{x'0}$ | ${}^sR_{LT'}^{x'x}$ | ${}^cR_{LT}^{z'x}$ |
| | $\mathcal{O}_{1-}^c$ | $\mathcal{O}_{2+}^c$ | $\mathcal{O}_{1+}^g$ | $\mathcal{O}_{1-}^g$ | $\mathcal{O}_{1+}^h$ | $\mathcal{O}_{1-}^h$ |
| $(c,g,h):98$ | $R_T^{z'x}$ | $R_T^{z'z}$ | ${}^sR_{LT}^{z'0}$ | ${}^cR_{LT'}^{x'0}$ | ${}^cR_{LT}^{x'x}$ | ${}^sR_{LT'}^{z'x}$ |
| | $\mathcal{O}_{1-}^c$ | $\mathcal{O}_{2+}^c$ | $\mathcal{O}_{1+}^g$ | $\mathcal{O}_{1-}^g$ | $\mathcal{O}_{2+}^h$ | $\mathcal{O}_{2-}^h$ |
| $(c,g,h):99$ | $R_T^{z'x}$ | $R_T^{z'z}$ | ${}^sR_{LT}^{z'0}$ | ${}^cR_{LT'}^{x'0}$ | ${}^sR_{LT'}^{x'x}$ | ${}^cR_{LT}^{x'x}$ |
| | $\mathcal{O}_{1-}^c$ | $\mathcal{O}_{2+}^c$ | $\mathcal{O}_{1+}^g$ | $\mathcal{O}_{1-}^g$ | $\mathcal{O}_{1+}^h$ | $\mathcal{O}_{2+}^h$ |

| | | | | | | |
|---|---|---|---|---|---|---|
| $(c, g, h) : 100$ | $R_T^{z'x}$ | $R_T^{z'z}$ | ${}^sR_{LT}^{z'0}$ | ${}^cR_{LT'}^{x'0}$ | ${}^sR_{LT'}^{x'x}$ | ${}^sR_{LT'}^{z'x}$ |
| | $\mathcal{O}_{1-}^c$ | $\mathcal{O}_{2+}^c$ | $\mathcal{O}_{1+}^g$ | $\mathcal{O}_{1-}^g$ | $\mathcal{O}_{1+}^h$ | $\mathcal{O}_{2-}^h$ |
| $(c, g, h) : 101$ | $R_T^{z'x}$ | $R_T^{z'z}$ | ${}^sR_{LT}^{z'0}$ | ${}^cR_{LT'}^{x'0}$ | ${}^cR_{LT}^{z'x}$ | ${}^cR_{LT}^{x'x}$ |
| | $\mathcal{O}_{1-}^c$ | $\mathcal{O}_{2+}^c$ | $\mathcal{O}_{1+}^g$ | $\mathcal{O}_{1-}^g$ | $\mathcal{O}_{1-}^h$ | $\mathcal{O}_{2+}^h$ |
| $(c, g, h) : 102$ | $R_T^{z'x}$ | $R_T^{z'z}$ | ${}^sR_{LT}^{z'0}$ | ${}^cR_{LT'}^{x'0}$ | ${}^cR_{LT}^{z'x}$ | ${}^sR_{LT'}^{z'x}$ |
| | $\mathcal{O}_{1-}^c$ | $\mathcal{O}_{2+}^c$ | $\mathcal{O}_{1+}^g$ | $\mathcal{O}_{1-}^g$ | $\mathcal{O}_{1-}^h$ | $\mathcal{O}_{2-}^h$ |
| $(c, g, h) : 103$ | $R_T^{z'x}$ | $R_T^{z'z}$ | ${}^cR_{LT'}^{z'0}$ | ${}^sR_{LT}^{x'0}$ | ${}^sR_{LT'}^{x'x}$ | ${}^cR_{LT}^{z'x}$ |
| | $\mathcal{O}_{1-}^c$ | $\mathcal{O}_{2+}^c$ | $\mathcal{O}_{2+}^g$ | $\mathcal{O}_{2-}^g$ | $\mathcal{O}_{1+}^h$ | $\mathcal{O}_{1-}^h$ |
| $(c, g, h) : 104$ | $R_T^{z'x}$ | $R_T^{z'z}$ | ${}^cR_{LT'}^{z'0}$ | ${}^sR_{LT}^{x'0}$ | ${}^cR_{LT}^{x'x}$ | ${}^sR_{LT'}^{z'x}$ |
| | $\mathcal{O}_{1-}^c$ | $\mathcal{O}_{2+}^c$ | $\mathcal{O}_{2+}^g$ | $\mathcal{O}_{2-}^g$ | $\mathcal{O}_{2+}^h$ | $\mathcal{O}_{2-}^h$ |
| $(c, g, h) : 105$ | $R_T^{z'x}$ | $R_T^{z'z}$ | ${}^cR_{LT'}^{z'0}$ | ${}^sR_{LT}^{x'0}$ | ${}^sR_{LT'}^{x'x}$ | ${}^cR_{LT}^{x'x}$ |
| | $\mathcal{O}_{1-}^c$ | $\mathcal{O}_{2+}^c$ | $\mathcal{O}_{2+}^g$ | $\mathcal{O}_{2-}^g$ | $\mathcal{O}_{1+}^h$ | $\mathcal{O}_{2+}^h$ |
| $(c, g, h) : 106$ | $R_T^{z'x}$ | $R_T^{z'z}$ | ${}^cR_{LT'}^{z'0}$ | ${}^sR_{LT}^{x'0}$ | ${}^sR_{LT'}^{x'x}$ | ${}^sR_{LT'}^{z'x}$ |
| | $\mathcal{O}_{1-}^c$ | $\mathcal{O}_{2+}^c$ | $\mathcal{O}_{2+}^g$ | $\mathcal{O}_{2-}^g$ | $\mathcal{O}_{1+}^h$ | $\mathcal{O}_{2-}^h$ |
| $(c, g, h) : 107$ | $R_T^{z'x}$ | $R_T^{z'z}$ | ${}^cR_{LT'}^{z'0}$ | ${}^sR_{LT}^{x'0}$ | ${}^cR_{LT}^{z'x}$ | ${}^cR_{LT}^{x'x}$ |
| | $\mathcal{O}_{1-}^c$ | $\mathcal{O}_{2+}^c$ | $\mathcal{O}_{2+}^g$ | $\mathcal{O}_{2-}^g$ | $\mathcal{O}_{1-}^h$ | $\mathcal{O}_{2+}^h$ |
| $(c, g, h) : 108$ | $R_T^{z'x}$ | $R_T^{z'z}$ | ${}^cR_{LT'}^{z'0}$ | ${}^sR_{LT}^{x'0}$ | ${}^cR_{LT}^{z'x}$ | ${}^sR_{LT'}^{z'x}$ |
| | $\mathcal{O}_{1-}^c$ | $\mathcal{O}_{2+}^c$ | $\mathcal{O}_{2+}^g$ | $\mathcal{O}_{2-}^g$ | $\mathcal{O}_{1-}^h$ | $\mathcal{O}_{2-}^h$ |
| $(c, g, h) : 109$ | $R_T^{z'x}$ | $R_T^{z'z}$ | ${}^sR_{LT}^{z'0}$ | ${}^cR_{LT'}^{z'0}$ | ${}^sR_{LT'}^{x'x}$ | ${}^cR_{LT}^{z'x}$ |
| | $\mathcal{O}_{1-}^c$ | $\mathcal{O}_{2+}^c$ | $\mathcal{O}_{1+}^g$ | $\mathcal{O}_{2+}^g$ | $\mathcal{O}_{1+}^h$ | $\mathcal{O}_{1-}^h$ |
| $(c, g, h) : 110$ | $R_T^{z'x}$ | $R_T^{z'z}$ | ${}^sR_{LT}^{z'0}$ | ${}^cR_{LT'}^{z'0}$ | ${}^cR_{LT}^{x'x}$ | ${}^sR_{LT'}^{z'x}$ |
| | $\mathcal{O}_{1-}^c$ | $\mathcal{O}_{2+}^c$ | $\mathcal{O}_{1+}^g$ | $\mathcal{O}_{2+}^g$ | $\mathcal{O}_{2+}^h$ | $\mathcal{O}_{2-}^h$ |
| $(c, g, h) : 111$ | $R_T^{z'x}$ | $R_T^{z'z}$ | ${}^sR_{LT}^{z'0}$ | ${}^cR_{LT'}^{z'0}$ | ${}^sR_{LT'}^{x'x}$ | ${}^cR_{LT}^{x'x}$ |
| | $\mathcal{O}_{1-}^c$ | $\mathcal{O}_{2+}^c$ | $\mathcal{O}_{1+}^g$ | $\mathcal{O}_{2+}^g$ | $\mathcal{O}_{1+}^h$ | $\mathcal{O}_{2+}^h$ |
| $(c, g, h) : 112$ | $R_T^{z'x}$ | $R_T^{z'z}$ | ${}^sR_{LT}^{z'0}$ | ${}^cR_{LT'}^{z'0}$ | ${}^sR_{LT'}^{x'x}$ | ${}^sR_{LT'}^{z'x}$ |
| | $\mathcal{O}_{1-}^c$ | $\mathcal{O}_{2+}^c$ | $\mathcal{O}_{1+}^g$ | $\mathcal{O}_{2+}^g$ | $\mathcal{O}_{1+}^h$ | $\mathcal{O}_{2-}^h$ |
| $(c, g, h) : 113$ | $R_T^{z'x}$ | $R_T^{z'z}$ | ${}^sR_{LT}^{z'0}$ | ${}^cR_{LT'}^{z'0}$ | ${}^cR_{LT}^{z'x}$ | ${}^cR_{LT}^{x'x}$ |
| | $\mathcal{O}_{1-}^c$ | $\mathcal{O}_{2+}^c$ | $\mathcal{O}_{1+}^g$ | $\mathcal{O}_{2+}^g$ | $\mathcal{O}_{1-}^h$ | $\mathcal{O}_{2+}^h$ |
| $(c, g, h) : 114$ | $R_T^{z'x}$ | $R_T^{z'z}$ | ${}^sR_{LT}^{z'0}$ | ${}^cR_{LT'}^{z'0}$ | ${}^cR_{LT}^{z'x}$ | ${}^sR_{LT'}^{z'x}$ |
| | $\mathcal{O}_{1-}^c$ | $\mathcal{O}_{2+}^c$ | $\mathcal{O}_{1+}^g$ | $\mathcal{O}_{2+}^g$ | $\mathcal{O}_{1-}^h$ | $\mathcal{O}_{2-}^h$ |
| $(c, g, h) : 115$ | $R_T^{z'x}$ | $R_T^{z'z}$ | ${}^sR_{LT}^{z'0}$ | ${}^sR_{LT}^{x'0}$ | ${}^sR_{LT'}^{x'x}$ | ${}^cR_{LT}^{z'x}$ |
| | $\mathcal{O}_{1-}^c$ | $\mathcal{O}_{2+}^c$ | $\mathcal{O}_{1+}^g$ | $\mathcal{O}_{2-}^g$ | $\mathcal{O}_{1+}^h$ | $\mathcal{O}_{1-}^h$ |
| $(c, g, h) : 116$ | $R_T^{z'x}$ | $R_T^{z'z}$ | ${}^sR_{LT}^{z'0}$ | ${}^sR_{LT}^{x'0}$ | ${}^cR_{LT}^{x'x}$ | ${}^sR_{LT'}^{z'x}$ |
| | $\mathcal{O}_{1-}^c$ | $\mathcal{O}_{2+}^c$ | $\mathcal{O}_{1+}^g$ | $\mathcal{O}_{2-}^g$ | $\mathcal{O}_{2+}^h$ | $\mathcal{O}_{2-}^h$ |
| $(c, g, h) : 117$ | $R_T^{z'x}$ | $R_T^{z'z}$ | ${}^sR_{LT}^{z'0}$ | ${}^sR_{LT}^{x'0}$ | ${}^sR_{LT'}^{x'x}$ | ${}^cR_{LT}^{x'x}$ |
| | $\mathcal{O}_{1-}^c$ | $\mathcal{O}_{2+}^c$ | $\mathcal{O}_{1+}^g$ | $\mathcal{O}_{2-}^g$ | $\mathcal{O}_{1+}^h$ | $\mathcal{O}_{2+}^h$ |
| $(c, g, h) : 118$ | $R_T^{z'x}$ | $R_T^{z'z}$ | ${}^sR_{LT}^{z'0}$ | ${}^sR_{LT}^{x'0}$ | ${}^sR_{LT'}^{x'x}$ | ${}^sR_{LT'}^{z'x}$ |
| | $\mathcal{O}_{1-}^c$ | $\mathcal{O}_{2+}^c$ | $\mathcal{O}_{1+}^g$ | $\mathcal{O}_{2-}^g$ | $\mathcal{O}_{1+}^h$ | $\mathcal{O}_{2-}^h$ |
| $(c, g, h) : 119$ | $R_T^{z'x}$ | $R_T^{z'z}$ | ${}^sR_{LT}^{z'0}$ | ${}^sR_{LT}^{x'0}$ | ${}^cR_{LT}^{z'x}$ | ${}^cR_{LT}^{x'x}$ |
| | $\mathcal{O}_{1-}^c$ | $\mathcal{O}_{2+}^c$ | $\mathcal{O}_{1+}^g$ | $\mathcal{O}_{2-}^g$ | $\mathcal{O}_{1-}^h$ | $\mathcal{O}_{2+}^h$ |
| $(c, g, h) : 120$ | $R_T^{z'x}$ | $R_T^{z'z}$ | ${}^sR_{LT}^{z'0}$ | ${}^sR_{LT}^{x'0}$ | ${}^cR_{LT}^{z'x}$ | ${}^sR_{LT'}^{z'x}$ |
| | $\mathcal{O}_{1-}^c$ | $\mathcal{O}_{2+}^c$ | $\mathcal{O}_{1+}^g$ | $\mathcal{O}_{2-}^g$ | $\mathcal{O}_{1-}^h$ | $\mathcal{O}_{2-}^h$ |
| $(c, g, h) : 121$ | $R_T^{z'x}$ | $R_T^{z'z}$ | ${}^cR_{LT'}^{x'0}$ | ${}^cR_{LT'}^{z'0}$ | ${}^sR_{LT'}^{x'x}$ | ${}^cR_{LT}^{z'x}$ |
| | $\mathcal{O}_{1-}^c$ | $\mathcal{O}_{2+}^c$ | $\mathcal{O}_{1-}^g$ | $\mathcal{O}_{2+}^g$ | $\mathcal{O}_{1+}^h$ | $\mathcal{O}_{1-}^h$ |
| $(c, g, h) : 122$ | $R_T^{z'x}$ | $R_T^{z'z}$ | ${}^cR_{LT'}^{x'0}$ | ${}^cR_{LT'}^{z'0}$ | ${}^cR_{LT}^{x'x}$ | ${}^sR_{LT'}^{z'x}$ |
| | $\mathcal{O}_{1-}^c$ | $\mathcal{O}_{2+}^c$ | $\mathcal{O}_{1-}^g$ | $\mathcal{O}_{2+}^g$ | $\mathcal{O}_{2+}^h$ | $\mathcal{O}_{2-}^h$ |
| $(c, g, h) : 123$ | $R_T^{z'x}$ | $R_T^{z'z}$ | ${}^cR_{LT'}^{x'0}$ | ${}^cR_{LT'}^{z'0}$ | ${}^sR_{LT'}^{x'x}$ | ${}^cR_{LT}^{x'x}$ |
| | $\mathcal{O}_{1-}^c$ | $\mathcal{O}_{2+}^c$ | $\mathcal{O}_{1-}^g$ | $\mathcal{O}_{2+}^g$ | $\mathcal{O}_{1+}^h$ | $\mathcal{O}_{2+}^h$ |
| $(c, g, h) : 124$ | $R_T^{z'x}$ | $R_T^{z'z}$ | ${}^cR_{LT'}^{x'0}$ | ${}^cR_{LT'}^{z'0}$ | ${}^sR_{LT'}^{x'x}$ | ${}^sR_{LT'}^{z'x}$ |
| | $\mathcal{O}_{1-}^c$ | $\mathcal{O}_{2+}^c$ | $\mathcal{O}_{1-}^g$ | $\mathcal{O}_{2+}^g$ | $\mathcal{O}_{1+}^h$ | $\mathcal{O}_{2-}^h$ |
| $(c, g, h) : 125$ | $R_T^{z'x}$ | $R_T^{z'z}$ | ${}^cR_{LT'}^{x'0}$ | ${}^cR_{LT'}^{z'0}$ | ${}^cR_{LT}^{z'x}$ | ${}^cR_{LT}^{x'x}$ |
| | $\mathcal{O}_{1-}^c$ | $\mathcal{O}_{2+}^c$ | $\mathcal{O}_{1-}^g$ | $\mathcal{O}_{2+}^g$ | $\mathcal{O}_{1-}^h$ | $\mathcal{O}_{2+}^h$ |
| $(c, g, h) : 126$ | $R_T^{z'x}$ | $R_T^{z'z}$ | ${}^cR_{LT'}^{x'0}$ | ${}^cR_{LT'}^{z'0}$ | ${}^cR_{LT}^{z'x}$ | ${}^sR_{LT'}^{z'x}$ |
| | $\mathcal{O}_{1-}^c$ | $\mathcal{O}_{2+}^c$ | $\mathcal{O}_{1-}^g$ | $\mathcal{O}_{2+}^g$ | $\mathcal{O}_{1-}^h$ | $\mathcal{O}_{2-}^h$ |
| $(c, g, h) : 127$ | $R_T^{z'x}$ | $R_T^{z'z}$ | ${}^cR_{LT'}^{x'0}$ | ${}^sR_{LT}^{x'0}$ | ${}^sR_{LT'}^{x'x}$ | ${}^cR_{LT}^{z'x}$ |
| | $\mathcal{O}_{1-}^c$ | $\mathcal{O}_{2+}^c$ | $\mathcal{O}_{1-}^g$ | $\mathcal{O}_{2-}^g$ | $\mathcal{O}_{1+}^h$ | $\mathcal{O}_{1-}^h$ |

| | | | | | | |
|---|---|---|---|---|---|---|
| $(c,g,h):128$ | $R_T^{z'x}$ | $R_T^{z'z}$ | $^{c}R_{LT'}^{x'0}$ | $^{s}R_{LT}^{x'0}$ | $^{c}R_{LT}^{x'x}$ | $^{s}R_{LT'}^{z'x}$ |
| | $\mathcal{O}_{1-}^{c}$ | $\mathcal{O}_{2+}^{c}$ | $\mathcal{O}_{1-}^{g}$ | $\mathcal{O}_{2-}^{g}$ | $\mathcal{O}_{2+}^{h}$ | $\mathcal{O}_{2-}^{h}$ |
| $(c,g,h):129$ | $R_T^{z'x}$ | $R_T^{z'z}$ | $^{c}R_{LT'}^{x'0}$ | $^{s}R_{LT}^{x'0}$ | $^{s}R_{LT'}^{x'x}$ | $^{c}R_{LT}^{x'x}$ |
| | $\mathcal{O}_{1-}^{c}$ | $\mathcal{O}_{2+}^{c}$ | $\mathcal{O}_{1-}^{g}$ | $\mathcal{O}_{2-}^{g}$ | $\mathcal{O}_{1+}^{h}$ | $\mathcal{O}_{2+}^{h}$ |
| $(c,g,h):130$ | $R_T^{z'x}$ | $R_T^{z'z}$ | $^{c}R_{LT'}^{x'0}$ | $^{s}R_{LT}^{x'0}$ | $^{s}R_{LT'}^{x'x}$ | $^{s}R_{LT'}^{z'x}$ |
| | $\mathcal{O}_{1-}^{c}$ | $\mathcal{O}_{2+}^{c}$ | $\mathcal{O}_{1-}^{g}$ | $\mathcal{O}_{2-}^{g}$ | $\mathcal{O}_{1+}^{h}$ | $\mathcal{O}_{2-}^{h}$ |
| $(c,g,h):131$ | $R_T^{z'x}$ | $R_T^{z'z}$ | $^{c}R_{LT'}^{x'0}$ | $^{s}R_{LT}^{x'0}$ | $^{c}R_{LT}^{z'x}$ | $^{c}R_{LT}^{x'x}$ |
| | $\mathcal{O}_{1-}^{c}$ | $\mathcal{O}_{2+}^{c}$ | $\mathcal{O}_{1-}^{g}$ | $\mathcal{O}_{2-}^{g}$ | $\mathcal{O}_{1-}^{h}$ | $\mathcal{O}_{2+}^{h}$ |
| $(c,g,h):132$ | $R_T^{z'x}$ | $R_T^{z'z}$ | $^{c}R_{LT'}^{x'0}$ | $^{s}R_{LT}^{x'0}$ | $^{c}R_{LT}^{z'x}$ | $^{s}R_{LT'}^{z'x}$ |
| | $\mathcal{O}_{1-}^{c}$ | $\mathcal{O}_{2+}^{c}$ | $\mathcal{O}_{1-}^{g}$ | $\mathcal{O}_{2-}^{g}$ | $\mathcal{O}_{1-}^{h}$ | $\mathcal{O}_{2-}^{h}$ |
| $(c,g,h):133$ | $R_T^{z'x}$ | $R_T^{x'x}$ | $^{s}R_{LT}^{z'0}$ | $^{c}R_{LT'}^{x'0}$ | $^{s}R_{LT'}^{x'x}$ | $^{s}R_{LT'}^{z'x}$ |
| | $\mathcal{O}_{1-}^{c}$ | $\mathcal{O}_{2-}^{c}$ | $\mathcal{O}_{1+}^{g}$ | $\mathcal{O}_{1-}^{g}$ | $\mathcal{O}_{1+}^{h}$ | $\mathcal{O}_{2-}^{h}$ |
| $(c,g,h):134$ | $R_T^{z'x}$ | $R_T^{x'x}$ | $^{s}R_{LT}^{z'0}$ | $^{c}R_{LT'}^{x'0}$ | $^{c}R_{LT}^{z'x}$ | $^{c}R_{LT}^{x'x}$ |
| | $\mathcal{O}_{1-}^{c}$ | $\mathcal{O}_{2-}^{c}$ | $\mathcal{O}_{1+}^{g}$ | $\mathcal{O}_{1-}^{g}$ | $\mathcal{O}_{1-}^{h}$ | $\mathcal{O}_{2+}^{h}$ |
| $(c,g,h):135$ | $R_T^{z'x}$ | $R_T^{x'x}$ | $^{c}R_{LT'}^{z'0}$ | $^{s}R_{LT}^{x'0}$ | $^{s}R_{LT'}^{x'x}$ | $^{s}R_{LT'}^{z'x}$ |
| | $\mathcal{O}_{1-}^{c}$ | $\mathcal{O}_{2-}^{c}$ | $\mathcal{O}_{2+}^{g}$ | $\mathcal{O}_{2-}^{g}$ | $\mathcal{O}_{1+}^{h}$ | $\mathcal{O}_{2-}^{h}$ |
| $(c,g,h):136$ | $R_T^{z'x}$ | $R_T^{x'x}$ | $^{c}R_{LT'}^{z'0}$ | $^{s}R_{LT}^{x'0}$ | $^{c}R_{LT}^{z'x}$ | $^{c}R_{LT}^{x'x}$ |
| | $\mathcal{O}_{1-}^{c}$ | $\mathcal{O}_{2-}^{c}$ | $\mathcal{O}_{2+}^{g}$ | $\mathcal{O}_{2-}^{g}$ | $\mathcal{O}_{1-}^{h}$ | $\mathcal{O}_{2+}^{h}$ |
| $(c,g,h):137$ | $R_T^{z'x}$ | $R_T^{x'x}$ | $^{s}R_{LT}^{z'0}$ | $^{c}R_{LT'}^{z'0}$ | $^{s}R_{LT'}^{x'x}$ | $^{s}R_{LT'}^{z'x}$ |
| | $\mathcal{O}_{1-}^{c}$ | $\mathcal{O}_{2-}^{c}$ | $\mathcal{O}_{1+}^{g}$ | $\mathcal{O}_{2+}^{g}$ | $\mathcal{O}_{1+}^{h}$ | $\mathcal{O}_{2-}^{h}$ |
| $(c,g,h):138$ | $R_T^{z'x}$ | $R_T^{x'x}$ | $^{s}R_{LT}^{z'0}$ | $^{c}R_{LT'}^{z'0}$ | $^{c}R_{LT}^{z'x}$ | $^{c}R_{LT}^{x'x}$ |
| | $\mathcal{O}_{1-}^{c}$ | $\mathcal{O}_{2-}^{c}$ | $\mathcal{O}_{1+}^{g}$ | $\mathcal{O}_{2+}^{g}$ | $\mathcal{O}_{1-}^{h}$ | $\mathcal{O}_{2+}^{h}$ |
| $(c,g,h):139$ | $R_T^{z'x}$ | $R_T^{x'x}$ | $^{s}R_{LT}^{z'0}$ | $^{s}R_{LT}^{x'0}$ | $^{s}R_{LT'}^{x'x}$ | $^{c}R_{LT}^{z'x}$ |
| | $\mathcal{O}_{1-}^{c}$ | $\mathcal{O}_{2-}^{c}$ | $\mathcal{O}_{1+}^{g}$ | $\mathcal{O}_{2-}^{g}$ | $\mathcal{O}_{1+}^{h}$ | $\mathcal{O}_{1-}^{h}$ |
| $(c,g,h):140$ | $R_T^{z'x}$ | $R_T^{x'x}$ | $^{s}R_{LT}^{z'0}$ | $^{s}R_{LT}^{x'0}$ | $^{c}R_{LT}^{x'x}$ | $^{s}R_{LT'}^{z'x}$ |
| | $\mathcal{O}_{1-}^{c}$ | $\mathcal{O}_{2-}^{c}$ | $\mathcal{O}_{1+}^{g}$ | $\mathcal{O}_{2-}^{g}$ | $\mathcal{O}_{2+}^{h}$ | $\mathcal{O}_{2-}^{h}$ |
| $(c,g,h):141$ | $R_T^{z'x}$ | $R_T^{x'x}$ | $^{s}R_{LT}^{z'0}$ | $^{s}R_{LT}^{x'0}$ | $^{s}R_{LT'}^{x'x}$ | $^{c}R_{LT}^{x'x}$ |
| | $\mathcal{O}_{1-}^{c}$ | $\mathcal{O}_{2-}^{c}$ | $\mathcal{O}_{1+}^{g}$ | $\mathcal{O}_{2-}^{g}$ | $\mathcal{O}_{1+}^{h}$ | $\mathcal{O}_{2+}^{h}$ |
| $(c,g,h):142$ | $R_T^{z'x}$ | $R_T^{x'x}$ | $^{s}R_{LT}^{z'0}$ | $^{s}R_{LT}^{x'0}$ | $^{s}R_{LT'}^{x'x}$ | $^{s}R_{LT'}^{z'x}$ |
| | $\mathcal{O}_{1-}^{c}$ | $\mathcal{O}_{2-}^{c}$ | $\mathcal{O}_{1+}^{g}$ | $\mathcal{O}_{2-}^{g}$ | $\mathcal{O}_{1+}^{h}$ | $\mathcal{O}_{2-}^{h}$ |
| $(c,g,h):143$ | $R_T^{z'x}$ | $R_T^{x'x}$ | $^{s}R_{LT}^{z'0}$ | $^{s}R_{LT}^{x'0}$ | $^{c}R_{LT}^{z'x}$ | $^{c}R_{LT}^{x'x}$ |
| | $\mathcal{O}_{1-}^{c}$ | $\mathcal{O}_{2-}^{c}$ | $\mathcal{O}_{1+}^{g}$ | $\mathcal{O}_{2-}^{g}$ | $\mathcal{O}_{1-}^{h}$ | $\mathcal{O}_{2+}^{h}$ |
| $(c,g,h):144$ | $R_T^{z'x}$ | $R_T^{x'x}$ | $^{s}R_{LT}^{z'0}$ | $^{s}R_{LT}^{x'0}$ | $^{c}R_{LT}^{z'x}$ | $^{s}R_{LT'}^{z'x}$ |
| | $\mathcal{O}_{1-}^{c}$ | $\mathcal{O}_{2-}^{c}$ | $\mathcal{O}_{1+}^{g}$ | $\mathcal{O}_{2-}^{g}$ | $\mathcal{O}_{1-}^{h}$ | $\mathcal{O}_{2-}^{h}$ |
| $(c,g,h):145$ | $R_T^{z'x}$ | $R_T^{x'x}$ | $^{c}R_{LT'}^{x'0}$ | $^{c}R_{LT'}^{z'0}$ | $^{s}R_{LT'}^{x'x}$ | $^{c}R_{LT}^{z'x}$ |
| | $\mathcal{O}_{1-}^{c}$ | $\mathcal{O}_{2-}^{c}$ | $\mathcal{O}_{1-}^{g}$ | $\mathcal{O}_{2+}^{g}$ | $\mathcal{O}_{1+}^{h}$ | $\mathcal{O}_{1-}^{h}$ |
| $(c,g,h):146$ | $R_T^{z'x}$ | $R_T^{x'x}$ | $^{c}R_{LT'}^{x'0}$ | $^{c}R_{LT'}^{z'0}$ | $^{c}R_{LT}^{x'x}$ | $^{s}R_{LT'}^{z'x}$ |
| | $\mathcal{O}_{1-}^{c}$ | $\mathcal{O}_{2-}^{c}$ | $\mathcal{O}_{1-}^{g}$ | $\mathcal{O}_{2+}^{g}$ | $\mathcal{O}_{2+}^{h}$ | $\mathcal{O}_{2-}^{h}$ |
| $(c,g,h):147$ | $R_T^{z'x}$ | $R_T^{x'x}$ | $^{c}R_{LT'}^{x'0}$ | $^{c}R_{LT'}^{z'0}$ | $^{s}R_{LT'}^{x'x}$ | $^{c}R_{LT}^{x'x}$ |
| | $\mathcal{O}_{1-}^{c}$ | $\mathcal{O}_{2-}^{c}$ | $\mathcal{O}_{1-}^{g}$ | $\mathcal{O}_{2+}^{g}$ | $\mathcal{O}_{1+}^{h}$ | $\mathcal{O}_{2+}^{h}$ |
| $(c,g,h):148$ | $R_T^{z'x}$ | $R_T^{x'x}$ | $^{c}R_{LT'}^{x'0}$ | $^{c}R_{LT'}^{z'0}$ | $^{s}R_{LT'}^{x'x}$ | $^{s}R_{LT'}^{z'x}$ |
| | $\mathcal{O}_{1-}^{c}$ | $\mathcal{O}_{2-}^{c}$ | $\mathcal{O}_{1-}^{g}$ | $\mathcal{O}_{2+}^{g}$ | $\mathcal{O}_{1+}^{h}$ | $\mathcal{O}_{2-}^{h}$ |
| $(c,g,h):149$ | $R_T^{z'x}$ | $R_T^{x'x}$ | $^{c}R_{LT'}^{x'0}$ | $^{c}R_{LT'}^{z'0}$ | $^{c}R_{LT}^{z'x}$ | $^{c}R_{LT}^{x'x}$ |
| | $\mathcal{O}_{1-}^{c}$ | $\mathcal{O}_{2-}^{c}$ | $\mathcal{O}_{1-}^{g}$ | $\mathcal{O}_{2+}^{g}$ | $\mathcal{O}_{1-}^{h}$ | $\mathcal{O}_{2+}^{h}$ |
| $(c,g,h):150$ | $R_T^{z'x}$ | $R_T^{x'x}$ | $^{c}R_{LT'}^{x'0}$ | $^{c}R_{LT'}^{z'0}$ | $^{c}R_{LT}^{z'x}$ | $^{s}R_{LT'}^{z'x}$ |
| | $\mathcal{O}_{1-}^{c}$ | $\mathcal{O}_{2-}^{c}$ | $\mathcal{O}_{1-}^{g}$ | $\mathcal{O}_{2+}^{g}$ | $\mathcal{O}_{1-}^{h}$ | $\mathcal{O}_{2-}^{h}$ |
| $(c,g,h):151$ | $R_T^{z'x}$ | $R_T^{x'x}$ | $^{c}R_{LT'}^{x'0}$ | $^{s}R_{LT}^{x'0}$ | $^{s}R_{LT'}^{x'x}$ | $^{s}R_{LT'}^{z'x}$ |
| | $\mathcal{O}_{1-}^{c}$ | $\mathcal{O}_{2-}^{c}$ | $\mathcal{O}_{1-}^{g}$ | $\mathcal{O}_{2-}^{g}$ | $\mathcal{O}_{1+}^{h}$ | $\mathcal{O}_{2-}^{h}$ |
| $(c,g,h):152$ | $R_T^{z'x}$ | $R_T^{x'x}$ | $^{c}R_{LT'}^{x'0}$ | $^{s}R_{LT}^{x'0}$ | $^{c}R_{LT}^{z'x}$ | $^{c}R_{LT}^{x'x}$ |
| | $\mathcal{O}_{1-}^{c}$ | $\mathcal{O}_{2-}^{c}$ | $\mathcal{O}_{1-}^{g}$ | $\mathcal{O}_{2-}^{g}$ | $\mathcal{O}_{1-}^{h}$ | $\mathcal{O}_{2+}^{h}$ |

[1] K. Nakayama, Phys. Rev. C **100**, no. 3, 035208 (2019) doi:10.1103/PhysRevC.100.035208 [arXiv:1809.00335 [nucl-th]].
[2] W. T. Chiang and F. Tabakin, Phys. Rev. C **55**, 2054 (1997) doi:10.1103/PhysRevC.55.2054 [nucl-th/9611053].
[3] Wolfram Research, Inc., Mathematica, Version 12.0, Champaign, IL (2019).
[4] L. Tiator, R. L. Workman, Y. Wunderlich and H. Haberzettl, Phys. Rev. C **96**, no. 2, 025210 (2017) doi:10.1103/PhysRevC.96.025210 [arXiv:1702.08375 [nucl-th]].
[5] Y. Wunderlich, P. Kroenert, F. Afzal and A. Thiel, Phys. Rev. C **102**, no.3, 034605 (2020) doi:10.1103/PhysRevC.102.034605 [arXiv:2004.14483 [nucl-th]].
